# Supplementary material for: Dynamic Importance in Diffusion U-Net for Enhanced Image Synthesis
Source: arXiv:2504.03471 source file (2025-05-05)
Supplement: Supplementary file 1 [file appendix.tex]

\clearpage

\newcommand{\secondtitle}[1]{
  \twocolumn[
    \centering\normalfont
    \Huge#1
    \vspace{1\baselineskip}
  ]
}

\secondtitle{Appendix}

% ----------

% 将标题 "Appendix" 添加到目录中
\addcontentsline{toc}{section}{Appendix}

% 设置目录深度
\setcounter{tocdepth}{1}

% 设置编号宽度

% 生成目录
\tableofcontents

% \newpage

% ----------
\vspace{10cm}
This appendix provides supplementary material that supports and extends the content presented in the main paper. 
The contents of the appendix are organized as follows:

\begin{itemize}
    \item Sec.~\ref{appx_sec-supplementary_proof_and_analysis_of_proposition_1} derives the variance of noise prediction error and analyzes the fundamental principles of our re-weighting strategy from the perspective of signal-to-noise ratio (SNR).

    \item Sect.~\ref{appx_sec-theory_experiment_consistency_analysis} discusses the consistency between the experimental results and the theoretical analysis. 

    \item Sec.~\ref{appx_sec-the_methodology_and_implementation_of_importance_probe} provides more details of our proposed Importance Probe (IP). 
    
    \item Sec.~\ref{appx_sec-experimental_setup_and_model_configuration} outlines the pre-trained models, computational libraries, and metric computations used in our experiments.

    \item Sec.~\ref{appx_sec-the_methodology_and_evaluation_of_dynamic_attention_pruning_tests} provides more details of our dynamic attention pruning tests, including the strategy design mechanism and more experimental results.  

    \item Sec.~\ref{appx_sec-empirical_analysis_of_synthesis_improvements} presents the qualitative results of our proposed re-weighting strategy, and discusses the impact of the hyper-parameters involved. 
    
    \item Sec.~\ref{appx_sec-limitations_and_future_work} discusses the limitations of our approach and potential directions for future work. 
\end{itemize}

\newpage

% ----------

% More Discussion on Proposition 1
\setcounter{proposition}{0}

\section{Supplementary Proof and Analysis of Proposition 1}
\label{appx_sec-supplementary_proof_and_analysis_of_proposition_1}

We first prove Prop. ~\ref{prop-reweighting} in the main paper, and provide more discussion. 

\begin{proposition}
    \label{prop-reweighting_appx}
    
    (Prop.~\ref{prop-reweighting} in the main paper) The variance of the error
    \begin{equation}
        \label{eq-the_variance_of_error_appx}
        \begin{split}
            & \text{Var}(\Delta \hat{\pmb{\epsilon}}) 
            \approx \textstyle\sum_i A_i^2 (w_i - 1)^2 
            \text{Var} (\pmb{g}_i (\pmb{\epsilon}) )
            \\ 
            &~~~~ + 
            \textstyle\sum_i A_i^2 w_i^2 \text{Var}(\pmb{f}_i (\pmb{x}_0)) 
            + 
            \textstyle\sum_i A_i^2 w_i^2 \text{Var}(\pmb{n}_i)
            , 
        \end{split}
    \end{equation}
    where $A_i$ denotes the mapping transformation from the output of the $i$-th Transformer block to the final noise prediction. 
\end{proposition}

\subsection{Preliminary} 

Given a clean sample $\pmb{x}_0$ and a variance schedule $\{\overline{\alpha}_i\}_{i = 1}^n$, the forward process of DDIM~\cite{song2022denoisingdiffusionimplicitmodels} can be written as
\begin{equation}
    \pmb{x}_t 
    = 
    \sqrt{\overline{\alpha}_t} \pmb{x}_0 + \sqrt{1 - \overline{\alpha}_t} \pmb{\epsilon}
    , 
\end{equation}
where $\pmb{\epsilon} \sim \mathcal{N}(\pmb{0}, \pmb{I})$ is the true noise. 

The deterministic reverse step is
\begin{equation}
    \pmb{x}_{t - 1}
    = 
    \sqrt{\overline{\alpha}_{t - 1}} \left(\dfrac{\pmb{x}_t - \sqrt{1 - \overline{\alpha}_t} \hat{\pmb{\epsilon}}_t}{\sqrt{\overline{\alpha}_t}}\right) + \sqrt{1 - \overline{\alpha}_{t - 1}} \hat{\pmb{\epsilon}}_t
    , 
\end{equation}
where $\hat{\pmb{\epsilon}}_t = \pmb{\epsilon}_\theta (\pmb{x}_t, t)$ represents the noise predicted by the U-Net parameterized by $\theta$ at time step $t$. 

The signal-to-noise ratio (SNR) in this single step is defined as
\begin{equation}
    \text{SNR} (\pmb{x}_t) 
    = 
    \dfrac{||\pmb{x}_0||^2}{\text{Var} (\Delta\pmb{\epsilon}_t)}
    = 
    \dfrac{||\pmb{x}_0||^2}{\text{Var} (\pmb{\epsilon} - \hat{\pmb{\epsilon}}_t)}
    , 
\end{equation}
where the numerator $||\pmb{x}_0||^2$ represents the \emph{power} of the true signal $\pmb{x}_0$, and the denominator $\Delta \pmb{\epsilon}_t = \pmb{\epsilon} - \hat{\pmb{\epsilon}}_t$ denotes the \emph{error} between the true noise $\pmb{\epsilon}$ and the predicted noise $\hat{\pmb{\epsilon}}_t$. 

% 双栏
\begin{table*}[t]
    \caption{
        (Tab.~\ref{tab-comparison_between_different_models_and_steps} in the main paper) 
        Comparison between different models and inference steps. 
        Cells with a red/orange/yellow background indicate the best/second-best/third-best performance, respectively.  
        Cells where the weighted performance is worse than the vanilla schedule are marked with a downward arrow $\downarrow$. 
        Blocks within the SD/SDXL family are numbered from 0/1 for symmetry. 
    }
    \centering
    \begin{tabular}{c | c c c : c c c | c c c : c c c}
        \hline
        \multirow{2}{*}{\textbf{Weighting}} &
        \multicolumn{3}{c:}{\textbf{SD-Turbo}} & 
        \multicolumn{3}{c|}{\textbf{SDXL-Turbo}} & 
        \multicolumn{3}{c:}{\textbf{SD v2.1}} & 
        \multicolumn{3}{c}{\textbf{SDXL}} \\
        ~ & 1 & 2 & 3 & 1 & 2 & 3 &
        10 & 15 & 20 & 10 & 15 & 20 \\

        \hline
        Vanilla & 
        0.2961 & 0.3059 & 0.3034 & 
        0.2587 & 0.2693 & 0.2666 & 
        0.2876 & 0.2908 & 0.2932 & 
        0.2830 & \tbest{0.2889} & \tbest{0.2904} \\

        \hdashline

        blk-0 & 
        \sbest{0.2987} & \best{0.3088} & \tbest{0.3045} & 
        / & / & / & 
        0.2860$\downarrow$ & 0.2915 & \sbest{0.2946} & 
        / & / & / \\
        
        blk-1 & 
        \best{0.2993} & 0.3066 & 0.3019$\downarrow$ & 
        \best{0.2591} & 0.2685$\downarrow$ & 0.2666 & 
        \tbest{0.2881} & 0.2908 & \tbest{0.2943} & 
        \sbest{0.2863} & \best{0.2907} & \best{0.2924} \\
        
        blk-2 & 
        0.2966 & 0.3065 & 0.3037 & 
        0.2584$\downarrow$ & 0.2686$\downarrow$ & 0.2661$\downarrow$ & 
        0.2880 & 0.2896$\downarrow$ & 0.2935 & 
        0.2842 & 0.2886$\downarrow$ & 0.2889$\downarrow$ \\
        
        blk-3 & 
        0.2962 & 0.3055$\downarrow$ & 0.3035 & 
        \sbest{0.2589} & \best{0.2697} & \tbest{0.2668} & 
        0.2876 & 0.2909 & 0.2934 & 
        0.2839 & 0.2877$\downarrow$ & 0.2898$\downarrow$ \\
        
        blk-4 & 
        0.2965 & \sbest{0.3074} & \sbest{0.3052} & 
        \tbest{0.2588} & \sbest{0.2695} & \best{0.2671} & 
        \sbest{0.2894} & \tbest{0.2917} & 0.2939 & 
        \tbest{0.2851} & \tbest{0.2889} & 0.2892$\downarrow$ \\
        
        blk-5 & 
        \tbest{0.2981} & 0.3066 & \best{0.3062} & 
        0.2576$\downarrow$ & \tbest{0.2694} & \sbest{0.2670} & 
        \best{0.2902} & \best{0.2923} & \best{0.2950} & 
        \best{0.2868} & \sbest{0.2904} & \best{0.2910} \\
        
        blk-6 & 
        0.2962 & \tbest{0.3072} & 0.3025$\downarrow$ & 
        / & / & / & 
        0.2880 & \sbest{0.2919} & 0.2927$\downarrow$ & 
        / & / & / \\
        
        \hline
    \end{tabular}
    \label{tab-comparison_between_different_models_and_steps_appx}
\end{table*}

\subsection{Modeling the Noise Prediction in U-Net} 

The Transformer blocks~\cite{vaswani2023attentionneed} within the U-Net~\cite{ronneberger2015unetconvolutionalnetworksbiomedical, petit2021unettransformerselfcross} process the input $\pmb{x}_t$, whose output contains features associated with both the signal components and the noise components. 
Specifically, the output of the $i$-th Transformer block can be modeled as
\begin{equation}
    \pmb{y}_i 
    = 
    \pmb{f}_i (\pmb{x}_0) + \pmb{g}_i (\pmb{\epsilon}) + \pmb{n}_i
    , 
\end{equation}
where:

\begin{itemize}
    \item $\pmb{f}_i (\pmb{x}_0)$: The feature components related to the signal $\pmb{x}_0$. 

    \item $\pmb{g}_i (\pmb{\epsilon})$: The feature components related to the noise $\pmb{\epsilon}$. 

    \item $\pmb{n}_i$: The intrinsic noise of the Transformer block, which is introduced by approximation errors or nonlinearities within the block. 
\end{itemize}

The attention mechanisms within the pre-trained Transformer blocks, including self-attention and cross-attention, are capable of distinguishing between the signal and the noise components in the input latent. 
As a result, $\pmb{f}_i (\pmb{x}_0)$ primarily captures the signal information, while $\pmb{g}_i (\pmb{\epsilon})$ mainly captures the noise information. 
These two components are not independent, as both are influenced by the noisy input $\pmb{x}_t$. 

For simplicity, we assume that: 

\begin{itemize}
    \item The signal components $\pmb{f}_i (\pmb{x}_0)$s of all Transformer blocks are independent of each other, so do the noise components $\pmb{g}_i (\pmb{\epsilon})$s. 
    
     \item$\pmb{f}_i (\pmb{x}_0)$ is independent of $\pmb{g}_j (\pmb{\epsilon})$ for any $(i, j)$ pair. 

    \item $\pmb{n}_i$ has zero mean and a fixed variance $\text{Var} (\pmb{n}_i)$. 

    \item The intrinsic errors $\pmb{n}_i$s of all Transformer blocks are independent of each other, as well as independent of the true noise $\pmb{\epsilon}$ and the noise prediction $\pmb{\epsilon}_t$. 
\end{itemize}

The output $\pmb{y}_i$ of each Transformer block in processed by the subsequent blocks (such as ResNet~\cite{he2016deep} blocks), ultimately forming the noise prediction of the U-Net: 
\begin{equation}
    \hat{\pmb{\epsilon}}_t 
    = 
    \pmb{h}(\{\pmb{y}_i\})
    .
\end{equation}

For simplicity, we assume that $\pmb{h}(\cdot)$ is a linear combination of the outputs from the Transformer blocks: 
\begin{equation}
    \hat{\pmb{\epsilon}}_t 
    = 
    \sum_i A_i \pmb{y}_i
    = 
    \sum_i A_i (\pmb{f}_i (\pmb{x}_0) + \pmb{g}_i (\pmb{\epsilon}) + \pmb{n}_i)
    ,
\end{equation}
where $A_i$ denotes the mapping transformation from the output of the $i$-th Transformer block to the final noise prediction. 

\subsection{Re-weighting the Output of Transformer Blocks}

We propose to re-weight the output of the $i$-th $(i = 0, 1, \cdots)$ Transformer block by a scaling factor $w_i > 0$ before passing it to the subsequent ResNet block (see Fig.~\ref{fig-weighted_u_net_appx}). 

After re-weighting, the output of the $i$-th Transformer block becomes
\begin{equation}
    \pmb{y}_i' 
    = 
    w_i \pmb{y}_i, 
\end{equation}
while the noise prediction becomes
\begin{equation}
    \hat{\pmb{\epsilon}}_t' 
    = 
    \sum_i A_i \pmb{y}_i'
    = 
    \sum_i A_i w_i (\pmb{f}_i (\pmb{x}_0) + \pmb{g}_i (\pmb{\epsilon}) + \pmb{n}_i)
    .
\end{equation}

% 图: U-Net 加权
\begin{figure}[h]
    \centering
    \includegraphics[width=0.98\linewidth]{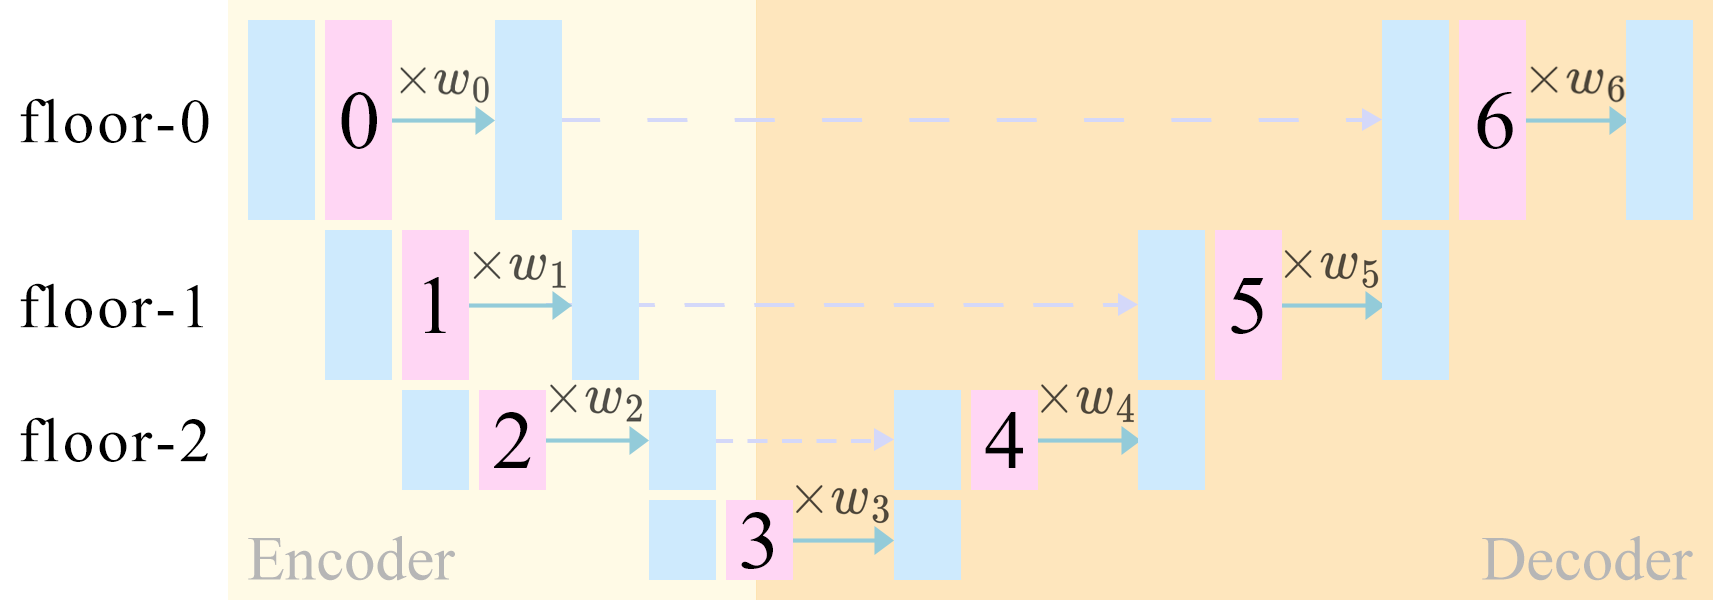}
    \caption{
        (Fig. 1 in the main paper) 
        Schematic of scaling the outputs of seven Transformer blocks before passing to the subsequent ResNet~\cite{he2016deep} blocks. 
        The blue rectangles represent the ResNet blocks, while the pink ones stand for the Transformer blocks. 
    }
    \label{fig-weighted_u_net_appx}
\end{figure}

\subsection{The Impact of Re-weighting on SNR}

The prediction error
\begin{equation}
    \Delta \hat{\pmb{\epsilon}}_t' 
    = 
    \pmb{\epsilon} - \hat{\pmb{\epsilon}}_t'
    = 
    \pmb{\epsilon} 
        - 
        \sum_i A_i w_i (\pmb{f}_i (\pmb{x}_0) + \pmb{g}_i (\pmb{\epsilon}) + \pmb{n}_i)
    . 
\end{equation}

The U-Net $\pmb{\epsilon}_\theta (\cdot)$ learns to predict noise from a noisy sample, which is trained with the objective
\begin{equation}
    \mathcal{L}_{\text{DM}}
    = 
    \mathbb{E}_{\pmb{x}_0, t, \pmb{\epsilon}} 
        ||
            \epsilon_\theta (\pmb{x}_t, t) - \pmb{\epsilon}
        ||_2^2. 
\end{equation}

Thus, 
\begin{equation}
    \sum_i A_i \pmb{g}_i (\pmb{\epsilon}) \approx \pmb{\epsilon}
    . 
\end{equation}

The variance of the error 
\begin{equation}
    \begin{split}
        &\text{Var} (\Delta \hat{\pmb{\epsilon}}_t')
        \\
        &= \text{Var}
            \left(
                \pmb{\epsilon} 
                - 
                \sum_i A_i w_i (\pmb{f}_i (\pmb{x}_0) + \pmb{g}_i (\pmb{\epsilon}) + \pmb{n}_i)
            \right)
        \\
        &\approx \text{Var}
            \left(
                \sum_i 
                [
                    A_i (w_i - 1) \pmb{g}_i (\pmb{\epsilon})
                    + A_i w_i \pmb{f}_i (\pmb{x}_0)
                    + A_i w_i \pmb{n}_i
                ]
            \right)
        \\
        &= 
            \sum_i A_i^2 (w_i - 1)^2 
            \text{Var} (\pmb{g}_i (\pmb{\epsilon}) )
            + 
            \sum_i A_i^2 w_i^2 \text{Var}(\pmb{f}_i (\pmb{x}_0))
        \\
        &~~~~+ 
            \sum_i A_i^2 w_i^2 \text{Var}(\pmb{n}_i)
        .
    \end{split}
    \label{eq-the_variance_of_the_error_appx}
\end{equation}

Thus, we have demonstrated Proposition 1. 

Note that, at any time step $t$, the variances $\text{Var}(\pmb{g}_i (\pmb{\epsilon}) )$, $\text{Var}(\pmb{f}_i (\pmb{x}_0))$ and $\text{Var}(\pmb{n}_i)$ are deterministic. 
To reduce $\text{Var} (\Delta \hat{\pmb{\epsilon}}_t')$, based on the \emph{rearrangement inequality}, we need to design a set of weights $\{w_i\}$ that assign higher weights to terms with smaller variances, while assign lower weights to terms with larger variances. 
Specifically: 

\begin{itemize}
    \item When $t$ is large, i.e., when the noise level is high, we should assign greater weights to blocks that can accurately distinguish the noise, namely those with smaller $\text{Var}(\pmb{g}_i)$. 

    \item When $t$ is small, i.e., when the noise level is low, we should assign greater weights to blocks that can accurately distinguish the signal, namely those with smaller $\text{Var}(\pmb{f}_i)$. 

    \item For all $t$, we should assign smaller weights to blocks with larger intrinsic noise, i.e., those with larger $\text{Var}(\pmb{n}_i)$. 
    It can also be seen as a measurement of the \emph{aleatoric uncertainty}
    \footnote{
        The aleatoric uncertainty refers to the inherent randomness or variability in the system or data. 
        It arises from stochastic processes or inherent noise in observations. 
        It cannot be reduced even with more information. 
    }
    \cite{der2009aleatory} of the block. 
\end{itemize}

By designing appropriate weights $\{w_i\}$, we can reduce $\text{Var} (\Delta \hat{\pmb{\epsilon}}_t')$, thus increasing the SNR. 
Simultaneously, we should balance the noise prediction and the signal prediction to avoid $\{w_i\}$ to misweight contributions of components, leading to degrade the denoising capability of the U-Net. 

\subsection{Relationships between Importance and Uncertainty}

On the one hand, high uncertainty often suggests high importance, as vital blocks tend to exhibit greater response variation when perturbed. 
This is because the model relies heavily on these blocks, making their outputs more sensitive to adjustments.

On the other hand, the capabilities of blocks with critical importance may be limited due to their unstable behavior. 
In other words, there exists an antagonistic relationship between importance and uncertainty. 
It necessitates additional constraints or adjustments (e.g., our proposed importance-based re-weighting schedule) for better and more stable performance. 

In summary, importance highlights the Transformer blocks within the U-Net that are most critical to the generation process, while uncertainty measures how robust or reliable their contributions are. 
Together, they offer a holistic view of the U-Net mechanisms, where importance indicates necessity, and uncertainty highlights stability, expanding the interpretability of DMs.

\subsection{Empirical Re-weighting Strategy}
\label{appx_sec-more_discussion_on_proposition_1-subsection-empirical_reweighting_strategy}

Our proposed \emph{Importance Probe} (IP) is designed to monitor the dynamic importance of the Transformer blocks throughout the denoising process. 
It can adaptively distinguish the importance of each block based on the denoising focus at each time step, which is measured by the mean squared error (MSE) between the noise predictions without explicit specification. 
The importance of each block is then quantified through the voting mechanism. 
More over, results from several runs of IP are aggregated via the voting mechanism, which helps to mitigate the impact of intrinsic noise $\pmb{n}_i$ on the importance ranking. 

By applying an importance-based re-weighting schedule, we can assign greater weights to the blocks that play a dominant role at each step, thereby increasing the SNR. Specifically: 

\begin{itemize}
    \item It is more likely to assign greater weights to bottleneck blocks, as they encode high-level features, and serve as the nexus between the encoder and decoder.
    
    \item In the early denoising, it is more likely to assign greater weights to mid-low-resolution blocks, emphasizing terms with smaller $\text{Var} (\pmb{f}_i)$. 

    \item In the later denoising, it is more likely to assign greater weights to high-resolution blocks, emphasizing terms with smaller $\text{Var} (\pmb{g}_i)$. 

    \item Throughout denoising, it is more likely to assign smaller weights to blocks with larger intrinsic noise, suppressing terms with larger $\text{Var} (\pmb{n}_i)$.
\end{itemize}

% Empirical Results and Theoretical Consistency
\section{Theory-Experiment Consistency Analysis}
\label{appx_sec-theory_experiment_consistency_analysis}

Empirically,~\cite{pnpDiffusion2022} has observed that: 

\begin{itemize}
    \item The high-resolution blocks within the U-Net primarily capture high-frequency (HF) information, such as details, edges and textures. 
    In our context, these blocks are dominated by $\pmb{g}_i$. 

    \item The low-resolution blocks within the U-Net capture low/mid-frequency (LF) information, such as layout and semantics. 
    In our context, these blocks are dominated by $\pmb{f}_i$. 
\end{itemize}

Experimental results in~\cite{yang2022diffusionprobabilisticmodelslim, cao2023masactrl, zhou2024generating, zhou2025attentiondistillationunifiedapproach} have also shown that: 
\begin{itemize}
    \item At early time steps, Diffusion models (DMs) primarily reconstruct low-frequency components. 
    \item At later time steps, DMs progressively recover high-frequency components. 
\end{itemize}
Recently,~\cite{chen2025free} theoretically proved these conclusions. 

Based on the above observations, we provide further discussion on our experimental results, demonstrating the consistency between the experimental phenomena and theoretical analysis. 

\subsection{Misweighting Contributions}

We evaluate static weighting schedules, where each block is assigned a weight of 1.1 respectively, in Tab.~\ref{tab-comparison_between_different_models_and_steps_appx}. 

Static weighting schedules cannot leverage the dynamic role evolution of the Transformer blocks throughout the denosing process. 
To ensure SNR improvement, ideally, one should design an oracle and time-universal set of weights $\{w_i\}$, that correctly re-weight $\text{Var} (\pmb{f}_i)$, $\text{Var} (\pmb{g}_i)$ and $\text{Var} (\pmb{n}_i)$. 
At the very least, the positive gains from re-weighting should outweigh the negative impacts. 
However, this study observes that, the importance of each block can change significantly during the inference process. 
Thus, in a static context, the aforementioned oracle $\{w_i\}$ does not always exist. 

Results in Tab.~\ref{tab-comparison_between_different_models_and_steps_appx} reveal that, applying certain weighting schedules leads to performance degradation compared to the vanilla weighting schedule. 
We speculate that, this occurs because misweighting the contributions of componenets will increase $\text{Var} (\Delta \hat{\pmb{\epsilon}}_t')$, thereby reducing the SNR. 
Fixed the number of inference steps, samples with lower SNR may not be fully denoised, resulting in lower aesthetic scores. 

Additionally, it can also be observed that, in a static context, assigning weights $w_i > 1.0$ to high-resolution blocks is more likely to improve the performance. 
Theoretically, it is because the weighted coefficient corresponding to $\text{Var}(\pmb{g}_i)$ in Eq.~\ref{eq-the_variance_of_the_error_appx} is $(w_i - 1)^2$, while the one for $\text{Var}(\pmb{f}_i)$ is $w_i^2$. 
Compared to statically re-weighting mid-low-resolution blocks (where $\pmb{f}_i$ dominates), statically re-weighting high-resolution blocks (where $\pmb{g}_i$ dominates) results in a smaller negative impact when a misweighting happens. 

\subsection{Appropriately Re-weighting Contributions}
\label{appx_section-empirical_results_and_theoretical_consistency_subsection-appropriately_reweighting_contributions}

\paragraph{Importance Ranking}
Conversely, we utilize the IP to obtain the importance of each block throughout the denoising process. 
The derived importance rankings of the prompt ``\emph{Some cut up fruit is sitting in a blender. }" are presented in Tab.~\ref{tab-importance_sdturbo_sdxlturbo_fruit_appx}. 

To more clearly illustrate the evolution of importance rankings of the blocks throughout the denoising process, we apply IP to 20-step inference SD v2.1 and SDXL using the same prompt.
Results are shown in Tab.~\ref{tab-importance_sd_sdxl_fruit_appx}. 

The importance rankings offer a preliminary glimpse into the dynamic shifts in importance. 
More precisely, the voting score and the importance scores provide a finer-grained perspective.

% 2 步 SD-Turbo/SDXL-Turbo 的重要性排名
\begin{table}[h]
    \centering
    \caption{
        (Tab.~\ref{tab-dynamic_importance_ranking_fruit} in the main paper) 
        Dynamic importance ranking of 2-step SD-Turbo/SDXL-Turbo U-Net, arranged in non-descending order. 
    }
    \begin{tabular}{c | c : c}
        \hline
        \multirow{2}{*}{\textbf{Step}} & 
        \multicolumn{2}{c}{\textbf{Importance Ranking}} \\

        ~ & SD-Turbo & SDXL-Turbo \\
        \hline

        0 & 0 1 2 4 6 5 3 & 1 2 5 3 4 \\ 
        1 & 1 0 5 4 2 6 3 & 1 2 5 4 3 \\ 

        \hline
    \end{tabular}
    \label{tab-importance_sdturbo_sdxlturbo_fruit_appx}
\end{table}

% 20 步推理 SD v2.1/SDXL 的重要性排名
\begin{table}[h]
    \centering
    \caption{
        Dynamic importance ranking of 20-step SD v2.1/SDXL U-Net, arranged in non-descending order. 
    }
    \begin{tabular}{c | c : c}
        \hline
        \multirow{2}{*}{\textbf{Step}} & 
        \multicolumn{2}{c}{\textbf{Importance Ranking}} \\

        ~ & SD v2.1 & SDXL \\
        \hline

        0 & 6 2 3 0 4 1 5 & 5 4 2 3 1 \\ 
        1 & 0 2 6 4 5 3 1 & 3 4 2 1 5 \\  
        2 & 6 5 1 0 2 4 3 & 1 5 2 3 4 \\  
        3 & 0 2 6 1 5 3 4 & 5 4 3 1 2 \\  
        4 & 0 6 5 1 3 4 2 & 4 5 1 2 3 \\  
        5 & 0 1 2 6 3 5 4 & 5 1 3 2 4 \\  
        6 & 0 5 4 3 1 6 2 & 5 1 4 3 2 \\  
        7 & 0 5 6 4 1 3 2 & 1 5 4 2 3 \\  
        8 & 0 5 6 1 2 4 3 & 5 1 4 3 2 \\  
        9 & 0 1 6 2 5 4 3 & 5 1 4 3 2 \\  
        10 & 0 6 1 5 2 4 3 & 5 1 4 3 2 \\  
        11 & 0 1 5 6 4 3 2 & 5 1 4 2 3 \\  
        12 & 0 5 4 6 1 2 3 & 5 1 3 2 4 \\  
        13 & 5 0 6 4 1 2 3 & 5 1 4 3 2 \\  
        14 & 0 5 6 4 1 2 3 & 5 1 2 4 3 \\  
        15 & 6 0 5 1 4 2 3 & 5 1 4 3 2 \\  
        16 & 0 5 6 1 2 4 3 & 5 1 4 3 2 \\  
        17 & 6 0 5 2 1 4 3 & 5 1 4 2 3 \\  
        18 & 0 5 6 1 3 4 2 & 5 1 4 2 3 \\  
        19 & 5 6 0 1 2 3 4 & 5 1 4 2 3 \\  
        
        \hline
    \end{tabular}
    \label{tab-importance_sd_sdxl_fruit_appx}
\end{table}

\paragraph{Voting Score}

The voting scores for 2-step-inference SD-Turbo and SDXL-Turbo, as well as for 20-step-inference SD v2.1 and SDXL, are listed in Tab.~\ref{tab-voting_score_sdturbo_sdxlturbo_fruit_appx} and Tab.~\ref{tab-voting_score_sd_sdxl_fruit_appx}. respectively. 
The corresponding bar charts are shown in Fig.~\ref{tab-bar_chart_voting_score-sdturbo}, Fig.~\ref{tab-bar_chart_voting_score-sdturbo}, Fig.~\ref{tab-bar_chart_voting_score-sd} and Fig.~\ref{tab-bar_chart_voting_score-sdxl}, respectively.

The bar charts more effectively illustrate the dynamic changes in the roles of the Transformer blocks throughout the denoising process. 
Overall, the importance of the blocks generally follows a trend of being higher in the middle (i.e., the bottleneck) and lower at the ends, particularly in multi-step inference (e.g., SD v2.1 and SDXL). 
Additionally, it can be observed that, the importance of structurally symmetric blocks always exhibits significant disparities. 

% 2 步 SD-Turbo/SDXL-Turbo 投票得分
\begin{table}[h]
    \centering
    \caption{
        Dynamic voting score of 2-step SD-Turbo/SDXL-Turbo U-Net, arranged in non-descending order. 
    }
    \begin{tabular}{c | c : c}
        \hline
        \multirow{2}{*}{\textbf{Step}} & 
        \multicolumn{2}{c}{\textbf{Voting Score}} \\

        ~ & SD-Turbo & SDXL-Turbo \\
        \hline

        0 & 26 37 58 87 62 78 72 & 26 39 53 59 48 \\ 
        1 & 40 39 66 84 65 53 73 & 28 40 70 45 42 \\ 

        \hline
    \end{tabular}
    \label{tab-voting_score_sdturbo_sdxlturbo_fruit_appx}
\end{table}

% 20 步 SD/SDXL 投票得分
\begin{table}[h]
    \centering
    \caption{
        Dynamic voting score of 20-step SD v2.1/SDXL U-Net, arranged in non-descending order. 
    }
    \begin{tabular}{c | c : c}
        \hline
        \multirow{2}{*}{\textbf{Step}} & 
        \multicolumn{2}{c}{\textbf{Voting Score}} \\

        ~ & SD v2.1 & SDXL \\
        \hline

        0 & 62 65 53 59 63 69 49 & 52 46 47 41 39 \\ 
        1 & 43 76 54 66 59 65 57 & 48 47 41 41 48 \\  
        2 & 57 53 63 82 70 49 46 & 40 45 47 50 43 \\  
        3 & 47 57 53 67 78 62 56 & 46 58 45 45 31 \\  
        4 & 44 58 76 63 70 55 54 & 45 51 52 36 41 \\  
        5 & 32 49 56 66 81 72 64 & 39 52 45 53 36 \\  
        6 & 32 64 72 63 62 61 66 & 40 56 49 48 32 \\  
        7 & 35 64 81 81 64 47 48 & 35 46 60 43 41 \\  
        8 & 40 57 60 86 69 54 54 & 41 54 53 42 35 \\  
        9 & 36 48 59 79 78 62 58 & 38 59 51 50 27 \\  
        10 & 41 56 61 79 72 57 54 & 37 62 53 47 26 \\  
        11 & 39 51 77 68 64 59 62 & 34 55 55 55 26 \\  
        12 & 39 63 78 86 53 42 59 & 35 54 53 59 24 \\  
        13 & 46 59 77 83 59 40 56 & 36 59 54 50 26 \\  
        14 & 39 67 75 90 56 43 50 & 41 49 57 57 21 \\  
        15 & 40 60 80 84 70 51 35 & 39 58 57 49 22 \\  
        16 & 31 64 67 84 76 40 58 & 43 66 53 45 18 \\  
        17 & 48 66 60 85 69 49 43 & 36 60 62 46 21 \\  
        18 & 42 64 79 73 74 42 46 & 33 57 58 55 22 \\  
        19 & 48 66 72 80 86 34 34 & 37 56 57 54 21 \\  
        
        \hline
    \end{tabular}
    \label{tab-voting_score_sd_sdxl_fruit_appx}
\end{table}

% 2 步 SD-Turbo 投票得分柱状图
\begin{table}[h]
    \centering
    \begin{tabular}{c c}
        \includegraphics[width=0.45\linewidth]{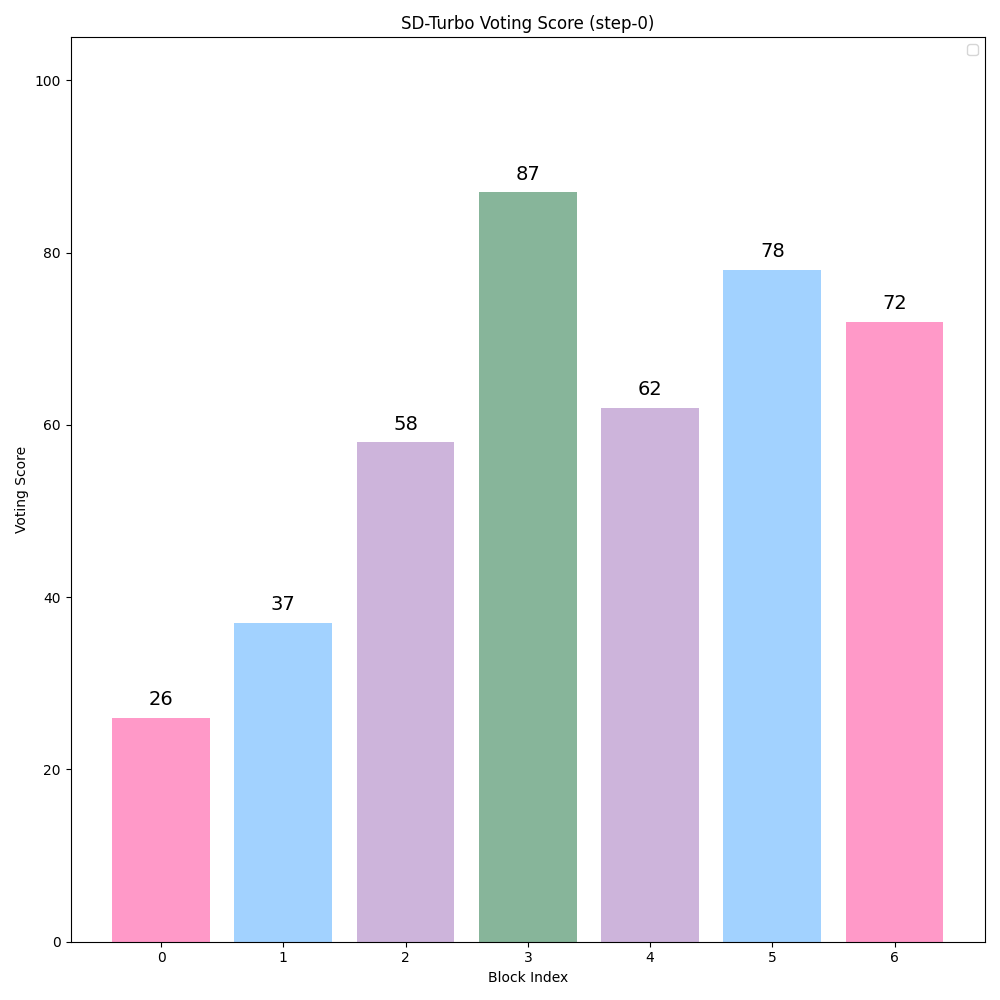} 
        & 
        \includegraphics[width=0.45\linewidth]{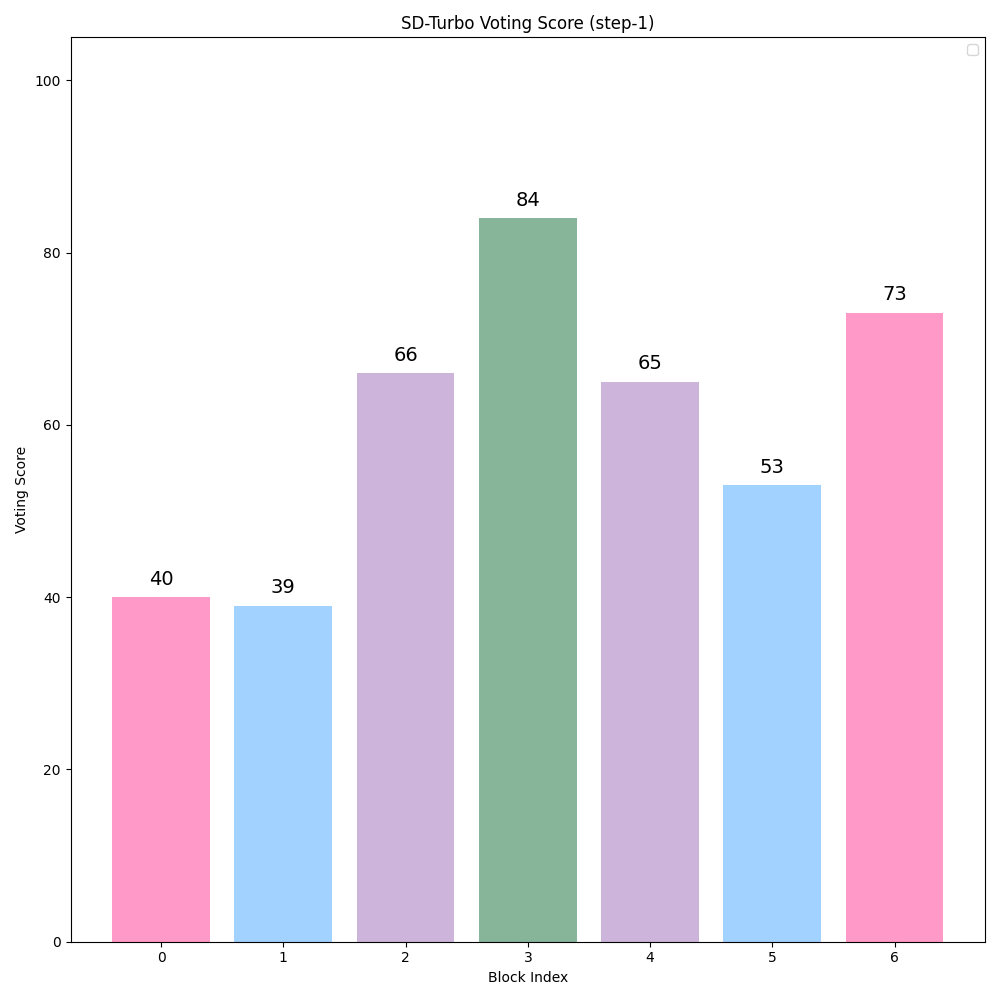}
    \end{tabular}
    \captionof{figure}{
        Bar charts of voting scores for SD-Turbo. 
    }
    \label{tab-bar_chart_voting_score-sdturbo}
\end{table}

% 2 步 SDXL-Turbo 投票得分柱状图
\begin{table}[h]
    \centering
    \begin{tabular}{c c}
        \includegraphics[width=0.45\linewidth]{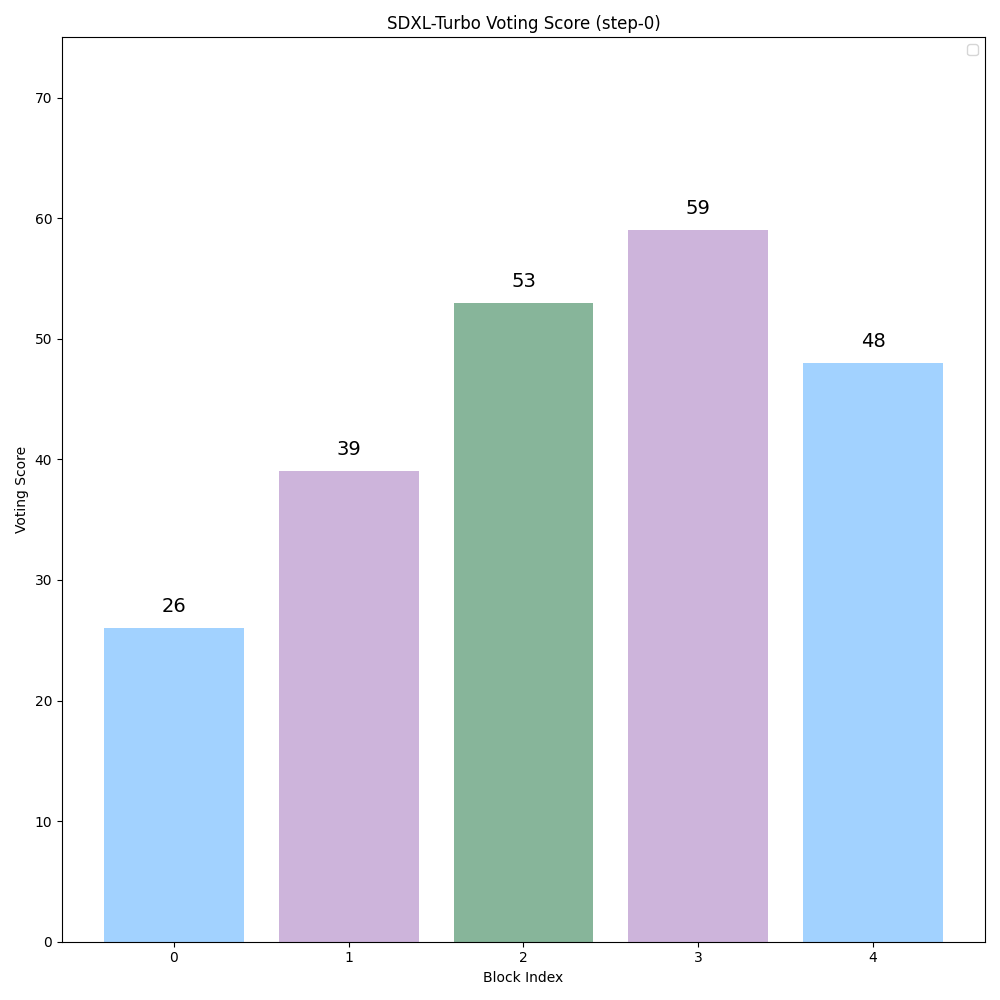} 
        & 
        \includegraphics[width=0.45\linewidth]{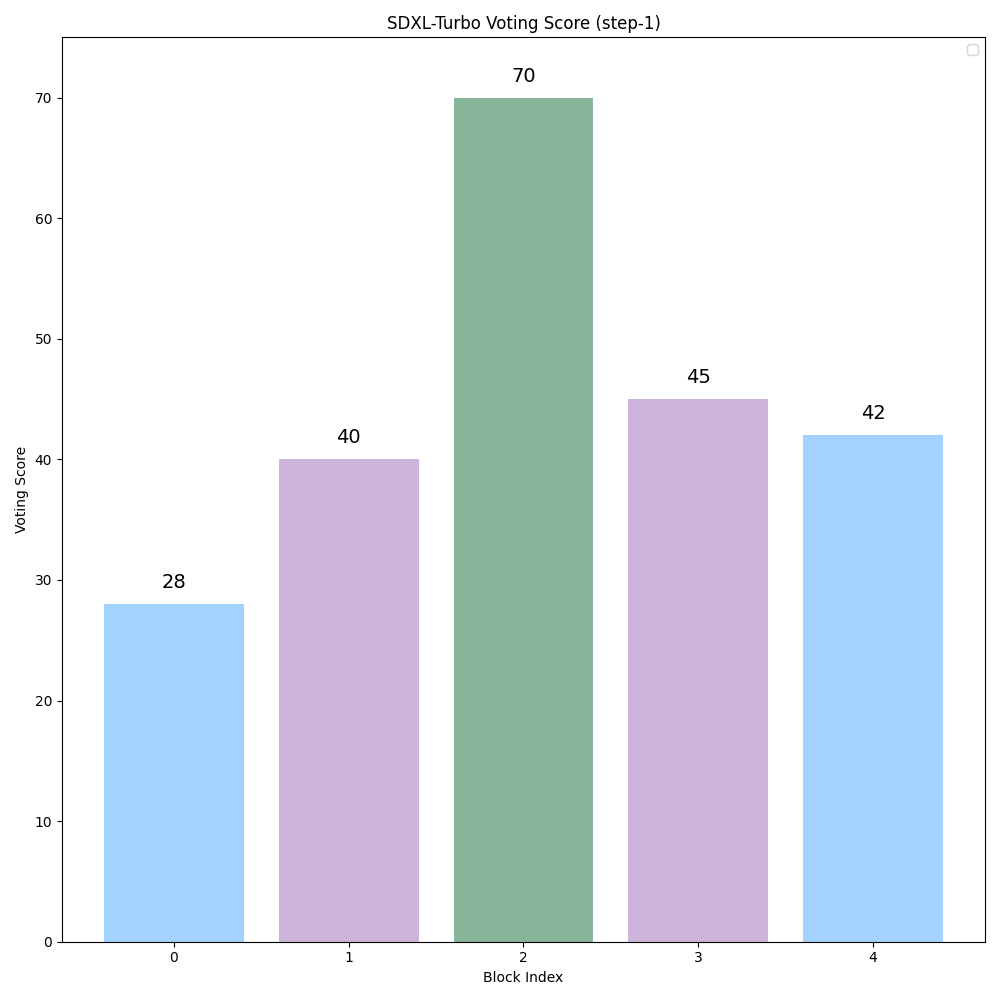}
    \end{tabular}
    \captionof{figure}{
        Bar charts of voting scores for SDXL-Turbo. 
    }
    \label{tab-bar_chart_voting_score-sdxlturbo}
\end{table}

% 20 步 SD 投票得分柱状图
\begin{table*}[h]
    \centering
    \begin{tabular}{c c c c c}
        \includegraphics[width=0.175\linewidth]{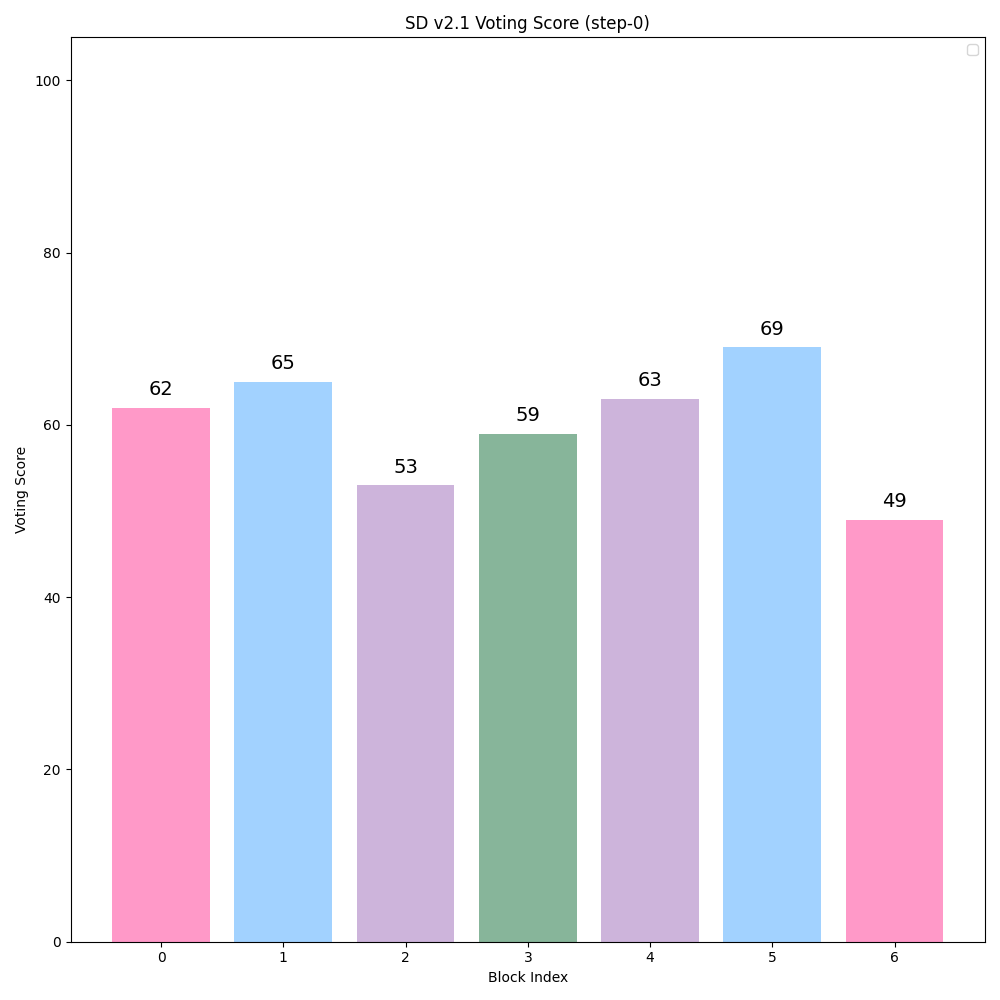} 
        & 
        \includegraphics[width=0.175\linewidth]{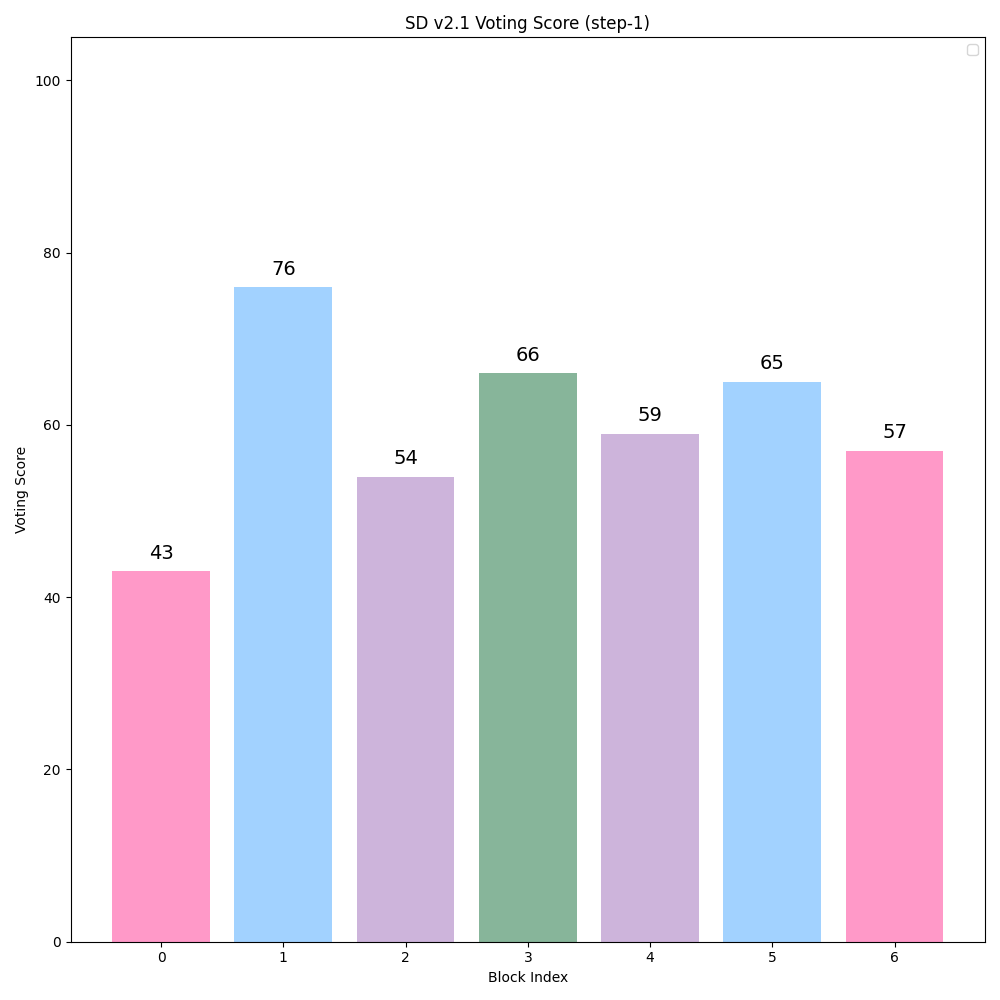}
        & 
        \includegraphics[width=0.175\linewidth]{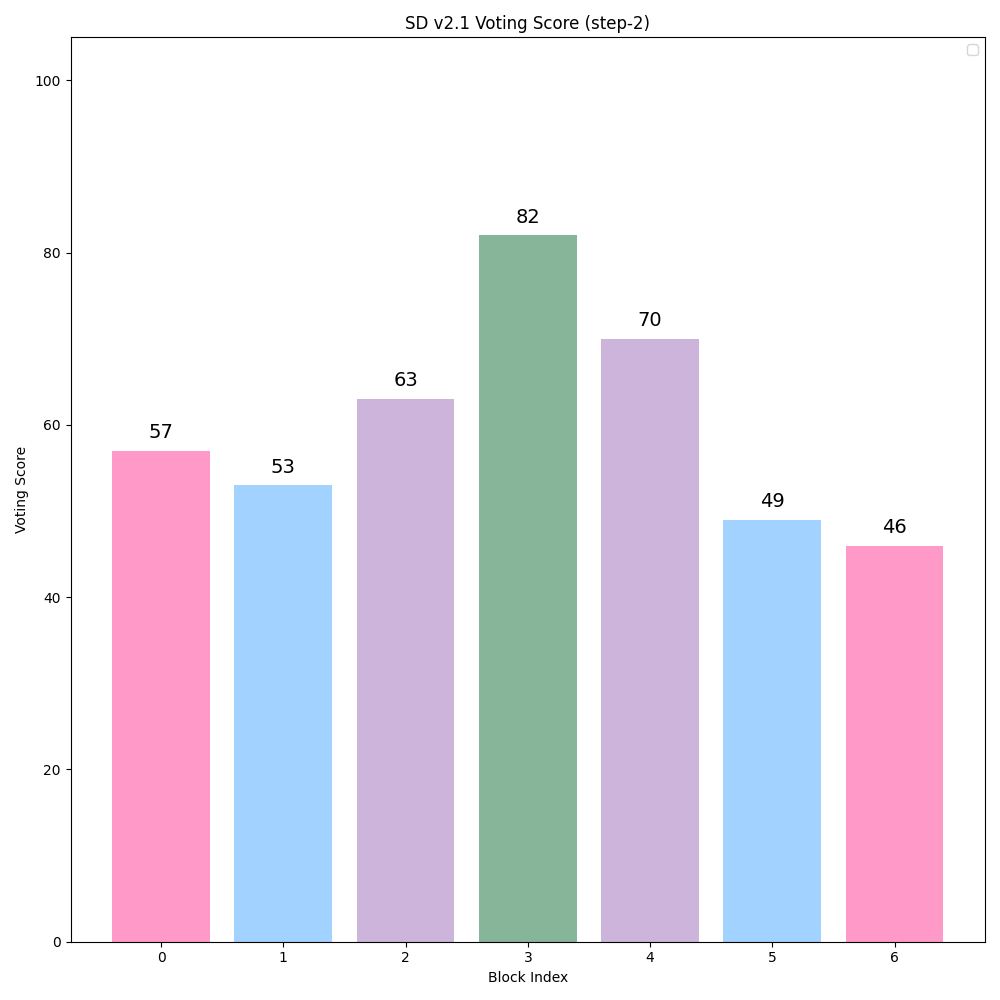}
        & 
        \includegraphics[width=0.175\linewidth]{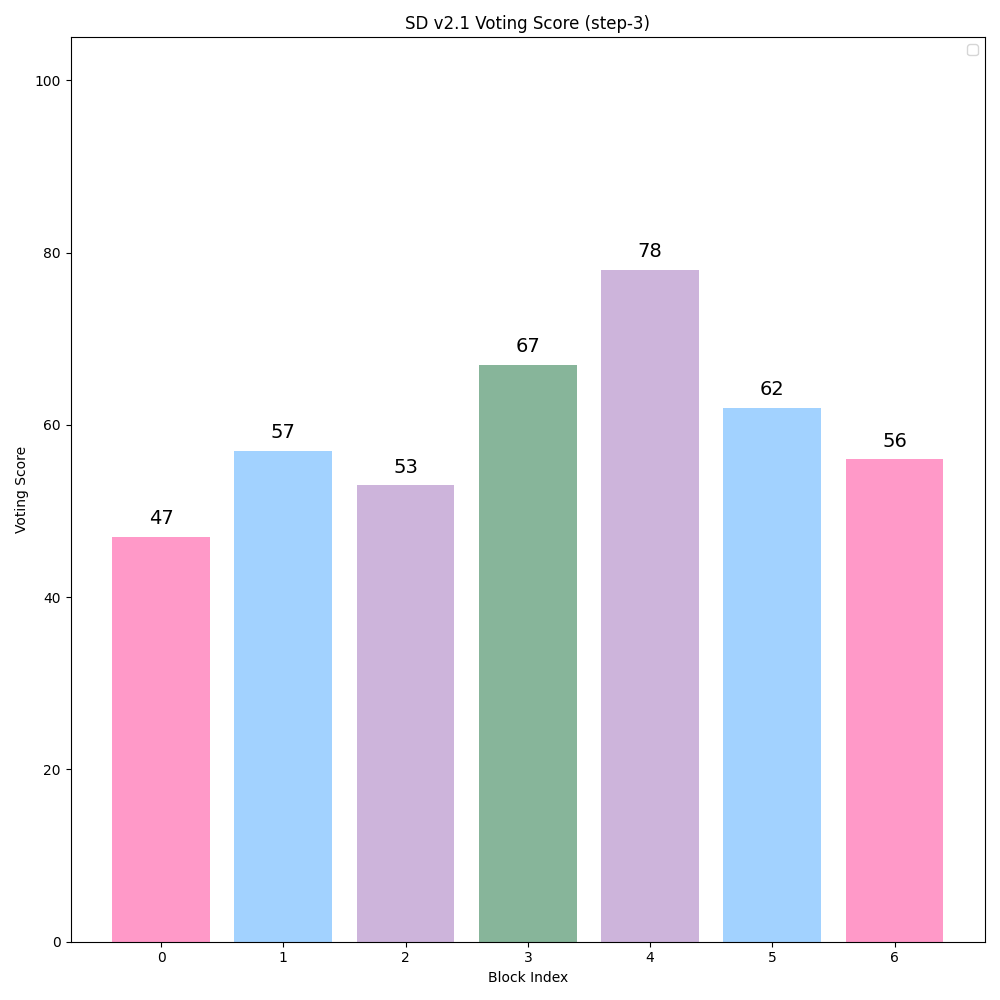}
        & 
        \includegraphics[width=0.175\linewidth]{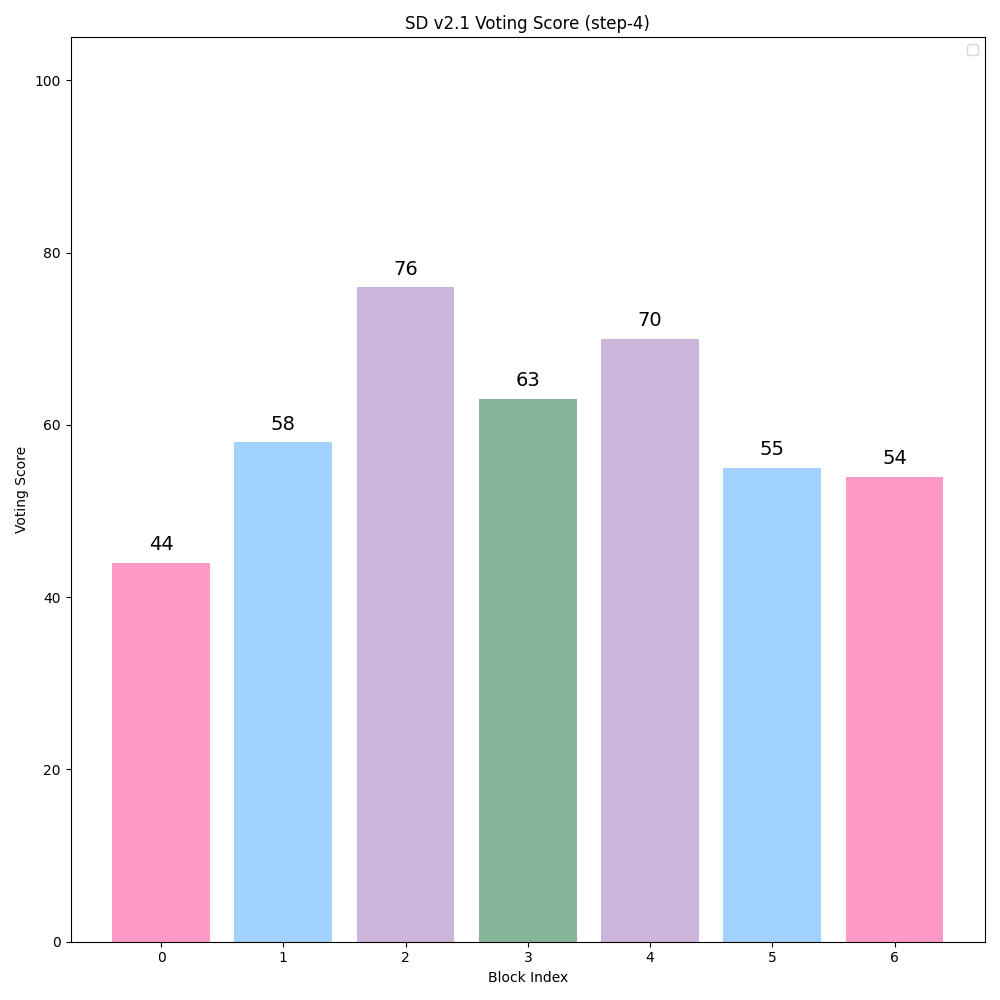}

        \\ 

        \includegraphics[width=0.175\linewidth]{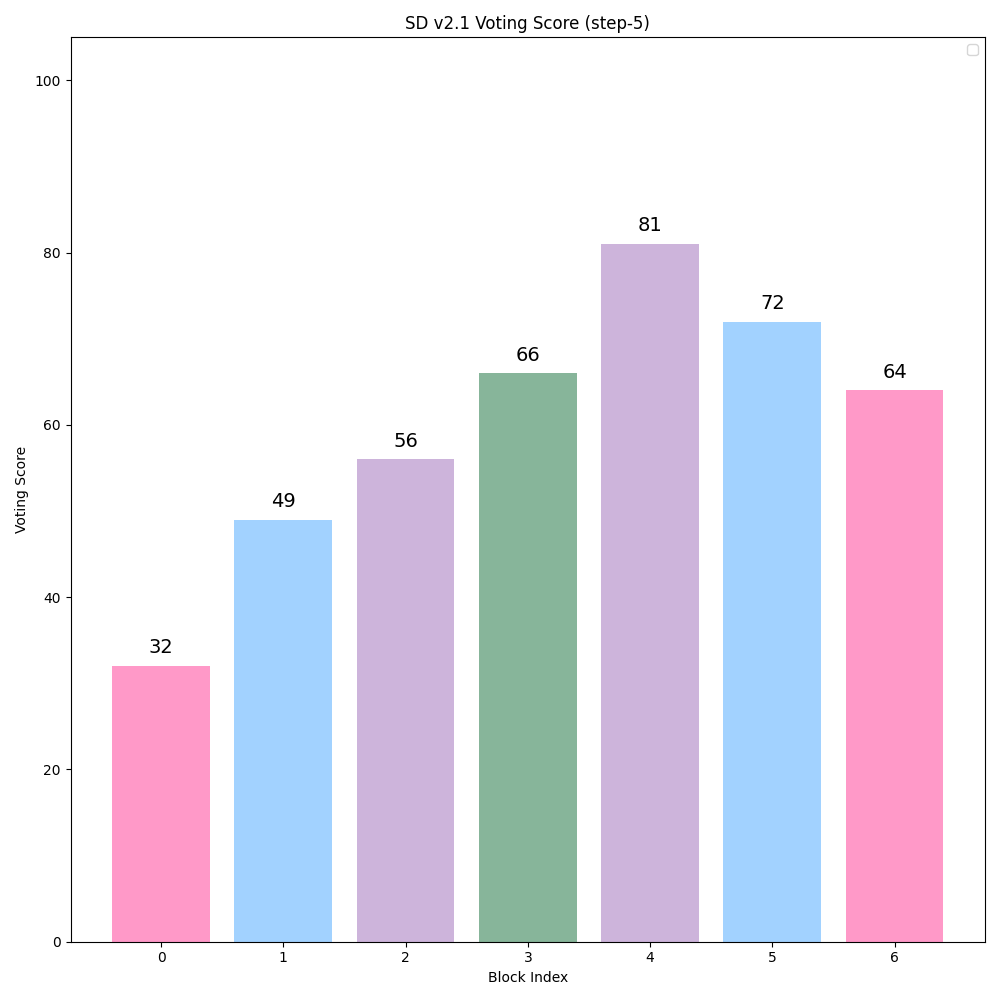} 
        & 
        \includegraphics[width=0.175\linewidth]{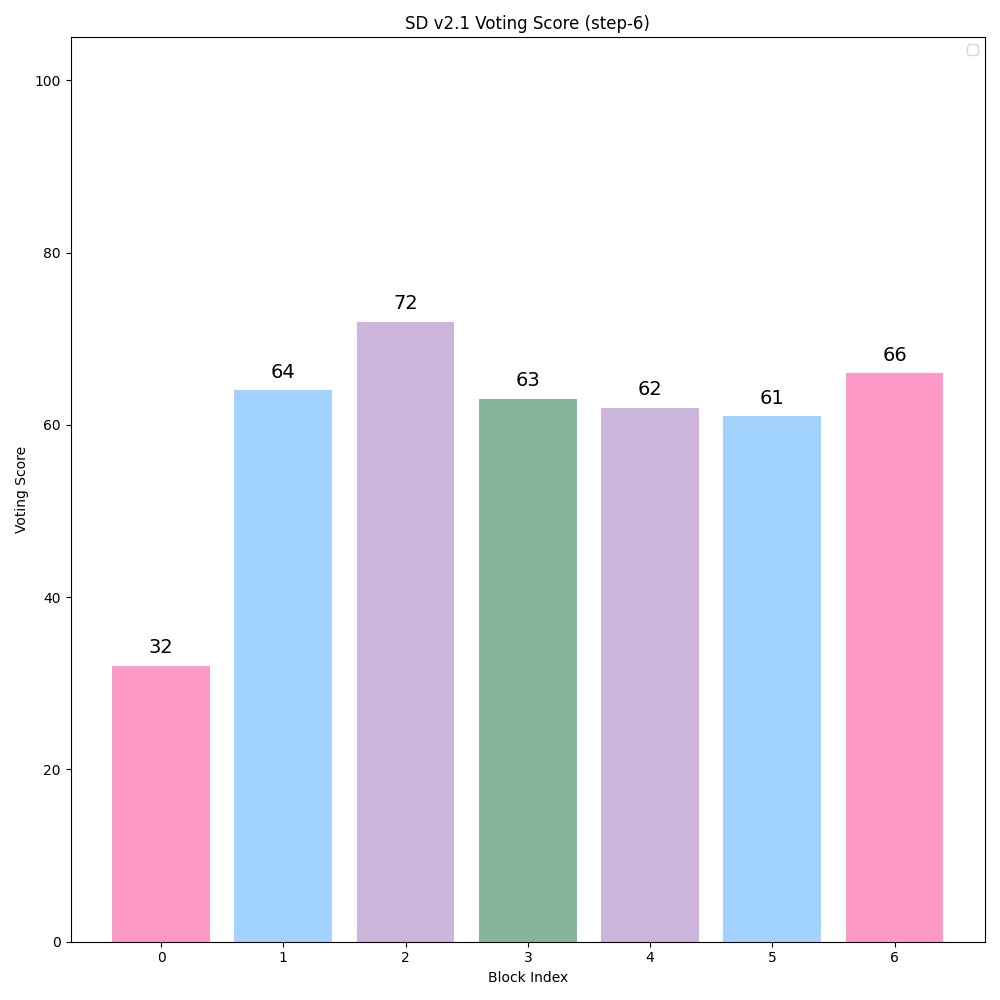}
        & 
        \includegraphics[width=0.175\linewidth]{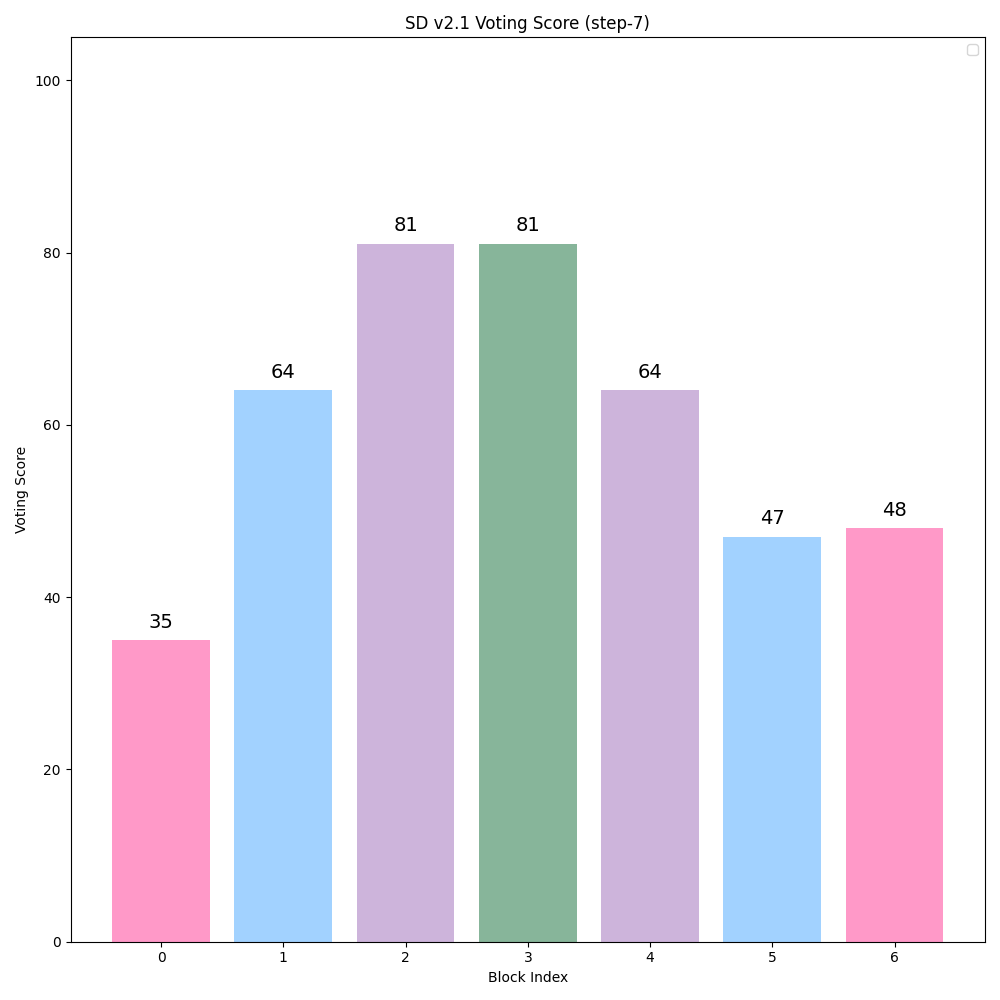}
        & 
        \includegraphics[width=0.175\linewidth]{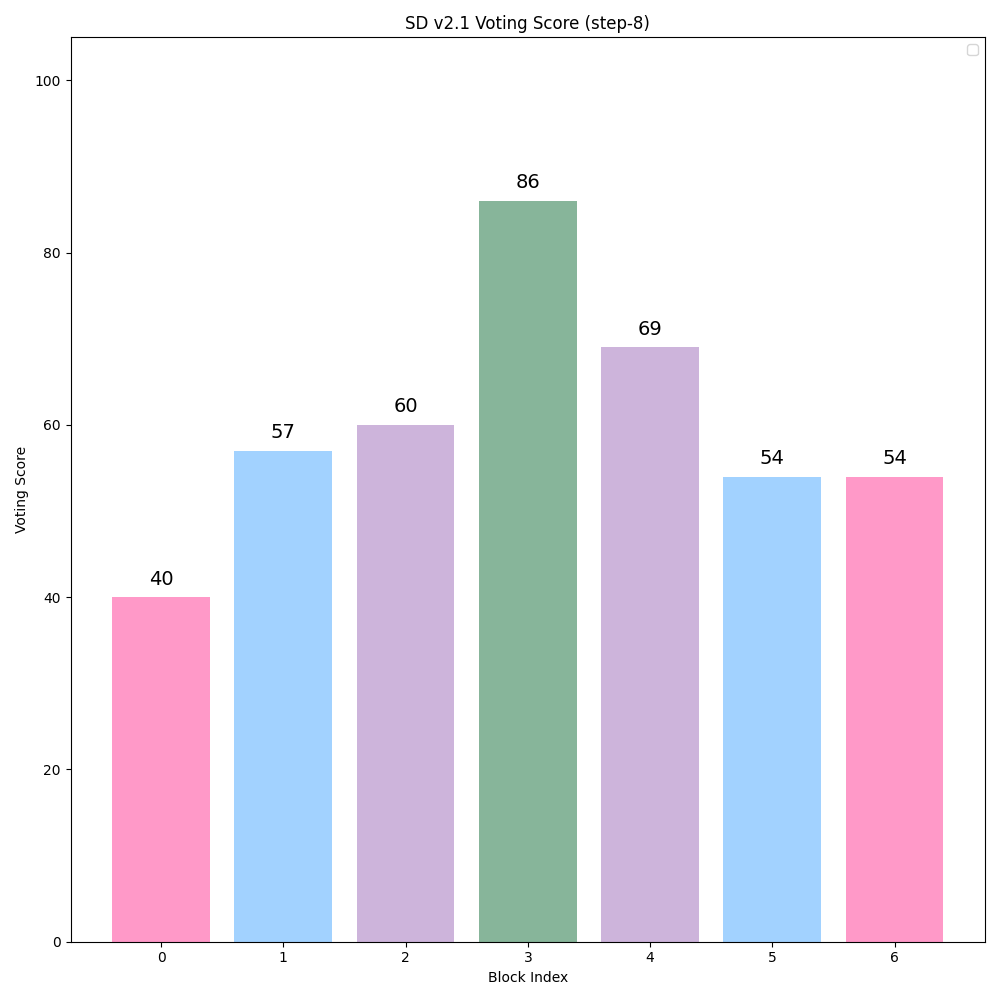}
        & 
        \includegraphics[width=0.175\linewidth]{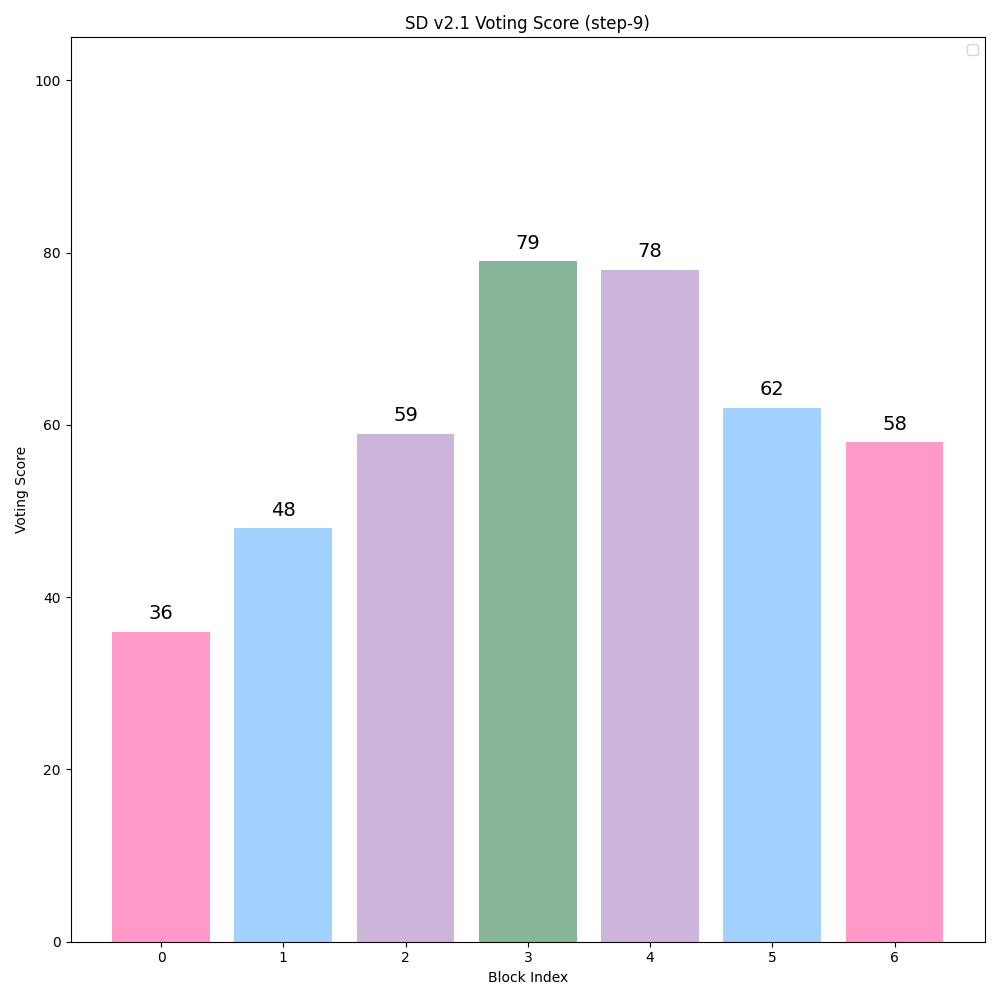}
        
        \\

        \includegraphics[width=0.175\linewidth]{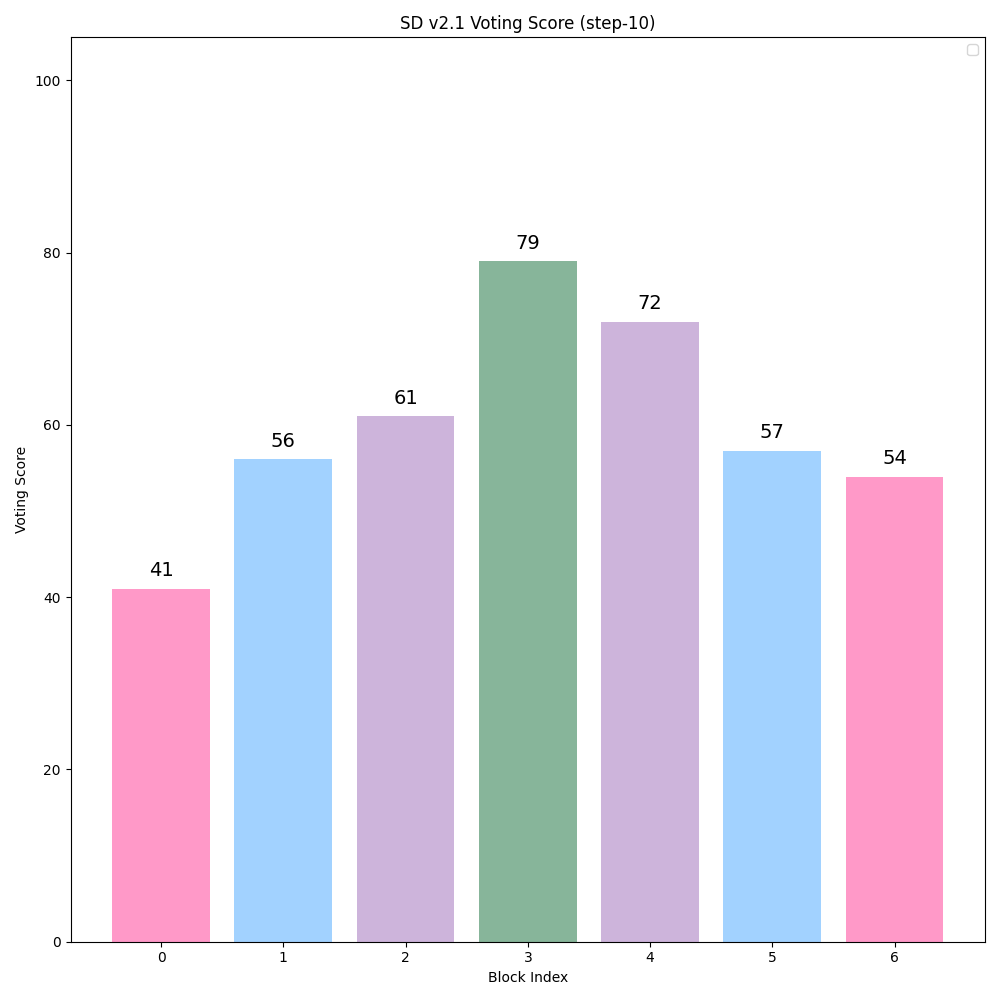} 
        & 
        \includegraphics[width=0.175\linewidth]{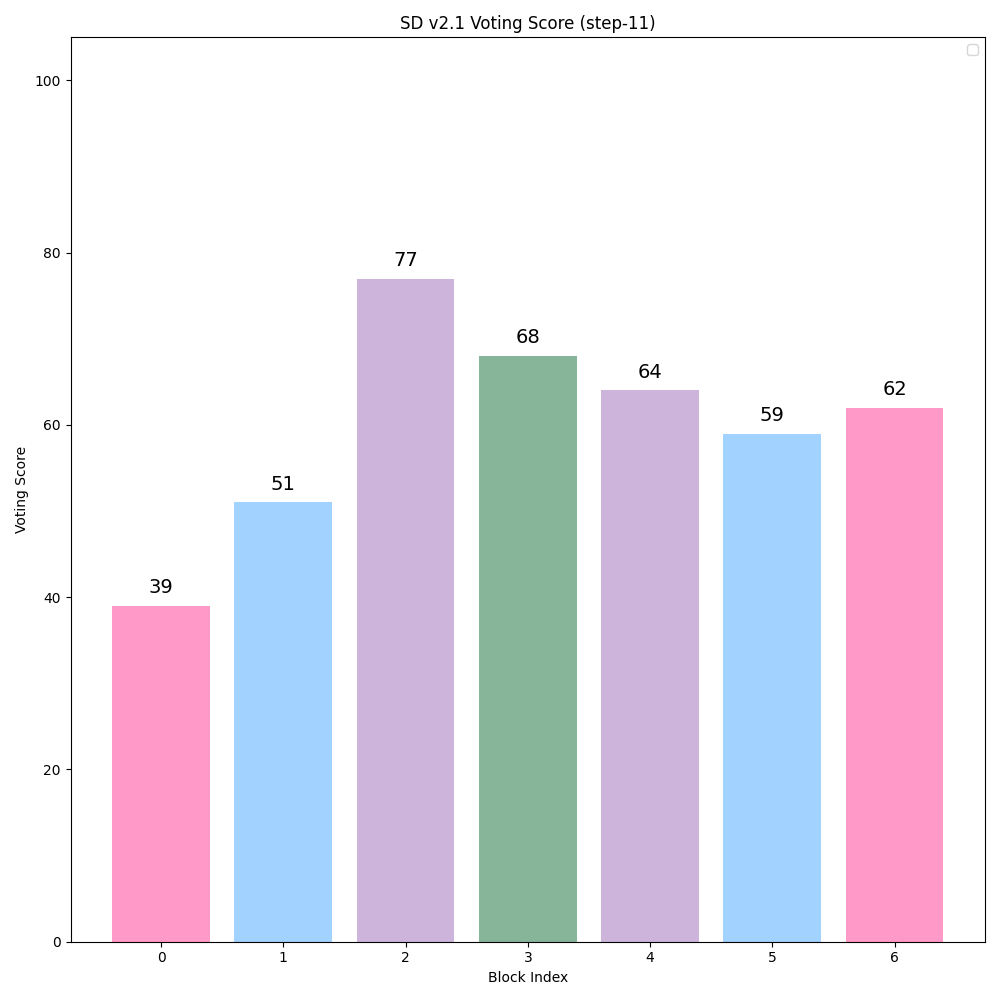}
        & 
        \includegraphics[width=0.175\linewidth]{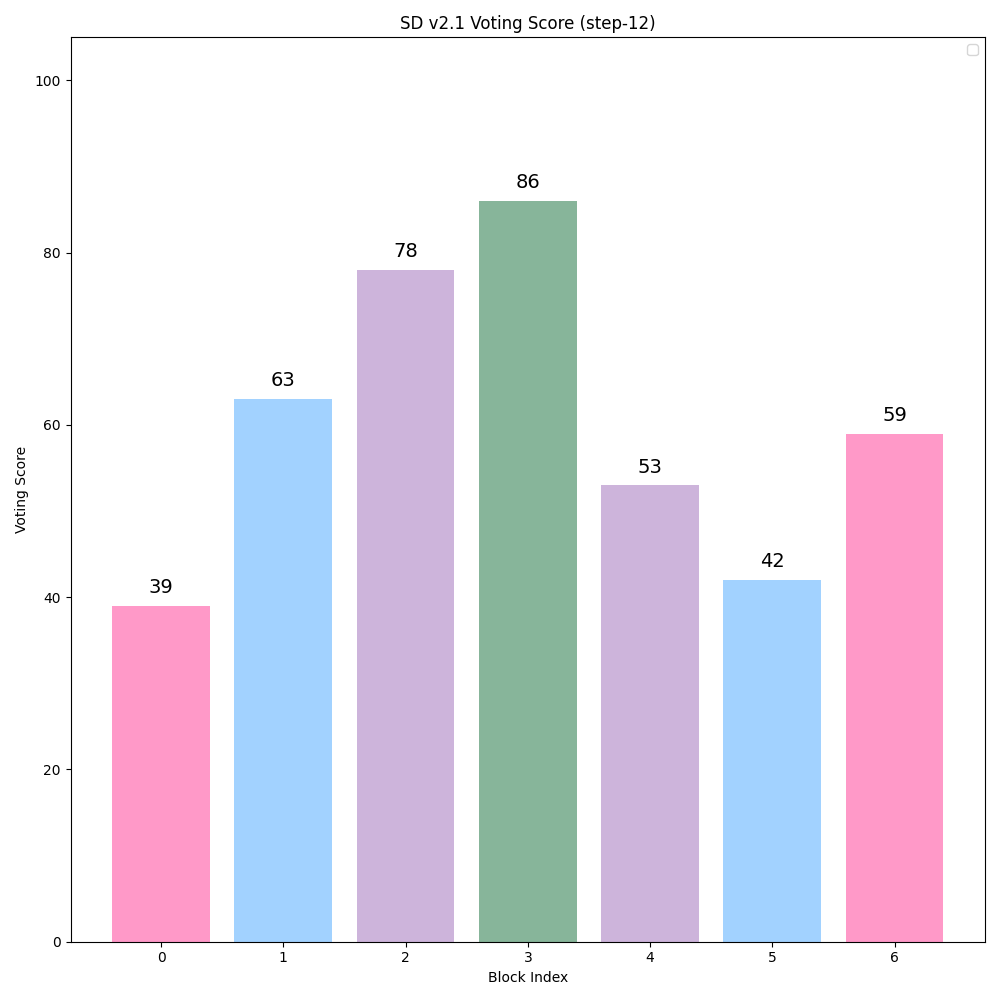}
        & 
        \includegraphics[width=0.175\linewidth]{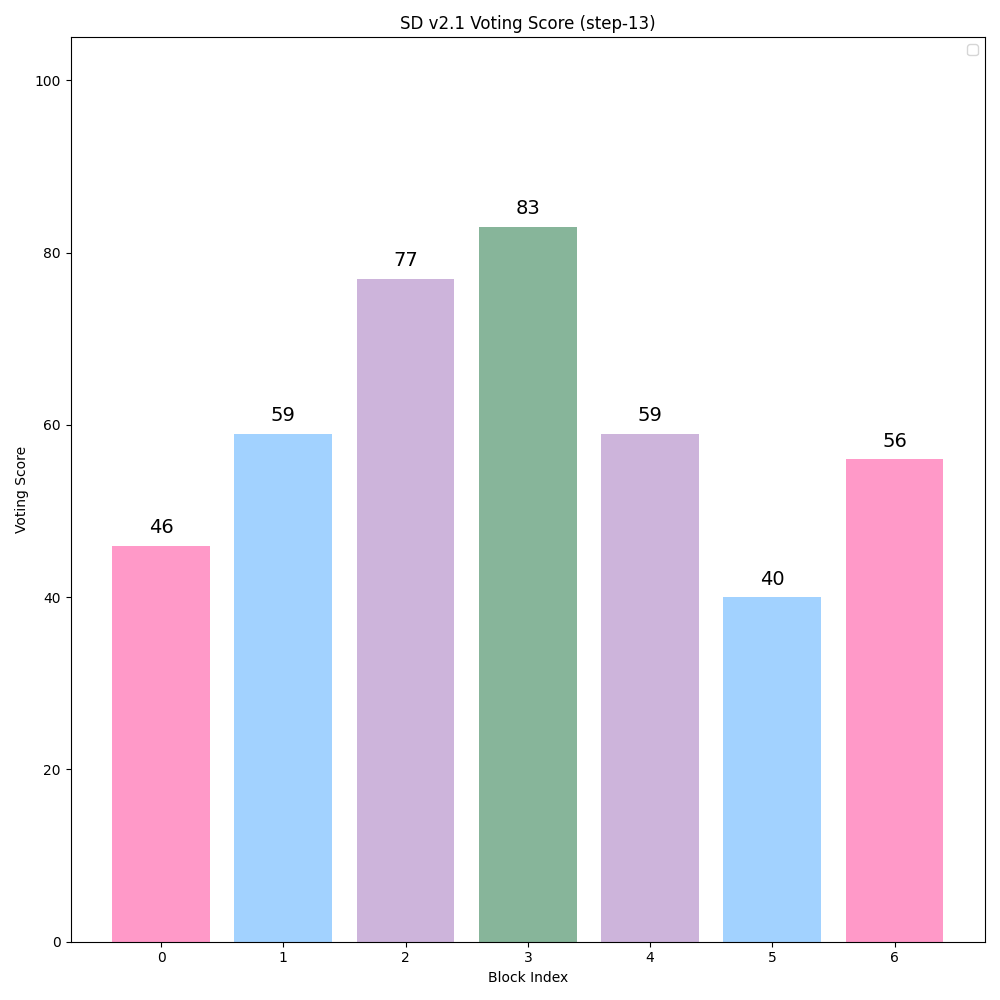}
        & 
        \includegraphics[width=0.175\linewidth]{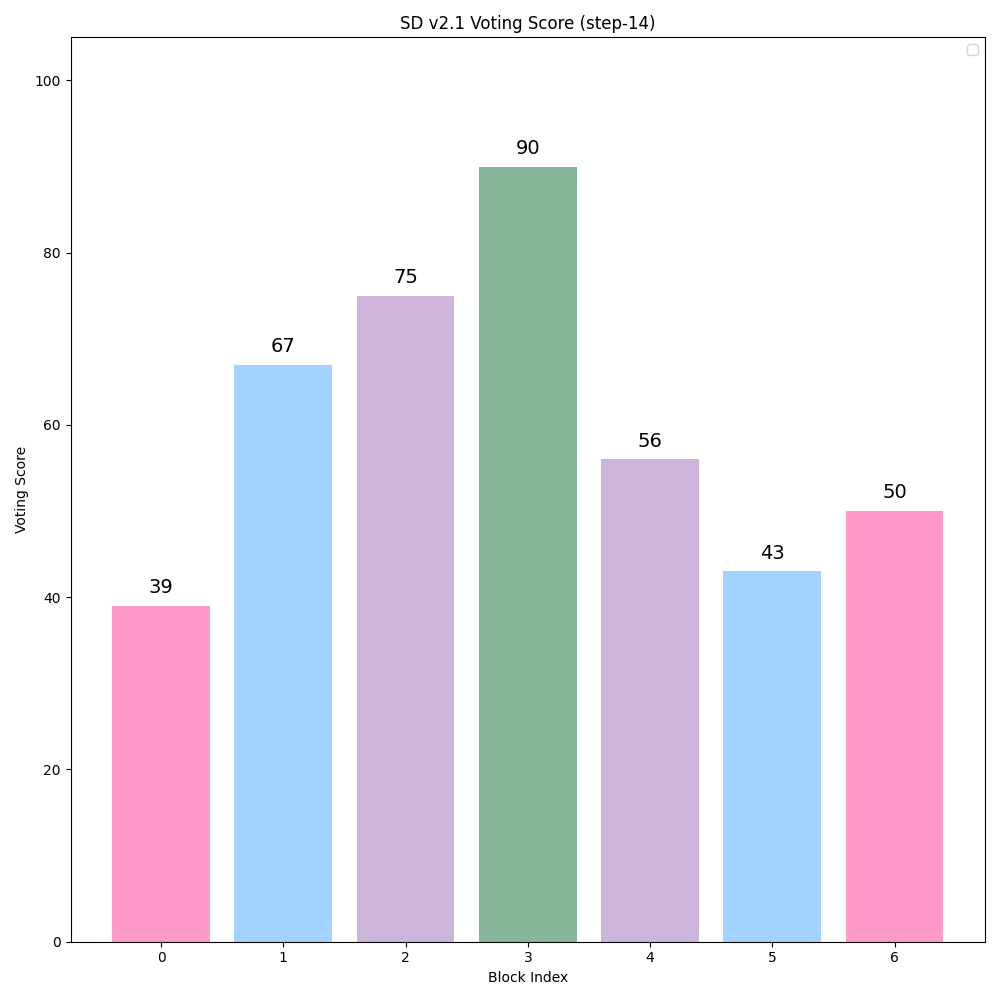}

        \\ 

        \includegraphics[width=0.175\linewidth]{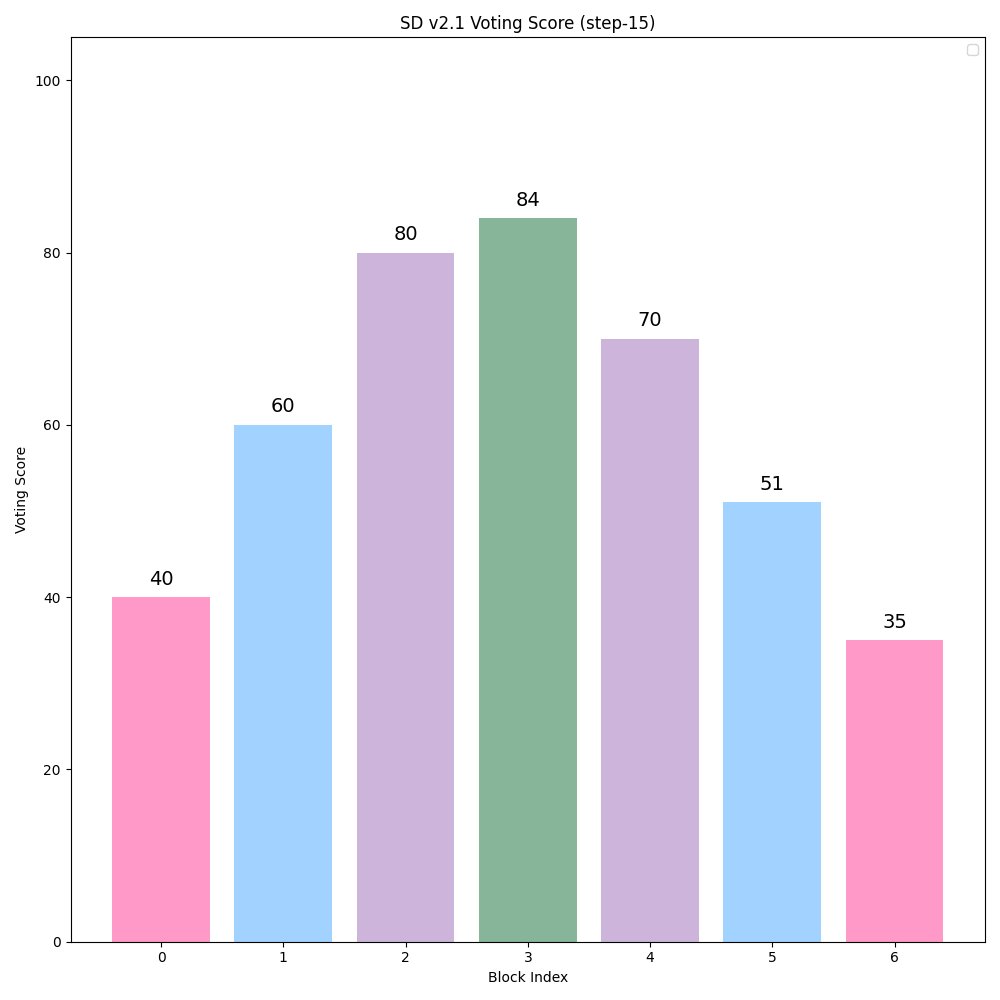} 
        & 
        \includegraphics[width=0.175\linewidth]{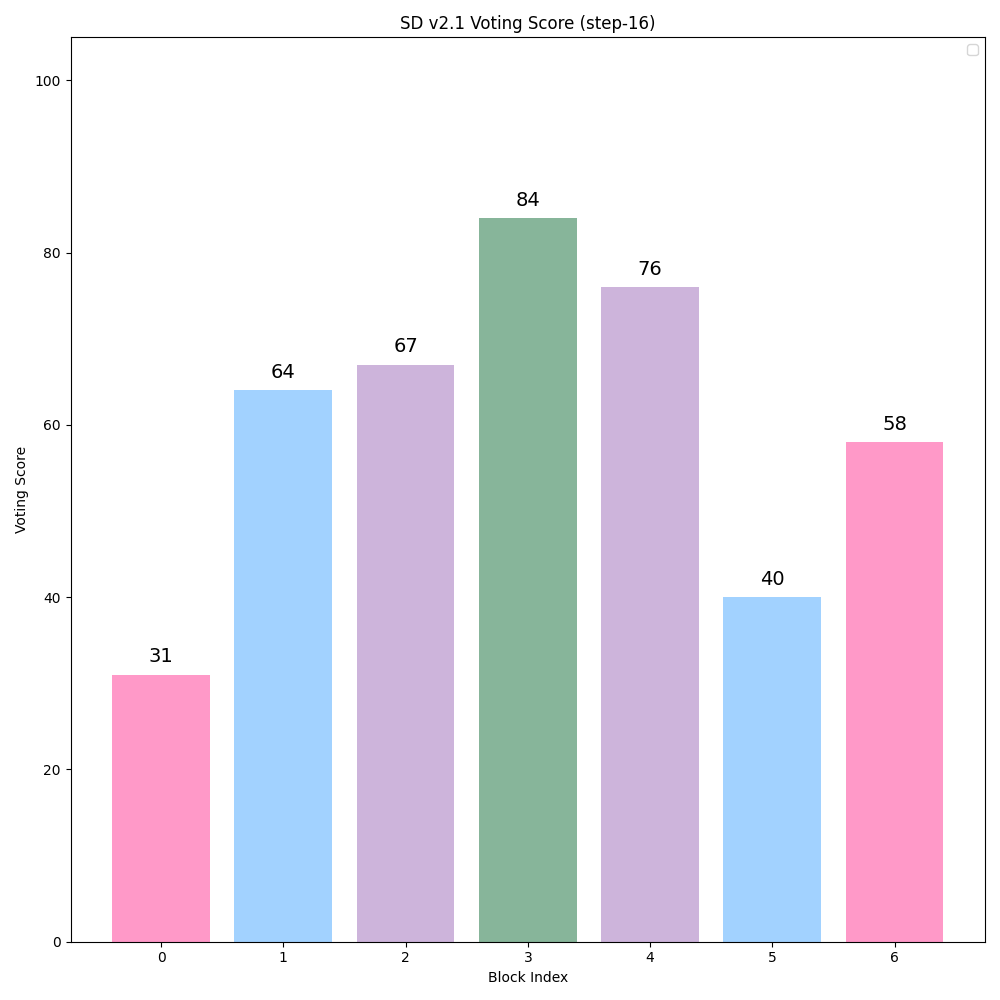}
        & 
        \includegraphics[width=0.175\linewidth]{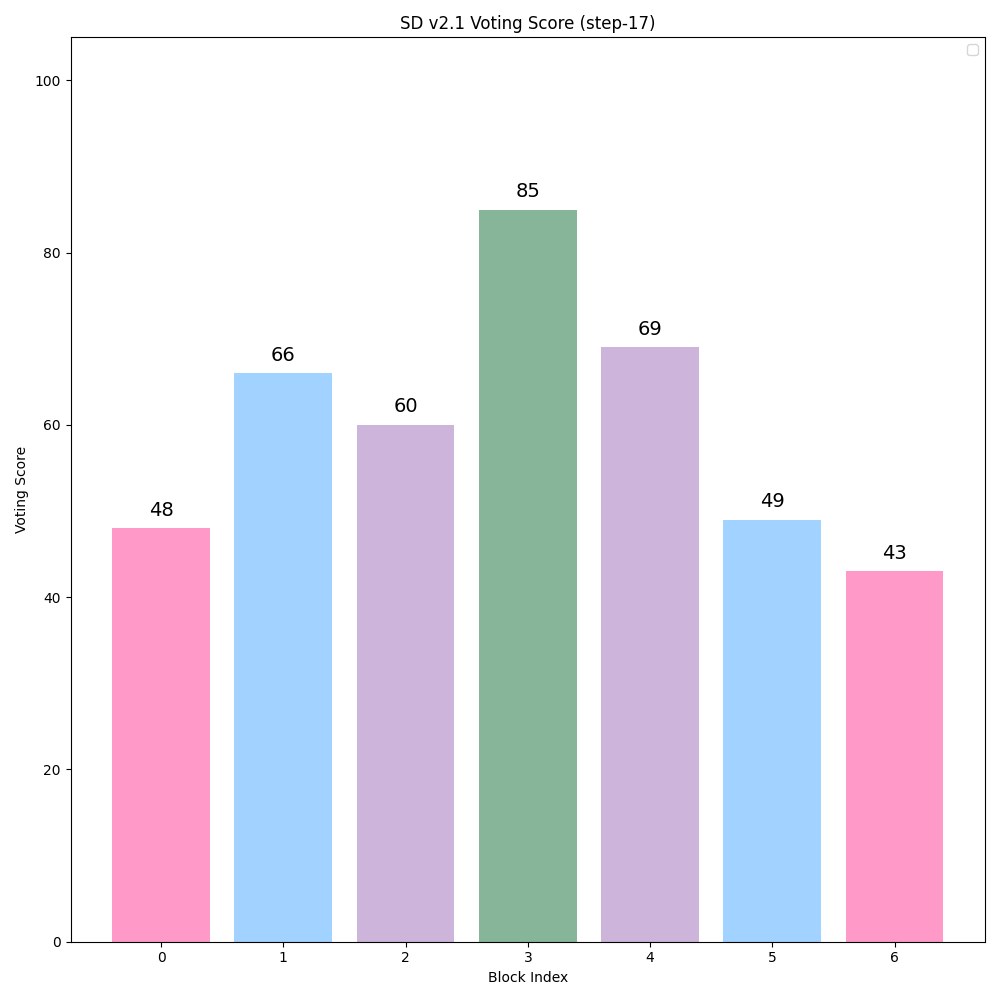}
        & 
        \includegraphics[width=0.175\linewidth]{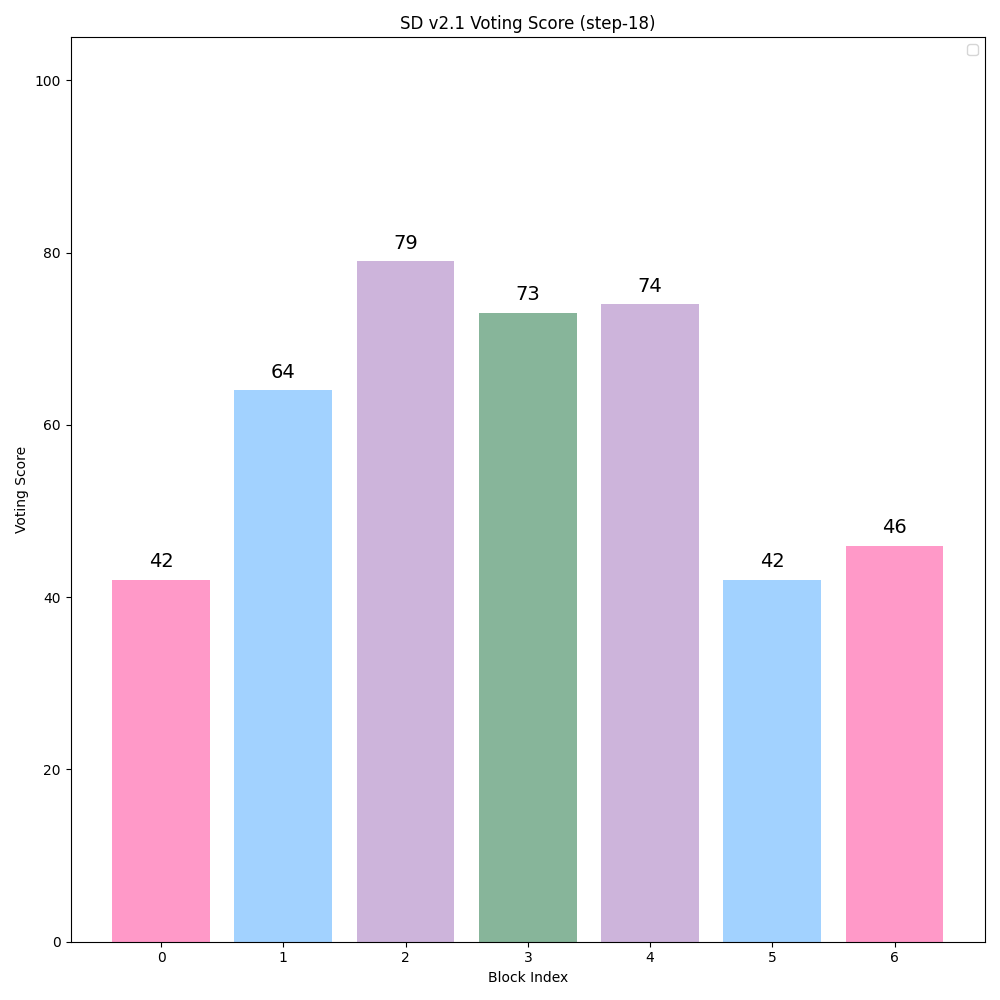}
        & 
        \includegraphics[width=0.175\linewidth]{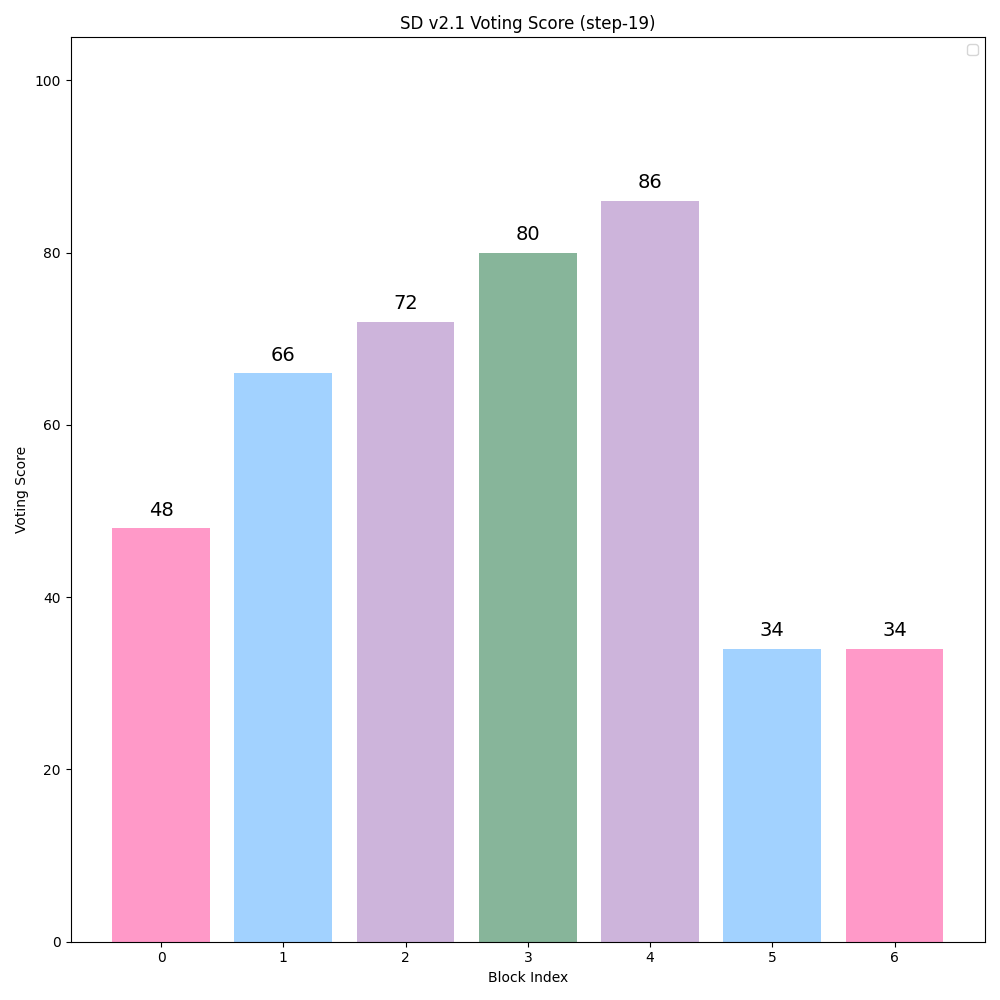}
    \end{tabular}
    \captionof{figure}{
        Bar charts of voting scores for SD v2.1. 
    }
    \label{tab-bar_chart_voting_score-sd}
\end{table*}

% 20 步 SDXL 投票得分柱状图
\begin{table*}[h]
    \centering
    \begin{tabular}{c c c c c}
        \includegraphics[width=0.175\linewidth]{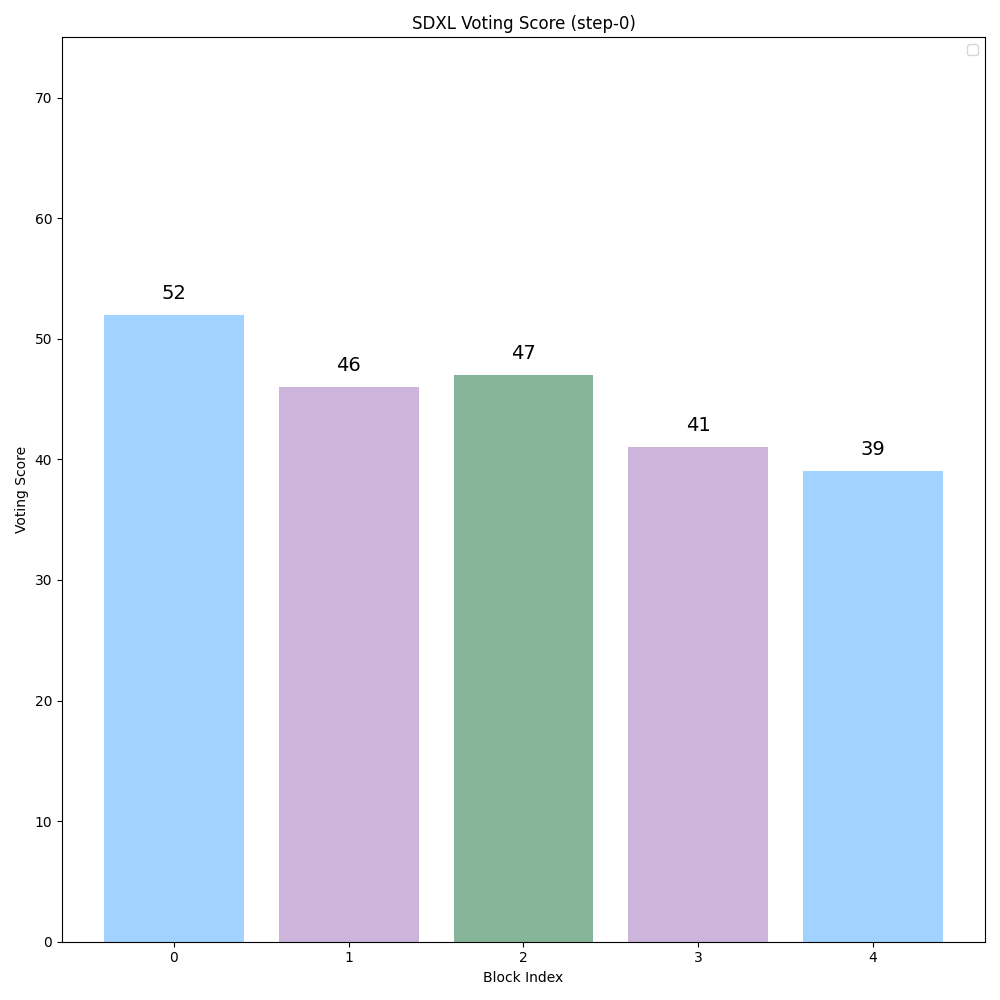} 
        & 
        \includegraphics[width=0.175\linewidth]{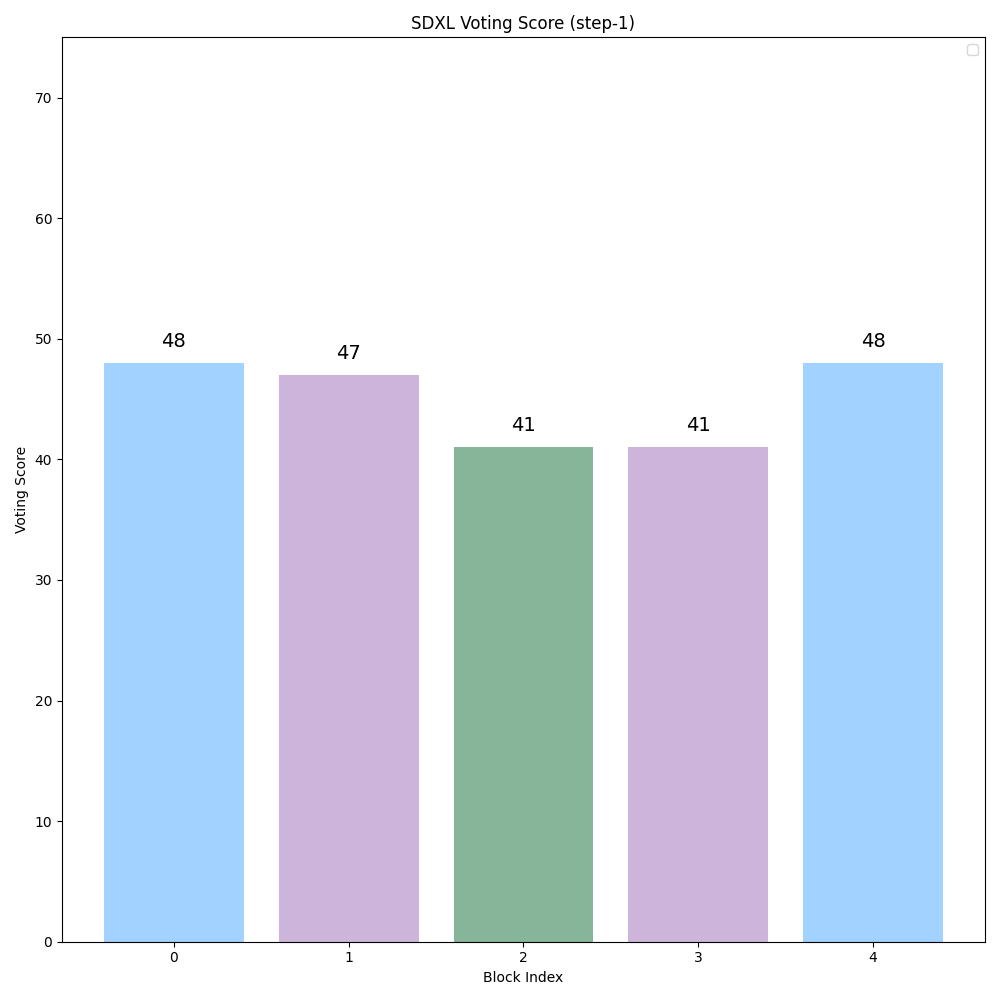}
        & 
        \includegraphics[width=0.175\linewidth]{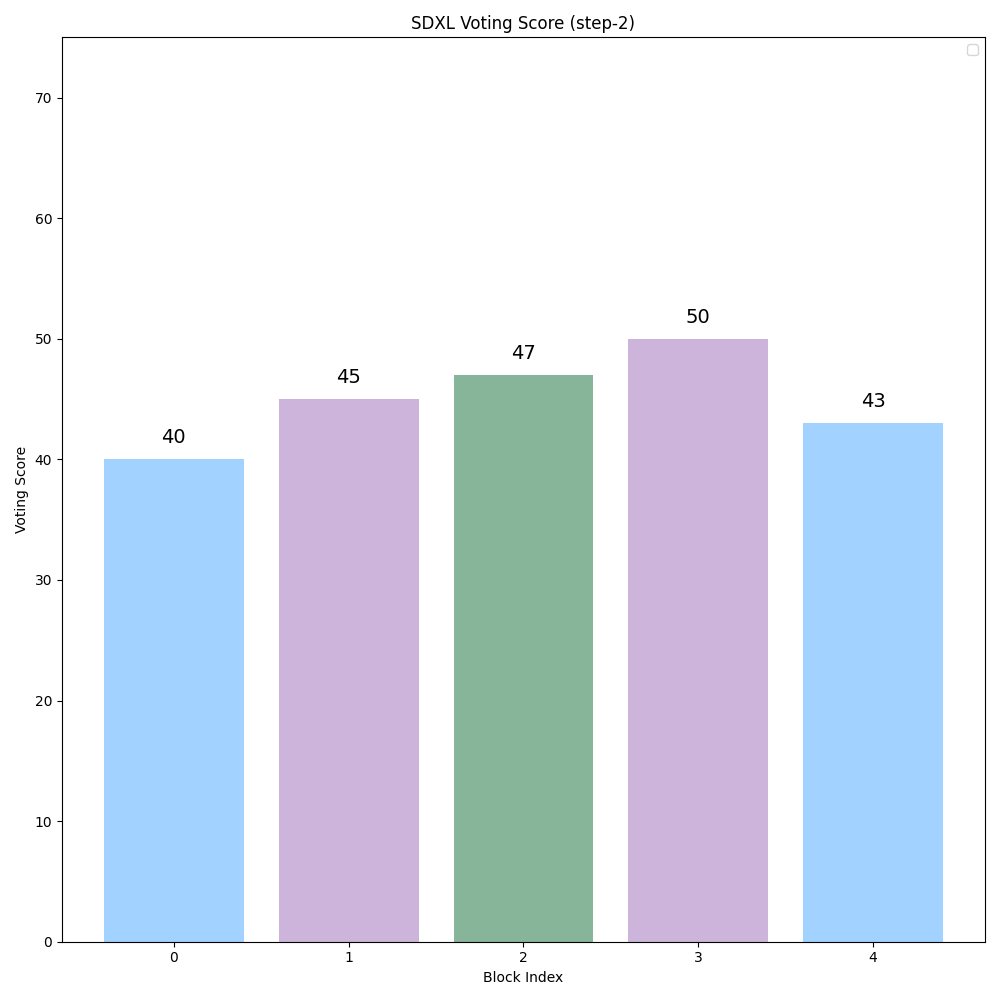}
        & 
        \includegraphics[width=0.175\linewidth]{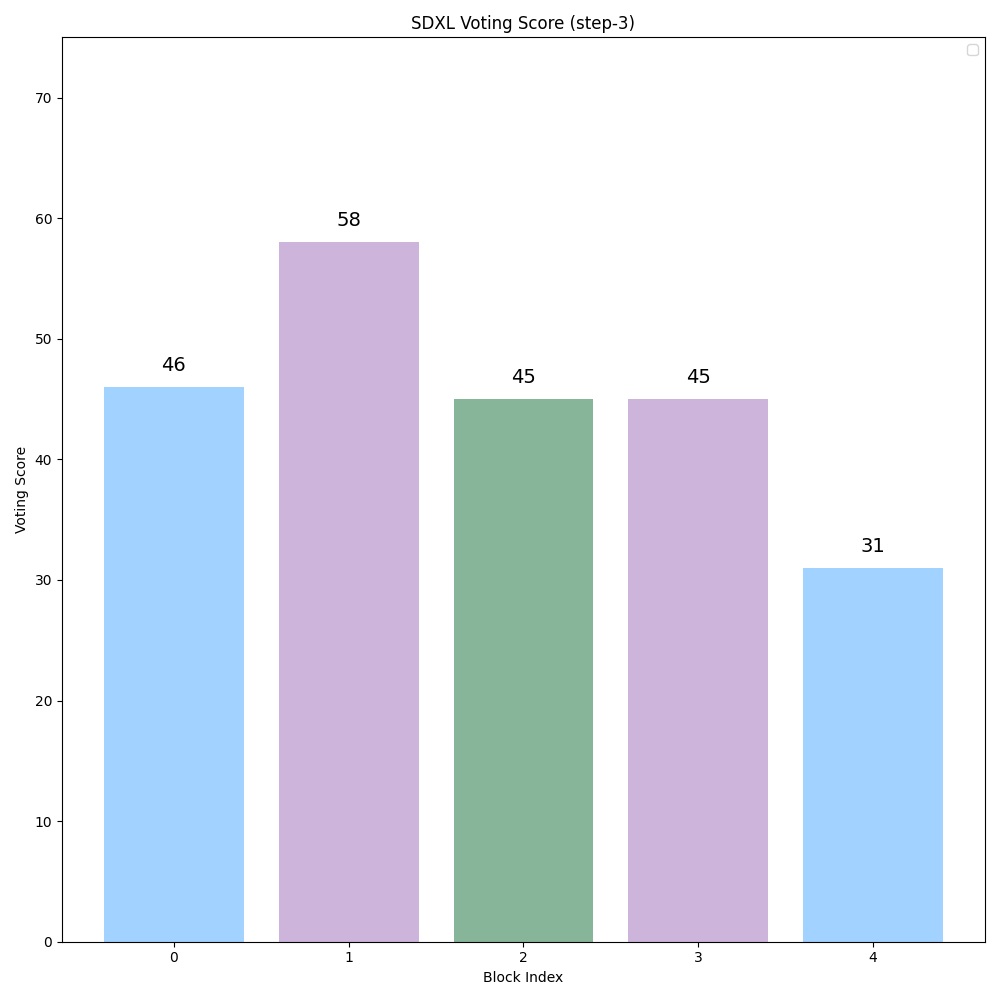}
        & 
        \includegraphics[width=0.175\linewidth]{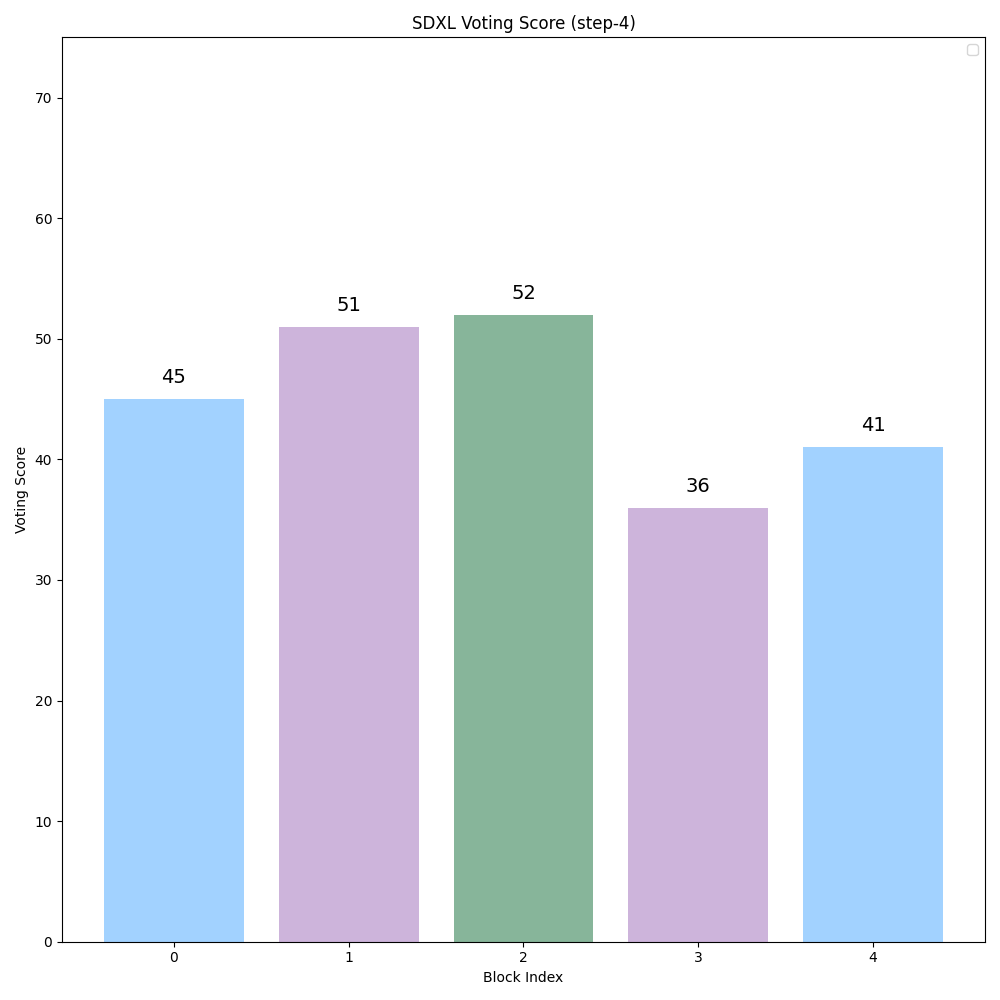}

        \\ 

        \includegraphics[width=0.175\linewidth]{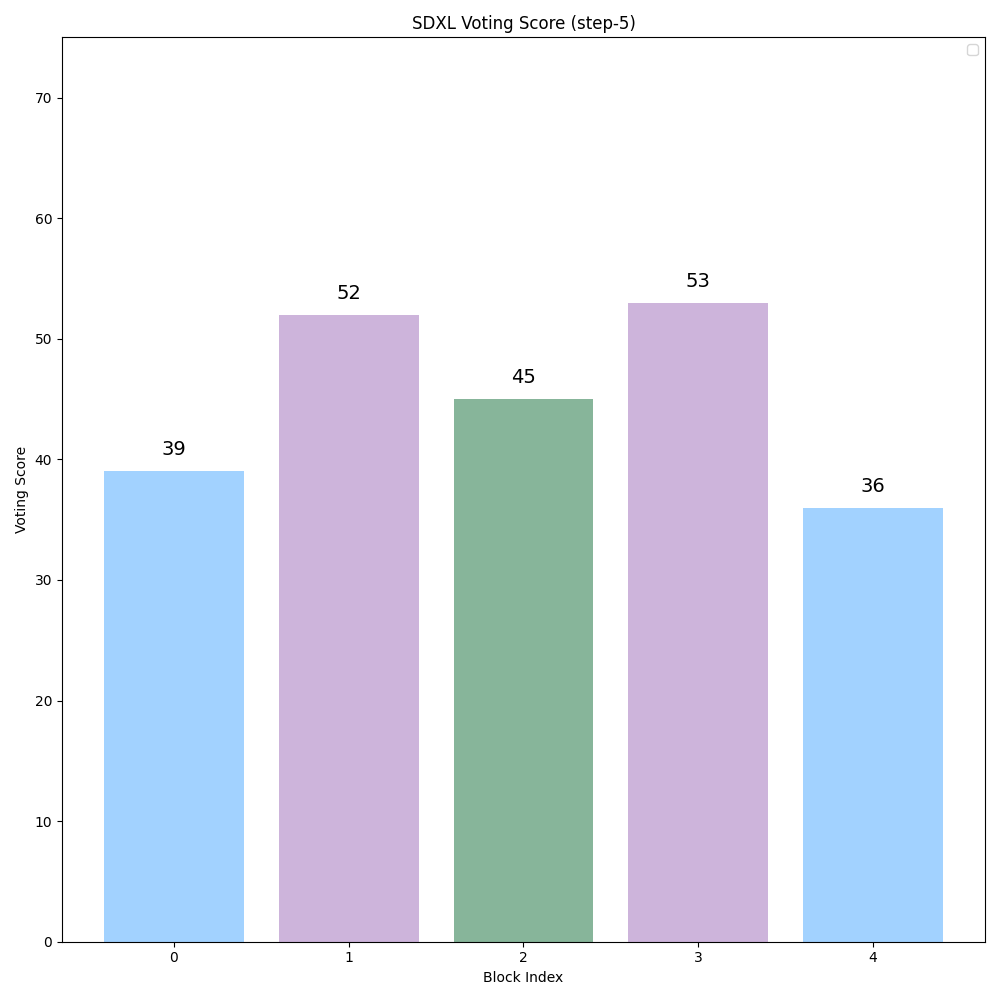} 
        & 
        \includegraphics[width=0.175\linewidth]{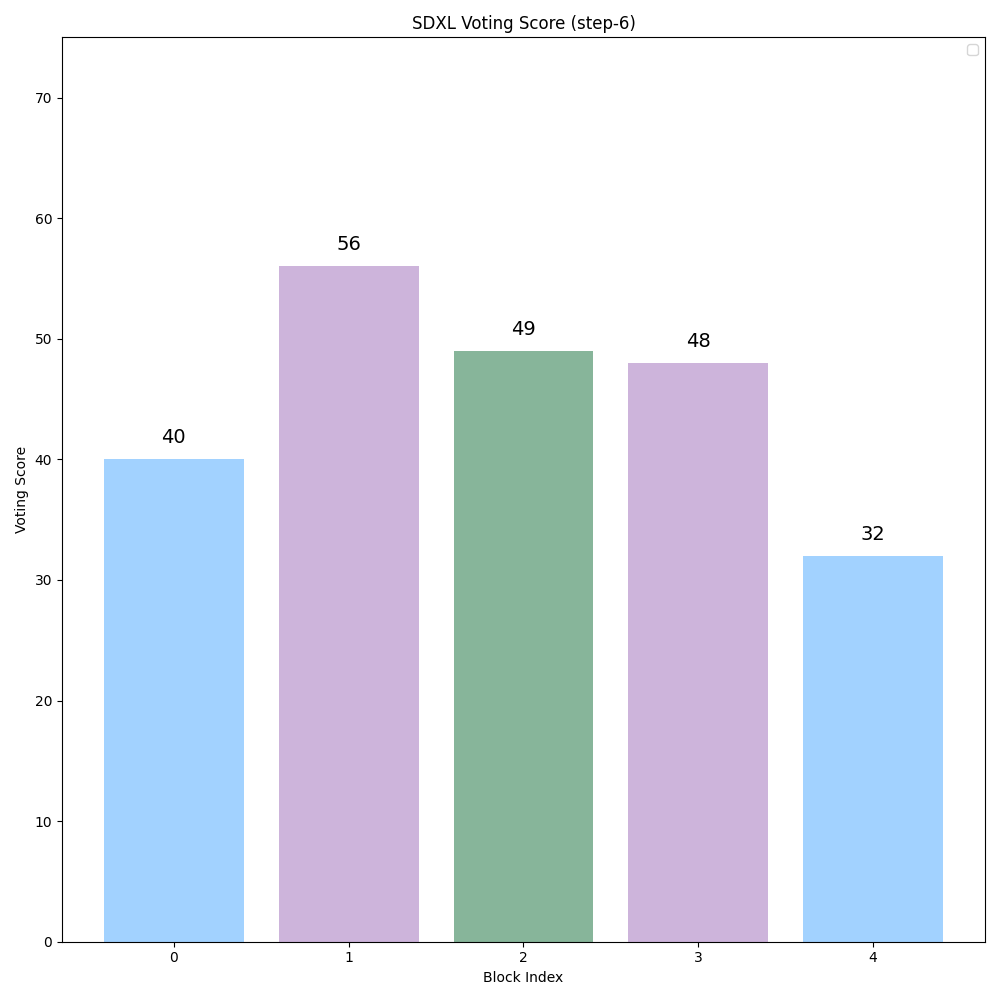}
        & 
        \includegraphics[width=0.175\linewidth]{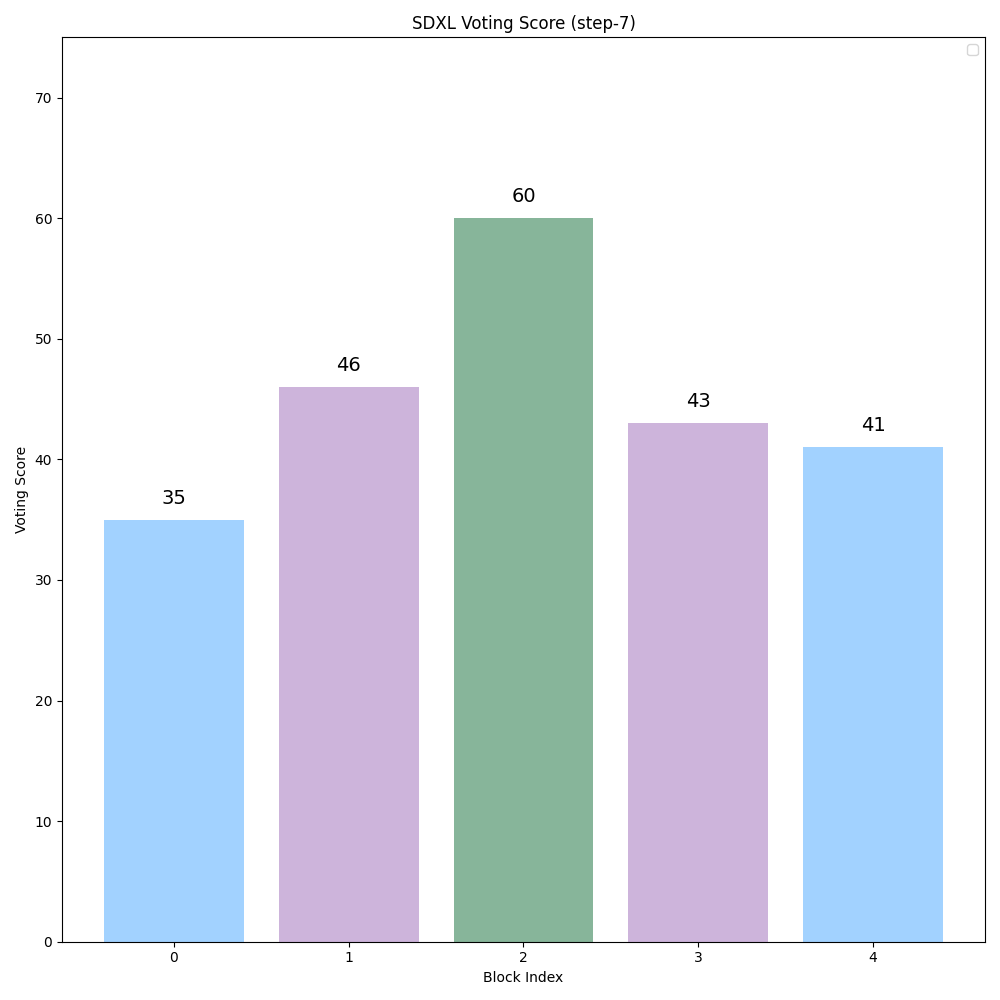}
        & 
        \includegraphics[width=0.175\linewidth]{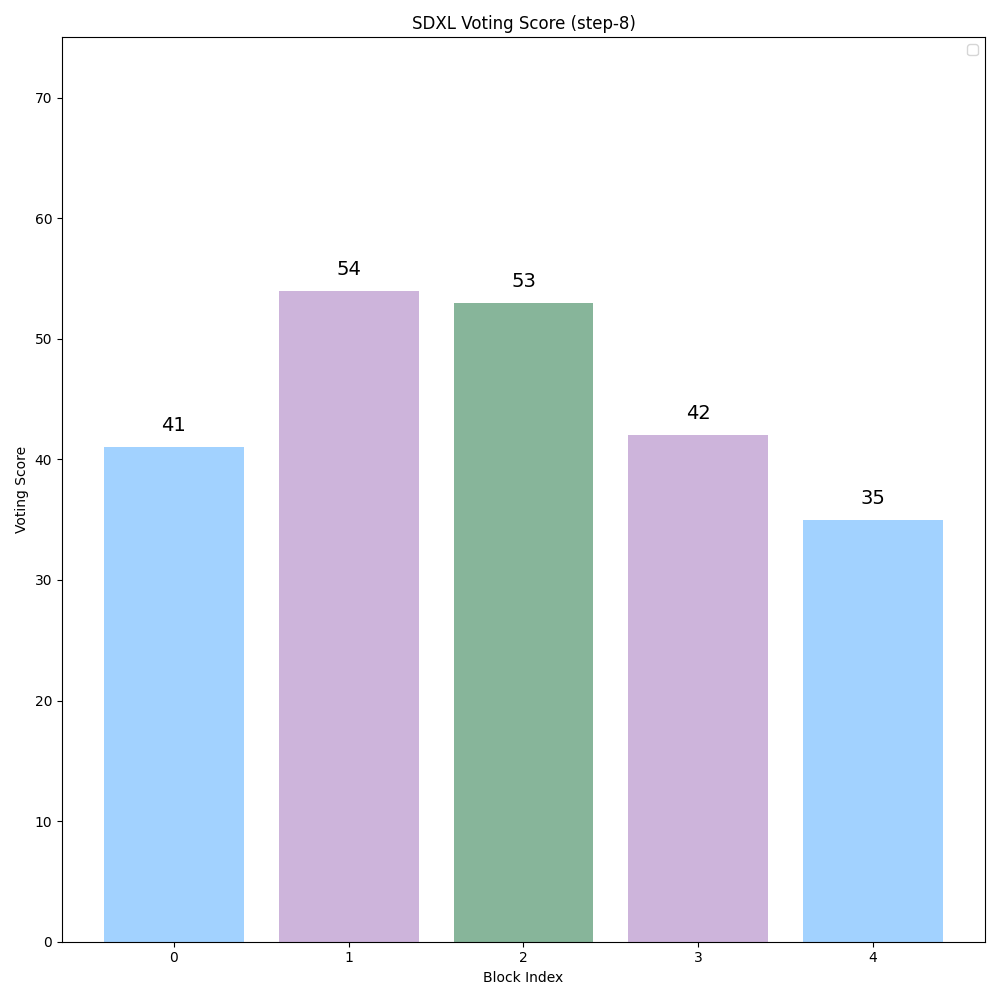}
        & 
        \includegraphics[width=0.175\linewidth]{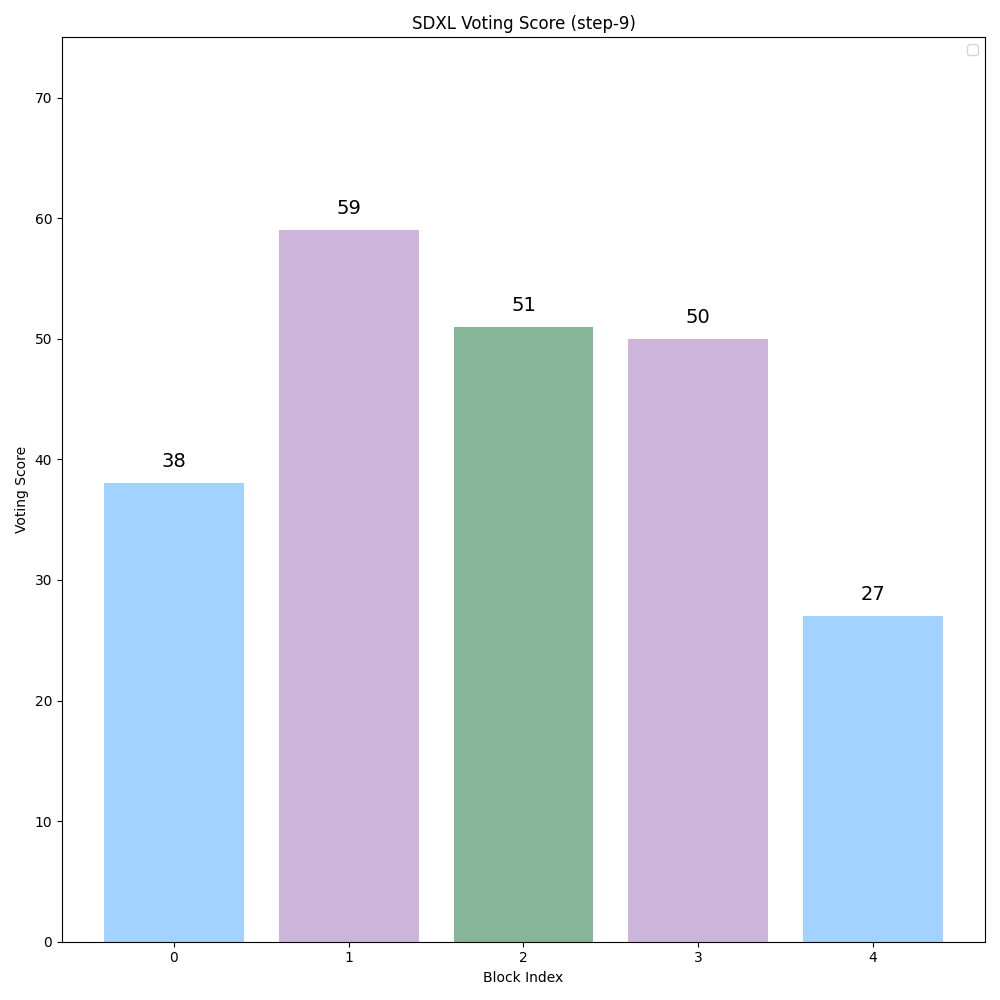}
        
        \\

        \includegraphics[width=0.175\linewidth]{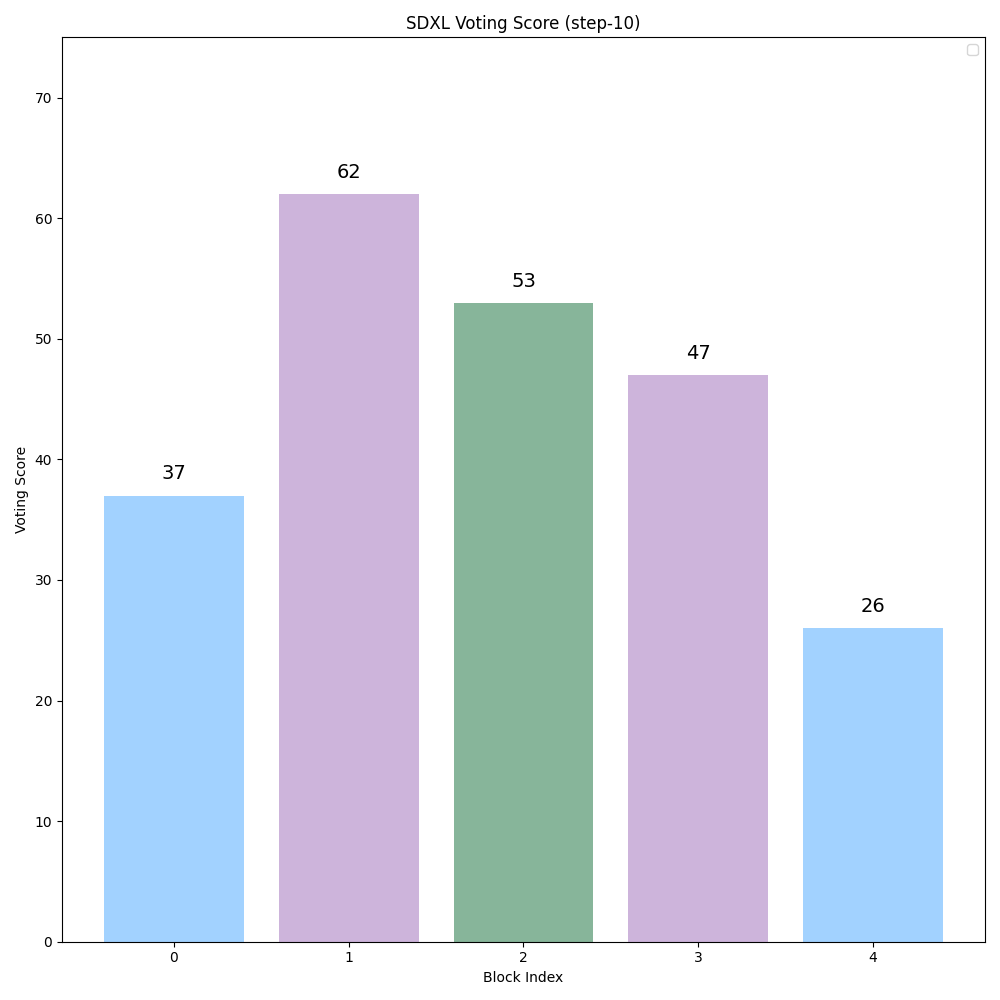} 
        & 
        \includegraphics[width=0.175\linewidth]{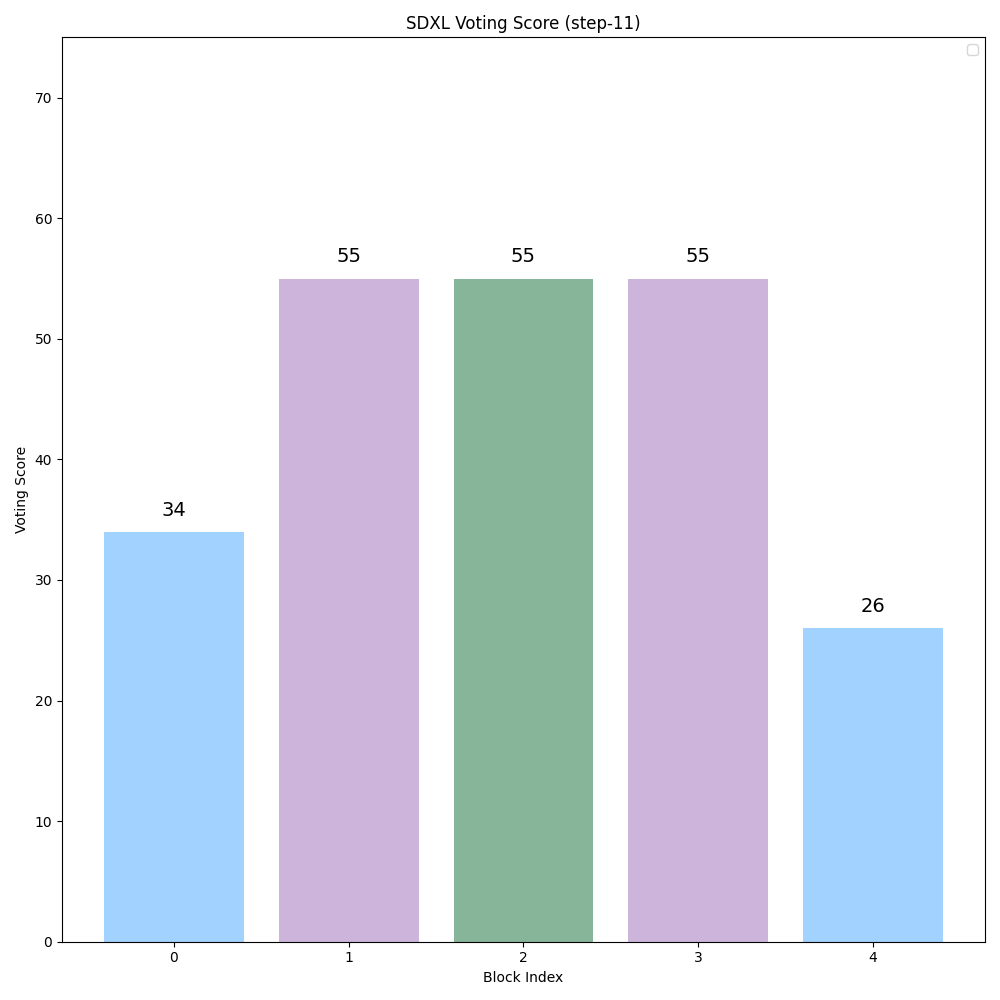}
        & 
        \includegraphics[width=0.175\linewidth]{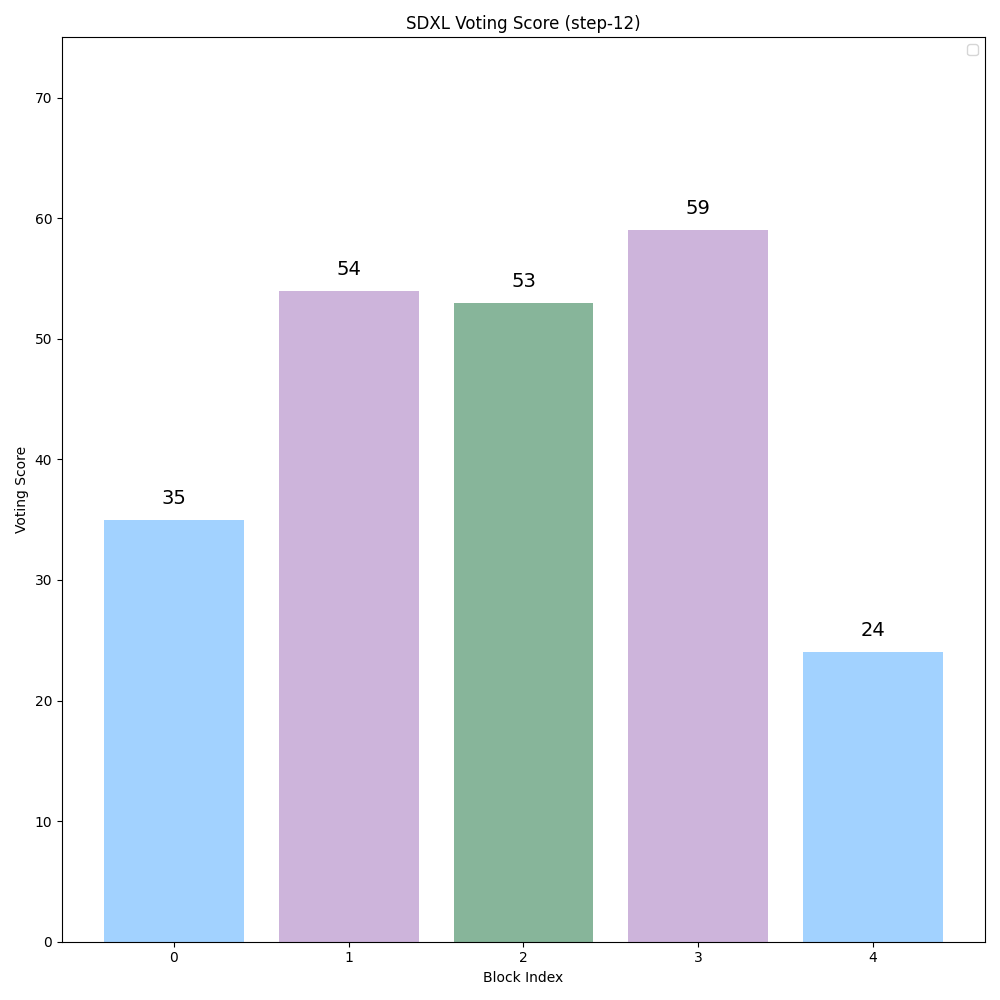}
        & 
        \includegraphics[width=0.175\linewidth]{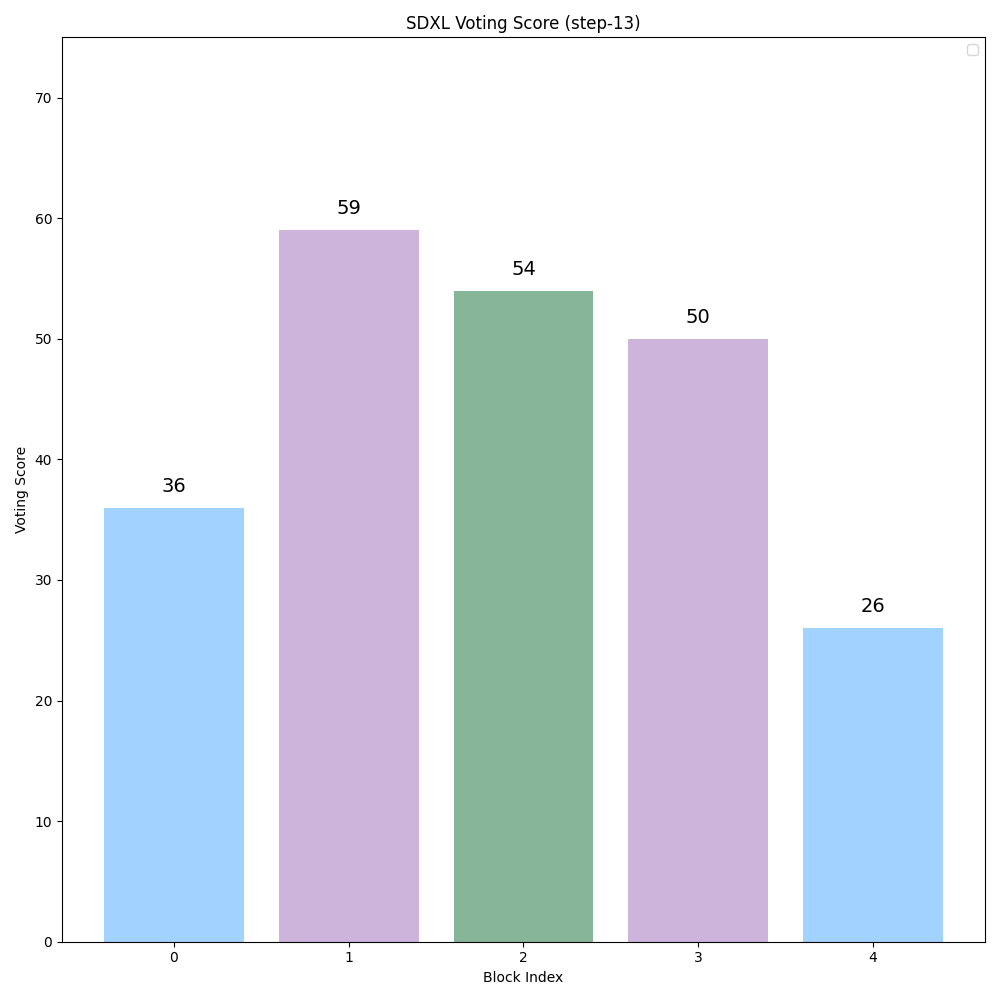}
        & 
        \includegraphics[width=0.175\linewidth]{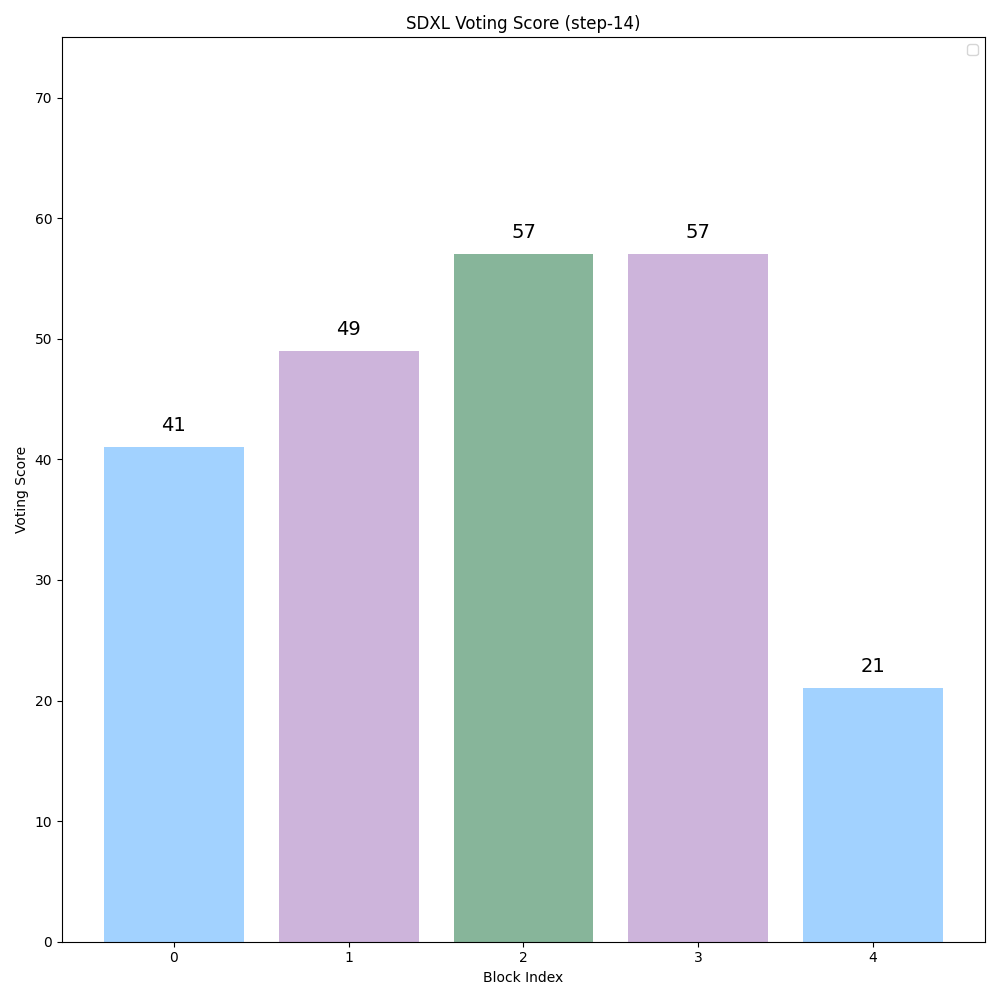}

        \\ 

        \includegraphics[width=0.175\linewidth]{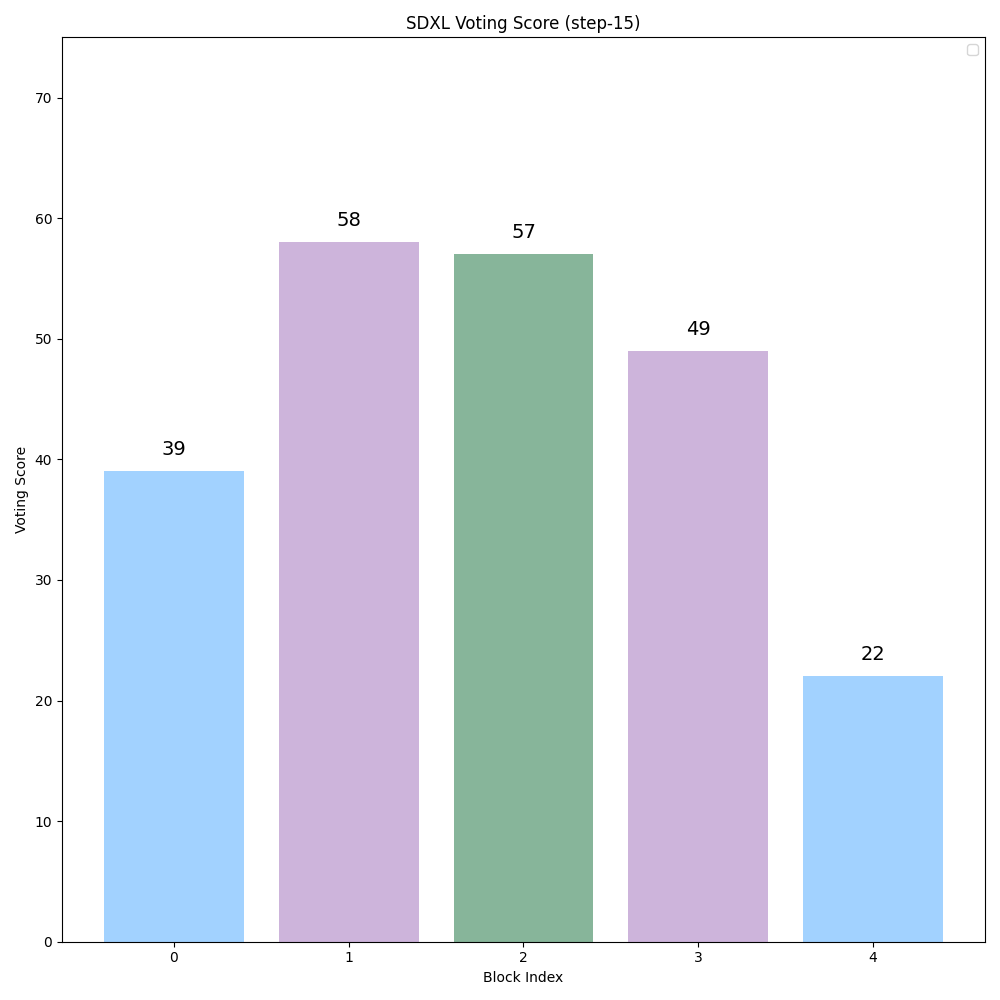} 
        & 
        \includegraphics[width=0.175\linewidth]{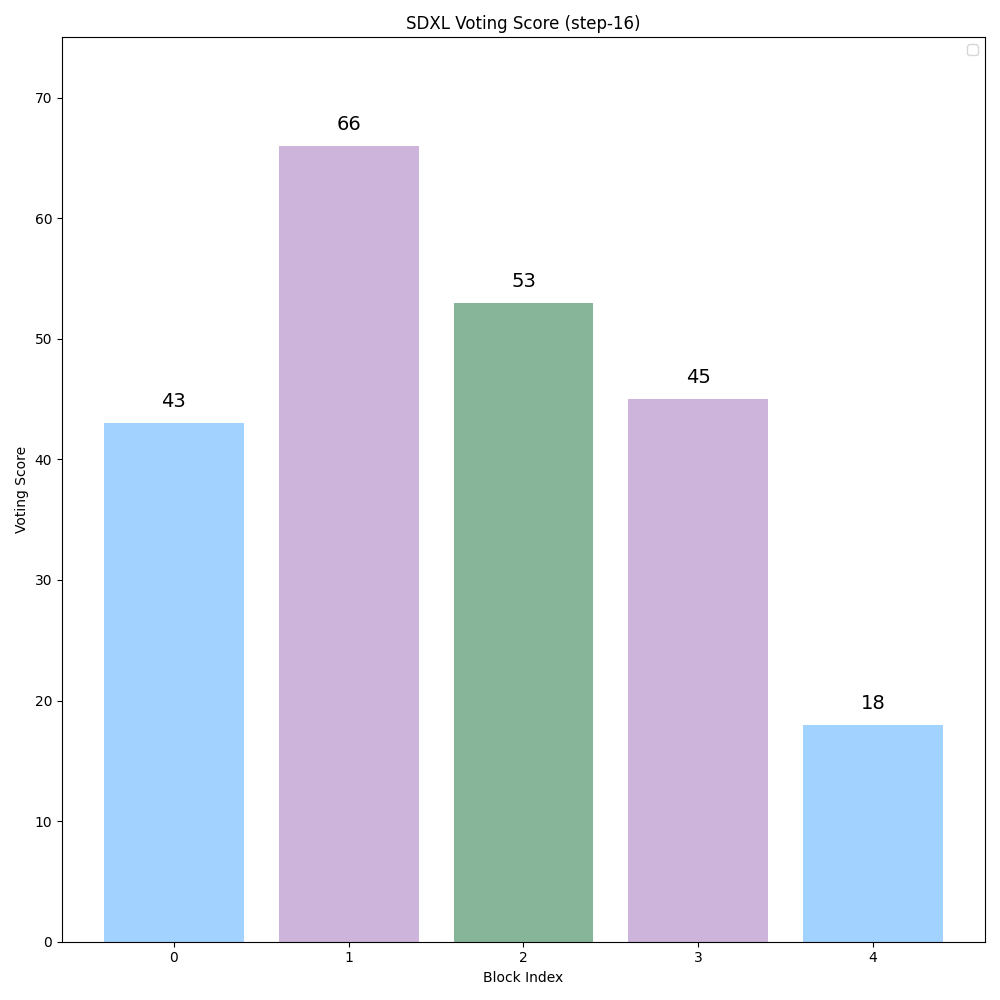}
        & 
        \includegraphics[width=0.175\linewidth]{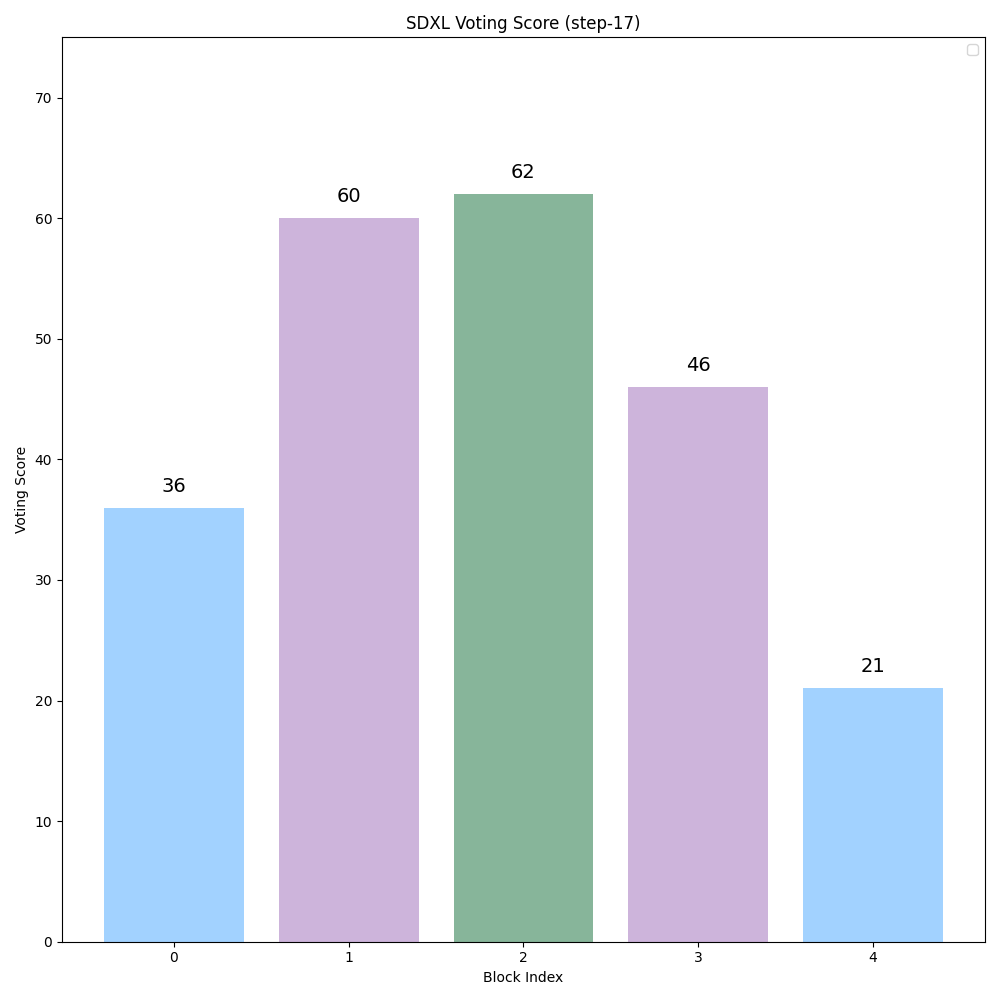}
        & 
        \includegraphics[width=0.175\linewidth]{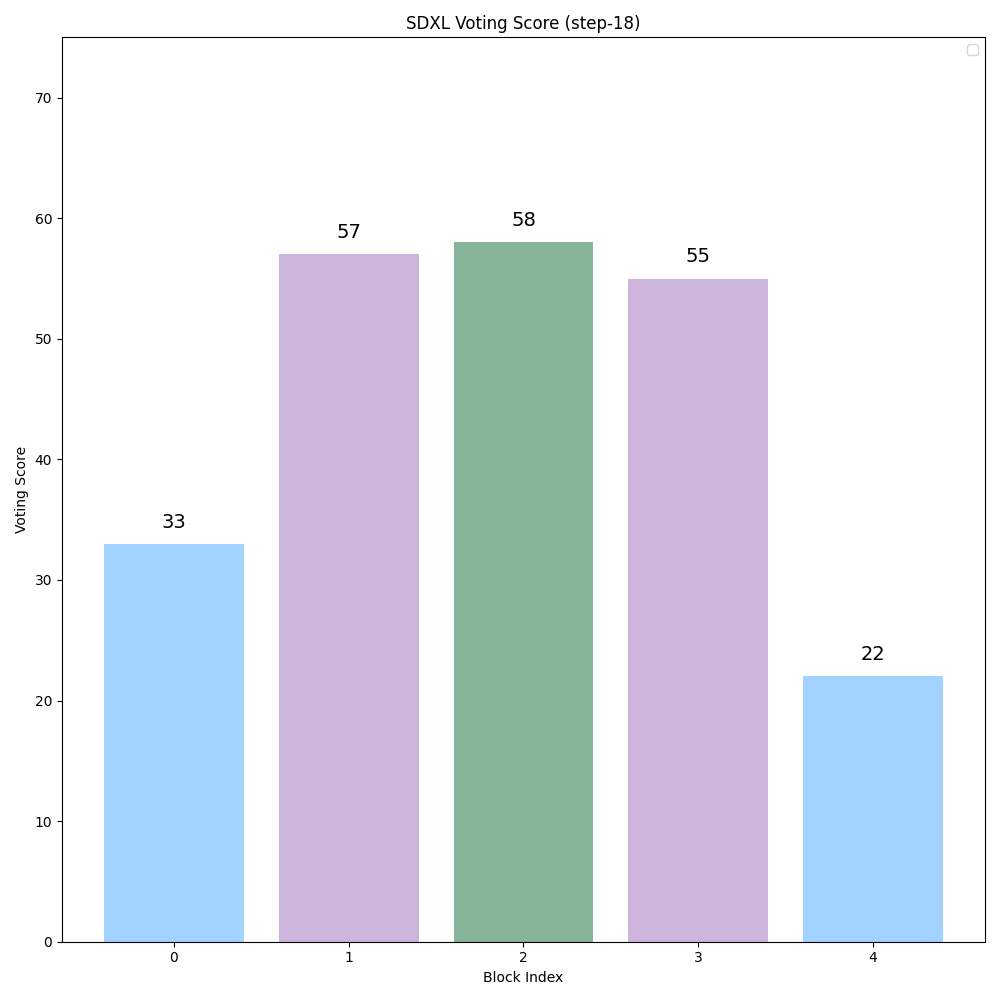}
        & 
        \includegraphics[width=0.175\linewidth]{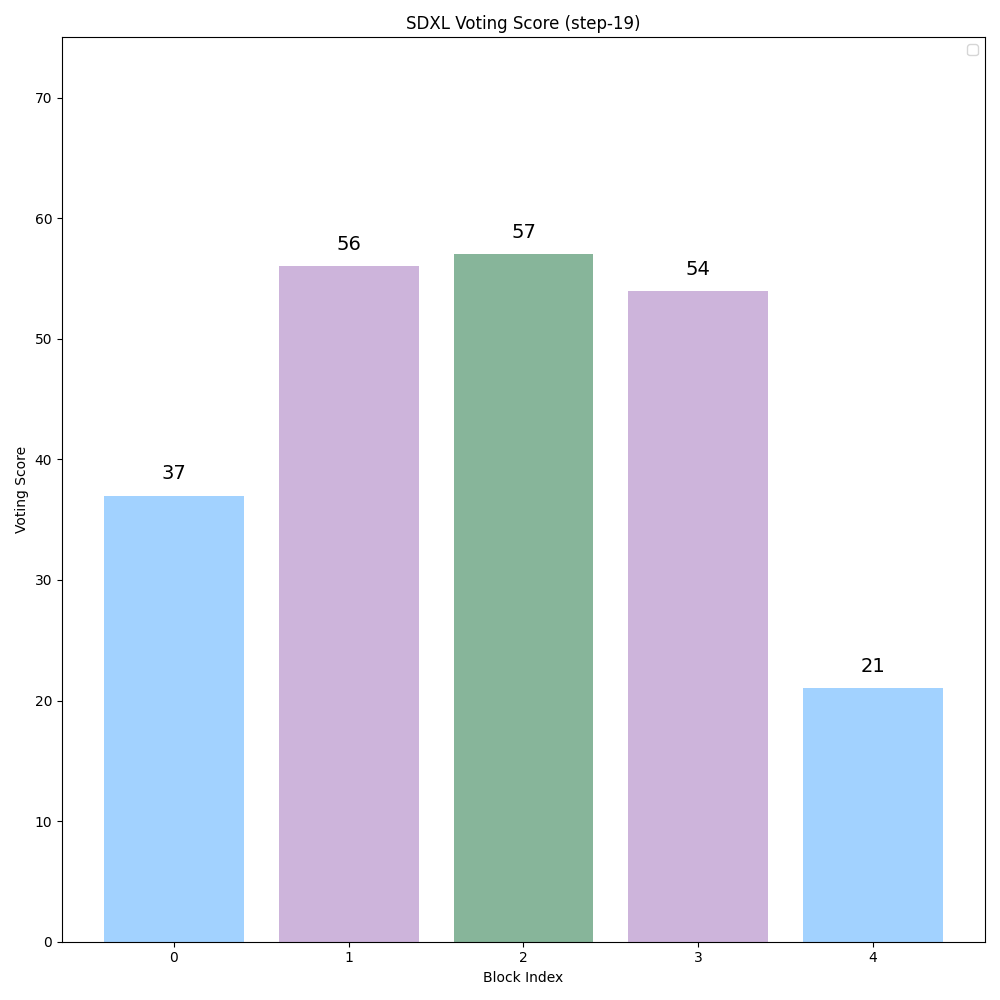}
    \end{tabular}
    \captionof{figure}{
        Bar charts of voting scores for SDXL. 
    }
    \label{tab-bar_chart_voting_score-sdxl}
\end{table*}

\paragraph{Importance Score}

To normalize the voting scores, we divide the above-mentioned voting scores by the maximum possible number of votes, and obtain the importance scores. 
The resulting heatmap is shown in Fig.~\ref{fig-heatmap_importance_score-sdturbo}, Fig.~\ref{fig-heatmap_importance_score-sdxlturbo}, Fig.~\ref{fig-heatmap_importance_score-sd} and Fig.~\ref{fig-heatmap_importance_score-sdxl}. 

The results demonstrate that, across different models and varying inference steps, the three blocks centered around the bottleneck consistently maintain a high level of importance throughout the inference process. 
This underscores the significance of the bottleneck structure to the U-Net's performance.

% 2 步 SD-Turbo 重要性得分热力图
\begin{figure}[ht]
    \centering
    \includegraphics[width=0.9\linewidth]{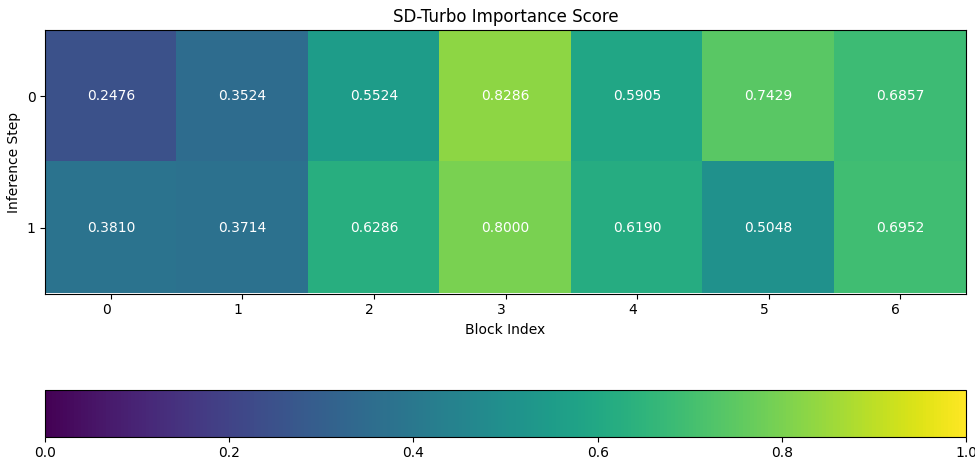}
    \caption{
        Heatmap of importance scores for SD-Turbo.  
    }
    \label{fig-heatmap_importance_score-sdturbo}
\end{figure}

% 2 步 SDXL-Turbo 重要性得分热力图
\begin{figure}[ht]
    \centering
    \includegraphics[width=0.9\linewidth]{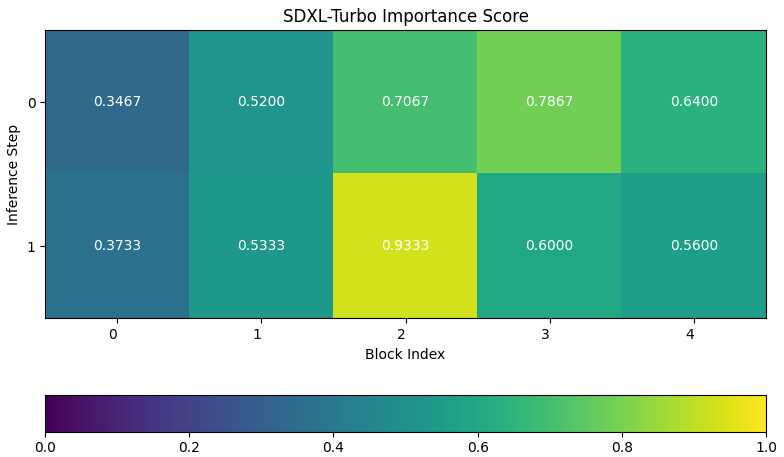}
    \caption{
        Heatmap of importance scores for SDXL-Turbo. 
    }
    \label{fig-heatmap_importance_score-sdxlturbo}
\end{figure}

% 20 步 SD 重要性得分热力图
\begin{figure}[ht]
    \centering
    \includegraphics[width=0.9\linewidth]{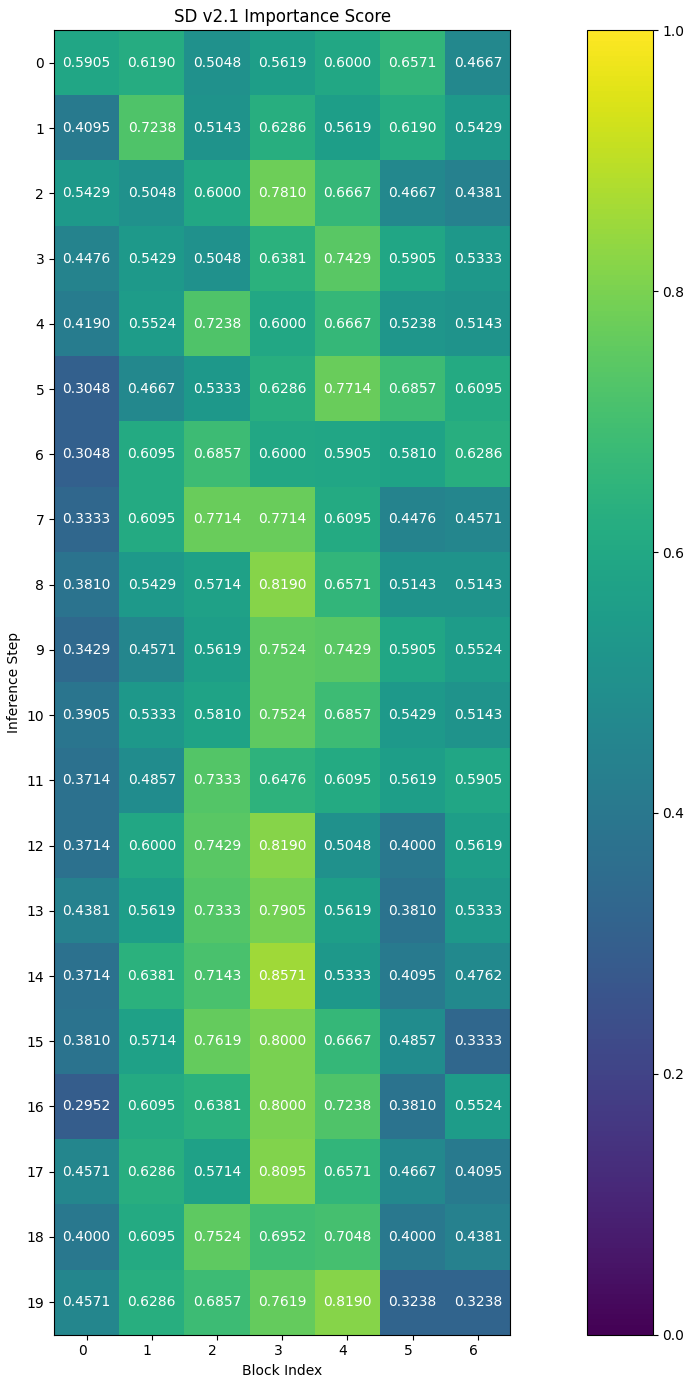}
    \caption{
        Heatmap of importance scores for SD v2.1. 
    }
    \label{fig-heatmap_importance_score-sd}
\end{figure}

% 20 步 SDXL 重要性得分热力图
\begin{figure}[ht]
    \centering
    \includegraphics[width=0.9\linewidth]{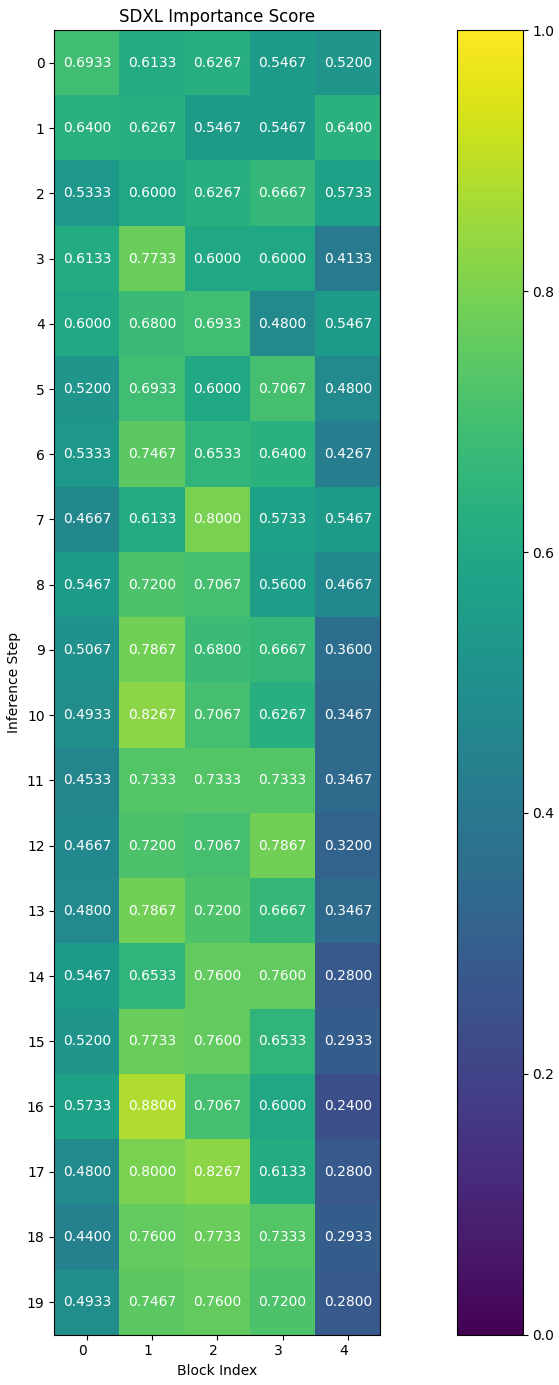}
    \caption{
        Heatmap of importance scores for SDXL. 
    }
    \label{fig-heatmap_importance_score-sdxl}
\end{figure}

\paragraph{Importance-based Re-weighting Schedule. }

We apply importance-based re-weighting to a wide range of prompts. 

Results are shown in Fig.~\ref{fig-hpd_sdturbo_sdxlturbo_fix_r_appx}. 
Unlike the static re-weighting schedules in Tab.~\ref{tab-comparison_between_different_models_and_steps_appx}, all our importance-based re-weighting schedules lead to performance improvements. 
It empirically validates the effectiveness of the IP, and the consistency between the experimental phenomena and theoretical analysis. 

% SD-Turbo/SDXL-Turbo 固定 r = 1.1, 随 l 变化的折线图
\begin{figure}[h]
    \centering
    \includegraphics[width=0.98\linewidth]{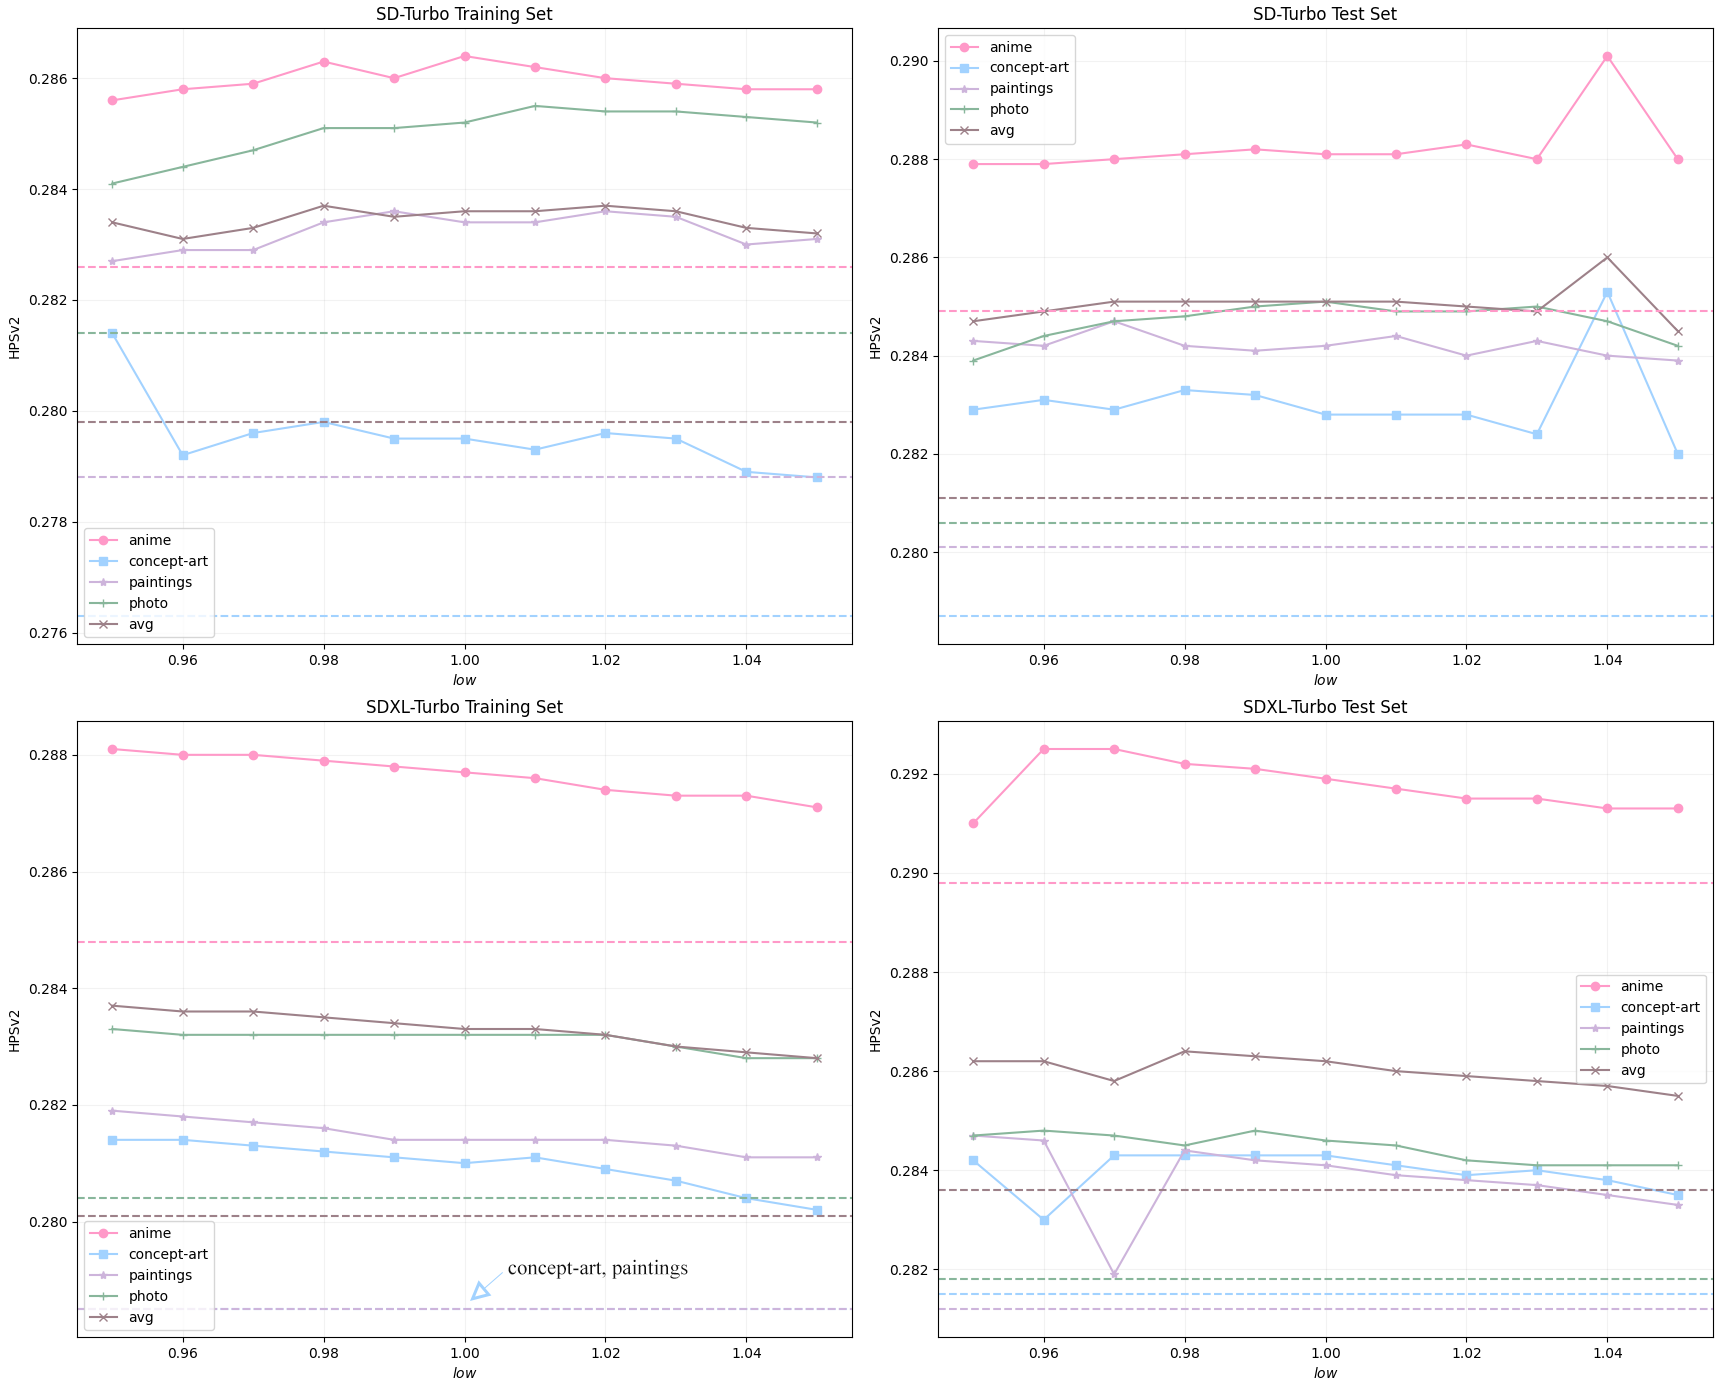}
    \caption{
        (Fig.~\ref{fig-hpd_sdturbo_sdxlturbo_fix_r} in the main paper. ) 
        Line chart showing the effect of re-weighting on SD-Turbo and SDXL-Turbo with fixed $high = 1.1$ as $low$ varies. 
        Lines of the same color represent the same category, where dashed lines indicate the vanilla schedule, and solid lines represent our re-weighting schedule. 
    }
    \label{fig-hpd_sdturbo_sdxlturbo_fix_r_appx}
\end{figure}

% Importance Probe Details
\section{More details of Importance Probe}
\label{appx_sec-the_methodology_and_implementation_of_importance_probe}

\subsection{Pseudo-Code of Importance Probe}

The pseudo-code of Importance Probe (IP) is summarized in Algo.~\ref{alg-weight_threshold_update}. 

% ---------= 伪代码中出现的操作 =---------
% 多参数 Input 的首个参数
\newcommand{\MultiInput}[1]{
  \textbf{Input:} 
  \begin{itemize}[leftmargin = 2em, noitemsep, topsep = 0pt]
    \item #1
  \end{itemize}
}

% 多参数 Output 的首个参数

% 增加参数
\newcommand{\AddItem}[1]{
  \begin{itemize}[leftmargin = 2em, noitemsep, topsep = 0pt]
    \item #1
  \end{itemize}
}

% 阈值更新过程伪代码
\begin{algorithm}
\caption{Importance Probe in a Epoch}
    % Input
    \MultiInput{\text{weight\_threshold\_matrix}}
    \AddItem{\text{history\_best\_weight\_matrix}}
    \AddItem{\text{letents}, \text{conditions}}

    \vspace{5pt}
    
    \begin{algorithmic}[1]
        \State $\text{weight\_threshold\_list} \newline
        \hspace*{10pt} \leftarrow \text{weight\_threshold\_matrix}[\text{inference\_step}]$
        \State $\text{best\_fitness} \leftarrow \text{cal\_fitness}(\text{weight\_threshold\_list})$
        \State
        \State $\text{best\_weight\_list} \leftarrow \varnothing$
        \State $\text{accepted\_mask} \leftarrow [\text{False}] \times \text{num\_inference\_step}$

        \State
        
        \For{$\text{inference\_step} = 0$ to $(\text{num\_inference\_step} - 1)$}
            \State $\text{time\_step} \leftarrow \text{time\_steps}[\text{inference\_step}]$
            \State $\epsilon_{\text{tea}} \leftarrow \text{tea\_U-Net}(\text{letents}, \text{conditions}, \text{time\_step})$
            
            \State 
            
            \State $\text{cur\_weight\_list} \newline 
            \hspace*{20pt} \leftarrow \text{history\_best\_weight\_matrix}[\text{inference\_step}]$
            
            \For{$\text{stu\_try} = 1$ to $(\text{num\_stu\_try} - 1)$}
                \State $\text{weight\_list}$ \newline 
                    \hspace*{40pt} $\leftarrow \text{WeightBiasSchedule}(\text{cur\_weight\_list})$ 
                
                \State $\text{stu\_U-Net.set\_weight}(\text{weight\_list})$
                
                \State $\epsilon_{\text{stu}} \leftarrow \text{stu\_U-Net}(\text{letents},  \text{conditions}, \text{time\_step})$

                \State 
                
                \If{$\text{criterion}(\epsilon_{\text{tea}}, \epsilon_{\text{stu}}) \leq \text{loss\_threshold}$}
                    \State $\text{tmp\_fitness} = \text{cal\_fitness}(\text{weight\_list})$
                    \If{$\text{tmp\_fitness} > \text{best\_fitness}$}
                        \State $\text{best\_fitness} \leftarrow \text{tmp\_fitness}$
                        \State $\text{best\_weight\_list} \leftarrow \text{weight\_list}$
                    \EndIf
                \EndIf
            \EndFor
            \State
            \If{$\text{best\_weight\_list} == \varnothing$}
                \State $\text{weight\_threshold\_matrix}[\text{inference\_step}]$ \newline
                    \hspace*{40pt} $\leftarrow \text{cur\_weight\_list}$
            \Else
                \State $\text{accepted\_mask}[\text{inference\_step}] \leftarrow \text{True}$
                \State $\text{weight\_threshold\_matrix}[\text{inference\_step}]$ \newline
                    \hspace*{40pt} $\leftarrow \text{best\_weight\_list}$
                \State $\text{history\_best\_weight\_matrix}[\text{inference\_step}]$ \newline
                    \hspace*{40pt} $\leftarrow \text{best\_weight\_list}$
            \EndIf

            \State 

            \State $\text{latents} \leftarrow \text{scheduler.step}(\text{latents}, \epsilon_{\text{tea}}, \text{time\_step})$
        \EndFor

        \State 

        \State $\text{weight\_threshold\_matrix}$ \newline
            \hspace*{10pt} $\leftarrow \text{ThresholdUpdateScheduler}(\text{accepted\_mask})$
    \end{algorithmic}
\label{alg-weight_threshold_update}
\end{algorithm}

\subsection{Threshold Update Schedule}

Let ``the weight set is accepted" to be event $A$, and ``the current threshold being too high, moderate, or too low" be events $B_1$, $B_2$ and $B_3$, respectively. 

Let $Q = [\pmb{q}_1, \cdots, \pmb{q}_n]$ be the current optimal threshold matrix, where $n$ is the number of inference steps and $\pmb{q}_i \in [0, 1]^m\ \ (1 \leq i \leq n)$ stands for the optimal thresholds for the $m$ target blocks. 

If an optimal weight matrix $W = [\pmb{w}_1, \cdots, \pmb{w}_n]$ is found during an iteration, where $\pmb{w}_i \in [0, 1]^m\ \ (1 \leq i \leq n)$ represents the optimal weights for the $m$ target layers, then the new thresholds matrix $Q' = [\pmb{q}_1', \cdots, \pmb{q}_n']$ are obtained as follows:

For an accepted weight set $\pmb{w}_i$ :

\begin{equation}
    \begin{aligned}
        \pmb{q}_i' =
        &~ P(B_1 \mid A) \times (\pmb{q}_i / 2) \\
        &+ P(B_2 \mid A) \times \pmb{q}_i + P(B_3 \mid A) \times (\pmb{w}_i - \varepsilon)
    \end{aligned}, 
    \label{eq-threshold_update_accpeted}
\end{equation}
while for a rejected one $\pmb{w}_j$:
\begin{equation}
    \begin{aligned}
        \pmb{q}_j' = 
        &~ P(B_1 \mid \overline{A}) \times (\pmb{q}_j / 2) \\
        &+ P(B_2 \mid \overline{A}) \times \pmb{q}_j + P(B_3 \mid \overline{A}) \times (\pmb{w}_j - \varepsilon)
    \end{aligned}, 
    \label{eq-threshold_update_rejected}
\end{equation}
where $\varepsilon$ is a minute positive number. 

Since the thresholds tend to stabilize to moderate values during the probing process, we set $P(B_2 \mid A)$ in Eq.~\ref{eq-threshold_update_accpeted} to linearly increase from $P_{\text{st}} (B_2 \mid A)$ to $P_{\text{ed}} (B_2 \mid A)$, and $P(B_3 \mid A)$ to linearly decrease from $P_{\text{st}} (B_3 \mid A)$ to $P_{\text{ed}} (B_3 \mid A)$. 
Similarly, in Eq.~\ref{eq-threshold_update_rejected}, $P(B_1 \mid \overline{A})$ and $P(B_2 \mid \overline{A})$ are set to decrease and increase, respectively. 

Compared to the common hard or soft update strategies, our conditional-expectation-based threshold update strategy can counteract the biases introduced by randomness in a stochastic environment, providing more reliable updates.

\subsection{Importance Ranking in a Single Run of IP}

Let $n$ and $m$ be the number of inference steps and the number of probing targets (the number of attention blocks in this study) respectively. 

We will obtain a sequence of weight threshold lists in a run of IP, denoted by $\pmb{\text{wt}} = [\pmb{\text{wt}}^{(0)}, \cdots, \pmb{\text{wt}}^{(n - 1)}]$, where $\pmb{\text{wt}}^{(t)} = [\pmb{\text{wt}}_0^{(t)}, \cdots, \pmb{\text{wt}}_{m - 1}^{(t)}]$ represents the weight thresholds for each block at denoising step $t$. 

For each inference step $t$, the \emph{importance ranking} $\pmb{\text{rk}}^{(t)}$ is derived by sorting the list of block indices $[0, \cdots, m - 1]$ based on the corresponding weight thresholds in $\text{wt}^{(t)}$ in non-descreasing order. 
For short, $\pmb{\text{rk}}^{(t)} = \mathrm{argsort}(\pmb{\text{wt}}^{(t)})$, where $\mathrm{argsort}$ returns the permutation of indices that sorts $\pmb{\text{wt}}^{(t)}$ in ascending order. 
To ensure the uniqueness of each threshold value and avoid redundancy, we introduce small random perturbations to $\pmb{\text{wt}}^{(t)}$ before computation, which ensures that no identical threshold values exist, thereby allowing for the derivation of a reasonable importance ranking for any set of threshold values.

The derived importance rankings can be represented as a sequence of vectors $\pmb{\text{rk}} = [\pmb{\text{rk}}^{(0)}, \cdots, \pmb{\text{rk}}^{(n - 1)}]$, where each vector corresponds to a permutation of $0$ to $(m - 1)$.

\subsection{Noise Prediction Tolerance \& Weight Bias Schedule}

\cite{esser2024scaling} noted that, when training diffusion models, the time steps at the beginning and end are easier to learn, while the intermediate time steps are more challenging. 

We selectively follow this observation.  
The maximum allowed tolerance for noise prediction and the maximum magnitude of perturbations in the Importance Bias Schedule are set to increase linearly along the inference progress. 
It aims to constrain the student U-Net to follow the denoising trajectory of the teacher U-Net in the early stages, while encouraging the student U-Net to explore finer image details in the later stages independently. 
This strategy enables the IP to better distinguish the importance of different blocks through larger perturbations.

In the early denoising, we choose a smaller tolerance to counteract the stochasticity in the probing process, thereby achieving faster convergence.

\subsection{Hyper-parameters}

\paragraph{Importance Probe}

For each specific task, we conduct a few runs of IP, with each round consisting of several perturbations to the weights and updates to the threshold values. 
We empirically found that the setting of $15$ runs and $20$ perturbations per run, is sufficient to achieve a relatively \emph{stable} importance ranking in the subsequent voting mechanism. 

Specifically, it can be ensured that, when the statistics from the rounds of voting are traversed in any order, the sequences of importance rankings derived from the last $5$ prefixes of each traversal have a distance no greater than $\dfrac{n}{2}$. 
The \emph{distance} of two sequences of importance rankings $\pmb{\text{rk}}_a = [\pmb{\text{rk}}_{a}^{(0)}, \cdots, \pmb{\text{rk}}_{a}^{(n - 1)}]$ and $\pmb{\text{rk}}_b = [\pmb{\text{rk}}_{b}^{(0)}, \cdots, \pmb{\text{rk}}_{b}^{(n - 1)}]$ is computed as
\begin{equation}
    \text{dist} (\pmb{\text{rk}}_a, \pmb{\text{rk}}_b)
    = 
    \sum_{t = 0}^{n - 1} \text{dist} (\pmb{\text{rk}}_{a}^{(t)}, \pmb{\text{rk}}_{b}^{(t)})
    , 
\end{equation}
where $\text{dist} (\pmb{\text{rk}}_{a}^{(t)}, \pmb{\text{rk}}_{b}^{(t)})$ is the \emph{distance} between the two importance rankings $\pmb{\text{rk}}_{a}^{(t)}$ and $\pmb{\text{rk}}_{b}^{(t)}$, which is defined as the bubble sort distance of these two permutations. 

\paragraph{Noise Prediction Tolerance \& Weight Bias Schedule}

The maximum allowed noise prediction tolerance is set to linearly increase from $1\text{e}-4$ to $2\text{e}-4$. 

The maximum magnitude of the perturbations in the Weight Bias Schedule is set to linearly increase from $0.02$ to $0.05$. 

\paragraph{Threshold Update Schedule}

We selected the following hyper-parameters for the Threshold Update Schedule across all tasks. 

\begin{table}[h]
    \centering
    \caption{
        Hyper-parameters for the Weight Threshold Update Schedule. 
    }
    \begin{tabular}{c | c}
        \hline
        Param Name & Value \\
        \hline

        $\epsilon$ & $1\text{e}-2$ \\

        \hdashline

        $P(B_1 \mid A)$ & $0.06$ \\
        $P_{\text{st}} (B_2 \mid A)$ & $0.47$ \\ 
        $P_{\text{ed}} (B_2 \mid A)$ & $0.84$ \\ 
        $P_{\text{st}} (B_3 \mid A)$ & $0.47$ \\ 
        $P_{\text{ed}} (B_3 \mid A)$ & $0.10$ \\ 

        \hdashline

        $P_{\text{st}} (B_1 \mid \overline{A})$ & $0.48$ \\ 
        $P_{\text{ed}} (B_1 \mid \overline{A})$ & $0.30$ \\ 
        $P_{\text{st}} (B_2 \mid \overline{A})$ & $0.48$ \\ 
        $P_{\text{ed}} (B_2 \mid \overline{A})$ & $0.66$ \\ 
        
        $P(B_3 \mid \overline{A})$ & $0.04$ \\ 

        \hline
    \end{tabular}
    \label{tab-hyper_parameter_weight_threshold_update_schedule}
\end{table}

\subsection{Limitations}

The Importance Probe requires multiple rounds of heuristic search, with each round involving several epochs, to counteract the influence of randomness. 
This process incurs a significant computational overhead. 

Besides, the maximum noise prediction tolerance, the maximum perturbation magnitude of the Weight Bias Schedule, and the conditional probabilities of the Threshold Update Schedule need to be empirically and manually selected, which may not be applicable to all scenarios.

% Implementation Details
\section{Experiment Setup and Configuration}
\label{appx_sec-experimental_setup_and_model_configuration}

This section provides the implementation details of our experiments to facilitate the reproduction.

\subsection{Pre-trained Models}

We selected the following pre-trained models as fundamental models in this project: 

\begin{itemize}
    \item \textbf{stabilityai/sd-turbo}~\cite{sauer2023adversarialdiffusiondistillation} at \\
    \href{https://huggingface.co/stabilityai/sd-turbo}{https://huggingface.co/stabilityai/sd-turbo}. 

    \item \textbf{stabilityai/sdxl-turbo}~\cite{sauer2024fasthighresolutionimagesynthesis} at \\
    \href{https://huggingface.co/stabilityai/sdxl-turbo}{https://huggingface.co/stabilityai/sdxl-turbo}. 

    \item \textbf{stabilityai/stable-diffusion-2-1-base}~\cite{rombach2022highresolutionimagesynthesislatent} at \\
    \href{https://huggingface.co/stabilityai/stable-diffusion-2-1-base}{https://huggingface.co/stabilityai/stable-diffusion-2-1-base}. 

    \item \textbf{stabilityai/stable-diffusion-xl-base-1.0}~\cite{podell2023sdxlimprovinglatentdiffusion} at \\ 
    \href{https://huggingface.co/stabilityai/stable-diffusion-xl-base-1.0}{https://huggingface.co/stabilityai/stable-diffusion-xl-base-1.0}. 
\end{itemize}

We employ the fp16 versions of the aforementioned models for fine-tuning and inference. 

\subsection{Metric Computation}

We utilized the following third-party libraries for metric computation: 

\begin{itemize}
    \item \textbf{Human Preference Score v2} (1.2.0)~\cite{wu2023humanpreferencescorev2} at \\
    \href{https://github.com/tgxs002/HPSv2}{https://github.com/tgxs002/HPSv2}. 

    \item \text{pytorch-fid} (0.3.0)~\cite{yu2021frechet} at \\
    \href{https://github.com/mseitzer/pytorch-fid}{https://github.com/mseitzer/pytorch-fid}. 

    \item \text{lpips} (0.1.4)~\cite{zhang2018unreasonable} at \\ 
    \href{https://github.com/richzhang/PerceptualSimilarity}{https://github.com/richzhang/PerceptualSimilarity}. 
\end{itemize}

\subsection{Implementation}

We modified the the HuggingFace diffusers~\cite{von-platen-etal-2022-diffusers} library for implementation in this project.

% Dynamic Attention Pruning Tests Details
\section{Supplementary to Dynamic Attention Pruning}
\label{appx_sec-the_methodology_and_evaluation_of_dynamic_attention_pruning_tests}

\subsection{Overview}

We provide a schematic of dynamic attention pruning of diffusion U-Net in Fig.~\ref{fig-dynamic_pruning}. 

\begin{figure}[h]
    \centering
    \includegraphics[width=0.98\linewidth]{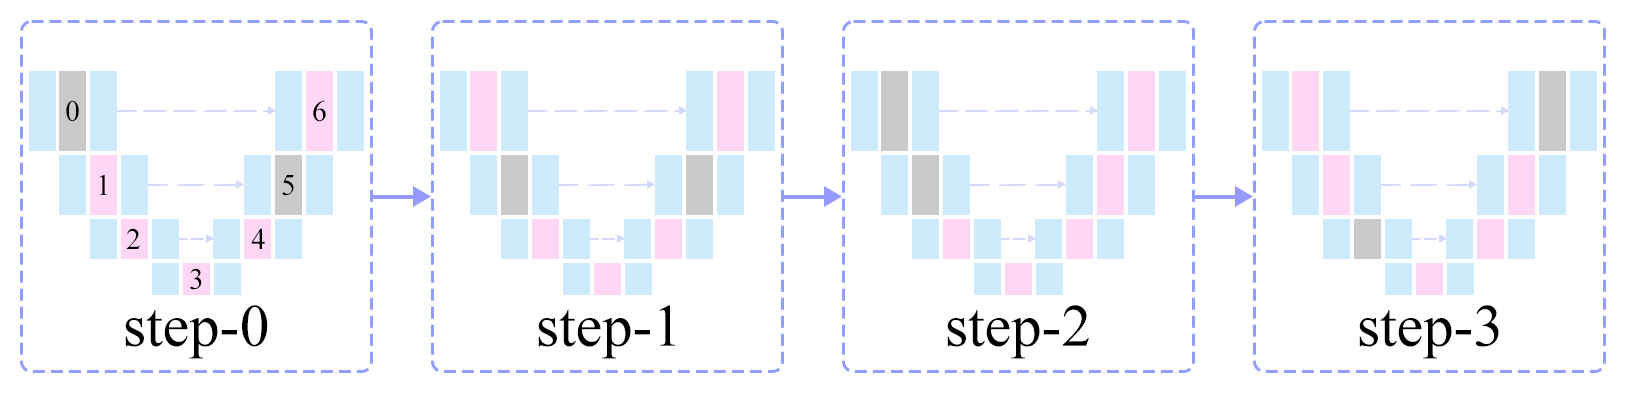}
    \caption{
        The schematic of dynamic pruning of SD U-Net, in which the gray rectangles represent the skipped Transformer blocks in that step. 
    }
    \label{fig-dynamic_pruning}
    \vspace{-10pt}
\end{figure}

\subsection{Strategy Design Mechanism}

Due to the potential synergistic effects among components within the network, simply skipping the least important blocks does not always guarantee optimal performance. 
To address this, we introduce a \emph{strategy design mechanism} to design skipping strategies based on the derived importance ranking. 

Specifically, at each denoising step, we focus on the three blocks with the lowest importance scores. 
Denote the indices of these blocks at step $t$ as $idx_0^{(t)}$, $idx_1^{(t)}$, $idx_2^{(t)}$. 

\begin{itemize}
    \item For single-block skipping strategies, we consider skipping block-$idx_0^{(t)}$ or block-$idx_1^{(t)}$ or block-$idx_2^{(t)}$. 
    \item For two-block skipping strategies, examine all the combinations of skipping (block-$idx_0^{(t)}$ and block-$idx_1^{(t)}$) or (block-$idx_0^{(t)}$ and block-$idx_2^{(t)}$) or (block-$idx_1^{(t)}$ and block-$idx_2^{(t)}$). 
\end{itemize}

We employ Depth First Search (DFS) to traverse all recommended skipping block combinations across the inference steps, constructing a set of task-specific skipping strategies.
For skipping strategies that involve skipping $k\ \ (1 \leq k \leq 3)$ block(s), $(C_3^k)^n$ schedule(s) will be recommended, and some of them may be duplicated or overlap with baseline strategies. 

\subsection{Experimental Settings}

We select the pre-trained SD-Turbo as the fundamental model. 
Following Sec.~\ref{appx_section-empirical_results_and_theoretical_consistency_subsection-appropriately_reweighting_contributions}, we choose the 2-step-inference task with the prompt ``\emph{Some cut up fruit is sitting in a blender.}'' as our target task.

For each skipping strategy provided by the strategy design mechanism, the student U-Net, adopting the corresponding skipping strategy, is fine-tuned on the training set under the supervision of the full teacher U-Net. 
We set the seeds for the training and test sets to $0$ and $21$, respectively, with each set comprising 100 distinct generation trajectories from the teacher U-Net.

We set the batch size to $8$. 
The student U-Net is fine-tuned for $300$ epochs with a learning rate of $5\mathrm{e}-6$. 
The fine-tuned student U-Net is then used for sampling, and the generation quality is compared with that of the teacher U-Net.

\subsection{Skipping Strategies}

All the recommended skipping strategies provided by the strategy design mechanism are listed in Tab.~\ref{tab-skipping_strategy_sdturbo_fruit_all}. 

% SD-Turbo 跳过策略 (全)
\begin{table}[h]
    \centering
    \begin{tabular}{c | c c | c}
        \hline
        
        \textbf{Strategy} & \multicolumn{2}{c|}{\textbf{Skipped Block Indices}} & \multirow{2}{*}{\textbf{Note}}  \\
        
        \textbf{Index} & step-0 & step-1 & ~ \\
        
        \hline

        % skip-1: baseline
        a.0 & 0 & 0 & block-0 \\
        a.1 & 1 & 1 & block-1\\
        a.2 & 2 & 2 & block-2 \\
        a.3 & 3 & 3 & block-3 \\
        a.4 & 4 & 4 & block-4\\
        a.5 & 5 & 5 & block-5 \\
        a.6 & 6 & 6 & block-6 \\

        \hdashline

        % skip-1: ours
        b.0 & 0 & 1 & ~ \\
        b.1 & 0 & 0 & identical to a.0 \\
        b.2 & 1 & 1 & identical to a.1 \\
        b.3 & 1 & 0 & ~ \\

        \hline

        % skip-2: baseline
        c.0 & 0, 6 & 0, 6 & floor-0 \\
        c.1 & 1, 5 & 1, 5 & floor-1 \\
        c.2 & 2, 4 & 2, 4 & floor-2 \\

        \hdashline

        % skip-2: ours
        d.0 & 0, 1 & 0, 1 & ~ \\
        d.1 & 0, 1 & 1, 5 & ~ \\
        d.2 & 0, 1 & 0, 5 & ~ \\
        d.3 & 0, 2 & 0, 1 & ~ \\
        d.4 & 0, 2 & 1, 5 & ~ \\
        d.5 & 0, 2 & 0, 5 & ~ \\
        d.6 & 1, 2 & 0, 1 & ~ \\
        d.7 & 1, 2 & 1, 5 & ~ \\
        d.8 & 1, 2 & 0, 5 & ~ \\

        \hline
    \end{tabular}
    \caption{
        Table of task-specific skipping strategies. 
    }
    \label{tab-skipping_strategy_sdturbo_fruit_all}
\end{table}

\subsection{Qualitative Results}

We provide qualitative results of samples generated by the pruned U-Net under different skipping strategies in Fig.~\ref{fig-sample_pruned_sdturbo_fruit_skip_1_a}, Fig.~\ref{fig-sample_pruned_sdturbo_fruit_skip_1_b}, Fig.~\ref{fig-sample_pruned_sdturbo_fruit_skip_2_c} and Fig.~\ref{fig-sample_pruned_sdturbo_fruit_skip_2_d}. 

The results demonstrate that, the U-Nets pruned under our skipping strategies achieve higher fidelity in pruned sampling (e.g., a more realistic blender), particularly when two blocks are skipped per step. 
Moreover, our pruned U-Net exhibits superior generalization on the test set.

\subsection{More Quantitative Results}

To quantitatively access the performance of the pruned U-Nets, we calculate some relative metrics are listed below: 

\begin{itemize}
    \item \textbf{FID} (Fréchet Inception Distance)~\cite{yu2021frechet}: measures the fidelity of the generated image compared to the original image. 
    \item \textbf{LPIPS} (Learned Perceptual Image Patch Similarity)~\cite{zhang2018unreasonable}: indicates the image quality and similarity. 
\end{itemize}

Using the samples generated by the teacher U-Net as the reference set, we calculate the FID and LPIPS for the fine-tuned student U-Net on the training and testing set, respectively. 

Quantitative results are presented in Table~\ref{tab-fid_lpips_fruit_all_appx}, with the corresponding scatter plots shown in Fig.~\ref{fig-scatter_fid_lpips_fruit_appx}. 
The results indicate that, the samples generated by our pruned U-Net achieve superior FID and LPIPS scores, particularly when two blocks are skipped per step. 

Notably, we find that, consistently skipping blk-3 (skipping strategy a.3) yields the best performance. 
We hypothesize that, this is due to blk-3 having the lowest resolution and the fewest parameters, allowing its functionality to be effectively compensated by the remaining two bottleneck blocks (blk-2 and blk-4). 
This hypothesis is supported by the results of the static skipping strategies in group (a).
It shows that statically skipping high-resolution blocks incurs a greater quality loss compared to statically skipping mid-low-resolution blocks.

Conversely, in a dynamic context, skipping mid-low-resolution blocks is not necessarily the optimal strategy. 
For instance, in the aforementioned experiments, our dynamic skipping strategy d.7 outperforms the static skipping strategy c.2. 
This highlights the importance of considering the dynamic importance shifts of blocks during the pruning process, rather than simply focusing on their resolutions.

% SD-Turbo 跳过策略 (全)
\begin{table}[h]
    \centering
    \begin{tabular}{c | c c : c c}
        \hline
        
        \textbf{Strategy} & \multicolumn{2}{c:}{\textbf{FID} $\downarrow$} & \multicolumn{2}{c}{\textbf{LPIPS} $\downarrow$} \\
        
        \textbf{Index} & train & test & train & test \\
        
        \hline

        % skip-1: baseline
        a.0 / \textbf{b.1} & 402.8469 & 397.1920 & 0.7148 & 0.6894 \\
        a.1 / b.2 & 241.3091 & 244.8477 & \sbest{0.6170} & 0.6201 \\
        a.2 & \sbest{176.8128} & \sbest{173.6468}  & \tbest{0.6309} & 0.6274 \\
        a.3 & \best{40.4357} & \best{39.7413} & \best{0.3915} & \best{0.5266} \\
        a.4 & \tbest{215.3175} & \tbest{214.6077}  & 0.6350 & \sbest{0.5603} \\
        a.5 & 242.5459 & 240.0058  & 0.6334 & \tbest{0.5763} \\
        a.6 & 401.0944 & 404.0254  & 0.8366 & 0.8085 \\

        \hdashline

        % skip-1: ours
        b.0 & 354.4077 & 356.5143  & 0.6550 & 0.6509 \\
        % b.1 & ~ & ~ \\
        % b.2 & ~ & ~ \\
        b.3 & 259.9984 & 259.2821  & 0.6439 & 0.6293 \\

        \hline

        % skip-2: baseline
        c.0 & 453.6726 & 456.1274  & 0.8295 & 0.8302 \\
        c.1 & 401.6146 & 401.9952  & \sbest{0.6595} & \best{0.6436} \\
        c.2 & 362.4762 & 357.4724  & \best{0.6513} & \sbest{0.6623} \\

        \hdashline

        % skip-2: ours
        d.0 & 457.7766 & 456.3885  & 0.6959 & 0.6964 \\
        d.1 & 467.9547 & 464.4429  & 0.7593 & 0.7642 \\
        d.2 & 472.7829 & 466.7573  & 0.8131 & 0.8022 \\
        d.3 & 409.4545 & 412.3269  & \tbest{0.6853} & \tbest{0.6822} \\
        d.4 & 371.9738 & 387.3718  & 0.7331 & 0.7514 \\
        d.5 & 374.8360 & 383.1508  & 0.7815 & 0.7822 \\
        d.6 & \tbest{313.1157} & \tbest{309.0396}  & 0.7194 & 0.7149 \\
        \textbf{d.7} & \best{305.8840} & \best{304.8817} & 0.7048 & 0.7084 \\
        d.8 & \sbest{307.3236} & \sbest{304.9316}  & 0.7339 & 0.7067 \\

        \hline
    \end{tabular}
    \caption{
        Comparison of FID and LPIPS between vanilla, baseline skipping strategies, and our suggested strategies. 
        Multiple skipping strategies between adjacent solid or dashed lines are grouped as one set. 
    }
    \label{tab-fid_lpips_fruit_all_appx}
\end{table}

\begin{figure}[h]
    \centering
    \includegraphics[width=0.98\linewidth]{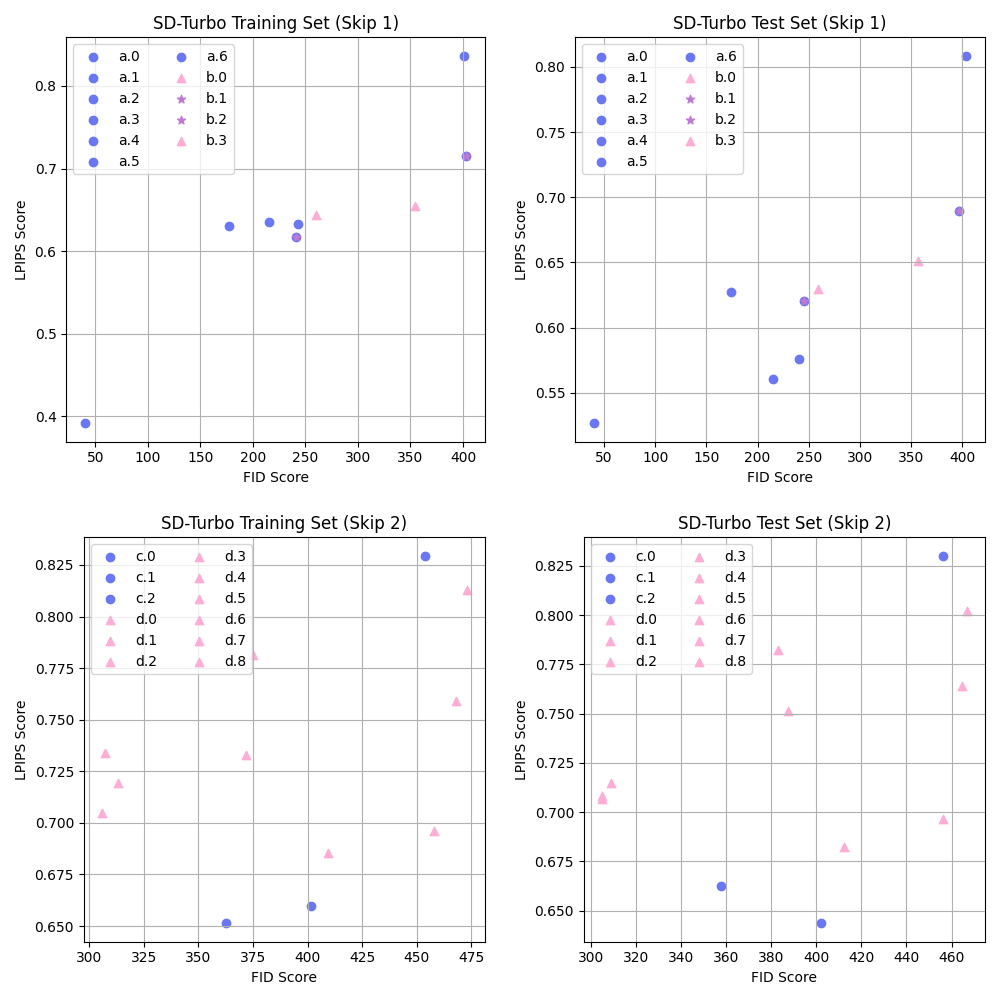}
    \caption{
        (Fig.~\ref{fig-scatter_fid_lpips_fruit} in the main paper)
        Scatter plot of FID and LPIPS under different skipping strategies (the further lower-left, the better). 
        Baseline strategies are represented by blue circles, unique points from our strategies are shown as pink triangles, while points overlapping with baseline points are marked with purple stars.
    }
    \label{fig-scatter_fid_lpips_fruit_appx}
    \vspace{-10pt}
\end{figure}

\subsection{Limitations}

While the skipping strategies generated by our approach are more likely to outperform baseline strategies, we cannot guarantee that the optimal solution(s) will be found among all possible skipping strategies.

% pruned sampling, SD-Turbo, fruit, vanilla 和 skip-1 baselines
\begin{table*}[t]
    \centering
    \begin{tabular}{c | c c c | c c c}
        \hline

        \textbf{Strategy Index} & ~ & \textbf{Training Set} & ~ & ~ & \textbf{Test Set} & ~ \\
        
        \hline

        \rule{0pt}{0pt} \\
        
        % Vanilla
        \parbox[t][-2.25cm][c]{2.0cm}{\centering Vanilla} & 
        \includegraphics[width=0.12\textwidth]{algorithm-figure-table/sample_pruned/training/23/default.png} & 
        \includegraphics[width=0.12\textwidth]{algorithm-figure-table/sample_pruned/training/52/default.png} & 
        \includegraphics[width=0.12\textwidth]{algorithm-figure-table/sample_pruned/training/74/default.png} & 
        \includegraphics[width=0.12\textwidth]{algorithm-figure-table/sample_pruned/test/22/default.png} & 
        \includegraphics[width=0.12\textwidth]{algorithm-figure-table/sample_pruned/test/73/default.png} & 
        \includegraphics[width=0.12\textwidth]{algorithm-figure-table/sample_pruned/test/83/default.png} \\

        \rule{0pt}{0pt} \\

        \hline

        \rule{0pt}{0pt} \\

        % a.0
        \parbox[t][-2.25cm][c]{2.0cm}{\centering a.0 / \textbf{b.1}} & 
        \includegraphics[width=0.12\textwidth]{algorithm-figure-table/sample_pruned/training/23/static-0.png} & 
        \includegraphics[width=0.12\textwidth]{algorithm-figure-table/sample_pruned/training/52/static-0.png} & 
        \includegraphics[width=0.12\textwidth]{algorithm-figure-table/sample_pruned/training/74/static-0.png} & 
        \includegraphics[width=0.12\textwidth]{algorithm-figure-table/sample_pruned/test/22/static-0.png} & 
        \includegraphics[width=0.12\textwidth]{algorithm-figure-table/sample_pruned/test/73/static-0.png} & 
        \includegraphics[width=0.12\textwidth]{algorithm-figure-table/sample_pruned/test/83/static-0.png} \\

        % a.1
        \parbox[t][-2.25cm][c]{2.0cm}{\centering a.1 / b.2} & 
        \includegraphics[width=0.12\textwidth]{algorithm-figure-table/sample_pruned/training/23/static-1.png} & 
        \includegraphics[width=0.12\textwidth]{algorithm-figure-table/sample_pruned/training/52/static-1.png} & 
        \includegraphics[width=0.12\textwidth]{algorithm-figure-table/sample_pruned/training/74/static-1.png} & 
        \includegraphics[width=0.12\textwidth]{algorithm-figure-table/sample_pruned/test/22/static-1.png} & 
        \includegraphics[width=0.12\textwidth]{algorithm-figure-table/sample_pruned/test/73/static-1.png} & 
        \includegraphics[width=0.12\textwidth]{algorithm-figure-table/sample_pruned/test/83/static-1.png} \\

        % a.2
        \parbox[t][-2.25cm][c]{2.0cm}{\centering a.2} & 
        \includegraphics[width=0.12\textwidth]{algorithm-figure-table/sample_pruned/training/23/static-2.png} & 
        \includegraphics[width=0.12\textwidth]{algorithm-figure-table/sample_pruned/training/52/static-2.png} & 
        \includegraphics[width=0.12\textwidth]{algorithm-figure-table/sample_pruned/training/74/static-2.png} & 
        \includegraphics[width=0.12\textwidth]{algorithm-figure-table/sample_pruned/test/22/static-2.png} & 
        \includegraphics[width=0.12\textwidth]{algorithm-figure-table/sample_pruned/test/73/static-2.png} & 
        \includegraphics[width=0.12\textwidth]{algorithm-figure-table/sample_pruned/test/83/static-2.png} \\

        % a.3
        \parbox[t][-2.25cm][c]{2.0cm}{\centering a.3} & 
        \includegraphics[width=0.12\textwidth]{algorithm-figure-table/sample_pruned/training/23/static-3.png} & 
        \includegraphics[width=0.12\textwidth]{algorithm-figure-table/sample_pruned/training/52/static-3.png} & 
        \includegraphics[width=0.12\textwidth]{algorithm-figure-table/sample_pruned/training/74/static-3.png} & 
        \includegraphics[width=0.12\textwidth]{algorithm-figure-table/sample_pruned/test/22/static-3.png} & 
        \includegraphics[width=0.12\textwidth]{algorithm-figure-table/sample_pruned/test/73/static-3.png} & 
        \includegraphics[width=0.12\textwidth]{algorithm-figure-table/sample_pruned/test/83/static-3.png} \\

        % a.4
        \parbox[t][-2.25cm][c]{2.0cm}{\centering a.4} & 
        \includegraphics[width=0.12\textwidth]{algorithm-figure-table/sample_pruned/training/23/static-4.png} & 
        \includegraphics[width=0.12\textwidth]{algorithm-figure-table/sample_pruned/training/52/static-4.png} & 
        \includegraphics[width=0.12\textwidth]{algorithm-figure-table/sample_pruned/training/74/static-4.png} & 
        \includegraphics[width=0.12\textwidth]{algorithm-figure-table/sample_pruned/test/22/static-4.png} & 
        \includegraphics[width=0.12\textwidth]{algorithm-figure-table/sample_pruned/test/73/static-4.png} & 
        \includegraphics[width=0.12\textwidth]{algorithm-figure-table/sample_pruned/test/83/static-4.png} \\

        % a.5
        \parbox[t][-2.25cm][c]{2.0cm}{\centering a.5} & 
        \includegraphics[width=0.12\textwidth]{algorithm-figure-table/sample_pruned/training/23/static-5.png} & 
        \includegraphics[width=0.12\textwidth]{algorithm-figure-table/sample_pruned/training/52/static-5.png} & 
        \includegraphics[width=0.12\textwidth]{algorithm-figure-table/sample_pruned/training/74/static-5.png} & 
        \includegraphics[width=0.12\textwidth]{algorithm-figure-table/sample_pruned/test/22/static-5.png} & 
        \includegraphics[width=0.12\textwidth]{algorithm-figure-table/sample_pruned/test/73/static-5.png} & 
        \includegraphics[width=0.12\textwidth]{algorithm-figure-table/sample_pruned/test/83/static-5.png} \\

        % a.6
        \parbox[t][-2.25cm][c]{2.0cm}{\centering a.6} & 
        \includegraphics[width=0.12\textwidth]{algorithm-figure-table/sample_pruned/training/23/static-6.png} & 
        \includegraphics[width=0.12\textwidth]{algorithm-figure-table/sample_pruned/training/52/static-6.png} & 
        \includegraphics[width=0.12\textwidth]{algorithm-figure-table/sample_pruned/training/74/static-6.png} & 
        \includegraphics[width=0.12\textwidth]{algorithm-figure-table/sample_pruned/test/22/static-6.png} & 
        \includegraphics[width=0.12\textwidth]{algorithm-figure-table/sample_pruned/test/73/static-6.png} & 
        \includegraphics[width=0.12\textwidth]{algorithm-figure-table/sample_pruned/test/83/static-6.png} \\

        \rule{0pt}{0pt} \\

        \hline
    \end{tabular}
    \captionof{figure}{
        Samples synthesized by Vanilla SD-Turbo U-Net, and U-Net with skipping strategies in group (a).
    }
    \label{fig-sample_pruned_sdturbo_fruit_skip_1_a}
\end{table*}

% pruned sampling, SD-Turbo, fruit skip-1 ours
\begin{table*}[t]
    \centering
    \begin{tabular}{c | c c c | c c c}
        \hline

        \textbf{Strategy Index} & ~ & \textbf{Training Set} & ~ & ~ & \textbf{Test Set} & ~ \\
        
        \hline

        \rule{0pt}{0pt} \\

        % b.0
        \parbox[t][-2.25cm][c]{2.0cm}{\centering b.0} & 
        \includegraphics[width=0.12\textwidth]{algorithm-figure-table/sample_pruned/training/23/skip-1_0.png} & 
        \includegraphics[width=0.12\textwidth]{algorithm-figure-table/sample_pruned/training/52/skip-1_0.png} & 
        \includegraphics[width=0.12\textwidth]{algorithm-figure-table/sample_pruned/training/74/skip-1_0.png} & 
        \includegraphics[width=0.12\textwidth]{algorithm-figure-table/sample_pruned/test/22/skip-1_0.png} & 
        \includegraphics[width=0.12\textwidth]{algorithm-figure-table/sample_pruned/test/73/skip-1_0.png} & 
        \includegraphics[width=0.12\textwidth]{algorithm-figure-table/sample_pruned/test/83/skip-1_0.png} \\

        % b.3
        \parbox[t][-2.25cm][c]{2.0cm}{\centering b.3} & 
        \includegraphics[width=0.12\textwidth]{algorithm-figure-table/sample_pruned/training/23/skip-1_3.png} & 
        \includegraphics[width=0.12\textwidth]{algorithm-figure-table/sample_pruned/training/52/skip-1_3.png} & 
        \includegraphics[width=0.12\textwidth]{algorithm-figure-table/sample_pruned/training/74/skip-1_3.png} & 
        \includegraphics[width=0.12\textwidth]{algorithm-figure-table/sample_pruned/test/22/skip-1_3.png} & 
        \includegraphics[width=0.12\textwidth]{algorithm-figure-table/sample_pruned/test/73/skip-1_3.png} & 
        \includegraphics[width=0.12\textwidth]{algorithm-figure-table/sample_pruned/test/83/skip-1_3.png} \\

        \rule{0pt}{0pt} \\

        \hline
    \end{tabular}
    \captionof{figure}{
        Samples synthesized by U-Net with skipping strategies in group (b).
    }
    \label{fig-sample_pruned_sdturbo_fruit_skip_1_b}
\end{table*}

% pruned sampling, SD-Turbo, fruit skip-2 baselines
\begin{table*}[t]
    \centering
    \begin{tabular}{c | c c c | c c c}
        \hline

        \textbf{Strategy Index} & ~ & \textbf{Training Set} & ~ & ~ & \textbf{Test Set} & ~ \\
        
        \hline

        \rule{0pt}{0pt} \\

        % c.0
        \parbox[t][-2.25cm][c]{2.0cm}{\centering c.0} & 
        \includegraphics[width=0.12\textwidth]{algorithm-figure-table/sample_pruned/training/23/static-0,6.png} & 
        \includegraphics[width=0.12\textwidth]{algorithm-figure-table/sample_pruned/training/52/static-0,6.png} & 
        \includegraphics[width=0.12\textwidth]{algorithm-figure-table/sample_pruned/training/74/static-0,6.png} & 
        \includegraphics[width=0.12\textwidth]{algorithm-figure-table/sample_pruned/test/22/static-0,6.png} & 
        \includegraphics[width=0.12\textwidth]{algorithm-figure-table/sample_pruned/test/73/static-0,6.png} & 
        \includegraphics[width=0.12\textwidth]{algorithm-figure-table/sample_pruned/test/83/static-0,6.png} \\

        % c.1
        \parbox[t][-2.25cm][c]{2.0cm}{\centering c.1} & 
        \includegraphics[width=0.12\textwidth]{algorithm-figure-table/sample_pruned/training/23/static-1,5.png} & 
        \includegraphics[width=0.12\textwidth]{algorithm-figure-table/sample_pruned/training/52/static-1,5.png} & 
        \includegraphics[width=0.12\textwidth]{algorithm-figure-table/sample_pruned/training/74/static-1,5.png} & 
        \includegraphics[width=0.12\textwidth]{algorithm-figure-table/sample_pruned/test/22/static-1,5.png} & 
        \includegraphics[width=0.12\textwidth]{algorithm-figure-table/sample_pruned/test/73/static-1,5.png} & 
        \includegraphics[width=0.12\textwidth]{algorithm-figure-table/sample_pruned/test/83/static-1,5.png} \\

        % c.2
        \parbox[t][-2.25cm][c]{2.0cm}{\centering c.2} & 
        \includegraphics[width=0.12\textwidth]{algorithm-figure-table/sample_pruned/training/23/static-2,4.png} & 
        \includegraphics[width=0.12\textwidth]{algorithm-figure-table/sample_pruned/training/52/static-2,4.png} & 
        \includegraphics[width=0.12\textwidth]{algorithm-figure-table/sample_pruned/training/74/static-2,4.png} & 
        \includegraphics[width=0.12\textwidth]{algorithm-figure-table/sample_pruned/test/22/static-2,4.png} & 
        \includegraphics[width=0.12\textwidth]{algorithm-figure-table/sample_pruned/test/73/static-2,4.png} & 
        \includegraphics[width=0.12\textwidth]{algorithm-figure-table/sample_pruned/test/83/static-2,4.png} \\

        \rule{0pt}{0pt} \\

        \hline
    \end{tabular}
    \captionof{figure}{
        Samples synthesized by U-Net with skipping strategies in group (c).
    }
    \label{fig-sample_pruned_sdturbo_fruit_skip_2_c}
\end{table*}

% pruned sampling, SD-Turbo, fruit skip-2 ours
\begin{table*}[t]
    \centering
    \begin{tabular}{c | c c c | c c c}
        \hline

        \textbf{Strategy Index} & ~ & \textbf{Training Set} & ~ & ~ & \textbf{Test Set} & ~ \\
        
        \hline

        \rule{0pt}{0pt} \\

        % d.0
        \parbox[t][-2.25cm][c]{2.0cm}{\centering d.0} & 
        \includegraphics[width=0.12\textwidth]{algorithm-figure-table/sample_pruned/training/23/skip-2_0.png} & 
        \includegraphics[width=0.12\textwidth]{algorithm-figure-table/sample_pruned/training/52/skip-2_0.png} & 
        \includegraphics[width=0.12\textwidth]{algorithm-figure-table/sample_pruned/training/74/skip-2_0.png} & 
        \includegraphics[width=0.12\textwidth]{algorithm-figure-table/sample_pruned/test/22/skip-2_0.png} & 
        \includegraphics[width=0.12\textwidth]{algorithm-figure-table/sample_pruned/test/73/skip-2_0.png} & 
        \includegraphics[width=0.12\textwidth]{algorithm-figure-table/sample_pruned/test/83/skip-2_0.png} \\

        % d.1
        \parbox[t][-2.25cm][c]{2.0cm}{\centering d.1} & 
        \includegraphics[width=0.12\textwidth]{algorithm-figure-table/sample_pruned/training/23/skip-2_1.png} & 
        \includegraphics[width=0.12\textwidth]{algorithm-figure-table/sample_pruned/training/52/skip-2_1.png} & 
        \includegraphics[width=0.12\textwidth]{algorithm-figure-table/sample_pruned/training/74/skip-2_1.png} & 
        \includegraphics[width=0.12\textwidth]{algorithm-figure-table/sample_pruned/test/22/skip-2_1.png} & 
        \includegraphics[width=0.12\textwidth]{algorithm-figure-table/sample_pruned/test/73/skip-2_1.png} & 
        \includegraphics[width=0.12\textwidth]{algorithm-figure-table/sample_pruned/test/83/skip-2_1.png} \\

        % d.2
        \parbox[t][-2.25cm][c]{2.0cm}{\centering d.2} & 
        \includegraphics[width=0.12\textwidth]{algorithm-figure-table/sample_pruned/training/23/skip-2_2.png} & 
        \includegraphics[width=0.12\textwidth]{algorithm-figure-table/sample_pruned/training/52/skip-2_2.png} & 
        \includegraphics[width=0.12\textwidth]{algorithm-figure-table/sample_pruned/training/74/skip-2_2.png} & 
        \includegraphics[width=0.12\textwidth]{algorithm-figure-table/sample_pruned/test/22/skip-2_2.png} & 
        \includegraphics[width=0.12\textwidth]{algorithm-figure-table/sample_pruned/test/73/skip-2_2.png} & 
        \includegraphics[width=0.12\textwidth]{algorithm-figure-table/sample_pruned/test/83/skip-2_2.png} \\

        % d.3
        \parbox[t][-2.25cm][c]{2.0cm}{\centering d.3} & 
        \includegraphics[width=0.12\textwidth]{algorithm-figure-table/sample_pruned/training/23/skip-2_3.png} & 
        \includegraphics[width=0.12\textwidth]{algorithm-figure-table/sample_pruned/training/52/skip-2_3.png} & 
        \includegraphics[width=0.12\textwidth]{algorithm-figure-table/sample_pruned/training/74/skip-2_3.png} & 
        \includegraphics[width=0.12\textwidth]{algorithm-figure-table/sample_pruned/test/22/skip-2_3.png} & 
        \includegraphics[width=0.12\textwidth]{algorithm-figure-table/sample_pruned/test/73/skip-2_3.png} & 
        \includegraphics[width=0.12\textwidth]{algorithm-figure-table/sample_pruned/test/83/skip-2_3.png} \\

        % d.4
        \parbox[t][-2.25cm][c]{2.0cm}{\centering d.4} & 
        \includegraphics[width=0.12\textwidth]{algorithm-figure-table/sample_pruned/training/23/skip-2_4.png} & 
        \includegraphics[width=0.12\textwidth]{algorithm-figure-table/sample_pruned/training/52/skip-2_4.png} & 
        \includegraphics[width=0.12\textwidth]{algorithm-figure-table/sample_pruned/training/74/skip-2_4.png} & 
        \includegraphics[width=0.12\textwidth]{algorithm-figure-table/sample_pruned/test/22/skip-2_4.png} & 
        \includegraphics[width=0.12\textwidth]{algorithm-figure-table/sample_pruned/test/73/skip-2_4.png} & 
        \includegraphics[width=0.12\textwidth]{algorithm-figure-table/sample_pruned/test/83/skip-2_4.png} \\

        % d.5
        \parbox[t][-2.25cm][c]{2.0cm}{\centering d.5} & 
        \includegraphics[width=0.12\textwidth]{algorithm-figure-table/sample_pruned/training/23/skip-2_5.png} & 
        \includegraphics[width=0.12\textwidth]{algorithm-figure-table/sample_pruned/training/52/skip-2_5.png} & 
        \includegraphics[width=0.12\textwidth]{algorithm-figure-table/sample_pruned/training/74/skip-2_5.png} & 
        \includegraphics[width=0.12\textwidth]{algorithm-figure-table/sample_pruned/test/22/skip-2_5.png} & 
        \includegraphics[width=0.12\textwidth]{algorithm-figure-table/sample_pruned/test/73/skip-2_5.png} & 
        \includegraphics[width=0.12\textwidth]{algorithm-figure-table/sample_pruned/test/83/skip-2_5.png} \\

        % d.6
        \parbox[t][-2.25cm][c]{2.0cm}{\centering d.6} & 
        \includegraphics[width=0.12\textwidth]{algorithm-figure-table/sample_pruned/training/23/skip-2_6.png} & 
        \includegraphics[width=0.12\textwidth]{algorithm-figure-table/sample_pruned/training/52/skip-2_6.png} & 
        \includegraphics[width=0.12\textwidth]{algorithm-figure-table/sample_pruned/training/74/skip-2_6.png} & 
        \includegraphics[width=0.12\textwidth]{algorithm-figure-table/sample_pruned/test/22/skip-2_6.png} & 
        \includegraphics[width=0.12\textwidth]{algorithm-figure-table/sample_pruned/test/73/skip-2_6.png} & 
        \includegraphics[width=0.12\textwidth]{algorithm-figure-table/sample_pruned/test/83/skip-2_6.png} \\

        % d.7
        \parbox[t][-2.25cm][c]{2.0cm}{\centering \textbf{d.7}} & 
        \includegraphics[width=0.12\textwidth]{algorithm-figure-table/sample_pruned/training/23/skip-2_7.png} & 
        \includegraphics[width=0.12\textwidth]{algorithm-figure-table/sample_pruned/training/52/skip-2_7.png} & 
        \includegraphics[width=0.12\textwidth]{algorithm-figure-table/sample_pruned/training/74/skip-2_7.png} & 
        \includegraphics[width=0.12\textwidth]{algorithm-figure-table/sample_pruned/test/22/skip-2_7.png} & 
        \includegraphics[width=0.12\textwidth]{algorithm-figure-table/sample_pruned/test/73/skip-2_7.png} & 
        \includegraphics[width=0.12\textwidth]{algorithm-figure-table/sample_pruned/test/83/skip-2_7.png} \\

        % d.8
        \parbox[t][-2.25cm][c]{2.0cm}{\centering d.8} & 
        \includegraphics[width=0.12\textwidth]{algorithm-figure-table/sample_pruned/training/23/skip-2_8.png} & 
        \includegraphics[width=0.12\textwidth]{algorithm-figure-table/sample_pruned/training/52/skip-2_8.png} & 
        \includegraphics[width=0.12\textwidth]{algorithm-figure-table/sample_pruned/training/74/skip-2_8.png} & 
        \includegraphics[width=0.12\textwidth]{algorithm-figure-table/sample_pruned/test/22/skip-2_8.png} & 
        \includegraphics[width=0.12\textwidth]{algorithm-figure-table/sample_pruned/test/73/skip-2_8.png} & 
        \includegraphics[width=0.12\textwidth]{algorithm-figure-table/sample_pruned/test/83/skip-2_8.png} \\

        \rule{0pt}{0pt} \\

        \hline
    \end{tabular}
    \captionof{figure}{
        Samples synthesized by U-Net with skipping strategies in group (d).
    }
    \label{fig-sample_pruned_sdturbo_fruit_skip_2_d}
\end{table*}

% Enhanced Image Synthesis Details
\section{Supplementary to Enhanced Image Synthesis}
\label{appx_sec-empirical_analysis_of_synthesis_improvements}

\subsection{Static Re-weighting Schedule Details}

\paragraph{Experimental Settings}

The results in Tab.~\ref{tab-comparison_between_different_models_and_steps_appx} are evaluated with 20 samples for each model under the following settings: 

\begin{itemize}
    \item \textbf{SD-Turbo}: 2-step inference with prompt ``\emph{A small baby bird on a piece of metal.}" from the \emph{photo} category in Human Preference Dataset v2~\cite{wu2023humanpreferencescorev2}. 

    \item \textbf{SDXL-Turbo}: 2-step inference with prompt ``\emph{A landscape with a building in the style of Simon Stalenhag.}" from the \emph{concept-art} category. 
    
    \item \textbf{SD v2.1}: 20-step inference with prompt ``\emph{A portrait of Fox McCloud firing a blaster in anthropomorphic furry art style from the Star Fox series, illustrated by Jim Burns.}" from the \emph{anime} category. 

    \item \textbf{SDXL}: 20-step inference with prompt ``\emph{An English woman plays the lute with a slender neck and long dark hair in a painting by WilliamAdolphe Bouguereau.}" from the \emph{paintings} category. 
\end{itemize}

\paragraph{Qualitative Results}

Samples of difference models with different inference steps, using the vanilla re-weighting schedule and our best re-weighting schedule (in Tab.~\ref{tab-comparison_between_different_models_and_steps_appx}) are shown in Fig.~\ref{fig-static_reweighting_sdturbo_sdxlturbo_appx} and Fig.~\ref{fig-static_reweighting_sd_sdxl_appx}, respectively. 

Under the same number of inference steps, the samples generated under our re-weighting schedule exhibit greater clarity and more vibrant colors, indicating our method's capability to enhance sampling aesthetics. 
Across different numbers of inference steps, the aesthetic quality of samples under our re-weighting schedule with fewer steps even surpasses that of samples under the vanilla re-weighting schedule with more steps. 
This suggests that, our method improves the SNR during sampling, thereby enhancing inference efficiency.

% SD-Turbo / SDXL-Turbo, static re-weighting 的采样图
\begin{table*}[h]
    \centering
    \begin{tabular}{c | c c c | c c c}
        \hline

        \textbf{Re-Weighting} & \multicolumn{3}{c|}{\textbf{SD-Turbo}} & \multicolumn{3}{c}{\textbf{SDXL-Turbo}} \\
        \textbf{Strategy} & 1-step & 2-step & 3-step & 1-step & 2-step & 3-step \\
        
        \hline

        \rule{0pt}{0pt} \\
        
        % default
        \parbox[t][-2.25cm][c]{2.0cm}{\centering Vanilla} & 
        \includegraphics[width=0.12\textwidth]{algorithm-figure-table/static_reweighting/sd-turbo/1_step/default.png} & 
        \includegraphics[width=0.12\textwidth]{algorithm-figure-table/static_reweighting/sd-turbo/2_step/default.png} & 
        \includegraphics[width=0.12\textwidth]{algorithm-figure-table/static_reweighting/sd-turbo/3_step/default.png} & 
        \includegraphics[width=0.12\textwidth]{algorithm-figure-table/static_reweighting/sdxl-turbo/1_step/default.png} & 
        \includegraphics[width=0.12\textwidth]{algorithm-figure-table/static_reweighting/sdxl-turbo/2_step/default.png} & 
        \includegraphics[width=0.12\textwidth]{algorithm-figure-table/static_reweighting/sdxl-turbo/3_step/default.png} \\
        
        % ours
        \parbox[t][-2.25cm][c]{2.0cm}{\centering Vanilla} & 
        \includegraphics[width=0.12\textwidth]{algorithm-figure-table/static_reweighting/sd-turbo/1_step/ours.png} & 
        \includegraphics[width=0.12\textwidth]{algorithm-figure-table/static_reweighting/sd-turbo/2_step/ours.png} & 
        \includegraphics[width=0.12\textwidth]{algorithm-figure-table/static_reweighting/sd-turbo/3_step/ours.png} & 
        \includegraphics[width=0.12\textwidth]{algorithm-figure-table/static_reweighting/sdxl-turbo/1_step/ours.png} & 
        \includegraphics[width=0.12\textwidth]{algorithm-figure-table/static_reweighting/sdxl-turbo/2_step/ours.png} & 
        \includegraphics[width=0.12\textwidth]{algorithm-figure-table/static_reweighting/sdxl-turbo/3_step/ours.png}
        \rule{0pt}{0pt} \\

        \rule{0pt}{0pt} \\

        \hline
    \end{tabular}
    \captionof{figure}{
        Samples of SD-Turbo and SDXL-Turbo with different inference steps, using the vanilla re-weighting schedule and our best re-weighting schedule, respectively. 
    }
    \label{fig-static_reweighting_sdturbo_sdxlturbo_appx}
\end{table*}

% SD / SDXL static re-weighting 的采样图
\begin{table*}[h]
    \centering
    \begin{tabular}{c | c c c | c c c}
        \hline

        \textbf{Re-Weighting} & \multicolumn{3}{c|}{\textbf{SD v2.1}} & \multicolumn{3}{c}{\textbf{SDXL}} \\
        \textbf{Strategy} & 10-step & 15-step & 20-step & 10-step & 15-step & 20-step \\
        
        \hline

        \rule{0pt}{0pt} \\
        
        % default
        \parbox[t][-2.25cm][c]{2.0cm}{\centering Vanilla} & 
        \includegraphics[width=0.12\textwidth]{algorithm-figure-table/static_reweighting/sd/10_step/default.png} & 
        \includegraphics[width=0.12\textwidth]{algorithm-figure-table/static_reweighting/sd/15_step/default.png} & 
        \includegraphics[width=0.12\textwidth]{algorithm-figure-table/static_reweighting/sd/20_step/default.png} & 
        \includegraphics[width=0.12\textwidth]{algorithm-figure-table/static_reweighting/sdxl/10_step/default.png} & 
        \includegraphics[width=0.12\textwidth]{algorithm-figure-table/static_reweighting/sdxl/15_step/default.png} & 
        \includegraphics[width=0.12\textwidth]{algorithm-figure-table/static_reweighting/sdxl/20_step/default.png} \\
        
        % ours
        \parbox[t][-2.25cm][c]{2.0cm}{\centering Vanilla} & 
        \includegraphics[width=0.12\textwidth]{algorithm-figure-table/static_reweighting/sd/10_step/ours.png} & 
        \includegraphics[width=0.12\textwidth]{algorithm-figure-table/static_reweighting/sd/15_step/ours.png} & 
        \includegraphics[width=0.12\textwidth]{algorithm-figure-table/static_reweighting/sd/20_step/ours.png} & 
        \includegraphics[width=0.12\textwidth]{algorithm-figure-table/static_reweighting/sdxl/10_step/ours.png} & 
        \includegraphics[width=0.12\textwidth]{algorithm-figure-table/static_reweighting/sdxl/15_step/ours.png} & 
        \includegraphics[width=0.12\textwidth]{algorithm-figure-table/static_reweighting/sdxl/20_step/ours.png} \\
        
        \rule{0pt}{0pt} \\

        \hline
    \end{tabular}
    \captionof{figure}{
        Samples of SD and SDXL with different inference steps, using the vanilla re-weighting schedule and our best re-weighting schedule, respectively. 
    }
    \label{fig-static_reweighting_sd_sdxl_appx}
\end{table*}

% importance-based re-weighting, SDXL-Turbo, 2
\begin{table*}[t]
    \centering
    \begin{tabular}{c | c c c c}
        \hline

        \multirow{2}{*}{\textbf{Models}} & \multicolumn{4}{c}{\textbf{Re-weighting Schedule}} \\
        ~ & Vanilla & $[0.98, 1.1]$ / $[0.95, 1.1]$ & $[0.98, 1.15]$ / $[0.95, 1.15]$ & $[0.98, 1.2]$ / $[0.95, 1.2]$ \\
        
        \hline

        \rule{0pt}{0pt} \\
        
        % SD-Turbo
        \parbox[t][-2.75cm][c]{2.0cm}{\centering SD-Turbo} & 
        \includegraphics[width=0.15\textwidth]{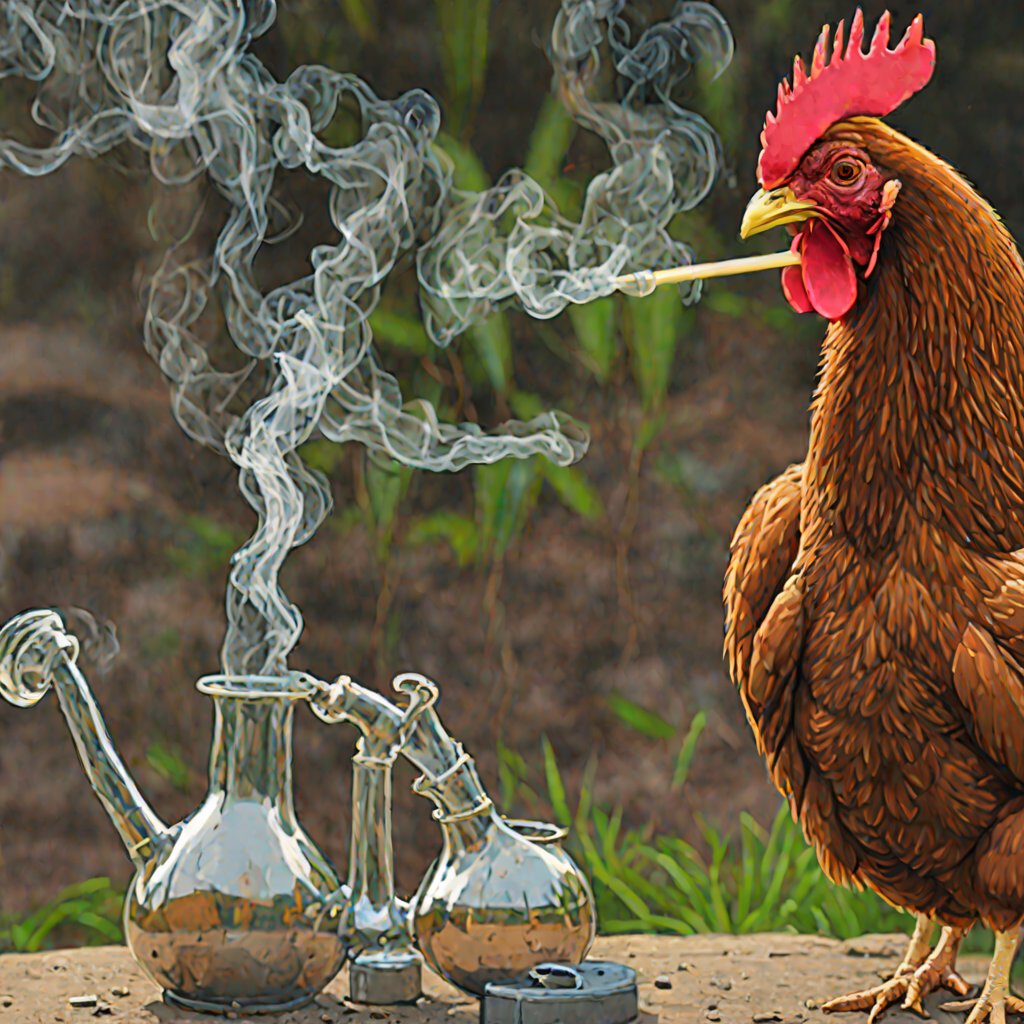} & \includegraphics[width=0.15\textwidth]{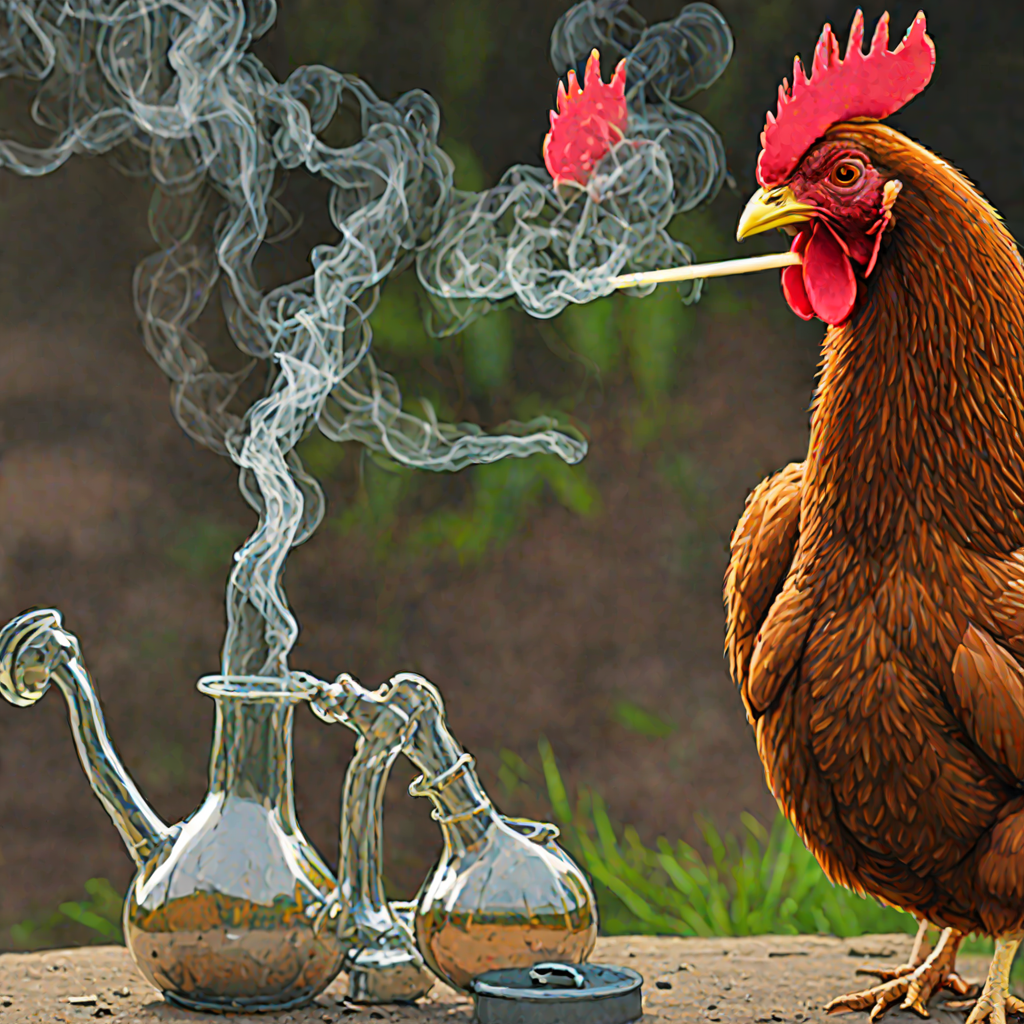} & 
        \includegraphics[width=0.15\textwidth]{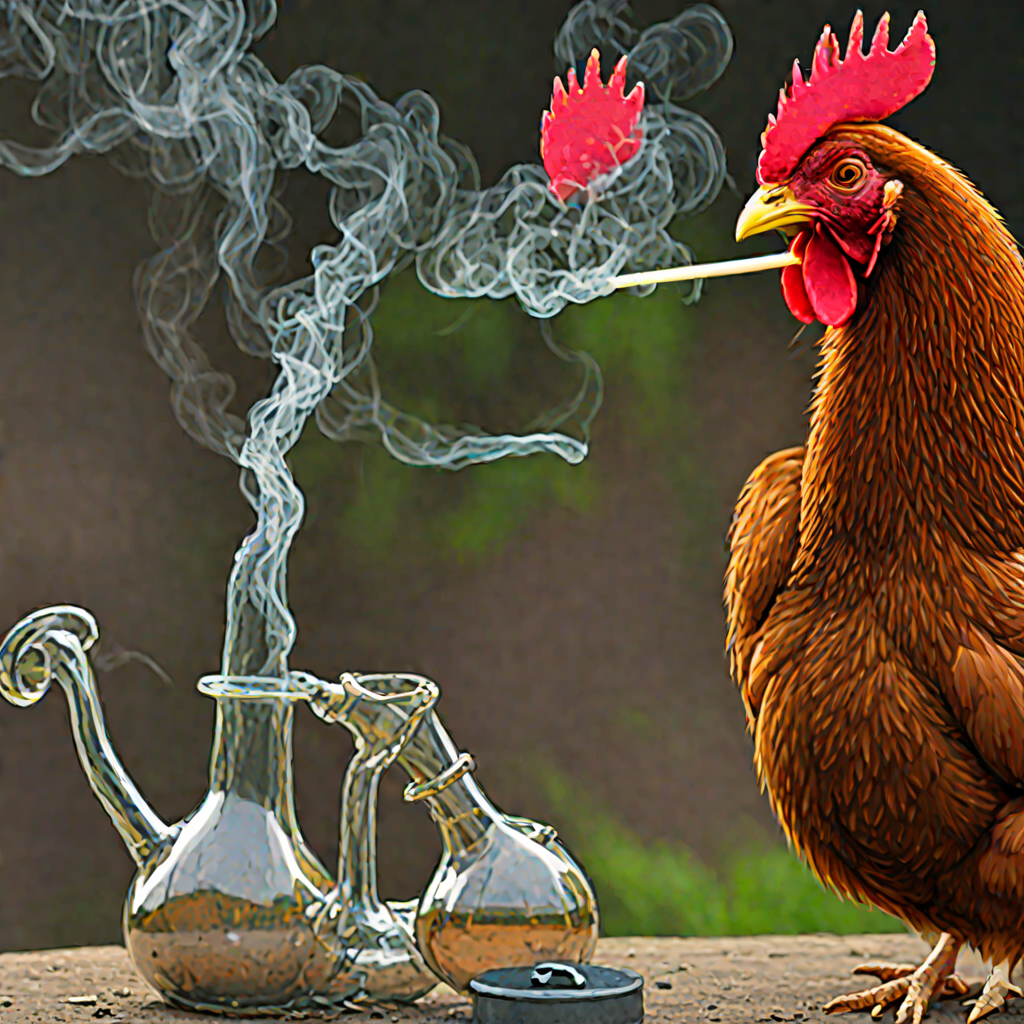} & 
        \includegraphics[width=0.15\textwidth]{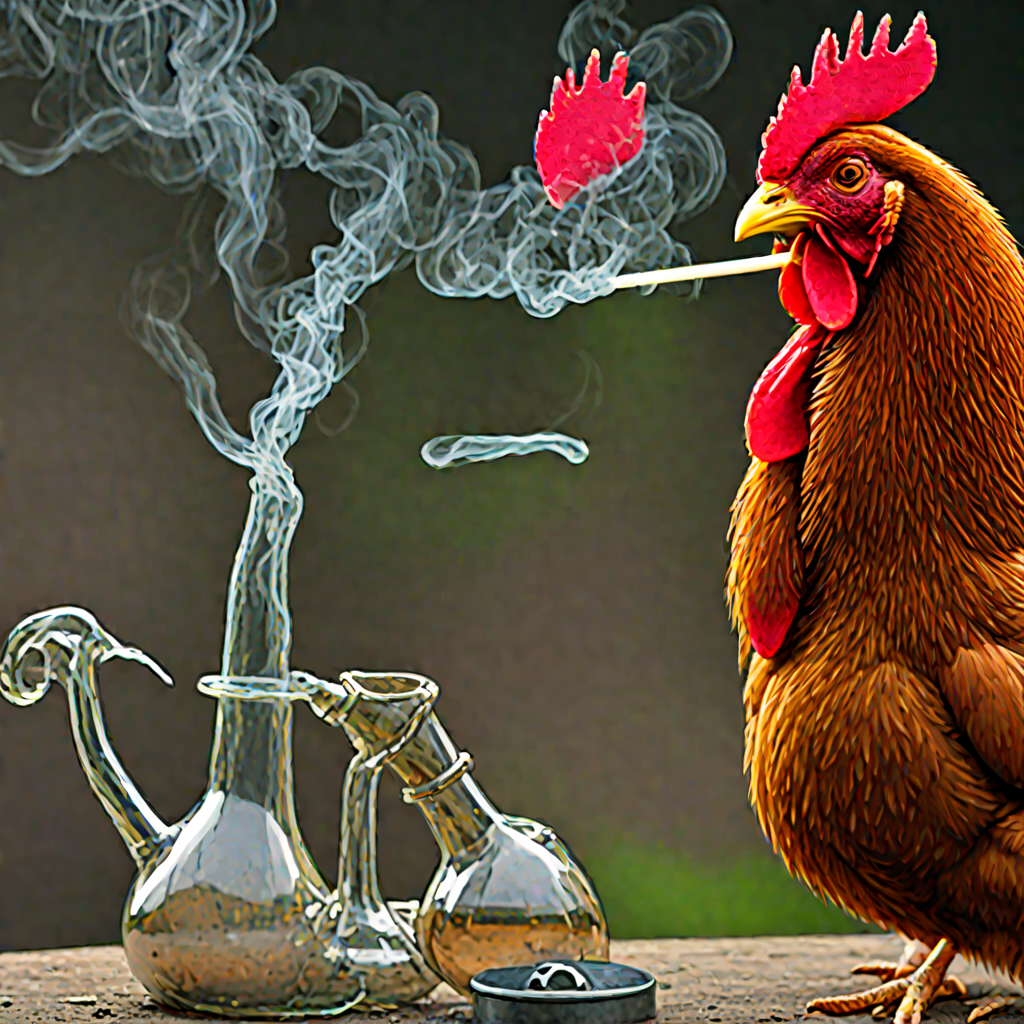} \\

        % SDXL-Turbo
        \parbox[t][-2.75cm][c]{2.0cm}{\centering SDXL-Turbo} & 
        \includegraphics[width=0.15\textwidth]{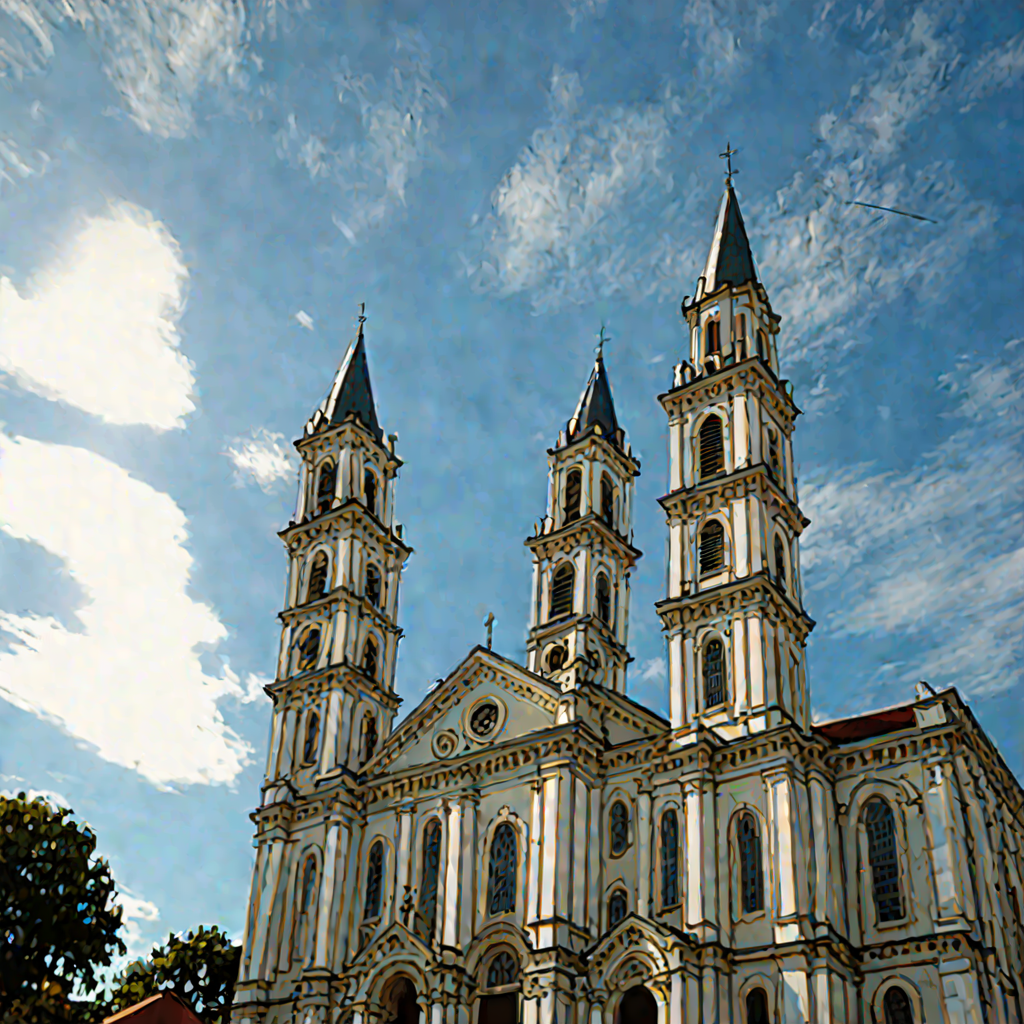} & \includegraphics[width=0.15\textwidth]{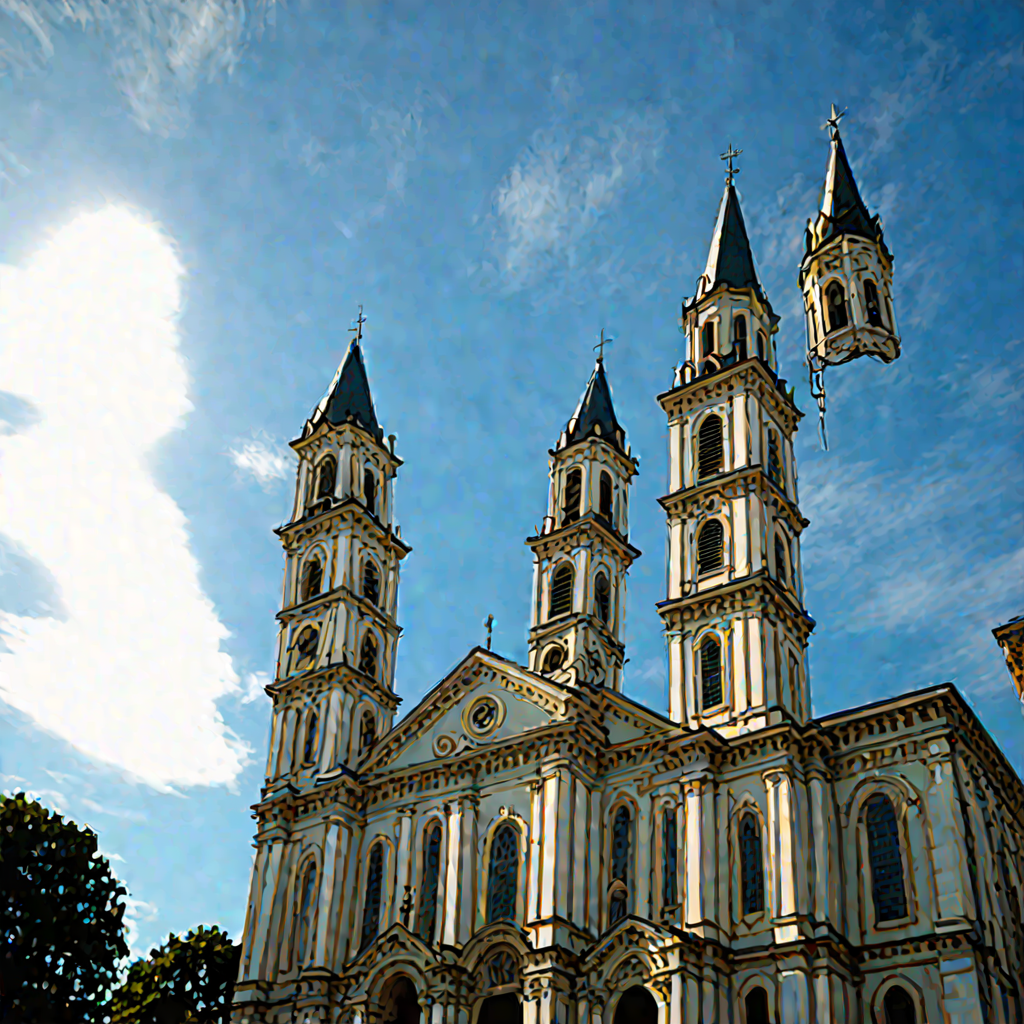} & 
        \includegraphics[width=0.15\textwidth]{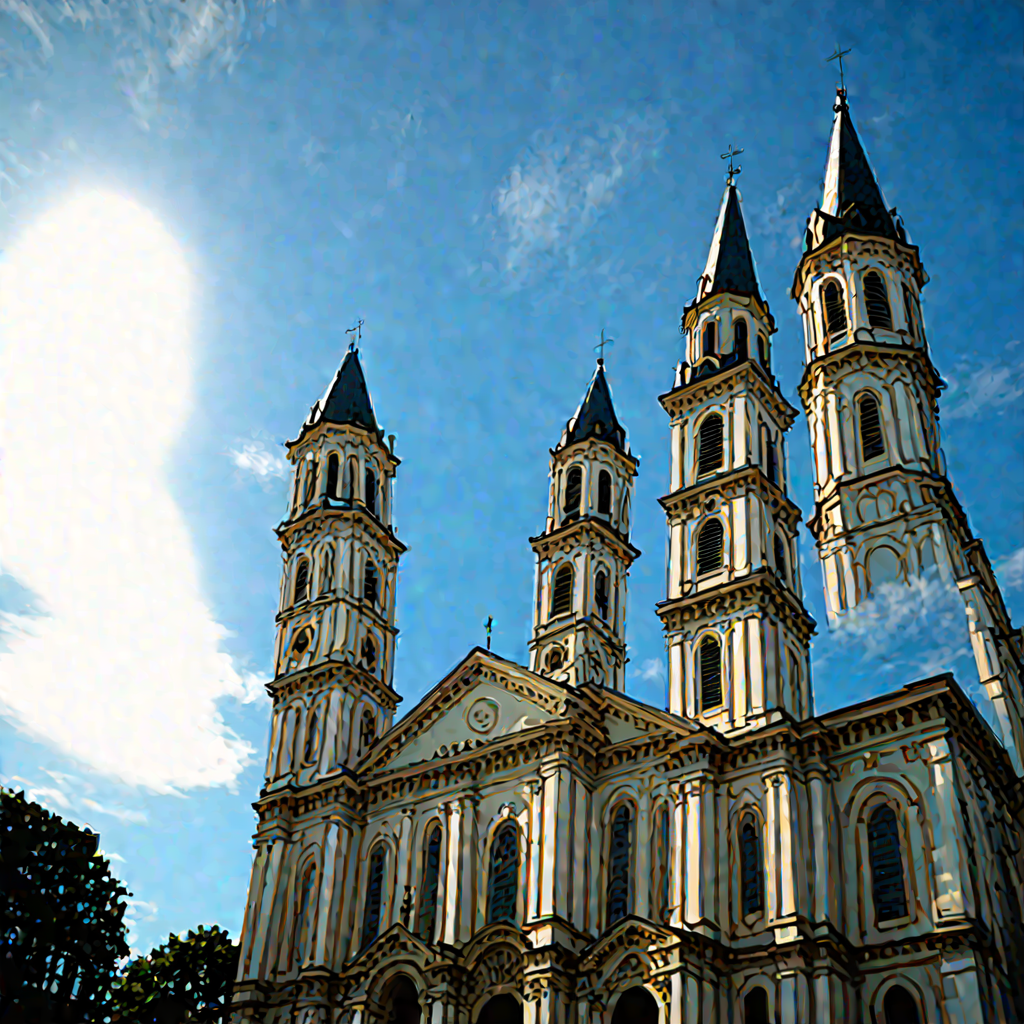} & 
        \includegraphics[width=0.15\textwidth]{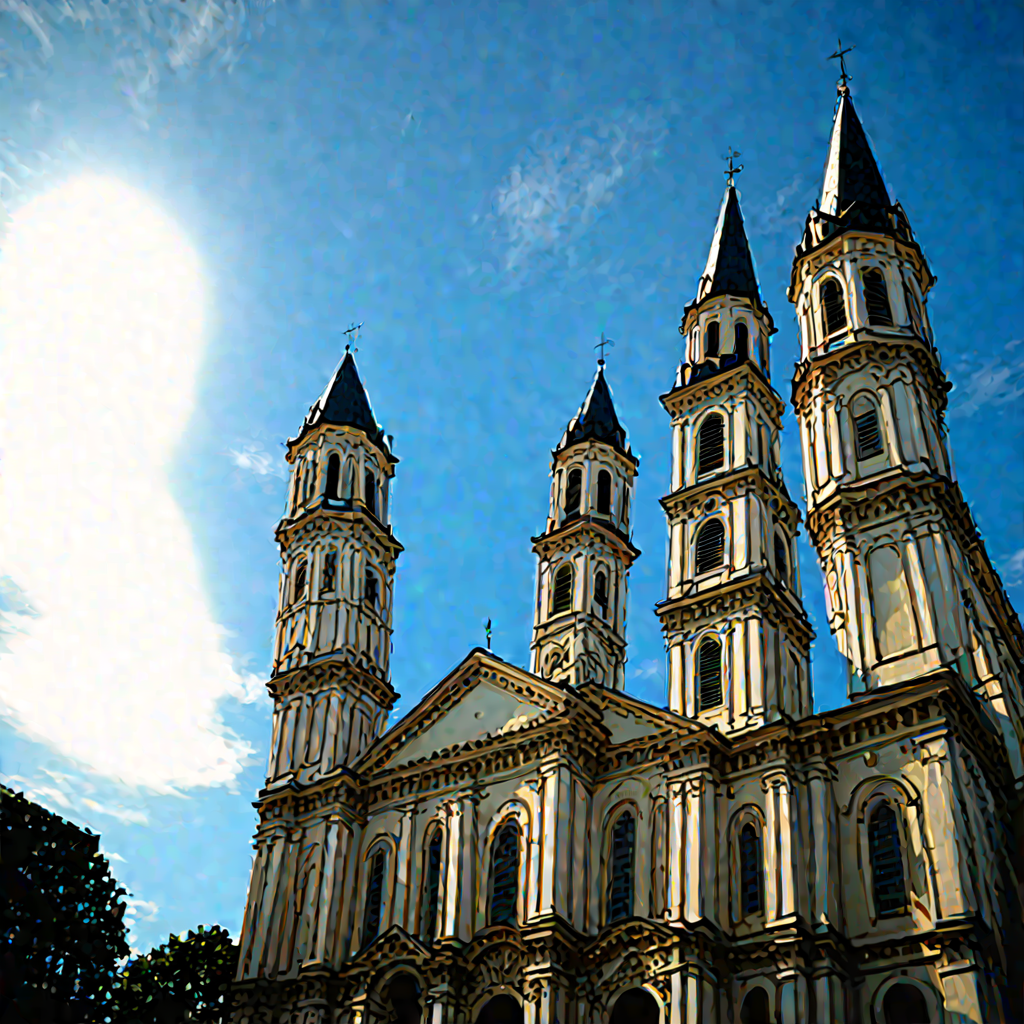} \\

        \rule{0pt}{0pt} \\

        \hline
    \end{tabular}
    \captionof{figure}{
        Failure cases of SD-Turbo and SDXL-Turbo under the optimal re-weighting schedules. 
    }
    \label{fig-failure_case}
\end{table*}

\subsection{Importance-based Re-weighting Schedule Details}

\paragraph{Qualitative Results}

The qualitative results shown in Fig.~\ref{fig-importance_based_reweighting_sdturbo_appx_1} and Fig.~\ref{fig-importance_based_reweighting_sdturbo_appx_2} are generated using 2-step-inference SD-Turbo under the following settings: 

\begin{itemize}
    \item \textbf{anime}: with prompt ``\emph{Walter White dressed as a medievalstyle king.}". 

    \item \textbf{concept-art}: with prompt ``\emph{Portrait of Guts from Berserk submerged in red water.}". 
    
    \item \textbf{paintings}: with prompt ``\emph{Male playing piano with audience surrounded by paintings by Gaston Bussiere, Craig Mullins, and J.C. Leyendecker.}". 

    \item \textbf{photo}: with prompt ``\emph{An old classic church is in front a big blue sky.}". 
\end{itemize}

It can be observed that our re-weighting schedule enhances the aesthetic quality of the samples (anime and photo), improves clarity (concept-art), and reduces background anomalies (paintings). 

The qualitative results shown in Fig.~\ref{fig-importance_based_reweighting_sdxlturbo_appx_1} and Fig.~\ref{fig-importance_based_reweighting_sdxlturbo_appx_2} are generated using 2-step-inference SDXL-Turbo under the following settings: 

\begin{itemize}
    \item \textbf{anime}: with prompt ``\emph{A cute anthropomorphic bear knight wearing a cape and crown in pale blue armor.}". 

    \item \textbf{concept-art}: with prompt ``\emph{A digital concept art of a machinist in uniform with a scifi repair tool and glowing lights.}". 
    
    \item \textbf{paintings}: with prompt ``\emph{A group of fairies playing cards on a table in a moonlit forest next to a pond filled with water lilies, artwork by Ida Rentoul Outhwaite.}". 

    \item \textbf{photo}: with prompt ``\emph{Two cats chill in the bathtub one is laying down. }". 
\end{itemize}

It can also be observed that our re-weighting schedule enhances the aesthetic quality of the samples (anime and concept-art), improves prompt alignment (paintings), and reduces anomalies in the main subjects (photo). 

% importance-based re-weighting, SD-Turbo, 1
\begin{table*}[t]
    \centering
    \begin{tabular}{c | c c c c}
        \hline

        \textbf{Re-Weighting} & \multicolumn{4}{c}{\textbf{SD-Turbo}} \\
        \textbf{Strategy} & anime & concept-art & paintings & photo \\
        
        \hline

        \rule{0pt}{0pt} \\
        
        % Vanilla
        \parbox[t][-2.75cm][c]{2.0cm}{\centering Vanilla} & 
        \includegraphics[width=0.15\textwidth]{algorithm-figure-table/importance_based_reweighting/sd-turbo/anime/default.png} & 
        \includegraphics[width=0.15\textwidth]{algorithm-figure-table/importance_based_reweighting/sd-turbo/concept-art/default.png} & 
        \includegraphics[width=0.15\textwidth]{algorithm-figure-table/importance_based_reweighting/sd-turbo/paintings/default.png} & 
        \includegraphics[width=0.15\textwidth]{algorithm-figure-table/importance_based_reweighting/sd-turbo/photo/default.png} \\

        \rule{0pt}{0pt} \\

        \hdashline

        \rule{0pt}{0pt} \\
            
        % [0.95, 1.1]
        \parbox[t][-2.75cm][c]{2.0cm}{\centering $[0.95, 1.1]$} & 
        \includegraphics[width=0.15\textwidth]{algorithm-figure-table/importance_based_reweighting/sd-turbo/anime/0.95_1.1.png} & 
        \includegraphics[width=0.15\textwidth]{algorithm-figure-table/importance_based_reweighting/sd-turbo/concept-art/0.95_1.1.png} & 
        \includegraphics[width=0.15\textwidth]{algorithm-figure-table/importance_based_reweighting/sd-turbo/paintings/0.95_1.1.png} & 
        \includegraphics[width=0.15\textwidth]{algorithm-figure-table/importance_based_reweighting/sd-turbo/photo/0.95_1.1.png} \\

        % [0.96, 1.1]
        \parbox[t][-2.75cm][c]{2.0cm}{\centering $[0.96, 1.1]$} & 
        \includegraphics[width=0.15\textwidth]{algorithm-figure-table/importance_based_reweighting/sd-turbo/anime/0.96_1.1.png} & 
        \includegraphics[width=0.15\textwidth]{algorithm-figure-table/importance_based_reweighting/sd-turbo/concept-art/0.96_1.1.png} & 
        \includegraphics[width=0.15\textwidth]{algorithm-figure-table/importance_based_reweighting/sd-turbo/paintings/0.96_1.1.png} & 
        \includegraphics[width=0.15\textwidth]{algorithm-figure-table/importance_based_reweighting/sd-turbo/photo/0.96_1.1.png} \\

        % [0.97, 1.1]
        \parbox[t][-2.75cm][c]{2.0cm}{\centering $[0.97, 1.1]$} & 
        \includegraphics[width=0.15\textwidth]{algorithm-figure-table/importance_based_reweighting/sd-turbo/anime/0.97_1.1.png} & 
        \includegraphics[width=0.15\textwidth]{algorithm-figure-table/importance_based_reweighting/sd-turbo/concept-art/0.97_1.1.png} & 
        \includegraphics[width=0.15\textwidth]{algorithm-figure-table/importance_based_reweighting/sd-turbo/paintings/0.97_1.1.png} & 
        \includegraphics[width=0.15\textwidth]{algorithm-figure-table/importance_based_reweighting/sd-turbo/photo/0.97_1.1.png} \\

        % [0.98, 1.1]
        \parbox[t][-2.75cm][c]{2.0cm}{\centering $[0.98, 1.1]$} & 
        \includegraphics[width=0.15\textwidth]{algorithm-figure-table/importance_based_reweighting/sd-turbo/anime/0.98_1.1.png} & 
        \includegraphics[width=0.15\textwidth]{algorithm-figure-table/importance_based_reweighting/sd-turbo/concept-art/0.98_1.1.png} & 
        \includegraphics[width=0.15\textwidth]{algorithm-figure-table/importance_based_reweighting/sd-turbo/paintings/0.98_1.1.png} & 
        \includegraphics[width=0.15\textwidth]{algorithm-figure-table/importance_based_reweighting/sd-turbo/photo/0.98_1.1.png} \\

        % [0.99, 1.1]
        \parbox[t][-2.75cm][c]{2.0cm}{\centering $[0.99, 1.1]$} & 
        \includegraphics[width=0.15\textwidth]{algorithm-figure-table/importance_based_reweighting/sd-turbo/anime/0.99_1.1.png} & 
        \includegraphics[width=0.15\textwidth]{algorithm-figure-table/importance_based_reweighting/sd-turbo/concept-art/0.99_1.1.png} & 
        \includegraphics[width=0.15\textwidth]{algorithm-figure-table/importance_based_reweighting/sd-turbo/paintings/0.99_1.1.png} & 
        \includegraphics[width=0.15\textwidth]{algorithm-figure-table/importance_based_reweighting/sd-turbo/photo/0.99_1.1.png} \\

        % [1.0, 1.1]
        \parbox[t][-2.75cm][c]{2.0cm}{\centering $[1.0, 1.1]$} & 
        \includegraphics[width=0.15\textwidth]{algorithm-figure-table/importance_based_reweighting/sd-turbo/anime/1.0_1.1.png} & 
        \includegraphics[width=0.15\textwidth]{algorithm-figure-table/importance_based_reweighting/sd-turbo/concept-art/1.0_1.1.png} & 
        \includegraphics[width=0.15\textwidth]{algorithm-figure-table/importance_based_reweighting/sd-turbo/paintings/1.0_1.1.png} & 
        \includegraphics[width=0.15\textwidth]{algorithm-figure-table/importance_based_reweighting/sd-turbo/photo/1.0_1.1.png} \\

        \rule{0pt}{0pt} \\

        \hline
    \end{tabular}
    \captionof{figure}{
        Samples synthesized by 2-step-inference SD-Turbo under difference re-weighting schedule. 
    }
    \label{fig-importance_based_reweighting_sdturbo_appx_1}
\end{table*}

% importance-based re-weighting, SD-Turbo, 2
% importance-based re-weighting, SD-Turbo, 2
\begin{table*}[t]
    \centering
    \begin{tabular}{c | c c c c}
        \hline

        \textbf{Re-Weighting} & \multicolumn{4}{c}{\textbf{SD-Turbo}} \\
        \textbf{Strategy} & anime & concept-art & paintings & photo \\
        
        \hline

        \rule{0pt}{0pt} \\
        
        % [1.01, 1.1]
        \parbox[t][-2.75cm][c]{2.0cm}{\centering $[1.01, 1.1]$} & 
        \includegraphics[width=0.15\textwidth]{algorithm-figure-table/importance_based_reweighting/sd-turbo/anime/1.01_1.1.png} & 
        \includegraphics[width=0.15\textwidth]{algorithm-figure-table/importance_based_reweighting/sd-turbo/concept-art/1.01_1.1.png} & 
        \includegraphics[width=0.15\textwidth]{algorithm-figure-table/importance_based_reweighting/sd-turbo/paintings/1.01_1.1.png} & 
        \includegraphics[width=0.15\textwidth]{algorithm-figure-table/importance_based_reweighting/sd-turbo/photo/1.01_1.1.png} \\

        % [1.02, 1.1]
        \parbox[t][-2.75cm][c]{2.0cm}{\centering $[1.02, 1.1]$} & 
        \includegraphics[width=0.15\textwidth]{algorithm-figure-table/importance_based_reweighting/sd-turbo/anime/1.02_1.1.png} & 
        \includegraphics[width=0.15\textwidth]{algorithm-figure-table/importance_based_reweighting/sd-turbo/concept-art/1.02_1.1.png} & 
        \includegraphics[width=0.15\textwidth]{algorithm-figure-table/importance_based_reweighting/sd-turbo/paintings/1.02_1.1.png} & 
        \includegraphics[width=0.15\textwidth]{algorithm-figure-table/importance_based_reweighting/sd-turbo/photo/1.02_1.1.png} \\

        % [1.03, 1.1]
        \parbox[t][-2.75cm][c]{2.0cm}{\centering $[1.03, 1.1]$} & 
        \includegraphics[width=0.15\textwidth]{algorithm-figure-table/importance_based_reweighting/sd-turbo/anime/1.03_1.1.png} & 
        \includegraphics[width=0.15\textwidth]{algorithm-figure-table/importance_based_reweighting/sd-turbo/concept-art/1.03_1.1.png} & 
        \includegraphics[width=0.15\textwidth]{algorithm-figure-table/importance_based_reweighting/sd-turbo/paintings/1.03_1.1.png} & 
        \includegraphics[width=0.15\textwidth]{algorithm-figure-table/importance_based_reweighting/sd-turbo/photo/1.03_1.1.png} \\

        % [1.04, 1.1]
        \parbox[t][-2.75cm][c]{2.0cm}{\centering $[1.04, 1.1]$} & 
        \includegraphics[width=0.15\textwidth]{algorithm-figure-table/importance_based_reweighting/sd-turbo/anime/1.04_1.1.png} & 
        \includegraphics[width=0.15\textwidth]{algorithm-figure-table/importance_based_reweighting/sd-turbo/concept-art/1.04_1.1.png} & 
        \includegraphics[width=0.15\textwidth]{algorithm-figure-table/importance_based_reweighting/sd-turbo/paintings/1.04_1.1.png} & 
        \includegraphics[width=0.15\textwidth]{algorithm-figure-table/importance_based_reweighting/sd-turbo/photo/1.04_1.1.png} \\

        % [1.05, 1.1]
        \parbox[t][-2.75cm][c]{2.0cm}{\centering $[1.05, 1.1]$} & 
        \includegraphics[width=0.15\textwidth]{algorithm-figure-table/importance_based_reweighting/sd-turbo/anime/1.05_1.1.png} & 
        \includegraphics[width=0.15\textwidth]{algorithm-figure-table/importance_based_reweighting/sd-turbo/concept-art/1.05_1.1.png} & 
        \includegraphics[width=0.15\textwidth]{algorithm-figure-table/importance_based_reweighting/sd-turbo/paintings/1.05_1.1.png} & 
        \includegraphics[width=0.15\textwidth]{algorithm-figure-table/importance_based_reweighting/sd-turbo/photo/1.05_1.1.png} \\

        \rule{0pt}{0pt} \\

        \hdashline

        \rule{0pt}{0pt} \\

        % [0.98, 1.15]
        \parbox[t][-2.75cm][c]{2.0cm}{\centering $[0.98, 1.15]$} & 
        \includegraphics[width=0.15\textwidth]{algorithm-figure-table/importance_based_reweighting/sd-turbo/anime/0.98_1.15.png} & 
        \includegraphics[width=0.15\textwidth]{algorithm-figure-table/importance_based_reweighting/sd-turbo/concept-art/0.98_1.15.png} & 
        \includegraphics[width=0.15\textwidth]{algorithm-figure-table/importance_based_reweighting/sd-turbo/paintings/0.98_1.15.png} & 
        \includegraphics[width=0.15\textwidth]{algorithm-figure-table/importance_based_reweighting/sd-turbo/photo/0.98_1.15.png} \\

        % [0.98, 1.2]
        \parbox[t][-2.75cm][c]{2.0cm}{\centering $[0.98, 1.2]$} & 
        \includegraphics[width=0.15\textwidth]{algorithm-figure-table/importance_based_reweighting/sd-turbo/anime/0.98_1.2.png} & 
        \includegraphics[width=0.15\textwidth]{algorithm-figure-table/importance_based_reweighting/sd-turbo/concept-art/0.98_1.2.png} & 
        \includegraphics[width=0.15\textwidth]{algorithm-figure-table/importance_based_reweighting/sd-turbo/paintings/0.98_1.2.png} & 
        \includegraphics[width=0.15\textwidth]{algorithm-figure-table/importance_based_reweighting/sd-turbo/photo/0.98_1.2.png} \\

        \rule{0pt}{0pt} \\

        \hline
    \end{tabular}
    \captionof{figure}{
        Samples synthesized by 2-step-inference SD-Turbo under difference re-weighting schedule (cont.). 
    }
    \label{fig-importance_based_reweighting_sdturbo_appx_2}
\end{table*}

% importance-based re-weighting, SDXL-Turbo, 1
% importance-based re-weighting, SDXL-Turbo, 1
\begin{table*}[t]
    \centering
    \begin{tabular}{c | c c c c}
        \hline

        \textbf{Re-Weighting} & \multicolumn{4}{c}{\textbf{SDXL-Turbo}} \\
        \textbf{Strategy} & anime & concept-art & paintings & photo \\
        
        \hline

        \rule{0pt}{0pt} \\
        
        % Vanilla
        \parbox[t][-2.75cm][c]{2.0cm}{\centering Vanilla} & 
        \includegraphics[width=0.15\textwidth]{algorithm-figure-table/importance_based_reweighting/sdxl-turbo/anime/default.png} & 
        \includegraphics[width=0.15\textwidth]{algorithm-figure-table/importance_based_reweighting/sdxl-turbo/concept-art/default.png} & 
        \includegraphics[width=0.15\textwidth]{algorithm-figure-table/importance_based_reweighting/sdxl-turbo/paintings/default.png} & 
        \includegraphics[width=0.15\textwidth]{algorithm-figure-table/importance_based_reweighting/sdxl-turbo/photo/default.png} \\

        \rule{0pt}{0pt} \\

        \hdashline

        \rule{0pt}{0pt} \\
            
        % [0.95, 1.1]
        \parbox[t][-2.75cm][c]{2.0cm}{\centering $[0.95, 1.1]$} & 
        \includegraphics[width=0.15\textwidth]{algorithm-figure-table/importance_based_reweighting/sdxl-turbo/anime/0.95_1.1.png} & 
        \includegraphics[width=0.15\textwidth]{algorithm-figure-table/importance_based_reweighting/sdxl-turbo/concept-art/0.95_1.1.png} & 
        \includegraphics[width=0.15\textwidth]{algorithm-figure-table/importance_based_reweighting/sdxl-turbo/paintings/0.95_1.1.png} & 
        \includegraphics[width=0.15\textwidth]{algorithm-figure-table/importance_based_reweighting/sdxl-turbo/photo/0.95_1.1.png} \\

        % [0.96, 1.1]
        \parbox[t][-2.75cm][c]{2.0cm}{\centering $[0.96, 1.1]$} & 
        \includegraphics[width=0.15\textwidth]{algorithm-figure-table/importance_based_reweighting/sdxl-turbo/anime/0.96_1.1.png} & 
        \includegraphics[width=0.15\textwidth]{algorithm-figure-table/importance_based_reweighting/sdxl-turbo/concept-art/0.96_1.1.png} & 
        \includegraphics[width=0.15\textwidth]{algorithm-figure-table/importance_based_reweighting/sdxl-turbo/paintings/0.96_1.1.png} & 
        \includegraphics[width=0.15\textwidth]{algorithm-figure-table/importance_based_reweighting/sdxl-turbo/photo/0.96_1.1.png} \\

        % [0.97, 1.1]
        \parbox[t][-2.75cm][c]{2.0cm}{\centering $[0.97, 1.1]$} & 
        \includegraphics[width=0.15\textwidth]{algorithm-figure-table/importance_based_reweighting/sdxl-turbo/anime/0.97_1.1.png} & 
        \includegraphics[width=0.15\textwidth]{algorithm-figure-table/importance_based_reweighting/sdxl-turbo/concept-art/0.97_1.1.png} & 
        \includegraphics[width=0.15\textwidth]{algorithm-figure-table/importance_based_reweighting/sdxl-turbo/paintings/0.97_1.1.png} & 
        \includegraphics[width=0.15\textwidth]{algorithm-figure-table/importance_based_reweighting/sdxl-turbo/photo/0.97_1.1.png} \\

        % [0.98, 1.1]
        \parbox[t][-2.75cm][c]{2.0cm}{\centering $[0.98, 1.1]$} & 
        \includegraphics[width=0.15\textwidth]{algorithm-figure-table/importance_based_reweighting/sdxl-turbo/anime/0.98_1.1.png} & 
        \includegraphics[width=0.15\textwidth]{algorithm-figure-table/importance_based_reweighting/sdxl-turbo/concept-art/0.98_1.1.png} & 
        \includegraphics[width=0.15\textwidth]{algorithm-figure-table/importance_based_reweighting/sdxl-turbo/paintings/0.98_1.1.png} & 
        \includegraphics[width=0.15\textwidth]{algorithm-figure-table/importance_based_reweighting/sdxl-turbo/photo/0.98_1.1.png} \\

        % [0.99, 1.1]
        \parbox[t][-2.75cm][c]{2.0cm}{\centering $[0.99, 1.1]$} & 
        \includegraphics[width=0.15\textwidth]{algorithm-figure-table/importance_based_reweighting/sdxl-turbo/anime/0.99_1.1.png} & 
        \includegraphics[width=0.15\textwidth]{algorithm-figure-table/importance_based_reweighting/sdxl-turbo/concept-art/0.99_1.1.png} & 
        \includegraphics[width=0.15\textwidth]{algorithm-figure-table/importance_based_reweighting/sdxl-turbo/paintings/0.99_1.1.png} & 
        \includegraphics[width=0.15\textwidth]{algorithm-figure-table/importance_based_reweighting/sdxl-turbo/photo/0.99_1.1.png} \\

        % [1.0, 1.1]
        \parbox[t][-2.75cm][c]{2.0cm}{\centering $[1.0, 1.1]$} & 
        \includegraphics[width=0.15\textwidth]{algorithm-figure-table/importance_based_reweighting/sdxl-turbo/anime/1.0_1.1.png} & 
        \includegraphics[width=0.15\textwidth]{algorithm-figure-table/importance_based_reweighting/sdxl-turbo/concept-art/1.0_1.1.png} & 
        \includegraphics[width=0.15\textwidth]{algorithm-figure-table/importance_based_reweighting/sdxl-turbo/paintings/1.0_1.1.png} & 
        \includegraphics[width=0.15\textwidth]{algorithm-figure-table/importance_based_reweighting/sdxl-turbo/photo/1.0_1.1.png} \\

        \rule{0pt}{0pt} \\

        \hline
    \end{tabular}
    \captionof{figure}{
        Samples synthesized by 2-step-inference SD-Turbo under difference re-weighting schedule. 
    }
    \label{fig-importance_based_reweighting_sdxlturbo_appx_1}
\end{table*}

% importance-based re-weighting, SDXL-Turbo, 2
% importance-based re-weighting, SDXL-Turbo, 2
\begin{table*}[t]
    \centering
    \begin{tabular}{c | c c c c}
        \hline

        \textbf{Re-Weighting} & \multicolumn{4}{c}{\textbf{SDXL-Turbo}} \\
        \textbf{Strategy} & anime & concept-art & paintings & photo \\
        
        \hline

        \rule{0pt}{0pt} \\
        
        % [1.01, 1.1]
        \parbox[t][-2.75cm][c]{2.0cm}{\centering $[1.01, 1.1]$} & 
        \includegraphics[width=0.15\textwidth]{algorithm-figure-table/importance_based_reweighting/sdxl-turbo/anime/1.01_1.1.png} & 
        \includegraphics[width=0.15\textwidth]{algorithm-figure-table/importance_based_reweighting/sdxl-turbo/concept-art/1.01_1.1.png} & 
        \includegraphics[width=0.15\textwidth]{algorithm-figure-table/importance_based_reweighting/sdxl-turbo/paintings/1.01_1.1.png} & 
        \includegraphics[width=0.15\textwidth]{algorithm-figure-table/importance_based_reweighting/sdxl-turbo/photo/1.01_1.1.png} \\

        % [1.02, 1.1]
        \parbox[t][-2.75cm][c]{2.0cm}{\centering $[1.02, 1.1]$} & 
        \includegraphics[width=0.15\textwidth]{algorithm-figure-table/importance_based_reweighting/sdxl-turbo/anime/1.02_1.1.png} & 
        \includegraphics[width=0.15\textwidth]{algorithm-figure-table/importance_based_reweighting/sdxl-turbo/concept-art/1.02_1.1.png} & 
        \includegraphics[width=0.15\textwidth]{algorithm-figure-table/importance_based_reweighting/sdxl-turbo/paintings/1.02_1.1.png} & 
        \includegraphics[width=0.15\textwidth]{algorithm-figure-table/importance_based_reweighting/sdxl-turbo/photo/1.02_1.1.png} \\

        % [1.03, 1.1]
        \parbox[t][-2.75cm][c]{2.0cm}{\centering $[1.03, 1.1]$} & 
        \includegraphics[width=0.15\textwidth]{algorithm-figure-table/importance_based_reweighting/sdxl-turbo/anime/1.03_1.1.png} & 
        \includegraphics[width=0.15\textwidth]{algorithm-figure-table/importance_based_reweighting/sdxl-turbo/concept-art/1.03_1.1.png} & 
        \includegraphics[width=0.15\textwidth]{algorithm-figure-table/importance_based_reweighting/sdxl-turbo/paintings/1.03_1.1.png} & 
        \includegraphics[width=0.15\textwidth]{algorithm-figure-table/importance_based_reweighting/sdxl-turbo/photo/1.03_1.1.png} \\

        % [1.04, 1.1]
        \parbox[t][-2.75cm][c]{2.0cm}{\centering $[1.04, 1.1]$} & 
        \includegraphics[width=0.15\textwidth]{algorithm-figure-table/importance_based_reweighting/sdxl-turbo/anime/1.04_1.1.png} & 
        \includegraphics[width=0.15\textwidth]{algorithm-figure-table/importance_based_reweighting/sdxl-turbo/concept-art/1.04_1.1.png} & 
        \includegraphics[width=0.15\textwidth]{algorithm-figure-table/importance_based_reweighting/sdxl-turbo/paintings/1.04_1.1.png} & 
        \includegraphics[width=0.15\textwidth]{algorithm-figure-table/importance_based_reweighting/sdxl-turbo/photo/1.04_1.1.png} \\

        % [1.05, 1.1]
        \parbox[t][-2.75cm][c]{2.0cm}{\centering $[1.05, 1.1]$} & 
        \includegraphics[width=0.15\textwidth]{algorithm-figure-table/importance_based_reweighting/sdxl-turbo/anime/1.05_1.1.png} & 
        \includegraphics[width=0.15\textwidth]{algorithm-figure-table/importance_based_reweighting/sdxl-turbo/concept-art/1.05_1.1.png} & 
        \includegraphics[width=0.15\textwidth]{algorithm-figure-table/importance_based_reweighting/sdxl-turbo/paintings/1.05_1.1.png} & 
        \includegraphics[width=0.15\textwidth]{algorithm-figure-table/importance_based_reweighting/sdxl-turbo/photo/1.05_1.1.png} \\

        \rule{0pt}{0pt} \\

        \hdashline

        \rule{0pt}{0pt} \\

        % [0.95, 1.15]
        \parbox[t][-2.75cm][c]{2.0cm}{\centering $[0.95, 1.15]$} & 
        \includegraphics[width=0.15\textwidth]{algorithm-figure-table/importance_based_reweighting/sdxl-turbo/anime/0.95_1.15.png} & 
        \includegraphics[width=0.15\textwidth]{algorithm-figure-table/importance_based_reweighting/sdxl-turbo/concept-art/0.95_1.15.png} & 
        \includegraphics[width=0.15\textwidth]{algorithm-figure-table/importance_based_reweighting/sdxl-turbo/paintings/0.95_1.15.png} & 
        \includegraphics[width=0.15\textwidth]{algorithm-figure-table/importance_based_reweighting/sdxl-turbo/photo/0.95_1.15.png} \\

        % [0.95, 1.2]
        \parbox[t][-2.75cm][c]{2.0cm}{\centering $[0.95, 1.2]$} & 
        \includegraphics[width=0.15\textwidth]{algorithm-figure-table/importance_based_reweighting/sdxl-turbo/anime/0.95_1.2.png} & 
        \includegraphics[width=0.15\textwidth]{algorithm-figure-table/importance_based_reweighting/sdxl-turbo/concept-art/0.95_1.2.png} & 
        \includegraphics[width=0.15\textwidth]{algorithm-figure-table/importance_based_reweighting/sdxl-turbo/paintings/0.95_1.2.png} & 
        \includegraphics[width=0.15\textwidth]{algorithm-figure-table/importance_based_reweighting/sdxl-turbo/photo/0.95_1.2.png} \\

        \rule{0pt}{0pt} \\

        \hline
    \end{tabular}
    \captionof{figure}{
        Samples synthesized by 2-step-inference SDXL-Turbo under difference re-weighting schedule (cont.). 
    }
    \label{fig-importance_based_reweighting_sdxlturbo_appx_2}
\end{table*}

\paragraph{Impacts of Parameters}

Fixing the upper bound $high$ of the weight range $[low, high]$, it can be observed that, as $low$ increases, the samples become clearer and sharper with more saturated colors. 
However, an excessively large $low$ may introduce anomalies, and lead to over-saturation of colors. 

Fixing the lower bound $low$ of the optimal re-weighting schedule ($low = 0.98$ for SD, and $low = 0.95$ for SDXL), it can be observed that, as $high$ increases, the colors in the samples become more saturated. 
An excessively large $high$ may also lead to over-saturation.

We provide the following empirical guidelines for selecting the range $[low, high]$: set $low$ slightly below $1.0$, and choose $high$ within the range $(1.0, 1.15)$. 

\paragraph{Failure Cases}

We present failure cases for SD-Turbo and SDXL-Turbo under their respective optimal re-weighting schedules, with samples generated under the following settings: 

\begin{itemize}
    \item \textbf{SD-Turbo}: 2-step inference with prompt ``\emph{A chicken smoking from a bong.}" under the re-weighting schedules of vanilla, $[0.98, 1.1]$, $[0.98, 1.15]$ and $[0.98, 1.2]$. 

    \item \textbf{SDXL-Turbo}: 2-step inference with prompt ``\emph{An old classic church is in front a big blue sky.}" under the re-weighting schedules of vanilla, $[0.95, 1.1]$, $[0.95, 1.15]$ and $[0.95, 1.2]$. 
\end{itemize}

It can be observed that, all our re-weighting schedules introduces anomalies in these cases. 

\subsection{Limitations}

Our importance-based re-weighting schedule essentially serves as an enhancement of the U-Net's inherent capabilities, which may account for our method's ability to achieve aesthetic enhancement while maintaining identity consistency. 

Consequently, the effects of re-weighting are partially contingent upon the quality of the original denoising trajectory. 
If the original trajectory leads to a low-quality region, our method may potentially further degrade the sampling quality.

\section{Limitations and Future Work}
\label{appx_sec-limitations_and_future_work}

While our method demonstrates strong generalization and robustness, the selection of its parameters (e.g., the weight range) remains empirical and may not be universally applicable. 
Future work could replace these manually selected hyper-parameters with learnable parameters, thereby adapting to a broader range of scenarios and potentially achieving better performance. 

Additionally, our proposed approach of monitoring the dynamic importance of network components using the Importance Probe, as well as the method of enhancing network capacities based on importance, may be transferable to other domains.
