# Supplementary material for: Dynamic Importance in Diffusion U-Net for Enhanced Image Synthesis
Source: arXiv:2504.03471 source file (2025-05-05)
Supplement: Supplementary file 2 [file dynamic_attention_pruning_tests_details.tex]

\section{Supplementary to Dynamic Attention Pruning}
\label{appx_sec-the_methodology_and_evaluation_of_dynamic_attention_pruning_tests}

\subsection{Overview}

We provide a schematic of dynamic attention pruning of diffusion U-Net in Fig.~\ref{fig-dynamic_pruning}. 

\begin{figure}[h]
    \centering
    \includegraphics[width=0.98\linewidth]{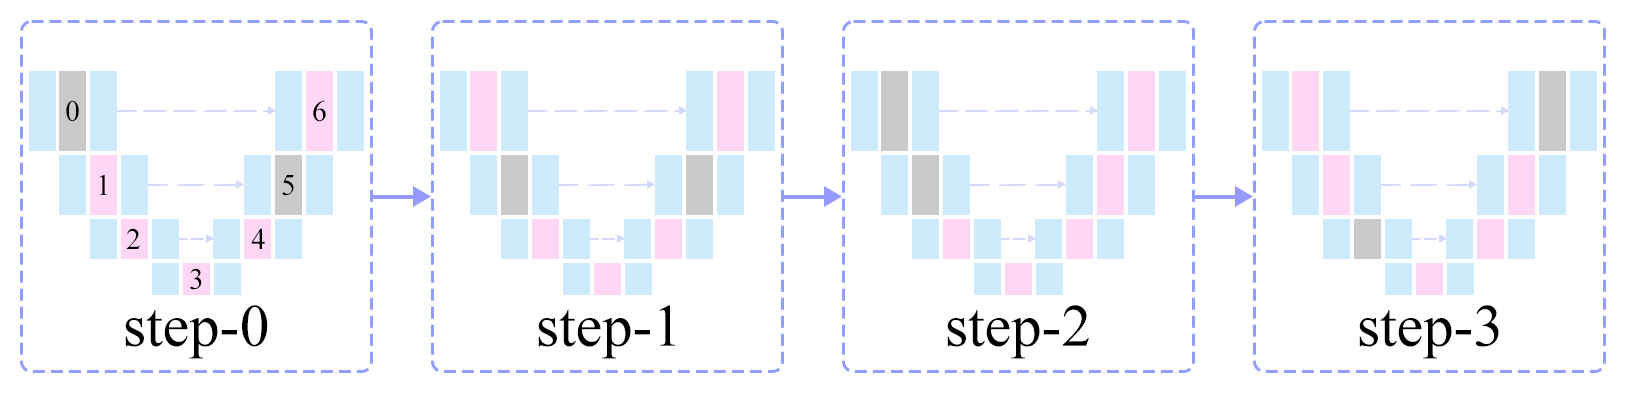}
    \caption{
        The schematic of dynamic pruning of SD U-Net, in which the gray rectangles represent the skipped Transformer blocks in that step. 
    }
    \label{fig-dynamic_pruning}
    \vspace{-10pt}
\end{figure}

\subsection{Strategy Design Mechanism}

Due to the potential synergistic effects among components within the network, simply skipping the least important blocks does not always guarantee optimal performance. 
To address this, we introduce a \emph{strategy design mechanism} to design skipping strategies based on the derived importance ranking. 

Specifically, at each denoising step, we focus on the three blocks with the lowest importance scores. 
Denote the indices of these blocks at step $t$ as $idx_0^{(t)}$, $idx_1^{(t)}$, $idx_2^{(t)}$. 

\begin{itemize}
    \item For single-block skipping strategies, we consider skipping block-$idx_0^{(t)}$ or block-$idx_1^{(t)}$ or block-$idx_2^{(t)}$. 
    \item For two-block skipping strategies, examine all the combinations of skipping (block-$idx_0^{(t)}$ and block-$idx_1^{(t)}$) or (block-$idx_0^{(t)}$ and block-$idx_2^{(t)}$) or (block-$idx_1^{(t)}$ and block-$idx_2^{(t)}$). 
\end{itemize}

We employ Depth First Search (DFS) to traverse all recommended skipping block combinations across the inference steps, constructing a set of task-specific skipping strategies.
For skipping strategies that involve skipping $k\ \ (1 \leq k \leq 3)$ block(s), $(C_3^k)^n$ schedule(s) will be recommended, and some of them may be duplicated or overlap with baseline strategies. 

\subsection{Experimental Settings}

We select the pre-trained SD-Turbo as the fundamental model. 
Following Sec.~\ref{appx_section-empirical_results_and_theoretical_consistency_subsection-appropriately_reweighting_contributions}, we choose the 2-step-inference task with the prompt ``\emph{Some cut up fruit is sitting in a blender.}'' as our target task.

For each skipping strategy provided by the strategy design mechanism, the student U-Net, adopting the corresponding skipping strategy, is fine-tuned on the training set under the supervision of the full teacher U-Net. 
We set the seeds for the training and test sets to $0$ and $21$, respectively, with each set comprising 100 distinct generation trajectories from the teacher U-Net.

We set the batch size to $8$. 
The student U-Net is fine-tuned for $300$ epochs with a learning rate of $5\mathrm{e}-6$. 
The fine-tuned student U-Net is then used for sampling, and the generation quality is compared with that of the teacher U-Net.

\subsection{Skipping Strategies}

All the recommended skipping strategies provided by the strategy design mechanism are listed in Tab.~\ref{tab-skipping_strategy_sdturbo_fruit_all}. 

% SD-Turbo 跳过策略 (全)
\begin{table}[h]
    \centering
    \begin{tabular}{c | c c | c}
        \hline
        
        \textbf{Strategy} & \multicolumn{2}{c|}{\textbf{Skipped Block Indices}} & \multirow{2}{*}{\textbf{Note}}  \\
        
        \textbf{Index} & step-0 & step-1 & ~ \\
        
        \hline

        % skip-1: baseline
        a.0 & 0 & 0 & block-0 \\
        a.1 & 1 & 1 & block-1\\
        a.2 & 2 & 2 & block-2 \\
        a.3 & 3 & 3 & block-3 \\
        a.4 & 4 & 4 & block-4\\
        a.5 & 5 & 5 & block-5 \\
        a.6 & 6 & 6 & block-6 \\

        \hdashline

        % skip-1: ours
        b.0 & 0 & 1 & ~ \\
        b.1 & 0 & 0 & identical to a.0 \\
        b.2 & 1 & 1 & identical to a.1 \\
        b.3 & 1 & 0 & ~ \\

        \hline

        % skip-2: baseline
        c.0 & 0, 6 & 0, 6 & floor-0 \\
        c.1 & 1, 5 & 1, 5 & floor-1 \\
        c.2 & 2, 4 & 2, 4 & floor-2 \\

        \hdashline

        % skip-2: ours
        d.0 & 0, 1 & 0, 1 & ~ \\
        d.1 & 0, 1 & 1, 5 & ~ \\
        d.2 & 0, 1 & 0, 5 & ~ \\
        d.3 & 0, 2 & 0, 1 & ~ \\
        d.4 & 0, 2 & 1, 5 & ~ \\
        d.5 & 0, 2 & 0, 5 & ~ \\
        d.6 & 1, 2 & 0, 1 & ~ \\
        d.7 & 1, 2 & 1, 5 & ~ \\
        d.8 & 1, 2 & 0, 5 & ~ \\

        \hline
    \end{tabular}
    \caption{
        Table of task-specific skipping strategies. 
    }
    \label{tab-skipping_strategy_sdturbo_fruit_all}
\end{table}

\subsection{Qualitative Results}

We provide qualitative results of samples generated by the pruned U-Net under different skipping strategies in Fig.~\ref{fig-sample_pruned_sdturbo_fruit_skip_1_a}, Fig.~\ref{fig-sample_pruned_sdturbo_fruit_skip_1_b}, Fig.~\ref{fig-sample_pruned_sdturbo_fruit_skip_2_c} and Fig.~\ref{fig-sample_pruned_sdturbo_fruit_skip_2_d}. 

The results demonstrate that, the U-Nets pruned under our skipping strategies achieve higher fidelity in pruned sampling (e.g., a more realistic blender), particularly when two blocks are skipped per step. 
Moreover, our pruned U-Net exhibits superior generalization on the test set.

\subsection{More Quantitative Results}

To quantitatively access the performance of the pruned U-Nets, we calculate some relative metrics are listed below: 

\begin{itemize}
    \item \textbf{FID} (Fréchet Inception Distance)~\cite{yu2021frechet}: measures the fidelity of the generated image compared to the original image. 
    \item \textbf{LPIPS} (Learned Perceptual Image Patch Similarity)~\cite{zhang2018unreasonable}: indicates the image quality and similarity. 
\end{itemize}

Using the samples generated by the teacher U-Net as the reference set, we calculate the FID and LPIPS for the fine-tuned student U-Net on the training and testing set, respectively. 

Quantitative results are presented in Table~\ref{tab-fid_lpips_fruit_all_appx}, with the corresponding scatter plots shown in Fig.~\ref{fig-scatter_fid_lpips_fruit_appx}. 
The results indicate that, the samples generated by our pruned U-Net achieve superior FID and LPIPS scores, particularly when two blocks are skipped per step. 

Notably, we find that, consistently skipping blk-3 (skipping strategy a.3) yields the best performance. 
We hypothesize that, this is due to blk-3 having the lowest resolution and the fewest parameters, allowing its functionality to be effectively compensated by the remaining two bottleneck blocks (blk-2 and blk-4). 
This hypothesis is supported by the results of the static skipping strategies in group (a).
It shows that statically skipping high-resolution blocks incurs a greater quality loss compared to statically skipping mid-low-resolution blocks.

Conversely, in a dynamic context, skipping mid-low-resolution blocks is not necessarily the optimal strategy. 
For instance, in the aforementioned experiments, our dynamic skipping strategy d.7 outperforms the static skipping strategy c.2. 
This highlights the importance of considering the dynamic importance shifts of blocks during the pruning process, rather than simply focusing on their resolutions.

% SD-Turbo 跳过策略 (全)
\begin{table}[h]
    \centering
    \begin{tabular}{c | c c : c c}
        \hline
        
        \textbf{Strategy} & \multicolumn{2}{c:}{\textbf{FID} $\downarrow$} & \multicolumn{2}{c}{\textbf{LPIPS} $\downarrow$} \\
        
        \textbf{Index} & train & test & train & test \\
        
        \hline

        % skip-1: baseline
        a.0 / \textbf{b.1} & 402.8469 & 397.1920 & 0.7148 & 0.6894 \\
        a.1 / b.2 & 241.3091 & 244.8477 & \sbest{0.6170} & 0.6201 \\
        a.2 & \sbest{176.8128} & \sbest{173.6468}  & \tbest{0.6309} & 0.6274 \\
        a.3 & \best{40.4357} & \best{39.7413} & \best{0.3915} & \best{0.5266} \\
        a.4 & \tbest{215.3175} & \tbest{214.6077}  & 0.6350 & \sbest{0.5603} \\
        a.5 & 242.5459 & 240.0058  & 0.6334 & \tbest{0.5763} \\
        a.6 & 401.0944 & 404.0254  & 0.8366 & 0.8085 \\

        \hdashline

        % skip-1: ours
        b.0 & 354.4077 & 356.5143  & 0.6550 & 0.6509 \\
        % b.1 & ~ & ~ \\
        % b.2 & ~ & ~ \\
        b.3 & 259.9984 & 259.2821  & 0.6439 & 0.6293 \\

        \hline

        % skip-2: baseline
        c.0 & 453.6726 & 456.1274  & 0.8295 & 0.8302 \\
        c.1 & 401.6146 & 401.9952  & \sbest{0.6595} & \best{0.6436} \\
        c.2 & 362.4762 & 357.4724  & \best{0.6513} & \sbest{0.6623} \\

        \hdashline

        % skip-2: ours
        d.0 & 457.7766 & 456.3885  & 0.6959 & 0.6964 \\
        d.1 & 467.9547 & 464.4429  & 0.7593 & 0.7642 \\
        d.2 & 472.7829 & 466.7573  & 0.8131 & 0.8022 \\
        d.3 & 409.4545 & 412.3269  & \tbest{0.6853} & \tbest{0.6822} \\
        d.4 & 371.9738 & 387.3718  & 0.7331 & 0.7514 \\
        d.5 & 374.8360 & 383.1508  & 0.7815 & 0.7822 \\
        d.6 & \tbest{313.1157} & \tbest{309.0396}  & 0.7194 & 0.7149 \\
        \textbf{d.7} & \best{305.8840} & \best{304.8817} & 0.7048 & 0.7084 \\
        d.8 & \sbest{307.3236} & \sbest{304.9316}  & 0.7339 & 0.7067 \\

        \hline
    \end{tabular}
    \caption{
        Comparison of FID and LPIPS between vanilla, baseline skipping strategies, and our suggested strategies. 
        Multiple skipping strategies between adjacent solid or dashed lines are grouped as one set. 
    }
    \label{tab-fid_lpips_fruit_all_appx}
\end{table}

\begin{figure}[h]
    \centering
    \includegraphics[width=0.98\linewidth]{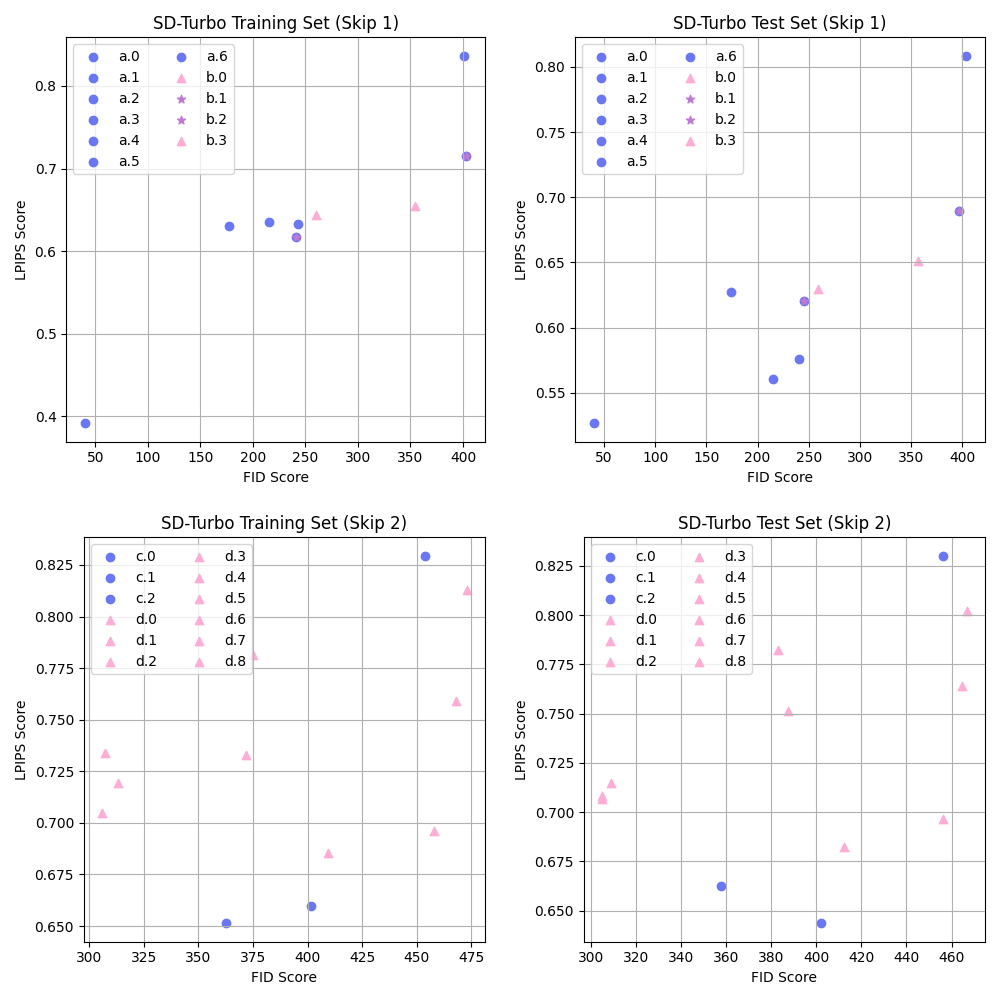}
    \caption{
        (Fig.~\ref{fig-scatter_fid_lpips_fruit} in the main paper)
        Scatter plot of FID and LPIPS under different skipping strategies (the further lower-left, the better). 
        Baseline strategies are represented by blue circles, unique points from our strategies are shown as pink triangles, while points overlapping with baseline points are marked with purple stars.
    }
    \label{fig-scatter_fid_lpips_fruit_appx}
    \vspace{-10pt}
\end{figure}

\subsection{Limitations}

While the skipping strategies generated by our approach are more likely to outperform baseline strategies, we cannot guarantee that the optimal solution(s) will be found among all possible skipping strategies.

% pruned sampling, SD-Turbo, fruit, vanilla 和 skip-1 baselines
\begin{table*}[t]
    \centering
    \begin{tabular}{c | c c c | c c c}
        \hline

        \textbf{Strategy Index} & ~ & \textbf{Training Set} & ~ & ~ & \textbf{Test Set} & ~ \\
        
        \hline

        \rule{0pt}{0pt} \\
        
        % Vanilla
        \parbox[t][-2.25cm][c]{2.0cm}{\centering Vanilla} & 
        \includegraphics[width=0.12\textwidth]{algorithm-figure-table/sample_pruned/training/23/default.png} & 
        \includegraphics[width=0.12\textwidth]{algorithm-figure-table/sample_pruned/training/52/default.png} & 
        \includegraphics[width=0.12\textwidth]{algorithm-figure-table/sample_pruned/training/74/default.png} & 
        \includegraphics[width=0.12\textwidth]{algorithm-figure-table/sample_pruned/test/22/default.png} & 
        \includegraphics[width=0.12\textwidth]{algorithm-figure-table/sample_pruned/test/73/default.png} & 
        \includegraphics[width=0.12\textwidth]{algorithm-figure-table/sample_pruned/test/83/default.png} \\

        \rule{0pt}{0pt} \\

        \hline

        \rule{0pt}{0pt} \\

        % a.0
        \parbox[t][-2.25cm][c]{2.0cm}{\centering a.0 / \textbf{b.1}} & 
        \includegraphics[width=0.12\textwidth]{algorithm-figure-table/sample_pruned/training/23/static-0.png} & 
        \includegraphics[width=0.12\textwidth]{algorithm-figure-table/sample_pruned/training/52/static-0.png} & 
        \includegraphics[width=0.12\textwidth]{algorithm-figure-table/sample_pruned/training/74/static-0.png} & 
        \includegraphics[width=0.12\textwidth]{algorithm-figure-table/sample_pruned/test/22/static-0.png} & 
        \includegraphics[width=0.12\textwidth]{algorithm-figure-table/sample_pruned/test/73/static-0.png} & 
        \includegraphics[width=0.12\textwidth]{algorithm-figure-table/sample_pruned/test/83/static-0.png} \\

        % a.1
        \parbox[t][-2.25cm][c]{2.0cm}{\centering a.1 / b.2} & 
        \includegraphics[width=0.12\textwidth]{algorithm-figure-table/sample_pruned/training/23/static-1.png} & 
        \includegraphics[width=0.12\textwidth]{algorithm-figure-table/sample_pruned/training/52/static-1.png} & 
        \includegraphics[width=0.12\textwidth]{algorithm-figure-table/sample_pruned/training/74/static-1.png} & 
        \includegraphics[width=0.12\textwidth]{algorithm-figure-table/sample_pruned/test/22/static-1.png} & 
        \includegraphics[width=0.12\textwidth]{algorithm-figure-table/sample_pruned/test/73/static-1.png} & 
        \includegraphics[width=0.12\textwidth]{algorithm-figure-table/sample_pruned/test/83/static-1.png} \\

        % a.2
        \parbox[t][-2.25cm][c]{2.0cm}{\centering a.2} & 
        \includegraphics[width=0.12\textwidth]{algorithm-figure-table/sample_pruned/training/23/static-2.png} & 
        \includegraphics[width=0.12\textwidth]{algorithm-figure-table/sample_pruned/training/52/static-2.png} & 
        \includegraphics[width=0.12\textwidth]{algorithm-figure-table/sample_pruned/training/74/static-2.png} & 
        \includegraphics[width=0.12\textwidth]{algorithm-figure-table/sample_pruned/test/22/static-2.png} & 
        \includegraphics[width=0.12\textwidth]{algorithm-figure-table/sample_pruned/test/73/static-2.png} & 
        \includegraphics[width=0.12\textwidth]{algorithm-figure-table/sample_pruned/test/83/static-2.png} \\

        % a.3
        \parbox[t][-2.25cm][c]{2.0cm}{\centering a.3} & 
        \includegraphics[width=0.12\textwidth]{algorithm-figure-table/sample_pruned/training/23/static-3.png} & 
        \includegraphics[width=0.12\textwidth]{algorithm-figure-table/sample_pruned/training/52/static-3.png} & 
        \includegraphics[width=0.12\textwidth]{algorithm-figure-table/sample_pruned/training/74/static-3.png} & 
        \includegraphics[width=0.12\textwidth]{algorithm-figure-table/sample_pruned/test/22/static-3.png} & 
        \includegraphics[width=0.12\textwidth]{algorithm-figure-table/sample_pruned/test/73/static-3.png} & 
        \includegraphics[width=0.12\textwidth]{algorithm-figure-table/sample_pruned/test/83/static-3.png} \\

        % a.4
        \parbox[t][-2.25cm][c]{2.0cm}{\centering a.4} & 
        \includegraphics[width=0.12\textwidth]{algorithm-figure-table/sample_pruned/training/23/static-4.png} & 
        \includegraphics[width=0.12\textwidth]{algorithm-figure-table/sample_pruned/training/52/static-4.png} & 
        \includegraphics[width=0.12\textwidth]{algorithm-figure-table/sample_pruned/training/74/static-4.png} & 
        \includegraphics[width=0.12\textwidth]{algorithm-figure-table/sample_pruned/test/22/static-4.png} & 
        \includegraphics[width=0.12\textwidth]{algorithm-figure-table/sample_pruned/test/73/static-4.png} & 
        \includegraphics[width=0.12\textwidth]{algorithm-figure-table/sample_pruned/test/83/static-4.png} \\

        % a.5
        \parbox[t][-2.25cm][c]{2.0cm}{\centering a.5} & 
        \includegraphics[width=0.12\textwidth]{algorithm-figure-table/sample_pruned/training/23/static-5.png} & 
        \includegraphics[width=0.12\textwidth]{algorithm-figure-table/sample_pruned/training/52/static-5.png} & 
        \includegraphics[width=0.12\textwidth]{algorithm-figure-table/sample_pruned/training/74/static-5.png} & 
        \includegraphics[width=0.12\textwidth]{algorithm-figure-table/sample_pruned/test/22/static-5.png} & 
        \includegraphics[width=0.12\textwidth]{algorithm-figure-table/sample_pruned/test/73/static-5.png} & 
        \includegraphics[width=0.12\textwidth]{algorithm-figure-table/sample_pruned/test/83/static-5.png} \\

        % a.6
        \parbox[t][-2.25cm][c]{2.0cm}{\centering a.6} & 
        \includegraphics[width=0.12\textwidth]{algorithm-figure-table/sample_pruned/training/23/static-6.png} & 
        \includegraphics[width=0.12\textwidth]{algorithm-figure-table/sample_pruned/training/52/static-6.png} & 
        \includegraphics[width=0.12\textwidth]{algorithm-figure-table/sample_pruned/training/74/static-6.png} & 
        \includegraphics[width=0.12\textwidth]{algorithm-figure-table/sample_pruned/test/22/static-6.png} & 
        \includegraphics[width=0.12\textwidth]{algorithm-figure-table/sample_pruned/test/73/static-6.png} & 
        \includegraphics[width=0.12\textwidth]{algorithm-figure-table/sample_pruned/test/83/static-6.png} \\

        \rule{0pt}{0pt} \\

        \hline
    \end{tabular}
    \captionof{figure}{
        Samples synthesized by Vanilla SD-Turbo U-Net, and U-Net with skipping strategies in group (a).
    }
    \label{fig-sample_pruned_sdturbo_fruit_skip_1_a}
\end{table*}

% pruned sampling, SD-Turbo, fruit skip-1 ours
\begin{table*}[t]
    \centering
    \begin{tabular}{c | c c c | c c c}
        \hline

        \textbf{Strategy Index} & ~ & \textbf{Training Set} & ~ & ~ & \textbf{Test Set} & ~ \\
        
        \hline

        \rule{0pt}{0pt} \\

        % b.0
        \parbox[t][-2.25cm][c]{2.0cm}{\centering b.0} & 
        \includegraphics[width=0.12\textwidth]{algorithm-figure-table/sample_pruned/training/23/skip-1_0.png} & 
        \includegraphics[width=0.12\textwidth]{algorithm-figure-table/sample_pruned/training/52/skip-1_0.png} & 
        \includegraphics[width=0.12\textwidth]{algorithm-figure-table/sample_pruned/training/74/skip-1_0.png} & 
        \includegraphics[width=0.12\textwidth]{algorithm-figure-table/sample_pruned/test/22/skip-1_0.png} & 
        \includegraphics[width=0.12\textwidth]{algorithm-figure-table/sample_pruned/test/73/skip-1_0.png} & 
        \includegraphics[width=0.12\textwidth]{algorithm-figure-table/sample_pruned/test/83/skip-1_0.png} \\

        % b.3
        \parbox[t][-2.25cm][c]{2.0cm}{\centering b.3} & 
        \includegraphics[width=0.12\textwidth]{algorithm-figure-table/sample_pruned/training/23/skip-1_3.png} & 
        \includegraphics[width=0.12\textwidth]{algorithm-figure-table/sample_pruned/training/52/skip-1_3.png} & 
        \includegraphics[width=0.12\textwidth]{algorithm-figure-table/sample_pruned/training/74/skip-1_3.png} & 
        \includegraphics[width=0.12\textwidth]{algorithm-figure-table/sample_pruned/test/22/skip-1_3.png} & 
        \includegraphics[width=0.12\textwidth]{algorithm-figure-table/sample_pruned/test/73/skip-1_3.png} & 
        \includegraphics[width=0.12\textwidth]{algorithm-figure-table/sample_pruned/test/83/skip-1_3.png} \\

        \rule{0pt}{0pt} \\

        \hline
    \end{tabular}
    \captionof{figure}{
        Samples synthesized by U-Net with skipping strategies in group (b).
    }
    \label{fig-sample_pruned_sdturbo_fruit_skip_1_b}
\end{table*}

% pruned sampling, SD-Turbo, fruit skip-2 baselines
\begin{table*}[t]
    \centering
    \begin{tabular}{c | c c c | c c c}
        \hline

        \textbf{Strategy Index} & ~ & \textbf{Training Set} & ~ & ~ & \textbf{Test Set} & ~ \\
        
        \hline

        \rule{0pt}{0pt} \\

        % c.0
        \parbox[t][-2.25cm][c]{2.0cm}{\centering c.0} & 
        \includegraphics[width=0.12\textwidth]{algorithm-figure-table/sample_pruned/training/23/static-0,6.png} & 
        \includegraphics[width=0.12\textwidth]{algorithm-figure-table/sample_pruned/training/52/static-0,6.png} & 
        \includegraphics[width=0.12\textwidth]{algorithm-figure-table/sample_pruned/training/74/static-0,6.png} & 
        \includegraphics[width=0.12\textwidth]{algorithm-figure-table/sample_pruned/test/22/static-0,6.png} & 
        \includegraphics[width=0.12\textwidth]{algorithm-figure-table/sample_pruned/test/73/static-0,6.png} & 
        \includegraphics[width=0.12\textwidth]{algorithm-figure-table/sample_pruned/test/83/static-0,6.png} \\

        % c.1
        \parbox[t][-2.25cm][c]{2.0cm}{\centering c.1} & 
        \includegraphics[width=0.12\textwidth]{algorithm-figure-table/sample_pruned/training/23/static-1,5.png} & 
        \includegraphics[width=0.12\textwidth]{algorithm-figure-table/sample_pruned/training/52/static-1,5.png} & 
        \includegraphics[width=0.12\textwidth]{algorithm-figure-table/sample_pruned/training/74/static-1,5.png} & 
        \includegraphics[width=0.12\textwidth]{algorithm-figure-table/sample_pruned/test/22/static-1,5.png} & 
        \includegraphics[width=0.12\textwidth]{algorithm-figure-table/sample_pruned/test/73/static-1,5.png} & 
        \includegraphics[width=0.12\textwidth]{algorithm-figure-table/sample_pruned/test/83/static-1,5.png} \\

        % c.2
        \parbox[t][-2.25cm][c]{2.0cm}{\centering c.2} & 
        \includegraphics[width=0.12\textwidth]{algorithm-figure-table/sample_pruned/training/23/static-2,4.png} & 
        \includegraphics[width=0.12\textwidth]{algorithm-figure-table/sample_pruned/training/52/static-2,4.png} & 
        \includegraphics[width=0.12\textwidth]{algorithm-figure-table/sample_pruned/training/74/static-2,4.png} & 
        \includegraphics[width=0.12\textwidth]{algorithm-figure-table/sample_pruned/test/22/static-2,4.png} & 
        \includegraphics[width=0.12\textwidth]{algorithm-figure-table/sample_pruned/test/73/static-2,4.png} & 
        \includegraphics[width=0.12\textwidth]{algorithm-figure-table/sample_pruned/test/83/static-2,4.png} \\

        \rule{0pt}{0pt} \\

        \hline
    \end{tabular}
    \captionof{figure}{
        Samples synthesized by U-Net with skipping strategies in group (c).
    }
    \label{fig-sample_pruned_sdturbo_fruit_skip_2_c}
\end{table*}

% pruned sampling, SD-Turbo, fruit skip-2 ours
\begin{table*}[t]
    \centering
    \begin{tabular}{c | c c c | c c c}
        \hline

        \textbf{Strategy Index} & ~ & \textbf{Training Set} & ~ & ~ & \textbf{Test Set} & ~ \\
        
        \hline

        \rule{0pt}{0pt} \\

        % d.0
        \parbox[t][-2.25cm][c]{2.0cm}{\centering d.0} & 
        \includegraphics[width=0.12\textwidth]{algorithm-figure-table/sample_pruned/training/23/skip-2_0.png} & 
        \includegraphics[width=0.12\textwidth]{algorithm-figure-table/sample_pruned/training/52/skip-2_0.png} & 
        \includegraphics[width=0.12\textwidth]{algorithm-figure-table/sample_pruned/training/74/skip-2_0.png} & 
        \includegraphics[width=0.12\textwidth]{algorithm-figure-table/sample_pruned/test/22/skip-2_0.png} & 
        \includegraphics[width=0.12\textwidth]{algorithm-figure-table/sample_pruned/test/73/skip-2_0.png} & 
        \includegraphics[width=0.12\textwidth]{algorithm-figure-table/sample_pruned/test/83/skip-2_0.png} \\

        % d.1
        \parbox[t][-2.25cm][c]{2.0cm}{\centering d.1} & 
        \includegraphics[width=0.12\textwidth]{algorithm-figure-table/sample_pruned/training/23/skip-2_1.png} & 
        \includegraphics[width=0.12\textwidth]{algorithm-figure-table/sample_pruned/training/52/skip-2_1.png} & 
        \includegraphics[width=0.12\textwidth]{algorithm-figure-table/sample_pruned/training/74/skip-2_1.png} & 
        \includegraphics[width=0.12\textwidth]{algorithm-figure-table/sample_pruned/test/22/skip-2_1.png} & 
        \includegraphics[width=0.12\textwidth]{algorithm-figure-table/sample_pruned/test/73/skip-2_1.png} & 
        \includegraphics[width=0.12\textwidth]{algorithm-figure-table/sample_pruned/test/83/skip-2_1.png} \\

        % d.2
        \parbox[t][-2.25cm][c]{2.0cm}{\centering d.2} & 
        \includegraphics[width=0.12\textwidth]{algorithm-figure-table/sample_pruned/training/23/skip-2_2.png} & 
        \includegraphics[width=0.12\textwidth]{algorithm-figure-table/sample_pruned/training/52/skip-2_2.png} & 
        \includegraphics[width=0.12\textwidth]{algorithm-figure-table/sample_pruned/training/74/skip-2_2.png} & 
        \includegraphics[width=0.12\textwidth]{algorithm-figure-table/sample_pruned/test/22/skip-2_2.png} & 
        \includegraphics[width=0.12\textwidth]{algorithm-figure-table/sample_pruned/test/73/skip-2_2.png} & 
        \includegraphics[width=0.12\textwidth]{algorithm-figure-table/sample_pruned/test/83/skip-2_2.png} \\

        % d.3
        \parbox[t][-2.25cm][c]{2.0cm}{\centering d.3} & 
        \includegraphics[width=0.12\textwidth]{algorithm-figure-table/sample_pruned/training/23/skip-2_3.png} & 
        \includegraphics[width=0.12\textwidth]{algorithm-figure-table/sample_pruned/training/52/skip-2_3.png} & 
        \includegraphics[width=0.12\textwidth]{algorithm-figure-table/sample_pruned/training/74/skip-2_3.png} & 
        \includegraphics[width=0.12\textwidth]{algorithm-figure-table/sample_pruned/test/22/skip-2_3.png} & 
        \includegraphics[width=0.12\textwidth]{algorithm-figure-table/sample_pruned/test/73/skip-2_3.png} & 
        \includegraphics[width=0.12\textwidth]{algorithm-figure-table/sample_pruned/test/83/skip-2_3.png} \\

        % d.4
        \parbox[t][-2.25cm][c]{2.0cm}{\centering d.4} & 
        \includegraphics[width=0.12\textwidth]{algorithm-figure-table/sample_pruned/training/23/skip-2_4.png} & 
        \includegraphics[width=0.12\textwidth]{algorithm-figure-table/sample_pruned/training/52/skip-2_4.png} & 
        \includegraphics[width=0.12\textwidth]{algorithm-figure-table/sample_pruned/training/74/skip-2_4.png} & 
        \includegraphics[width=0.12\textwidth]{algorithm-figure-table/sample_pruned/test/22/skip-2_4.png} & 
        \includegraphics[width=0.12\textwidth]{algorithm-figure-table/sample_pruned/test/73/skip-2_4.png} & 
        \includegraphics[width=0.12\textwidth]{algorithm-figure-table/sample_pruned/test/83/skip-2_4.png} \\

        % d.5
        \parbox[t][-2.25cm][c]{2.0cm}{\centering d.5} & 
        \includegraphics[width=0.12\textwidth]{algorithm-figure-table/sample_pruned/training/23/skip-2_5.png} & 
        \includegraphics[width=0.12\textwidth]{algorithm-figure-table/sample_pruned/training/52/skip-2_5.png} & 
        \includegraphics[width=0.12\textwidth]{algorithm-figure-table/sample_pruned/training/74/skip-2_5.png} & 
        \includegraphics[width=0.12\textwidth]{algorithm-figure-table/sample_pruned/test/22/skip-2_5.png} & 
        \includegraphics[width=0.12\textwidth]{algorithm-figure-table/sample_pruned/test/73/skip-2_5.png} & 
        \includegraphics[width=0.12\textwidth]{algorithm-figure-table/sample_pruned/test/83/skip-2_5.png} \\

        % d.6
        \parbox[t][-2.25cm][c]{2.0cm}{\centering d.6} & 
        \includegraphics[width=0.12\textwidth]{algorithm-figure-table/sample_pruned/training/23/skip-2_6.png} & 
        \includegraphics[width=0.12\textwidth]{algorithm-figure-table/sample_pruned/training/52/skip-2_6.png} & 
        \includegraphics[width=0.12\textwidth]{algorithm-figure-table/sample_pruned/training/74/skip-2_6.png} & 
        \includegraphics[width=0.12\textwidth]{algorithm-figure-table/sample_pruned/test/22/skip-2_6.png} & 
        \includegraphics[width=0.12\textwidth]{algorithm-figure-table/sample_pruned/test/73/skip-2_6.png} & 
        \includegraphics[width=0.12\textwidth]{algorithm-figure-table/sample_pruned/test/83/skip-2_6.png} \\

        % d.7
        \parbox[t][-2.25cm][c]{2.0cm}{\centering \textbf{d.7}} & 
        \includegraphics[width=0.12\textwidth]{algorithm-figure-table/sample_pruned/training/23/skip-2_7.png} & 
        \includegraphics[width=0.12\textwidth]{algorithm-figure-table/sample_pruned/training/52/skip-2_7.png} & 
        \includegraphics[width=0.12\textwidth]{algorithm-figure-table/sample_pruned/training/74/skip-2_7.png} & 
        \includegraphics[width=0.12\textwidth]{algorithm-figure-table/sample_pruned/test/22/skip-2_7.png} & 
        \includegraphics[width=0.12\textwidth]{algorithm-figure-table/sample_pruned/test/73/skip-2_7.png} & 
        \includegraphics[width=0.12\textwidth]{algorithm-figure-table/sample_pruned/test/83/skip-2_7.png} \\

        % d.8
        \parbox[t][-2.25cm][c]{2.0cm}{\centering d.8} & 
        \includegraphics[width=0.12\textwidth]{algorithm-figure-table/sample_pruned/training/23/skip-2_8.png} & 
        \includegraphics[width=0.12\textwidth]{algorithm-figure-table/sample_pruned/training/52/skip-2_8.png} & 
        \includegraphics[width=0.12\textwidth]{algorithm-figure-table/sample_pruned/training/74/skip-2_8.png} & 
        \includegraphics[width=0.12\textwidth]{algorithm-figure-table/sample_pruned/test/22/skip-2_8.png} & 
        \includegraphics[width=0.12\textwidth]{algorithm-figure-table/sample_pruned/test/73/skip-2_8.png} & 
        \includegraphics[width=0.12\textwidth]{algorithm-figure-table/sample_pruned/test/83/skip-2_8.png} \\

        \rule{0pt}{0pt} \\

        \hline
    \end{tabular}
    \captionof{figure}{
        Samples synthesized by U-Net with skipping strategies in group (d).
    }
    \label{fig-sample_pruned_sdturbo_fruit_skip_2_d}
\end{table*}
