# Supplementary material for: Dynamic Importance in Diffusion U-Net for Enhanced Image Synthesis
Source: arXiv:2504.03471 source file (2025-05-05)
Supplement: Supplementary file 3 [file empirical_results_and_theoretical_consistency.tex]

\section{Theory-Experiment Consistency Analysis}
\label{appx_sec-theory_experiment_consistency_analysis}

Empirically,~\cite{pnpDiffusion2022} has observed that: 

\begin{itemize}
    \item The high-resolution blocks within the U-Net primarily capture high-frequency (HF) information, such as details, edges and textures. 
    In our context, these blocks are dominated by $\pmb{g}_i$. 

    \item The low-resolution blocks within the U-Net capture low/mid-frequency (LF) information, such as layout and semantics. 
    In our context, these blocks are dominated by $\pmb{f}_i$. 
\end{itemize}

Experimental results in~\cite{yang2022diffusionprobabilisticmodelslim, cao2023masactrl, zhou2024generating, zhou2025attentiondistillationunifiedapproach} have also shown that: 
\begin{itemize}
    \item At early time steps, Diffusion models (DMs) primarily reconstruct low-frequency components. 
    \item At later time steps, DMs progressively recover high-frequency components. 
\end{itemize}
Recently,~\cite{chen2025free} theoretically proved these conclusions. 

Based on the above observations, we provide further discussion on our experimental results, demonstrating the consistency between the experimental phenomena and theoretical analysis. 

\subsection{Misweighting Contributions}

We evaluate static weighting schedules, where each block is assigned a weight of 1.1 respectively, in Tab.~\ref{tab-comparison_between_different_models_and_steps_appx}. 

Static weighting schedules cannot leverage the dynamic role evolution of the Transformer blocks throughout the denosing process. 
To ensure SNR improvement, ideally, one should design an oracle and time-universal set of weights $\{w_i\}$, that correctly re-weight $\text{Var} (\pmb{f}_i)$, $\text{Var} (\pmb{g}_i)$ and $\text{Var} (\pmb{n}_i)$. 
At the very least, the positive gains from re-weighting should outweigh the negative impacts. 
However, this study observes that, the importance of each block can change significantly during the inference process. 
Thus, in a static context, the aforementioned oracle $\{w_i\}$ does not always exist. 

Results in Tab.~\ref{tab-comparison_between_different_models_and_steps_appx} reveal that, applying certain weighting schedules leads to performance degradation compared to the vanilla weighting schedule. 
We speculate that, this occurs because misweighting the contributions of componenets will increase $\text{Var} (\Delta \hat{\pmb{\epsilon}}_t')$, thereby reducing the SNR. 
Fixed the number of inference steps, samples with lower SNR may not be fully denoised, resulting in lower aesthetic scores. 

Additionally, it can also be observed that, in a static context, assigning weights $w_i > 1.0$ to high-resolution blocks is more likely to improve the performance. 
Theoretically, it is because the weighted coefficient corresponding to $\text{Var}(\pmb{g}_i)$ in Eq.~\ref{eq-the_variance_of_the_error_appx} is $(w_i - 1)^2$, while the one for $\text{Var}(\pmb{f}_i)$ is $w_i^2$. 
Compared to statically re-weighting mid-low-resolution blocks (where $\pmb{f}_i$ dominates), statically re-weighting high-resolution blocks (where $\pmb{g}_i$ dominates) results in a smaller negative impact when a misweighting happens. 

\subsection{Appropriately Re-weighting Contributions}
\label{appx_section-empirical_results_and_theoretical_consistency_subsection-appropriately_reweighting_contributions}

\paragraph{Importance Ranking}
Conversely, we utilize the IP to obtain the importance of each block throughout the denoising process. 
The derived importance rankings of the prompt ``\emph{Some cut up fruit is sitting in a blender. }" are presented in Tab.~\ref{tab-importance_sdturbo_sdxlturbo_fruit_appx}. 

To more clearly illustrate the evolution of importance rankings of the blocks throughout the denoising process, we apply IP to 20-step inference SD v2.1 and SDXL using the same prompt.
Results are shown in Tab.~\ref{tab-importance_sd_sdxl_fruit_appx}. 

The importance rankings offer a preliminary glimpse into the dynamic shifts in importance. 
More precisely, the voting score and the importance scores provide a finer-grained perspective.

% 2 步 SD-Turbo/SDXL-Turbo 的重要性排名
\begin{table}[h]
    \centering
    \caption{
        (Tab.~\ref{tab-dynamic_importance_ranking_fruit} in the main paper) 
        Dynamic importance ranking of 2-step SD-Turbo/SDXL-Turbo U-Net, arranged in non-descending order. 
    }
    \begin{tabular}{c | c : c}
        \hline
        \multirow{2}{*}{\textbf{Step}} & 
        \multicolumn{2}{c}{\textbf{Importance Ranking}} \\

        ~ & SD-Turbo & SDXL-Turbo \\
        \hline

        0 & 0 1 2 4 6 5 3 & 1 2 5 3 4 \\ 
        1 & 1 0 5 4 2 6 3 & 1 2 5 4 3 \\ 

        \hline
    \end{tabular}
    \label{tab-importance_sdturbo_sdxlturbo_fruit_appx}
\end{table}

% 20 步推理 SD v2.1/SDXL 的重要性排名
\begin{table}[h]
    \centering
    \caption{
        Dynamic importance ranking of 20-step SD v2.1/SDXL U-Net, arranged in non-descending order. 
    }
    \begin{tabular}{c | c : c}
        \hline
        \multirow{2}{*}{\textbf{Step}} & 
        \multicolumn{2}{c}{\textbf{Importance Ranking}} \\

        ~ & SD v2.1 & SDXL \\
        \hline

        0 & 6 2 3 0 4 1 5 & 5 4 2 3 1 \\ 
        1 & 0 2 6 4 5 3 1 & 3 4 2 1 5 \\  
        2 & 6 5 1 0 2 4 3 & 1 5 2 3 4 \\  
        3 & 0 2 6 1 5 3 4 & 5 4 3 1 2 \\  
        4 & 0 6 5 1 3 4 2 & 4 5 1 2 3 \\  
        5 & 0 1 2 6 3 5 4 & 5 1 3 2 4 \\  
        6 & 0 5 4 3 1 6 2 & 5 1 4 3 2 \\  
        7 & 0 5 6 4 1 3 2 & 1 5 4 2 3 \\  
        8 & 0 5 6 1 2 4 3 & 5 1 4 3 2 \\  
        9 & 0 1 6 2 5 4 3 & 5 1 4 3 2 \\  
        10 & 0 6 1 5 2 4 3 & 5 1 4 3 2 \\  
        11 & 0 1 5 6 4 3 2 & 5 1 4 2 3 \\  
        12 & 0 5 4 6 1 2 3 & 5 1 3 2 4 \\  
        13 & 5 0 6 4 1 2 3 & 5 1 4 3 2 \\  
        14 & 0 5 6 4 1 2 3 & 5 1 2 4 3 \\  
        15 & 6 0 5 1 4 2 3 & 5 1 4 3 2 \\  
        16 & 0 5 6 1 2 4 3 & 5 1 4 3 2 \\  
        17 & 6 0 5 2 1 4 3 & 5 1 4 2 3 \\  
        18 & 0 5 6 1 3 4 2 & 5 1 4 2 3 \\  
        19 & 5 6 0 1 2 3 4 & 5 1 4 2 3 \\  
        
        \hline
    \end{tabular}
    \label{tab-importance_sd_sdxl_fruit_appx}
\end{table}

\paragraph{Voting Score}

The voting scores for 2-step-inference SD-Turbo and SDXL-Turbo, as well as for 20-step-inference SD v2.1 and SDXL, are listed in Tab.~\ref{tab-voting_score_sdturbo_sdxlturbo_fruit_appx} and Tab.~\ref{tab-voting_score_sd_sdxl_fruit_appx}. respectively. 
The corresponding bar charts are shown in Fig.~\ref{tab-bar_chart_voting_score-sdturbo}, Fig.~\ref{tab-bar_chart_voting_score-sdturbo}, Fig.~\ref{tab-bar_chart_voting_score-sd} and Fig.~\ref{tab-bar_chart_voting_score-sdxl}, respectively.

The bar charts more effectively illustrate the dynamic changes in the roles of the Transformer blocks throughout the denoising process. 
Overall, the importance of the blocks generally follows a trend of being higher in the middle (i.e., the bottleneck) and lower at the ends, particularly in multi-step inference (e.g., SD v2.1 and SDXL). 
Additionally, it can be observed that, the importance of structurally symmetric blocks always exhibits significant disparities. 

% 2 步 SD-Turbo/SDXL-Turbo 投票得分
\begin{table}[h]
    \centering
    \caption{
        Dynamic voting score of 2-step SD-Turbo/SDXL-Turbo U-Net, arranged in non-descending order. 
    }
    \begin{tabular}{c | c : c}
        \hline
        \multirow{2}{*}{\textbf{Step}} & 
        \multicolumn{2}{c}{\textbf{Voting Score}} \\

        ~ & SD-Turbo & SDXL-Turbo \\
        \hline

        0 & 26 37 58 87 62 78 72 & 26 39 53 59 48 \\ 
        1 & 40 39 66 84 65 53 73 & 28 40 70 45 42 \\ 

        \hline
    \end{tabular}
    \label{tab-voting_score_sdturbo_sdxlturbo_fruit_appx}
\end{table}

% 20 步 SD/SDXL 投票得分
\begin{table}[h]
    \centering
    \caption{
        Dynamic voting score of 20-step SD v2.1/SDXL U-Net, arranged in non-descending order. 
    }
    \begin{tabular}{c | c : c}
        \hline
        \multirow{2}{*}{\textbf{Step}} & 
        \multicolumn{2}{c}{\textbf{Voting Score}} \\

        ~ & SD v2.1 & SDXL \\
        \hline

        0 & 62 65 53 59 63 69 49 & 52 46 47 41 39 \\ 
        1 & 43 76 54 66 59 65 57 & 48 47 41 41 48 \\  
        2 & 57 53 63 82 70 49 46 & 40 45 47 50 43 \\  
        3 & 47 57 53 67 78 62 56 & 46 58 45 45 31 \\  
        4 & 44 58 76 63 70 55 54 & 45 51 52 36 41 \\  
        5 & 32 49 56 66 81 72 64 & 39 52 45 53 36 \\  
        6 & 32 64 72 63 62 61 66 & 40 56 49 48 32 \\  
        7 & 35 64 81 81 64 47 48 & 35 46 60 43 41 \\  
        8 & 40 57 60 86 69 54 54 & 41 54 53 42 35 \\  
        9 & 36 48 59 79 78 62 58 & 38 59 51 50 27 \\  
        10 & 41 56 61 79 72 57 54 & 37 62 53 47 26 \\  
        11 & 39 51 77 68 64 59 62 & 34 55 55 55 26 \\  
        12 & 39 63 78 86 53 42 59 & 35 54 53 59 24 \\  
        13 & 46 59 77 83 59 40 56 & 36 59 54 50 26 \\  
        14 & 39 67 75 90 56 43 50 & 41 49 57 57 21 \\  
        15 & 40 60 80 84 70 51 35 & 39 58 57 49 22 \\  
        16 & 31 64 67 84 76 40 58 & 43 66 53 45 18 \\  
        17 & 48 66 60 85 69 49 43 & 36 60 62 46 21 \\  
        18 & 42 64 79 73 74 42 46 & 33 57 58 55 22 \\  
        19 & 48 66 72 80 86 34 34 & 37 56 57 54 21 \\  
        
        \hline
    \end{tabular}
    \label{tab-voting_score_sd_sdxl_fruit_appx}
\end{table}

% 2 步 SD-Turbo 投票得分柱状图
\begin{table}[h]
    \centering
    \begin{tabular}{c c}
        \includegraphics[width=0.45\linewidth]{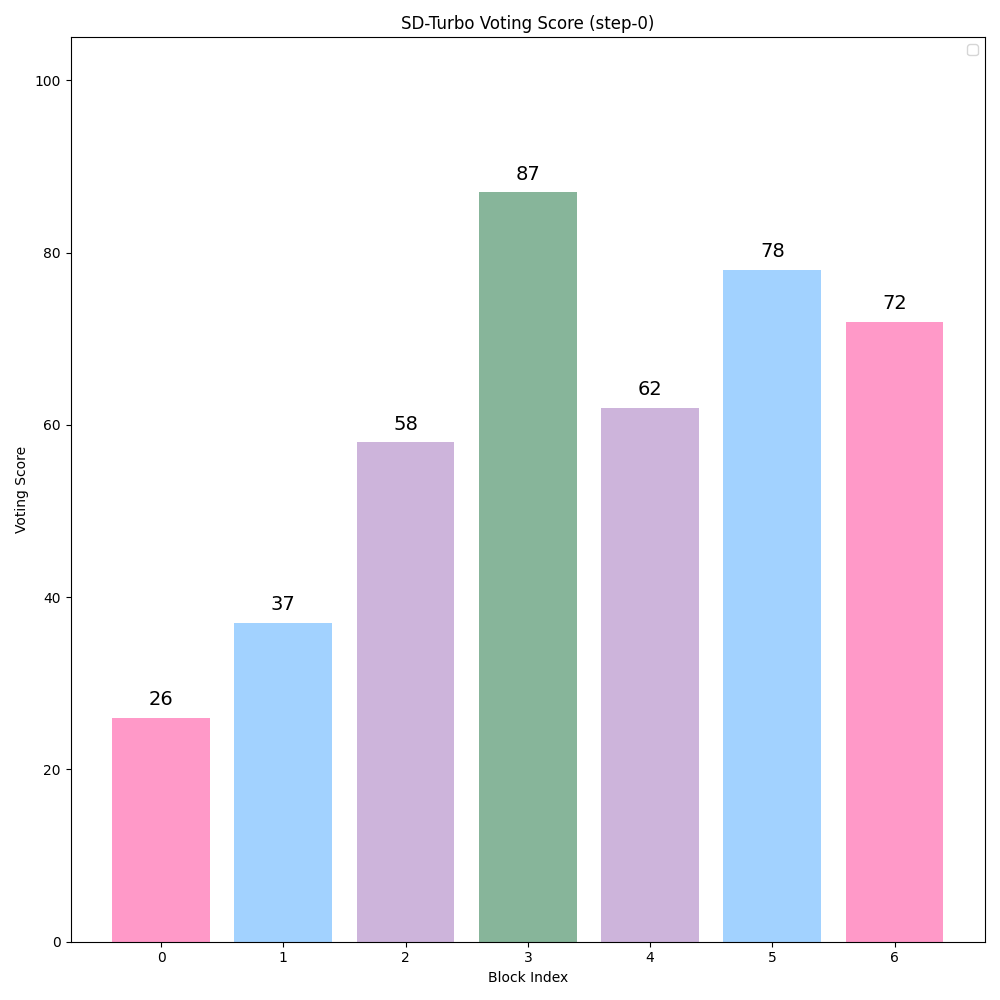} 
        & 
        \includegraphics[width=0.45\linewidth]{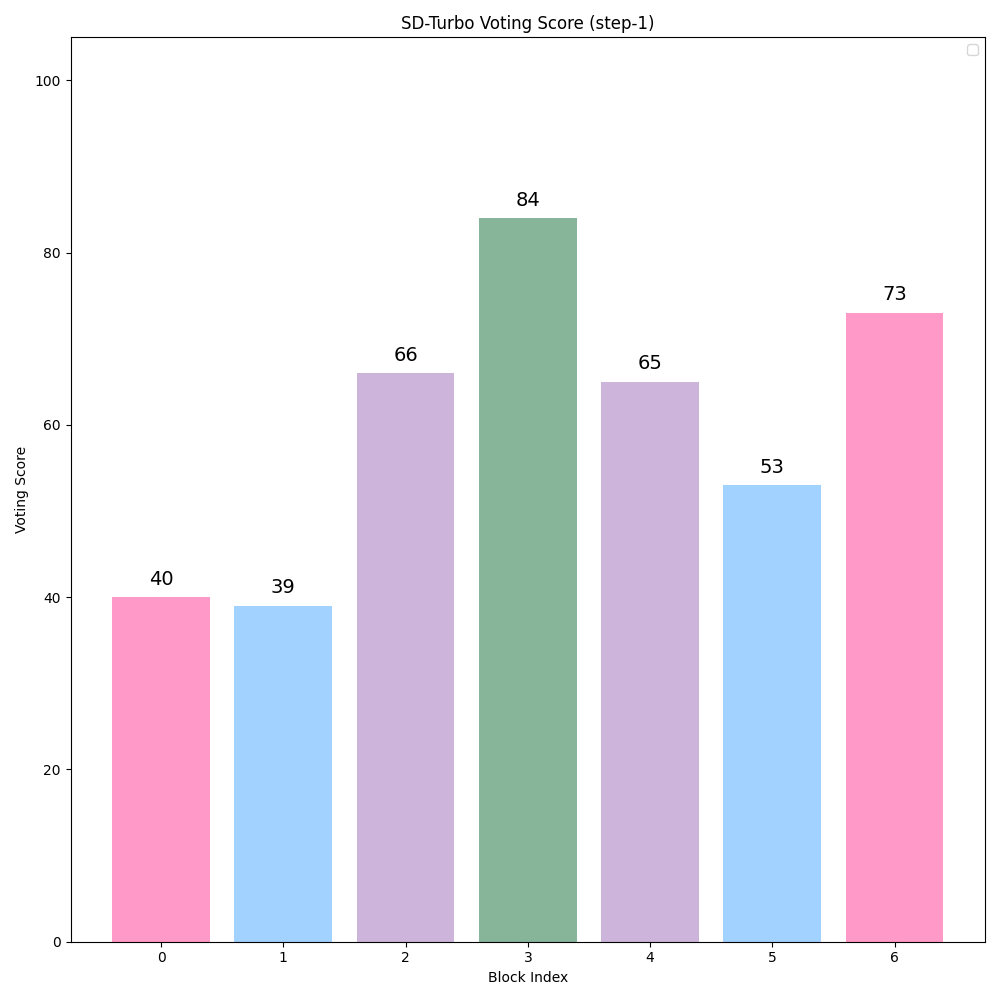}
    \end{tabular}
    \captionof{figure}{
        Bar charts of voting scores for SD-Turbo. 
    }
    \label{tab-bar_chart_voting_score-sdturbo}
\end{table}

% 2 步 SDXL-Turbo 投票得分柱状图
\begin{table}[h]
    \centering
    \begin{tabular}{c c}
        \includegraphics[width=0.45\linewidth]{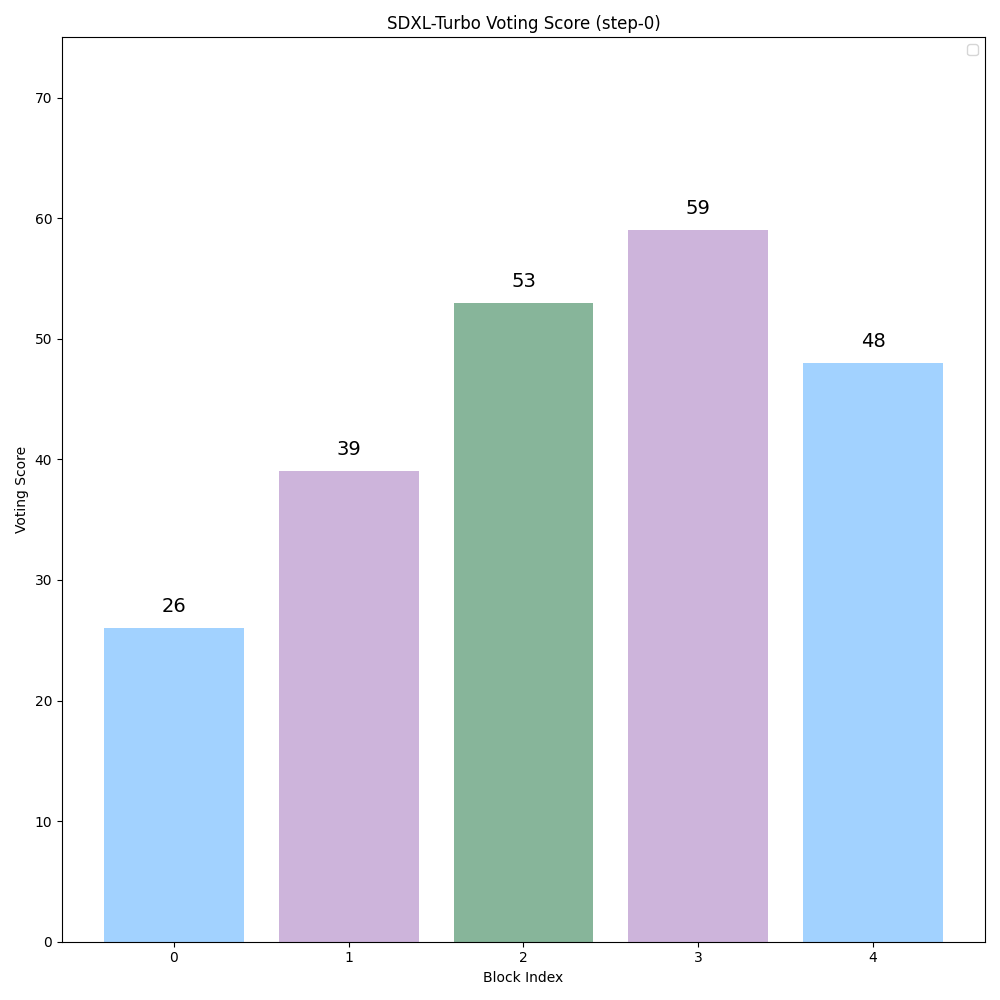} 
        & 
        \includegraphics[width=0.45\linewidth]{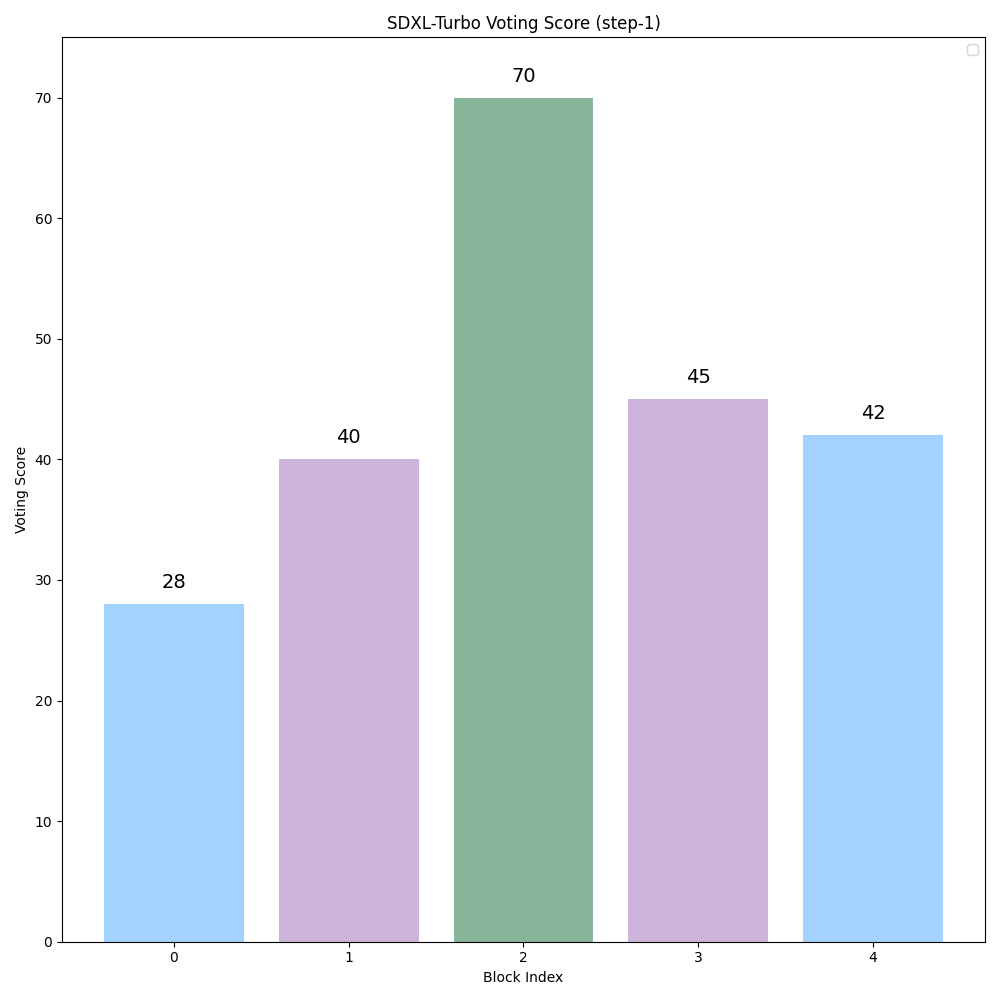}
    \end{tabular}
    \captionof{figure}{
        Bar charts of voting scores for SDXL-Turbo. 
    }
    \label{tab-bar_chart_voting_score-sdxlturbo}
\end{table}

% 20 步 SD 投票得分柱状图
\begin{table*}[h]
    \centering
    \begin{tabular}{c c c c c}
        \includegraphics[width=0.175\linewidth]{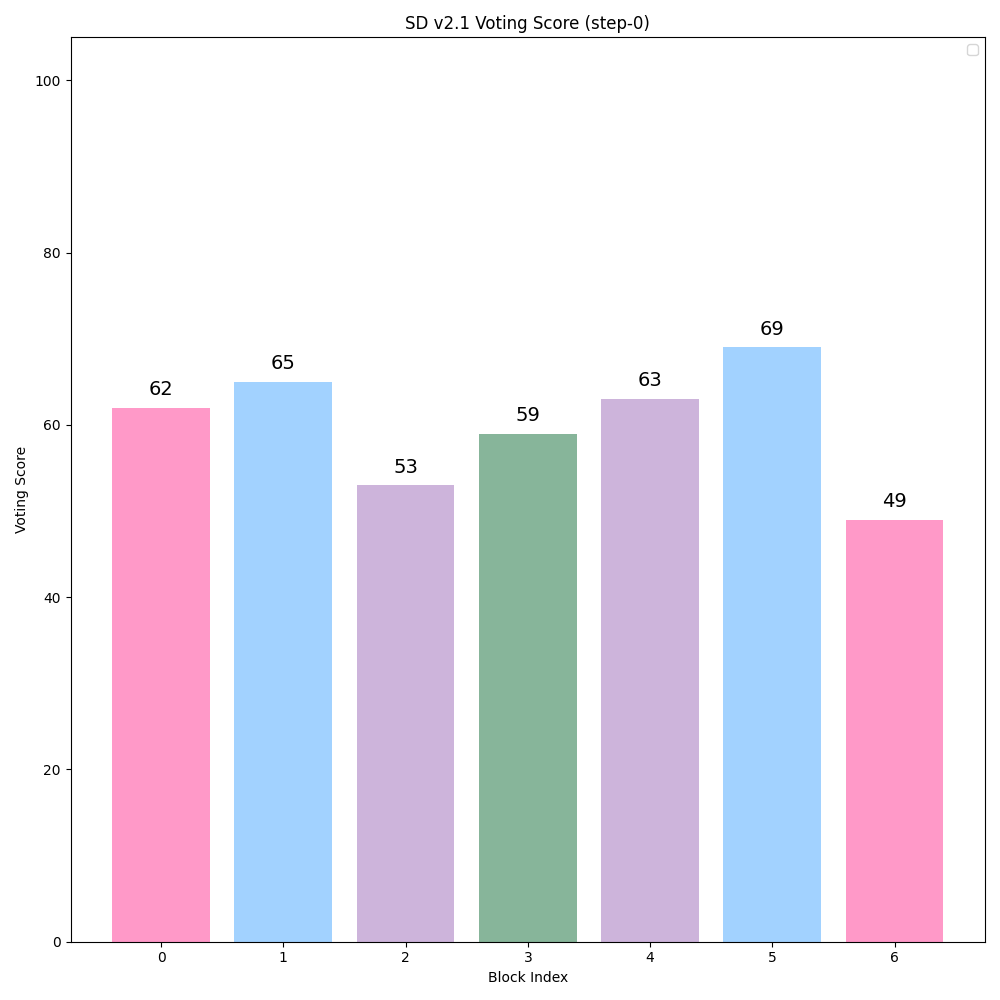} 
        & 
        \includegraphics[width=0.175\linewidth]{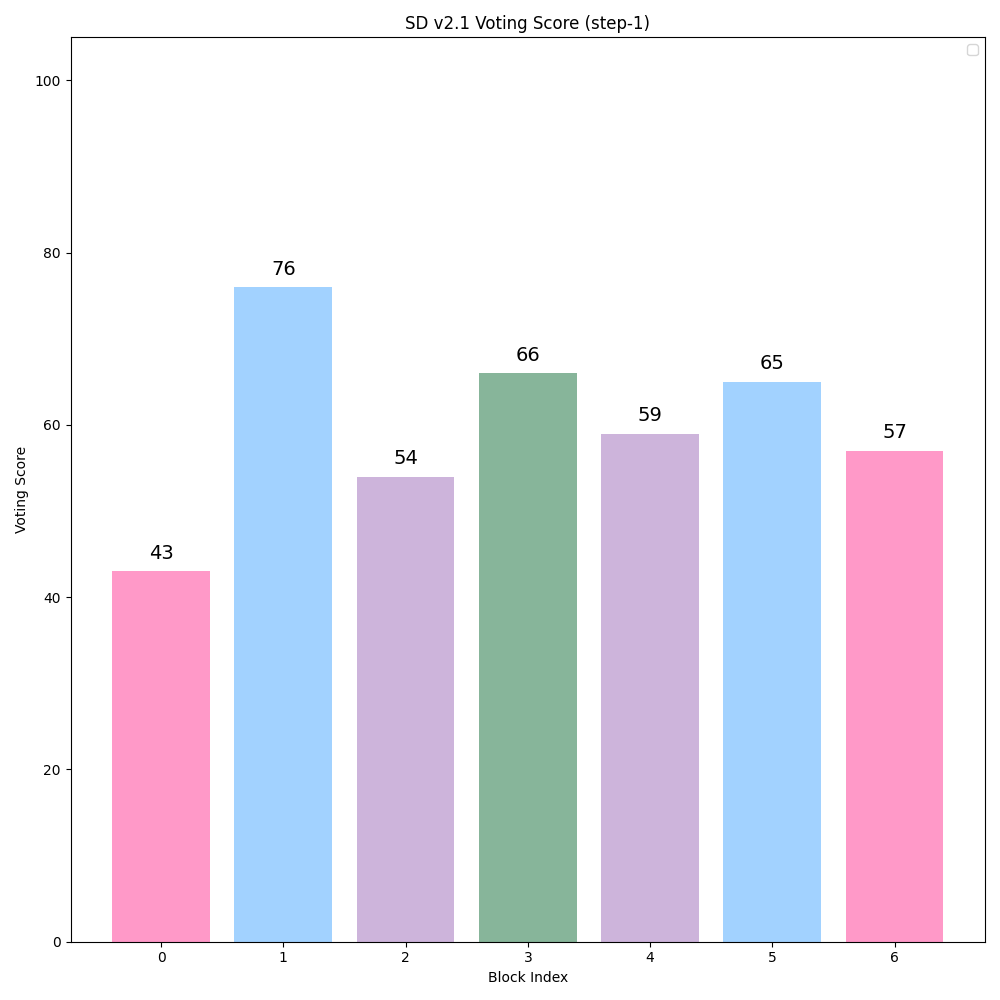}
        & 
        \includegraphics[width=0.175\linewidth]{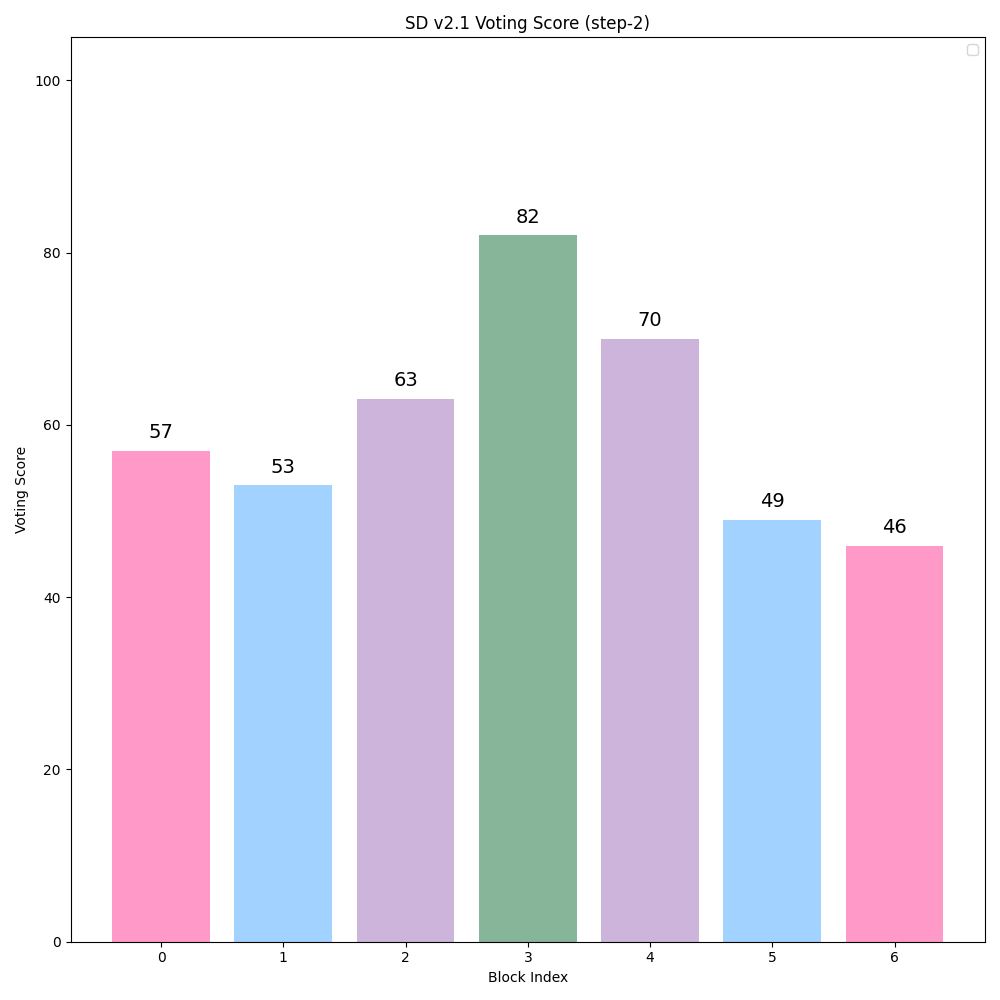}
        & 
        \includegraphics[width=0.175\linewidth]{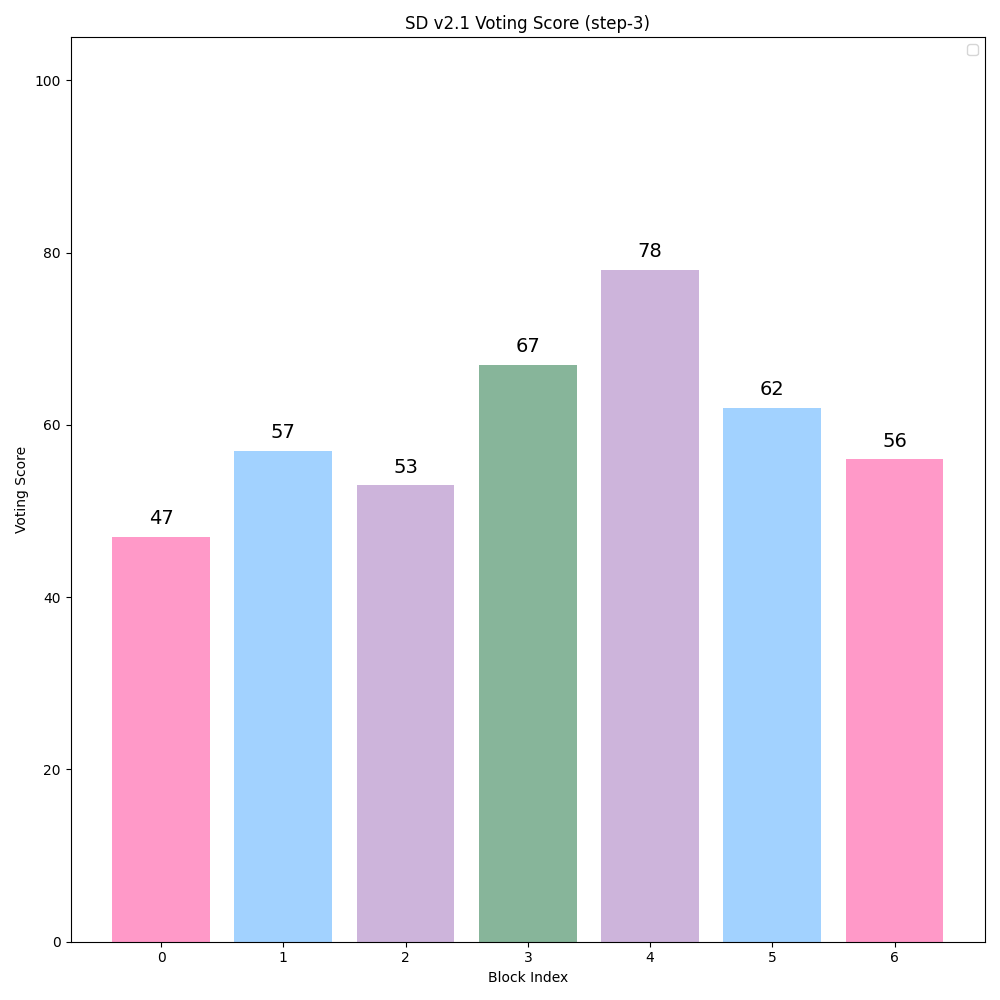}
        & 
        \includegraphics[width=0.175\linewidth]{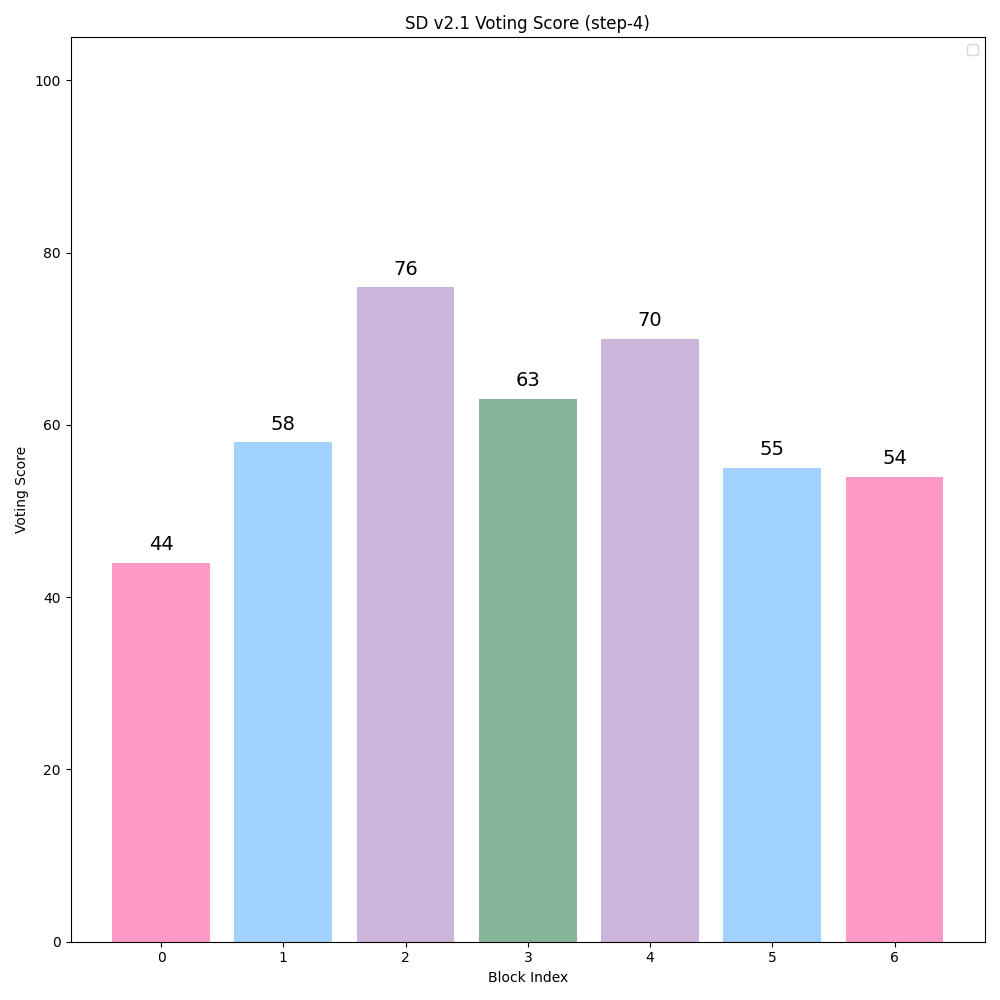}

        \\ 

        \includegraphics[width=0.175\linewidth]{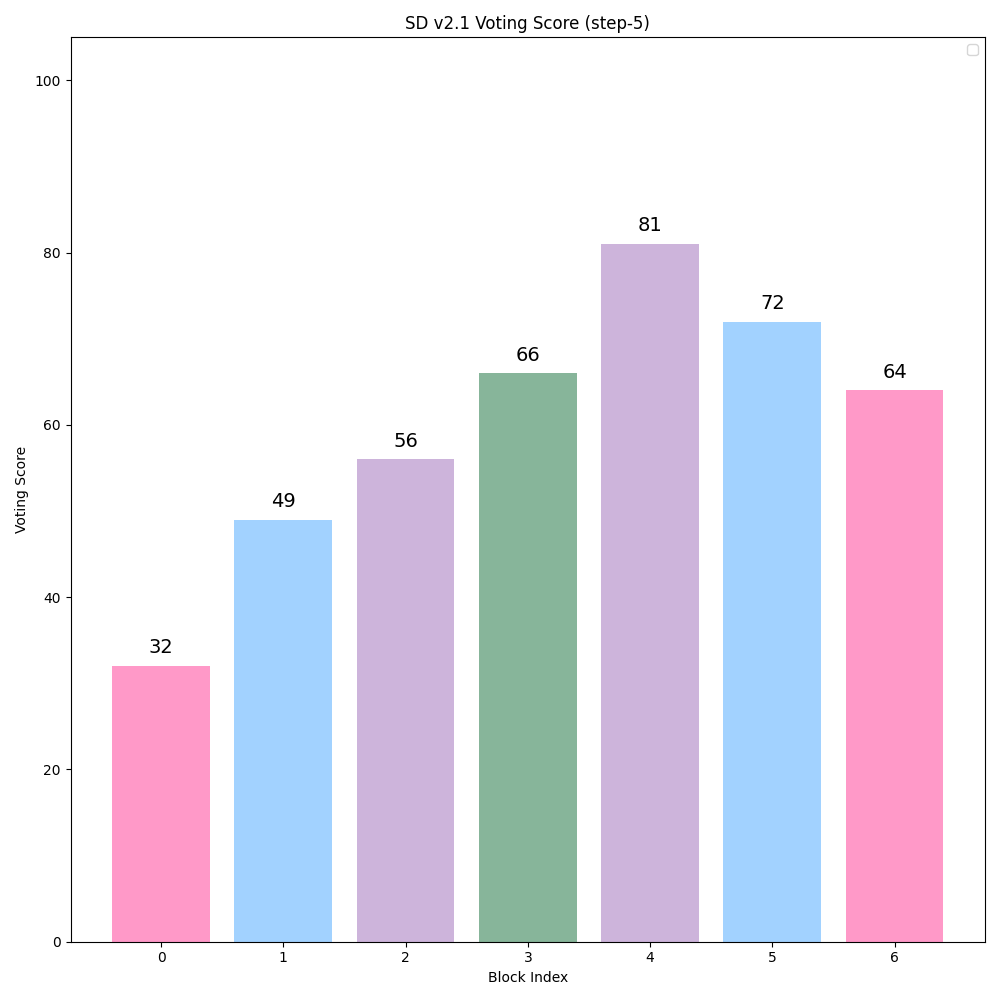} 
        & 
        \includegraphics[width=0.175\linewidth]{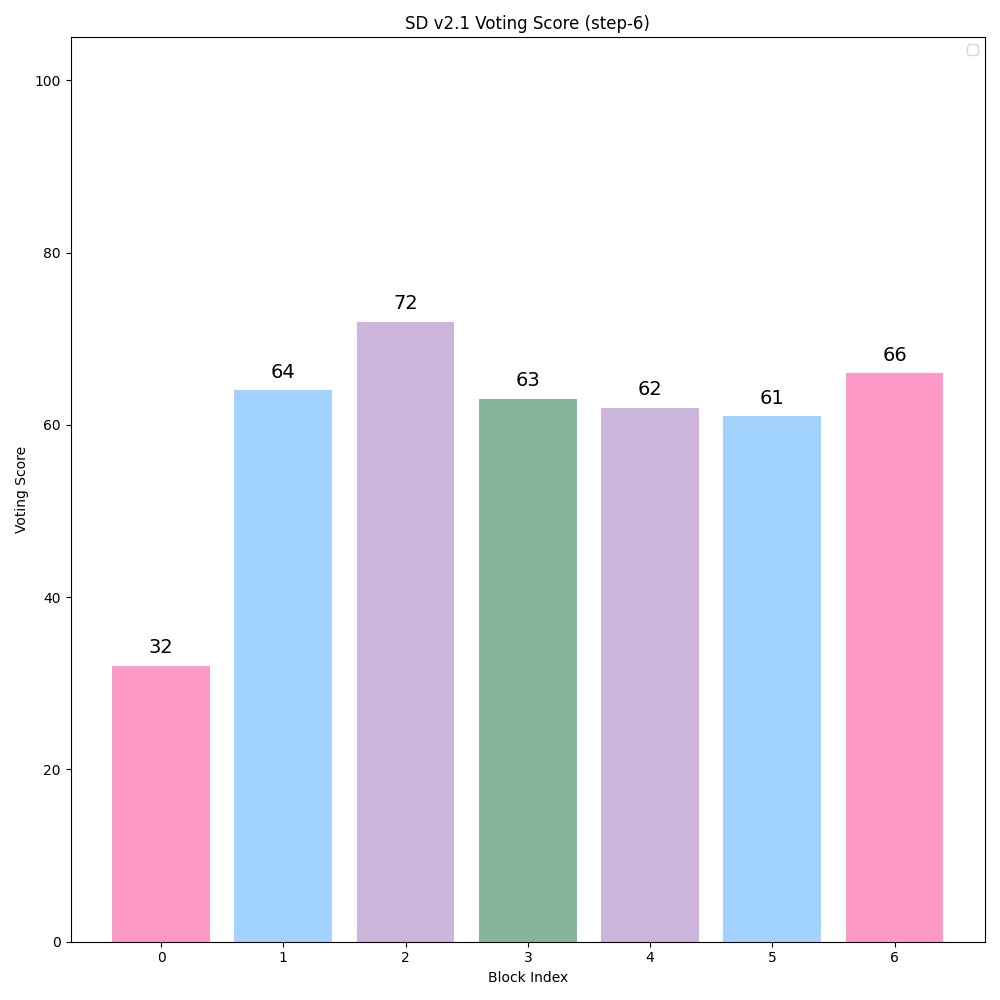}
        & 
        \includegraphics[width=0.175\linewidth]{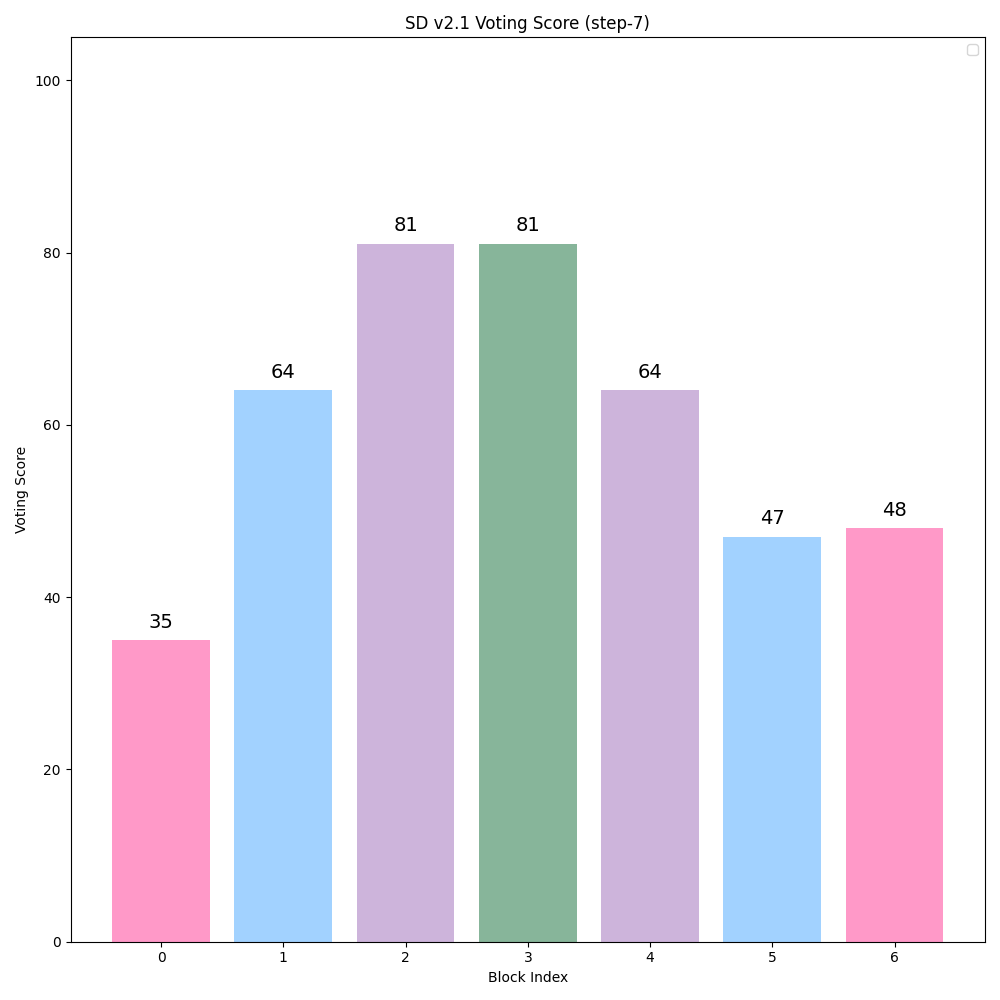}
        & 
        \includegraphics[width=0.175\linewidth]{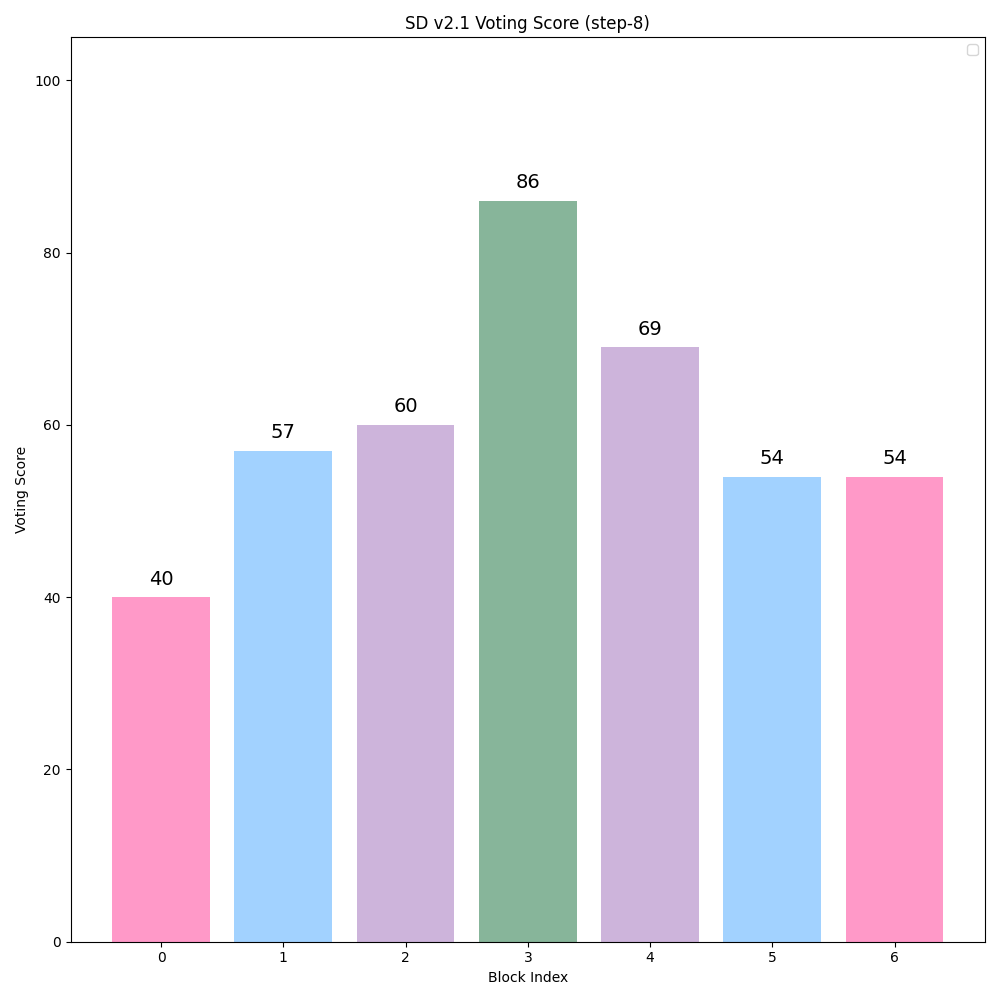}
        & 
        \includegraphics[width=0.175\linewidth]{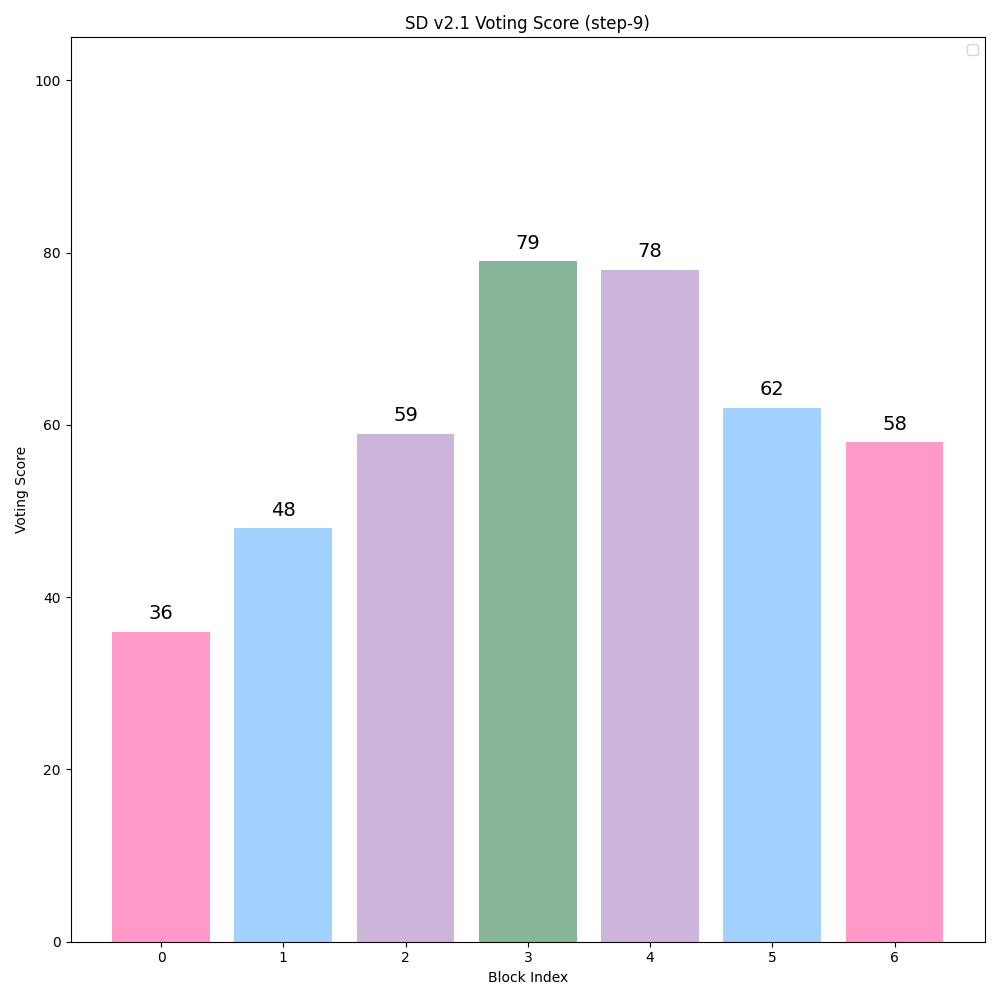}
        
        \\

        \includegraphics[width=0.175\linewidth]{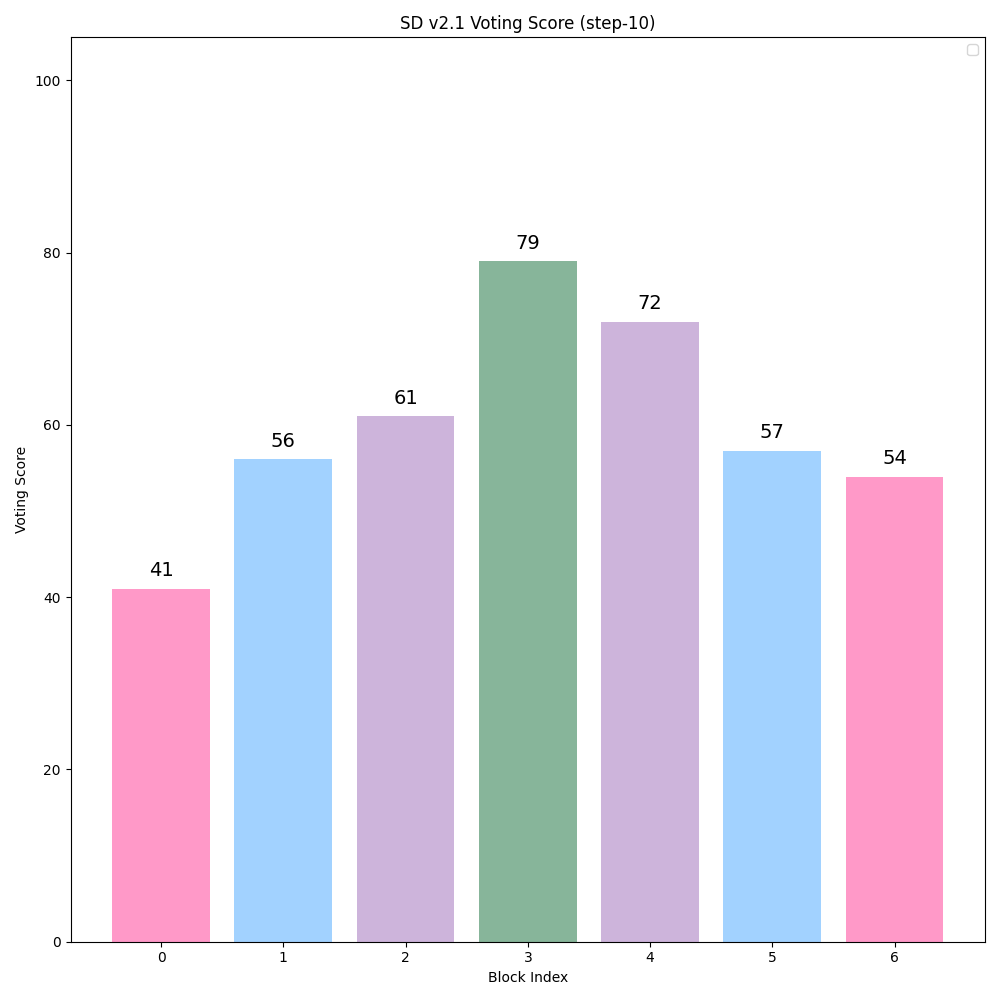} 
        & 
        \includegraphics[width=0.175\linewidth]{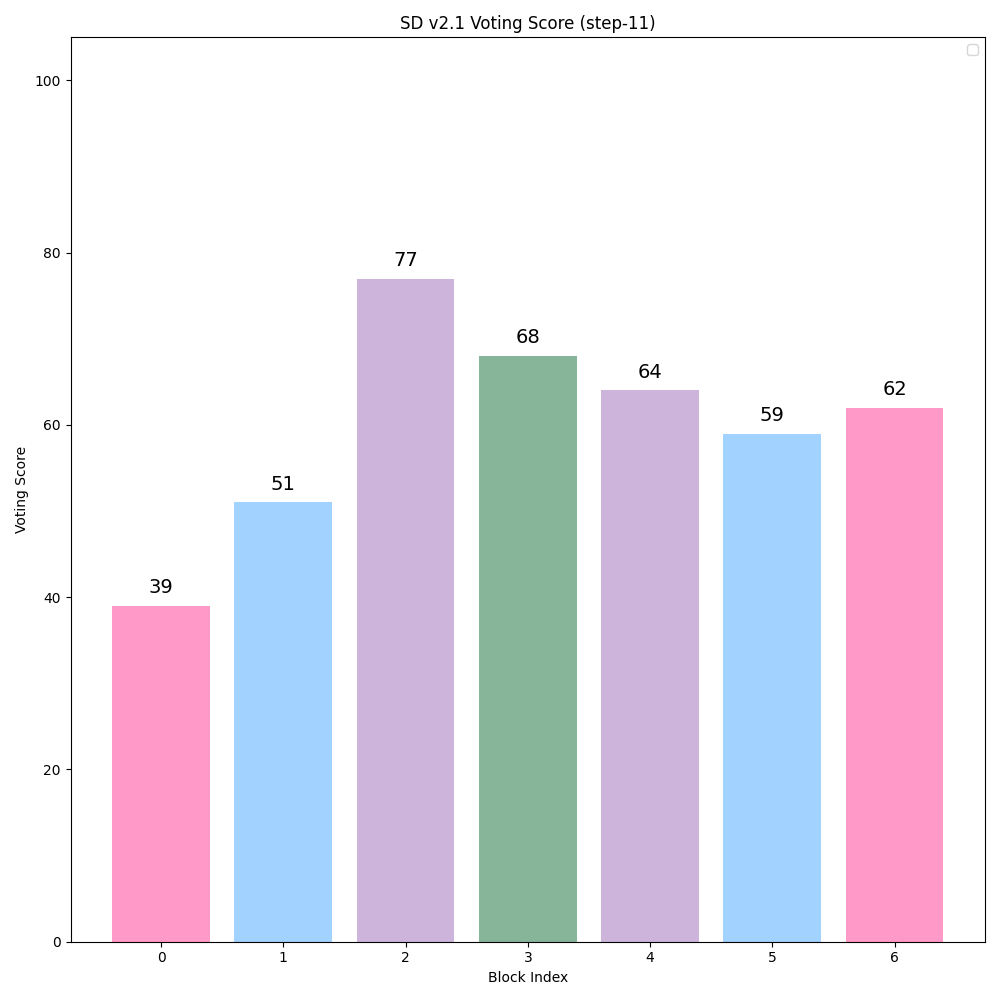}
        & 
        \includegraphics[width=0.175\linewidth]{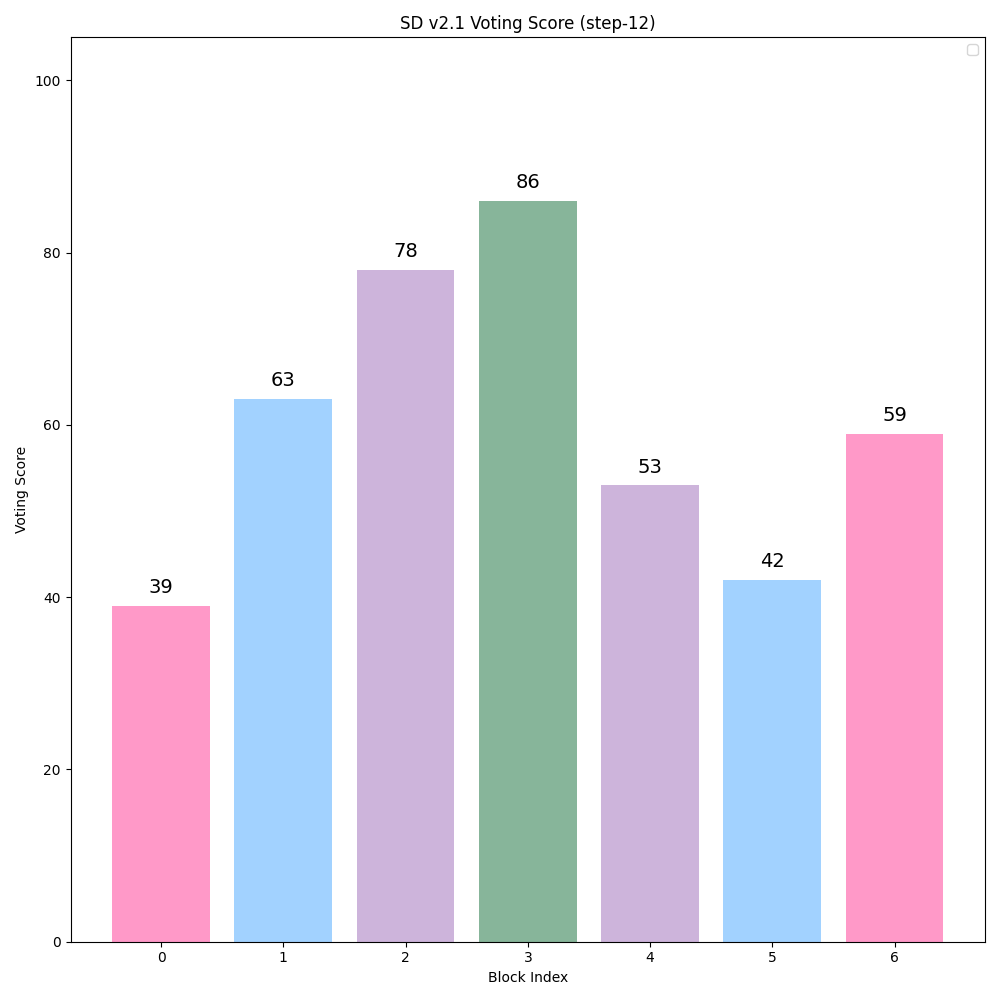}
        & 
        \includegraphics[width=0.175\linewidth]{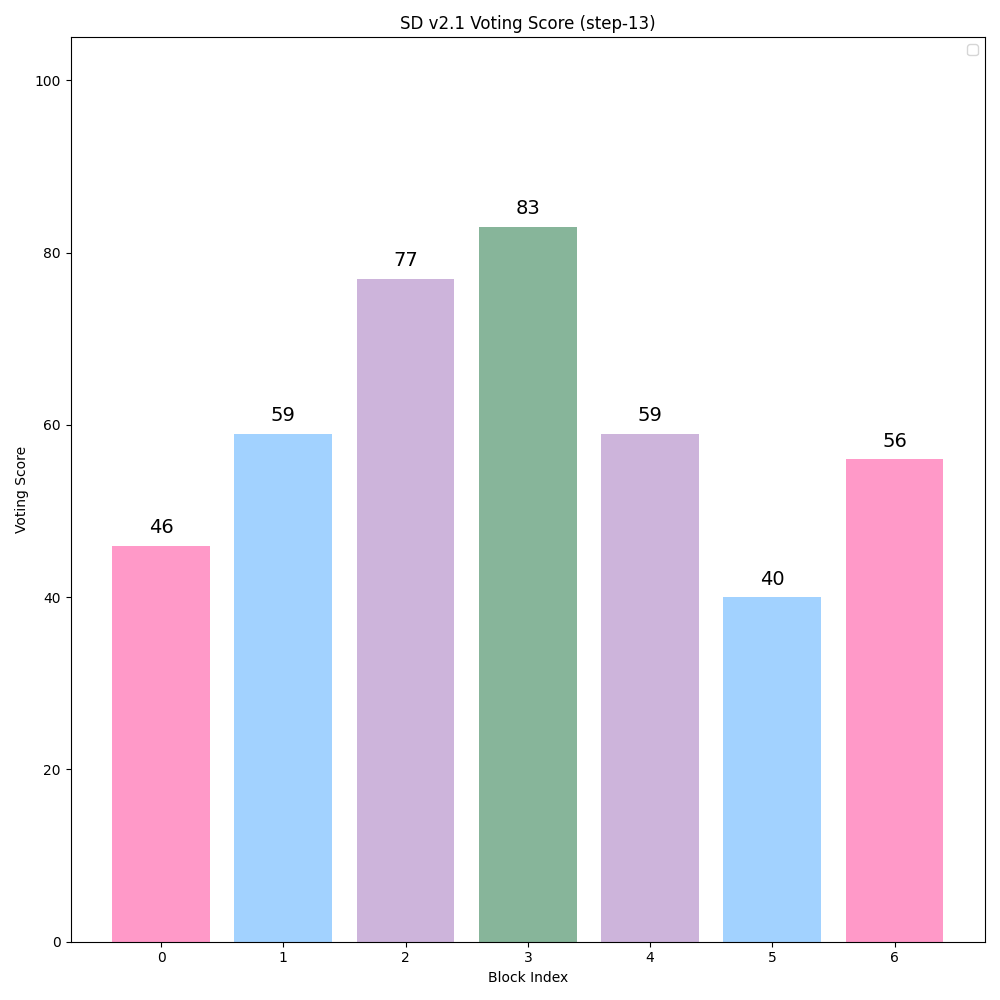}
        & 
        \includegraphics[width=0.175\linewidth]{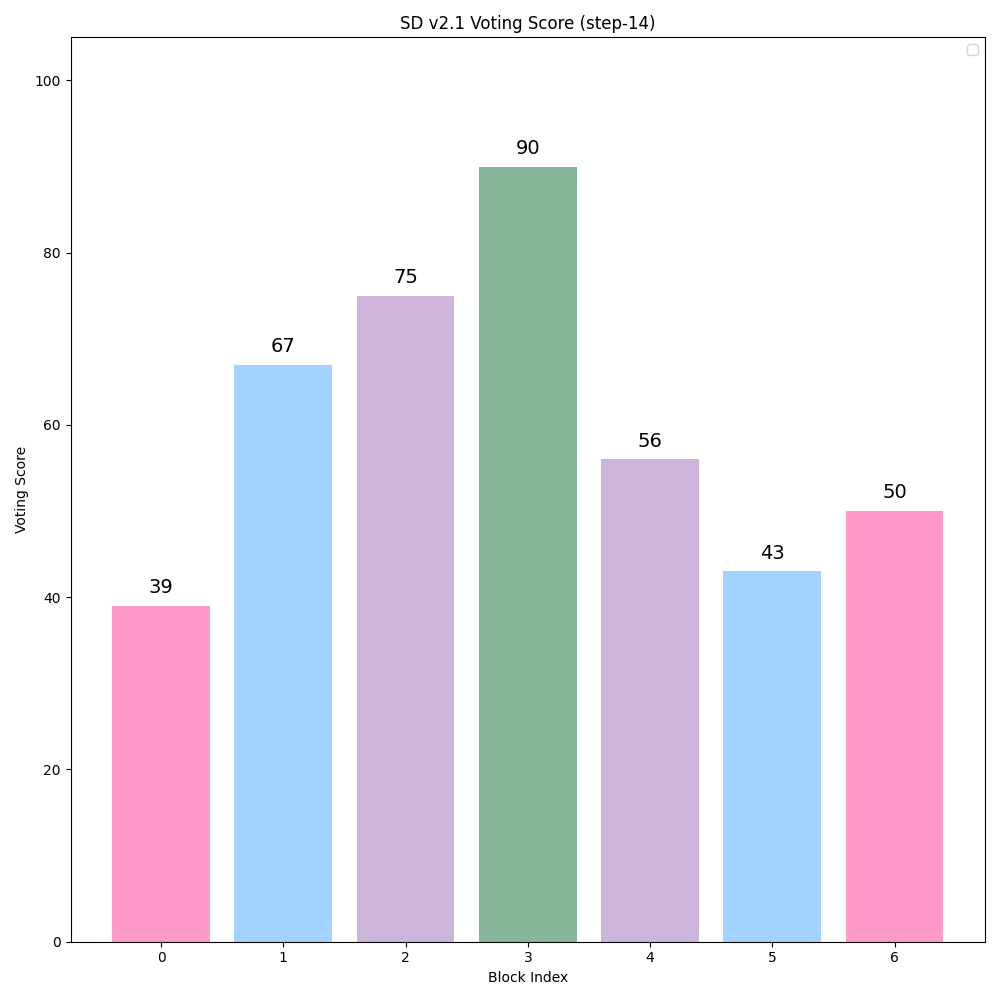}

        \\ 

        \includegraphics[width=0.175\linewidth]{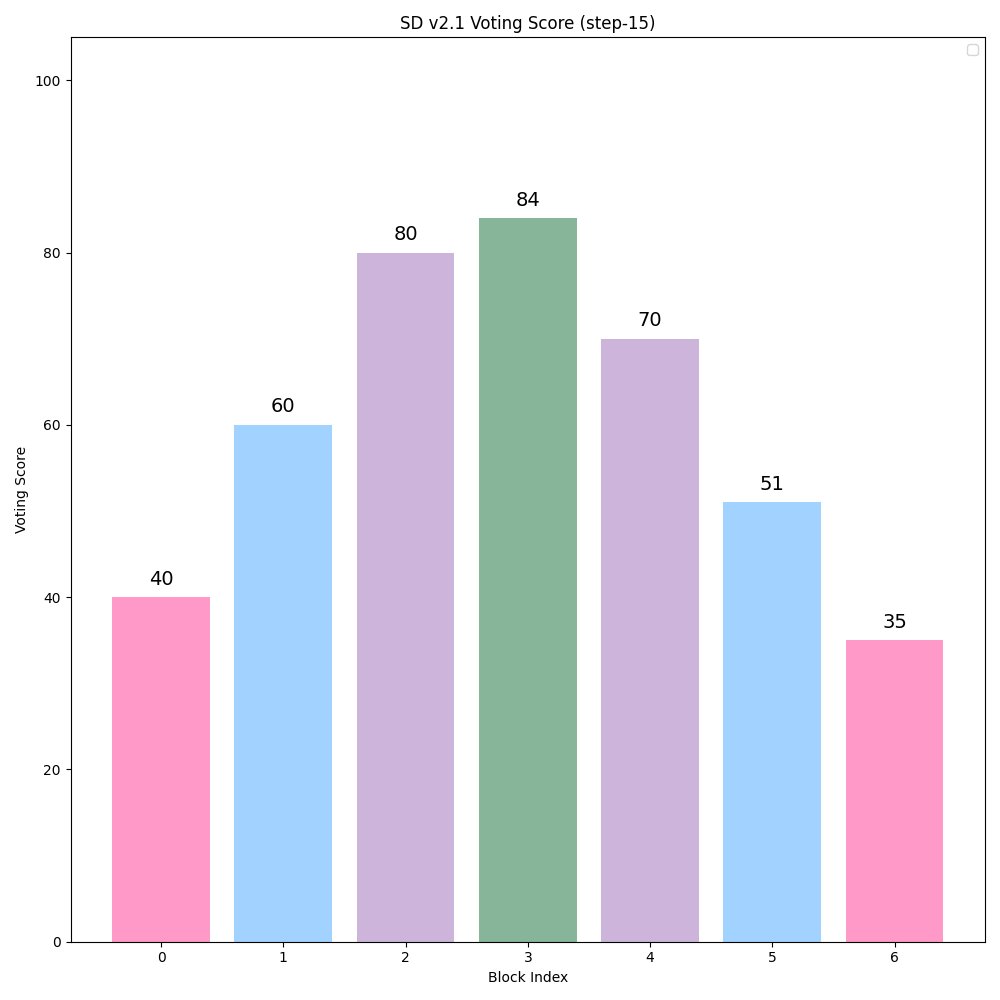} 
        & 
        \includegraphics[width=0.175\linewidth]{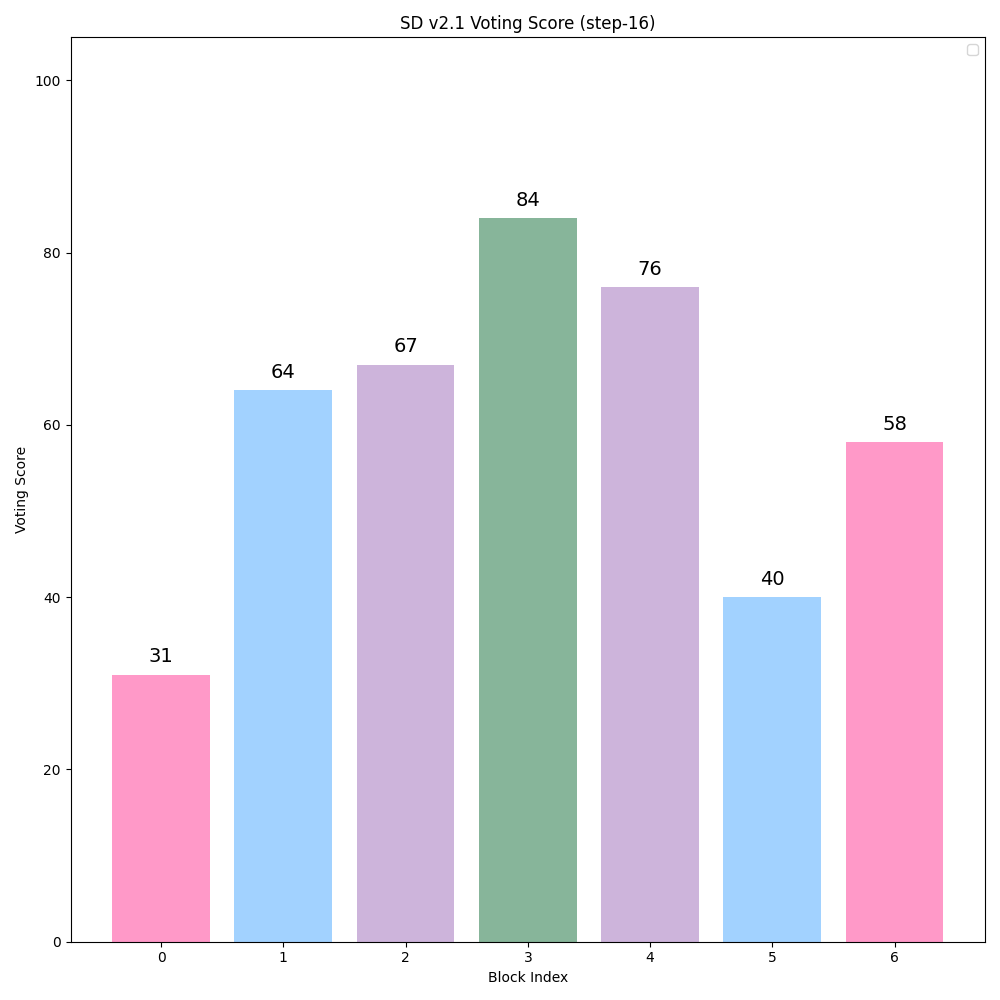}
        & 
        \includegraphics[width=0.175\linewidth]{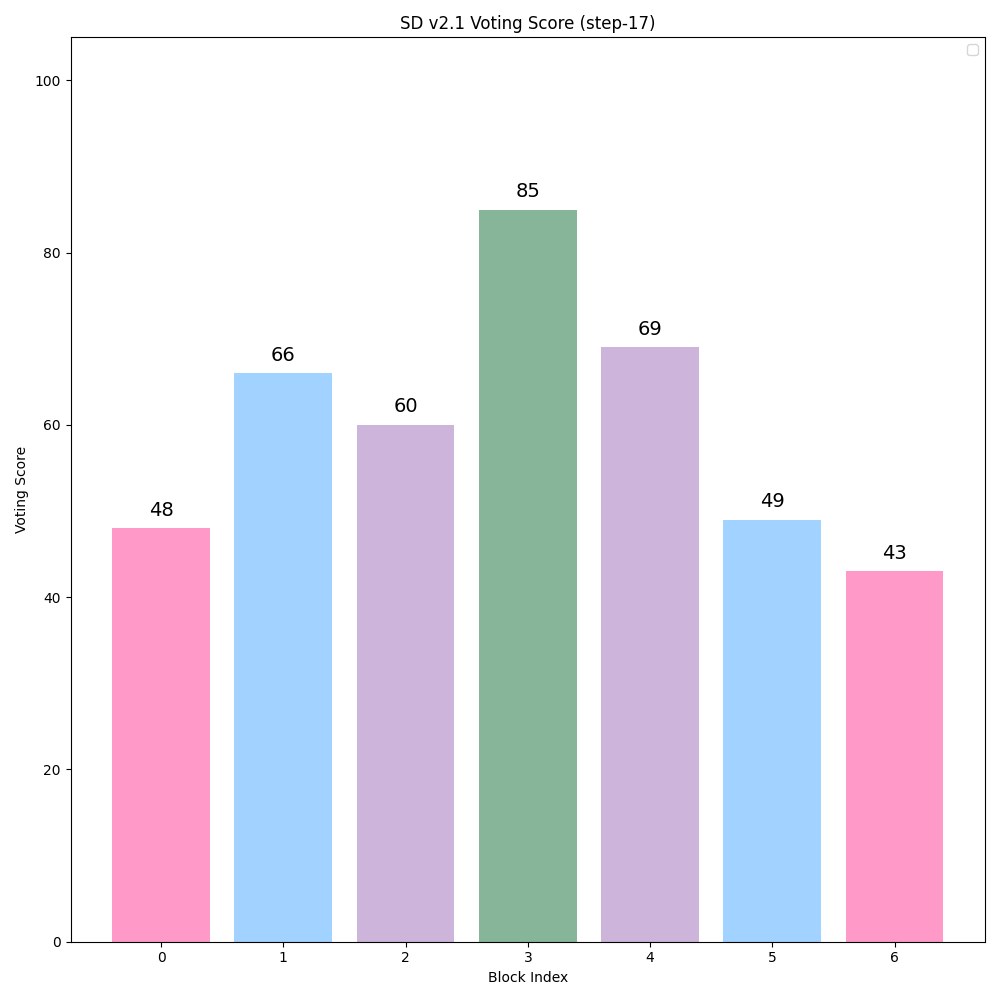}
        & 
        \includegraphics[width=0.175\linewidth]{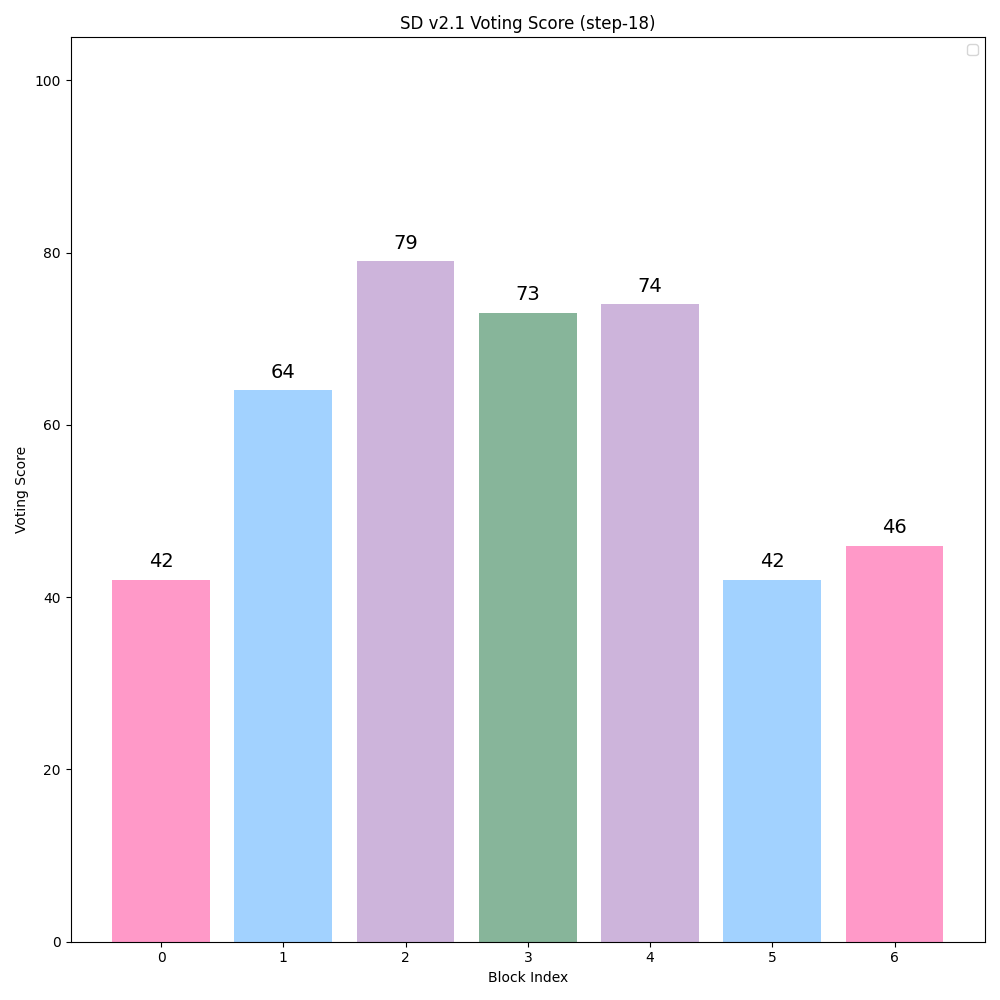}
        & 
        \includegraphics[width=0.175\linewidth]{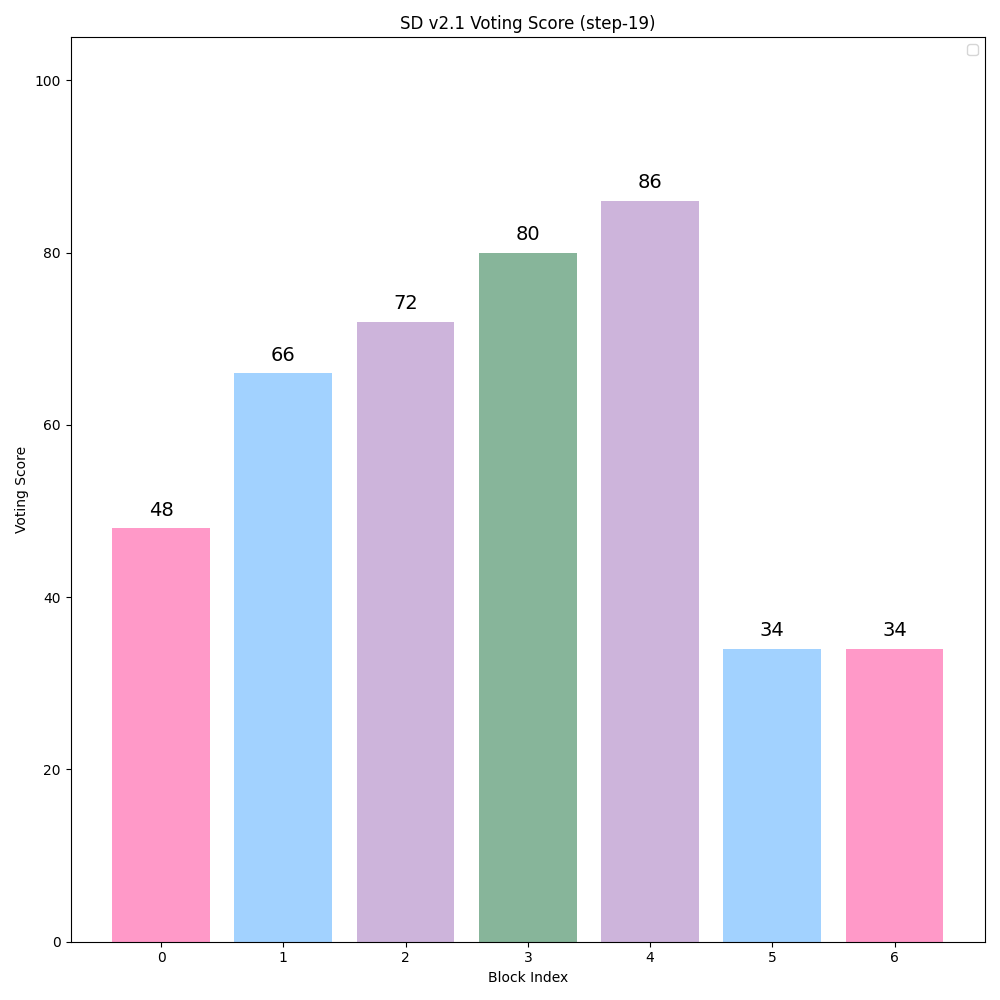}
    \end{tabular}
    \captionof{figure}{
        Bar charts of voting scores for SD v2.1. 
    }
    \label{tab-bar_chart_voting_score-sd}
\end{table*}

% 20 步 SDXL 投票得分柱状图
\begin{table*}[h]
    \centering
    \begin{tabular}{c c c c c}
        \includegraphics[width=0.175\linewidth]{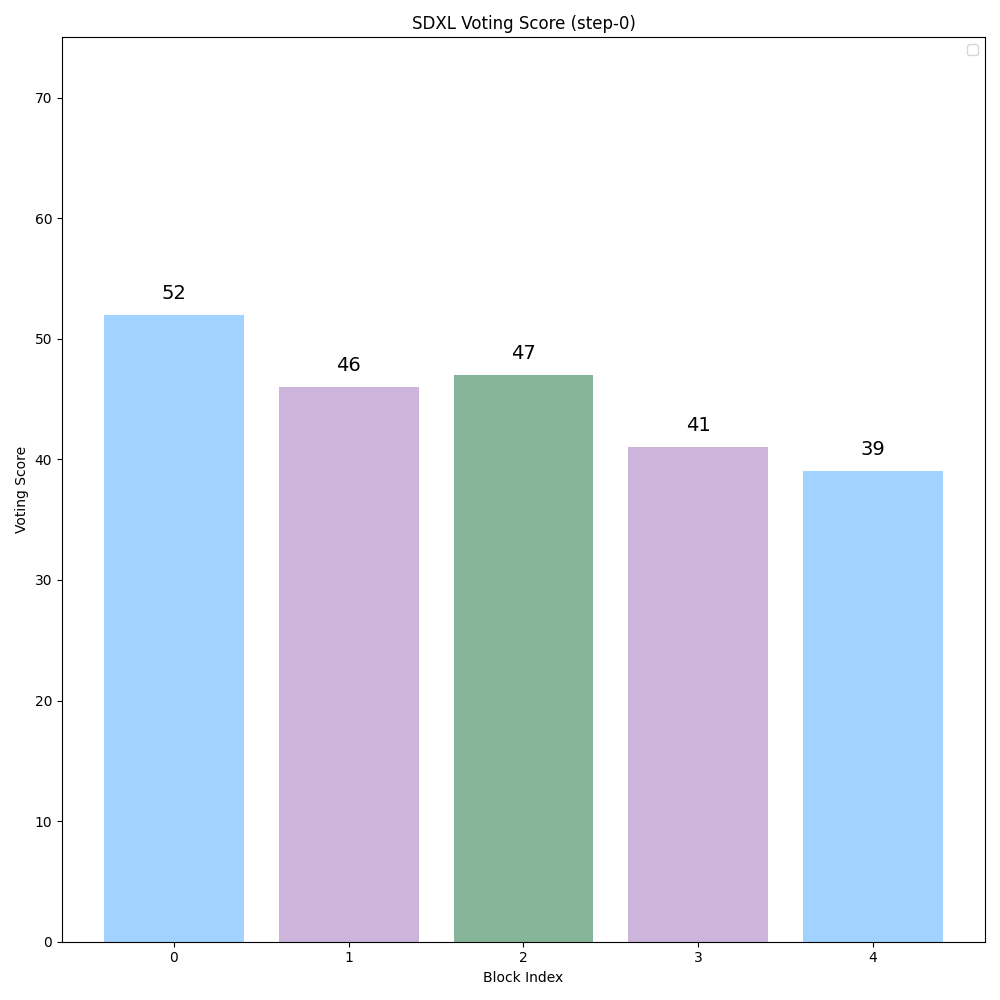} 
        & 
        \includegraphics[width=0.175\linewidth]{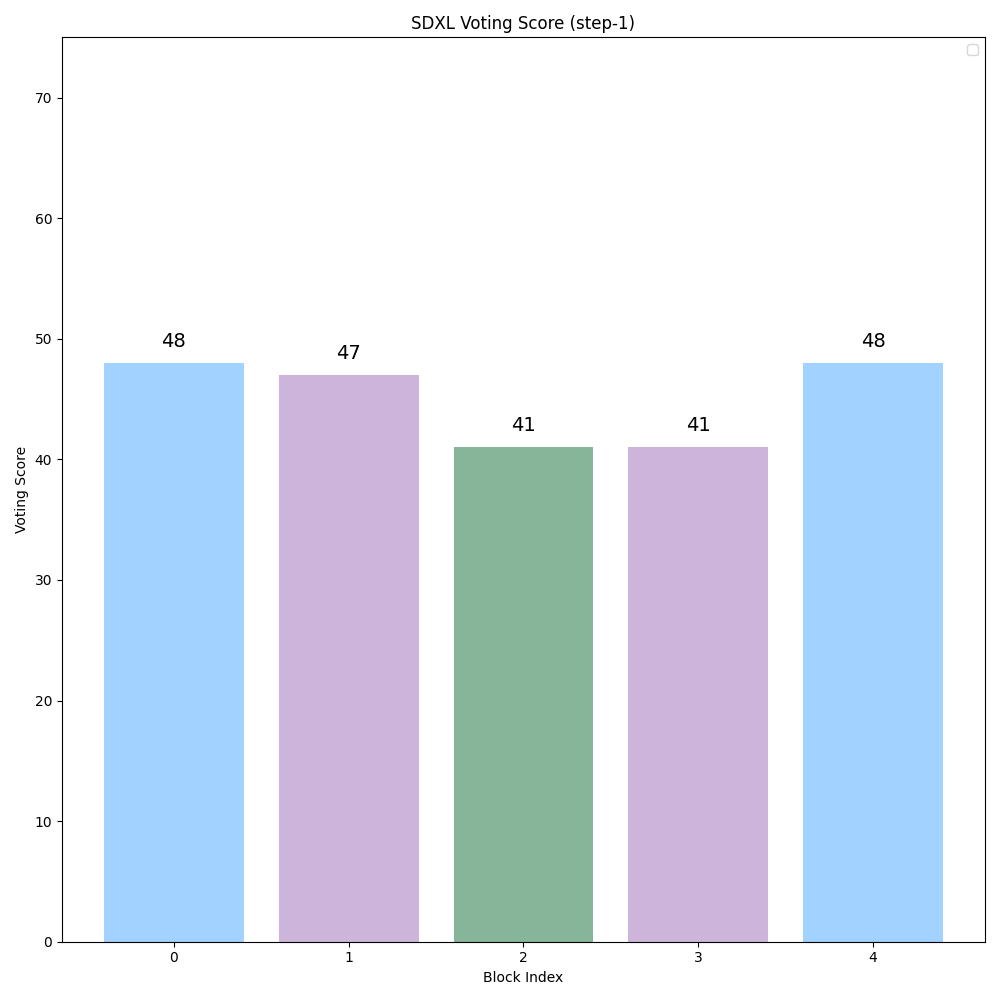}
        & 
        \includegraphics[width=0.175\linewidth]{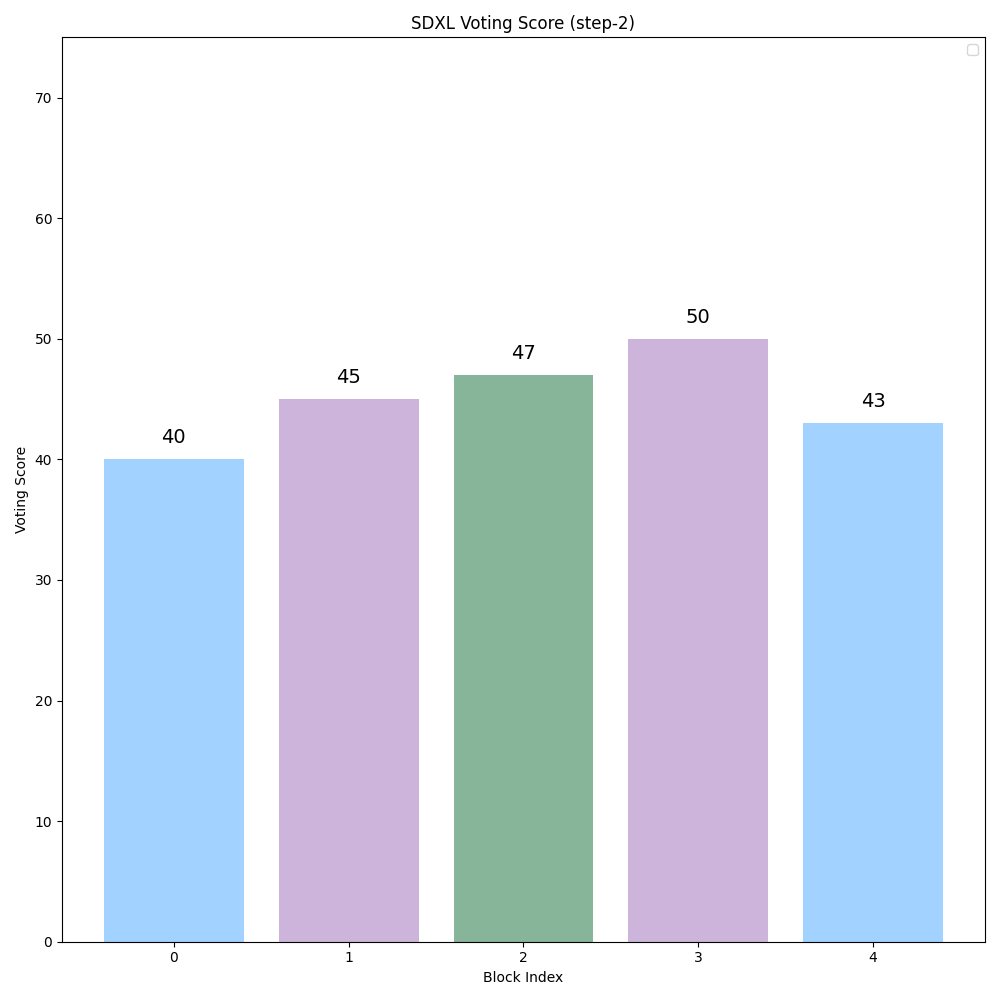}
        & 
        \includegraphics[width=0.175\linewidth]{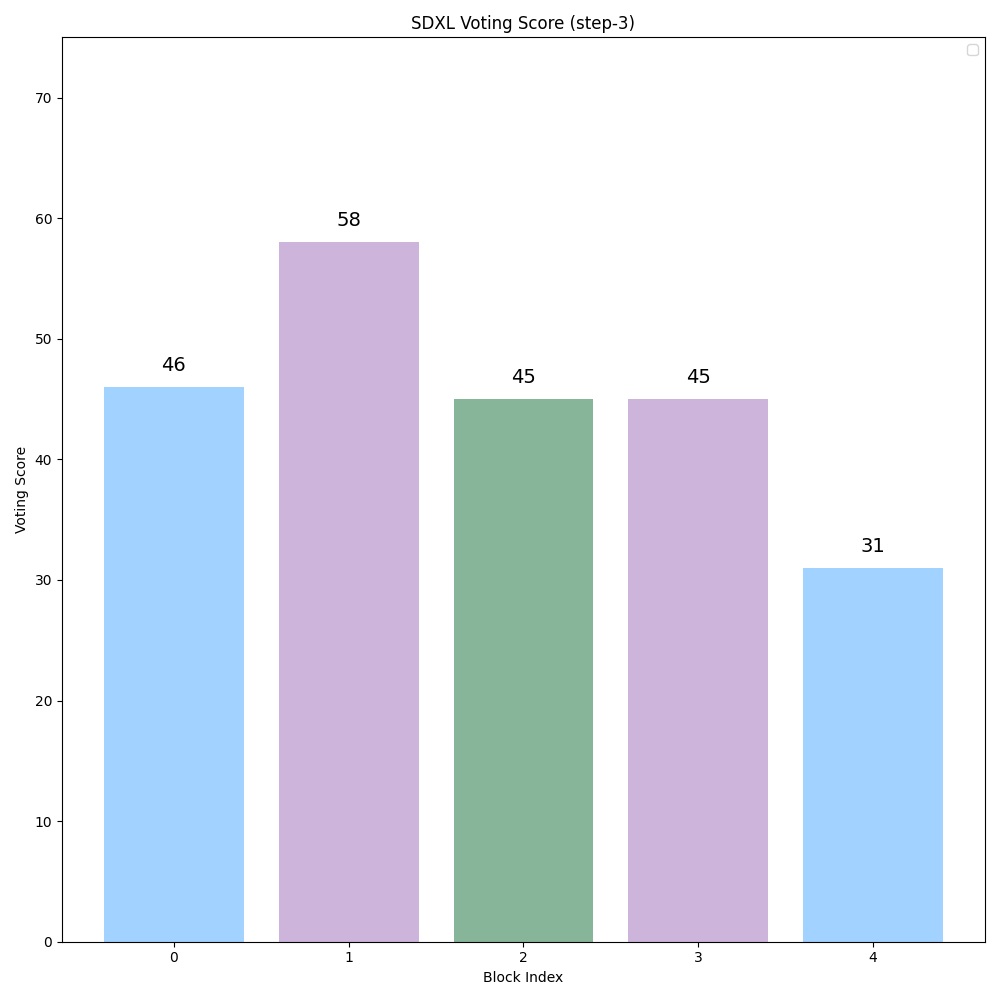}
        & 
        \includegraphics[width=0.175\linewidth]{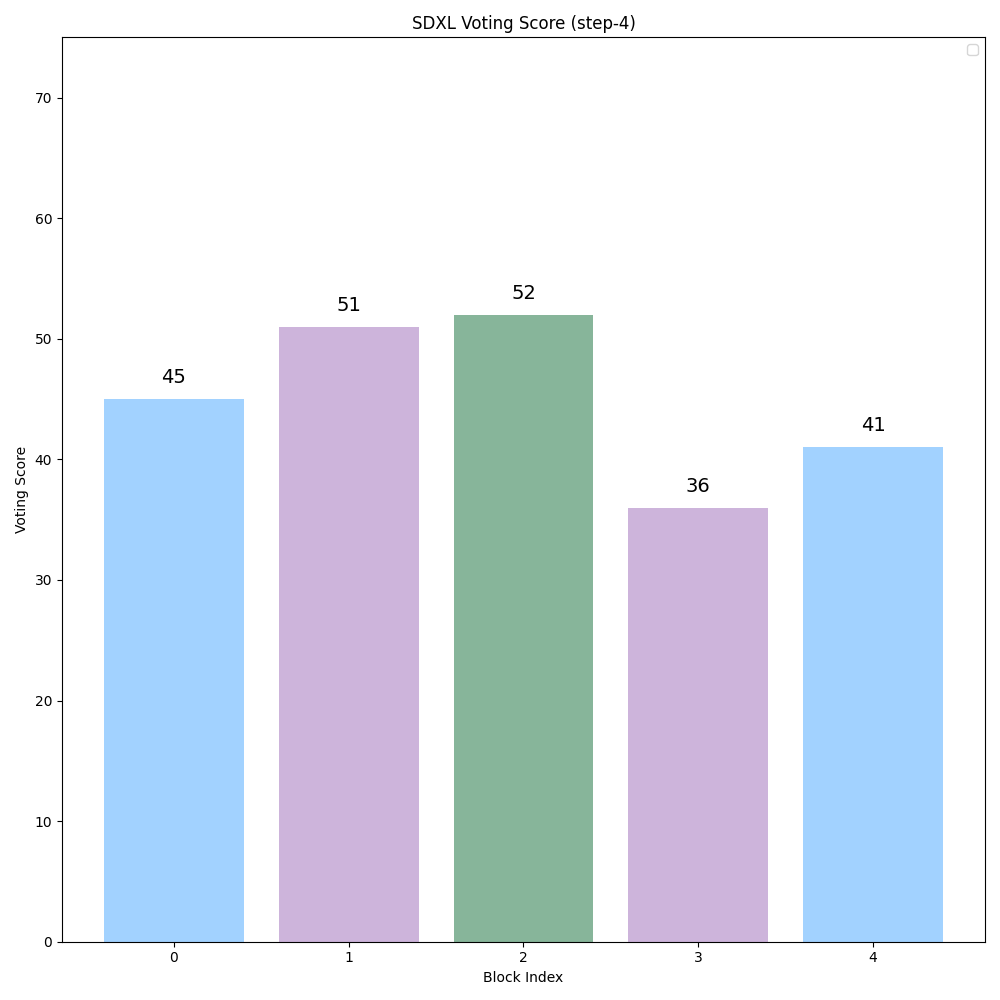}

        \\ 

        \includegraphics[width=0.175\linewidth]{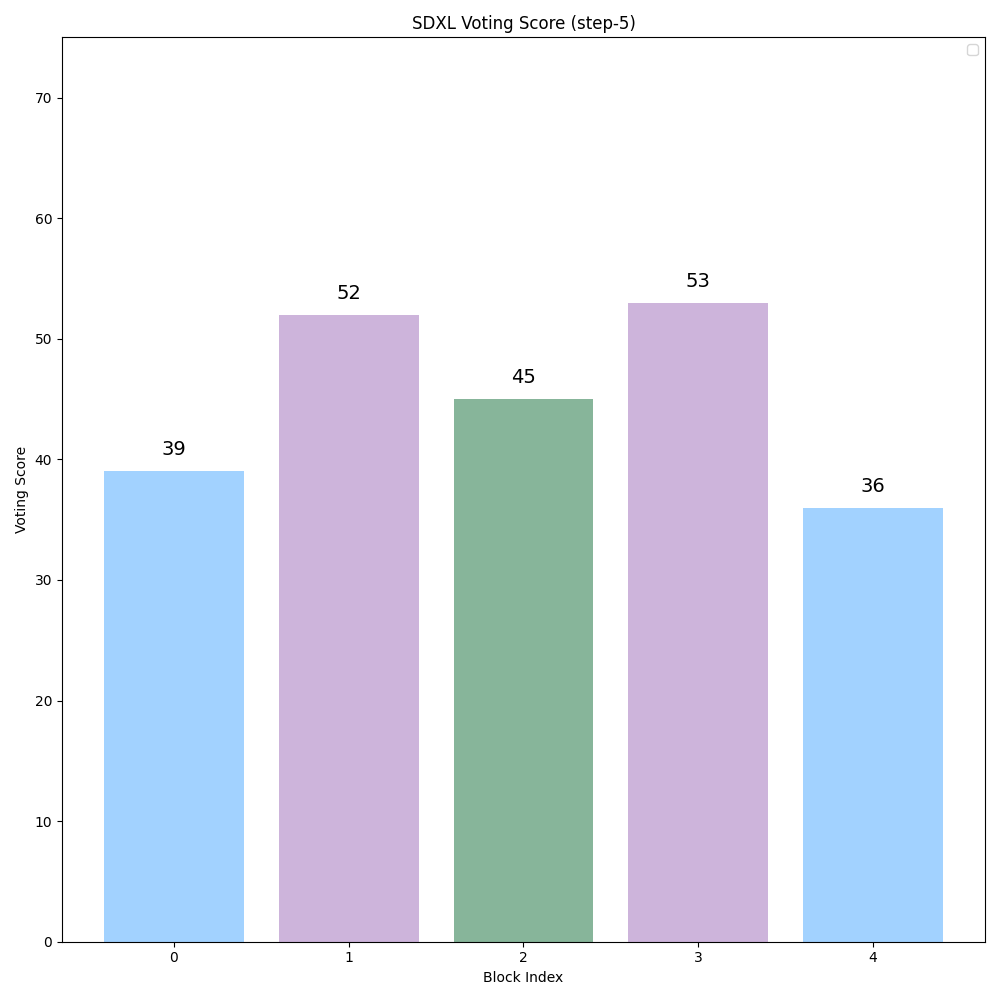} 
        & 
        \includegraphics[width=0.175\linewidth]{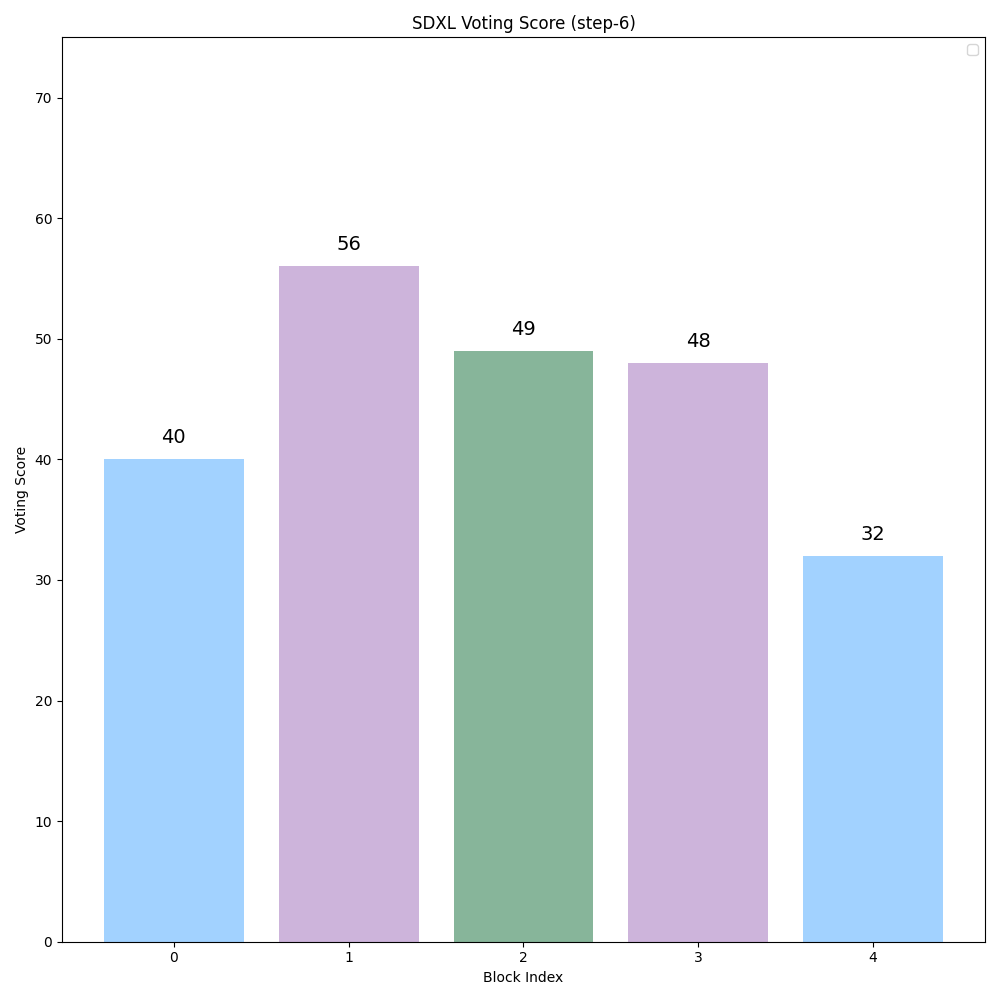}
        & 
        \includegraphics[width=0.175\linewidth]{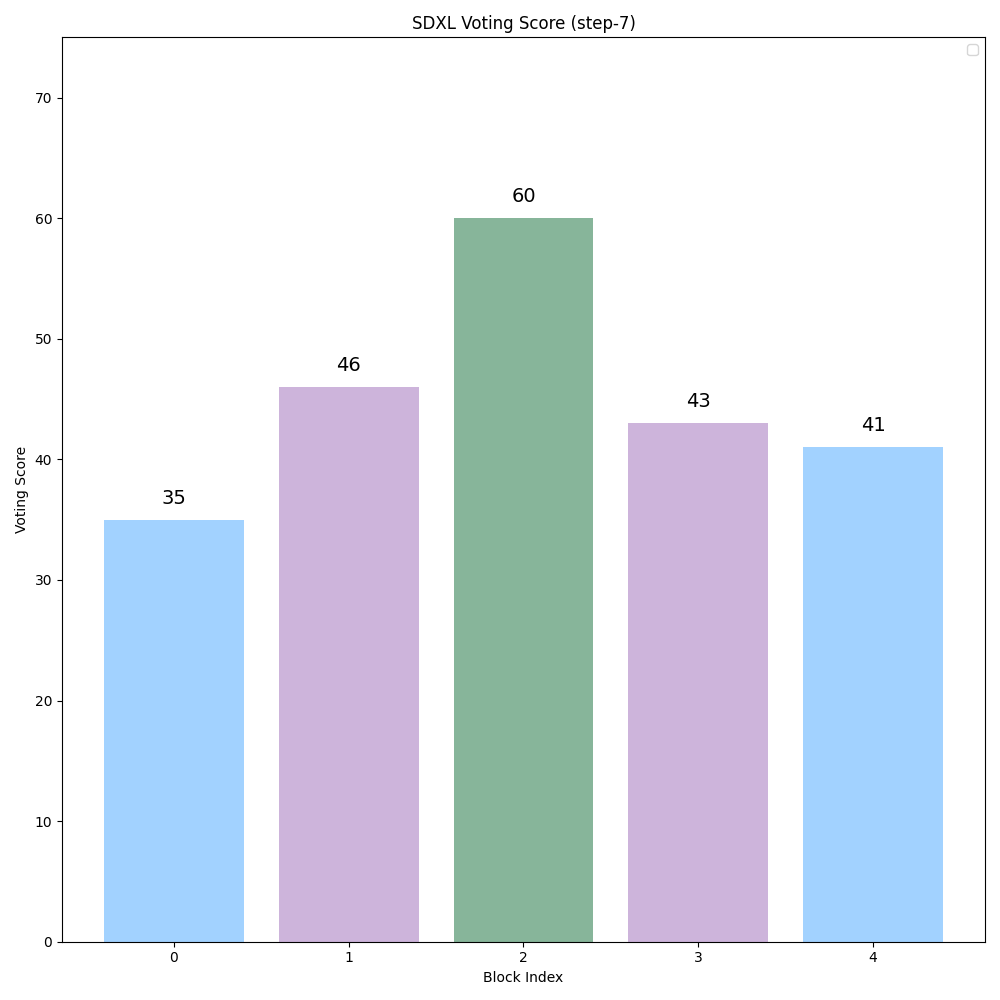}
        & 
        \includegraphics[width=0.175\linewidth]{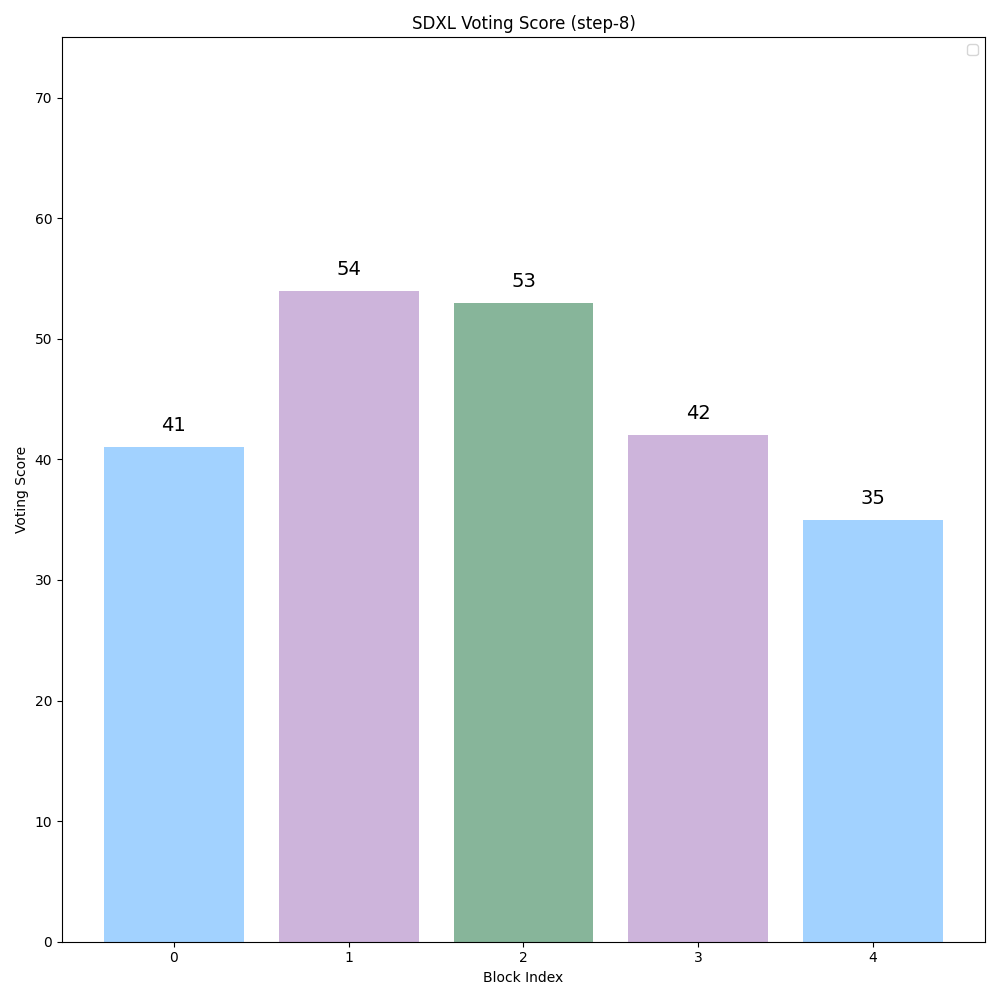}
        & 
        \includegraphics[width=0.175\linewidth]{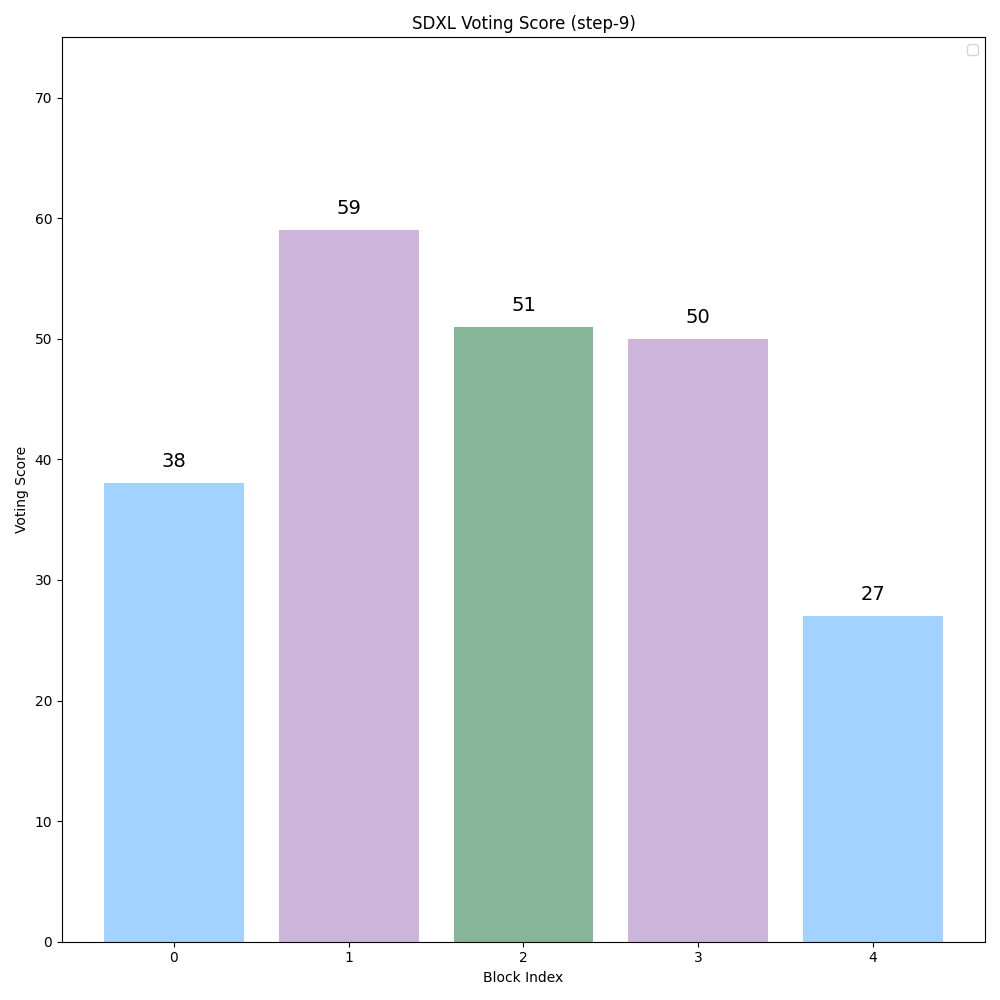}
        
        \\

        \includegraphics[width=0.175\linewidth]{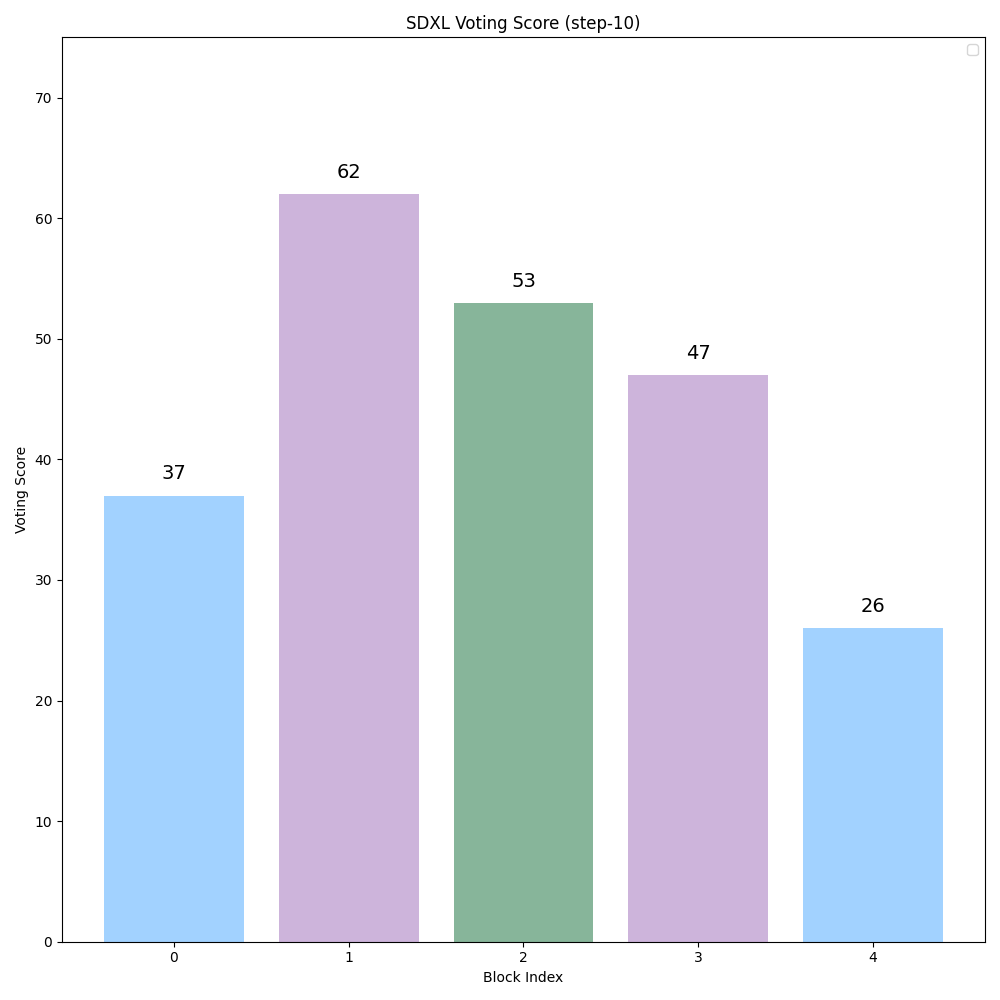} 
        & 
        \includegraphics[width=0.175\linewidth]{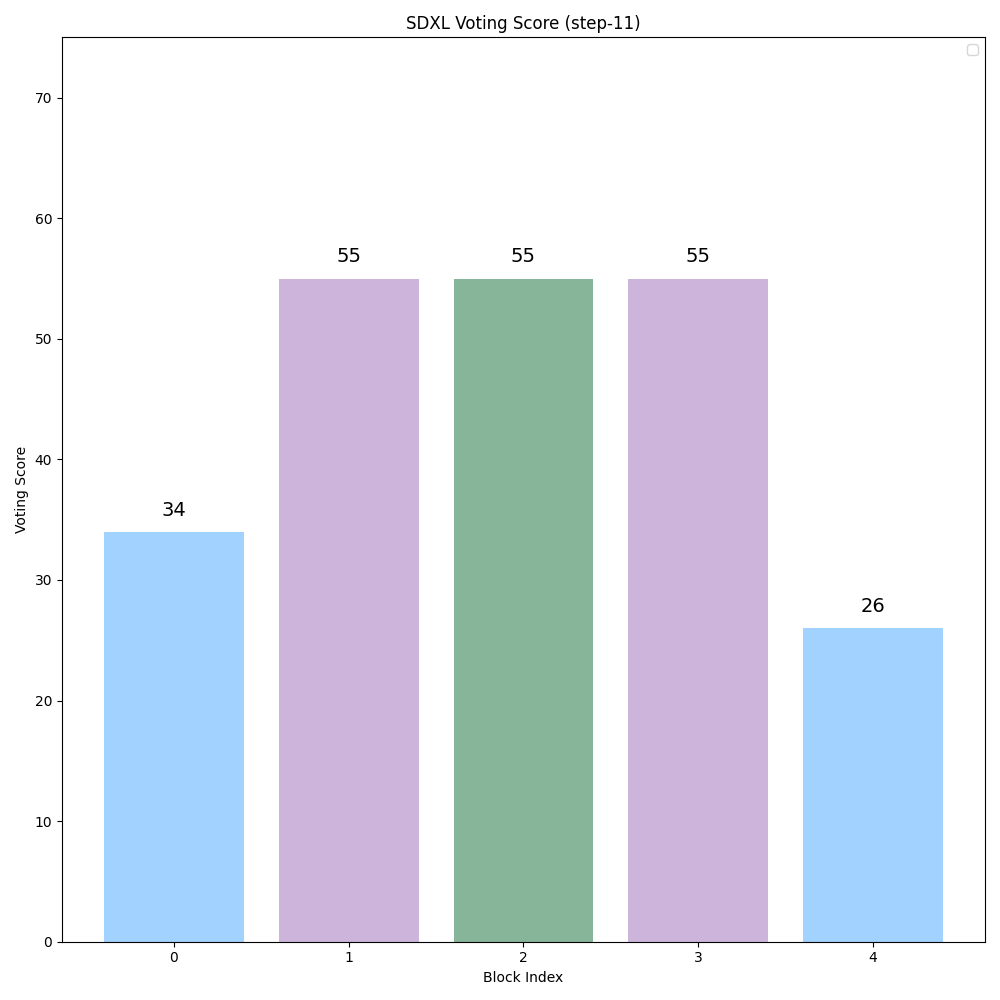}
        & 
        \includegraphics[width=0.175\linewidth]{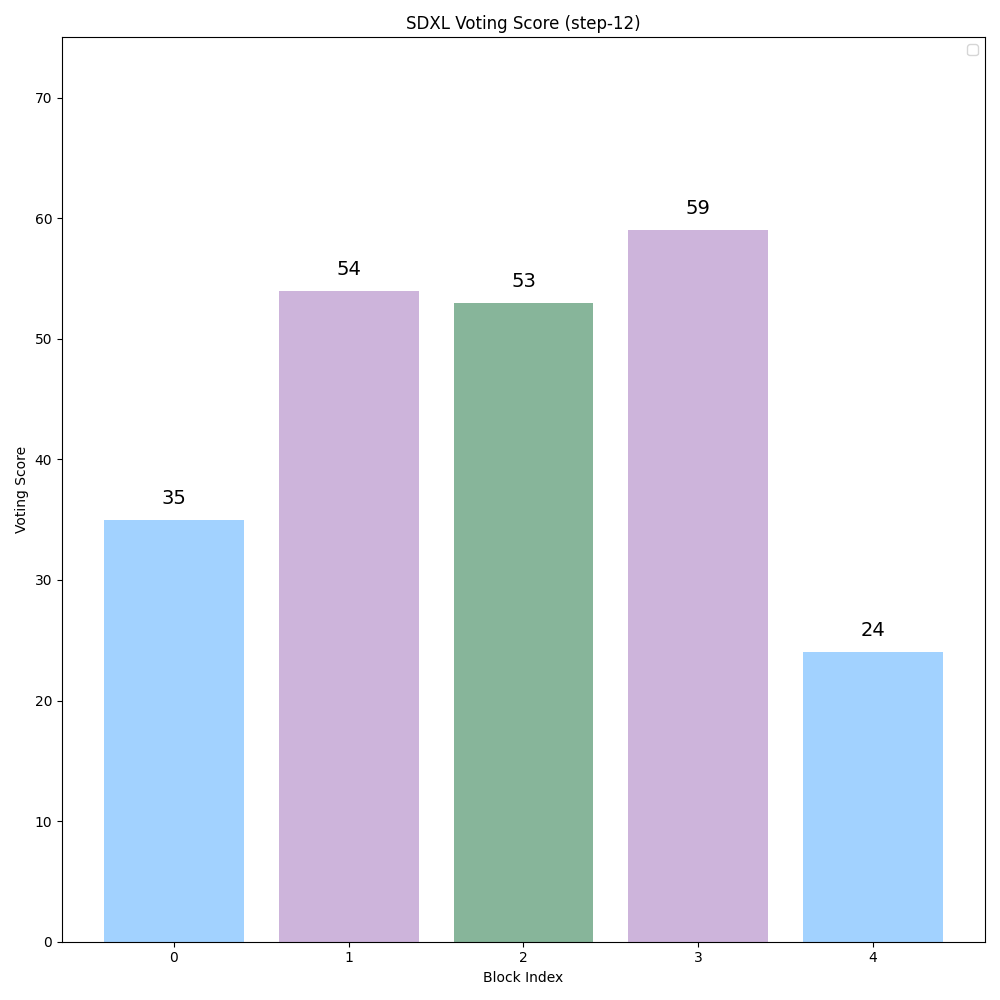}
        & 
        \includegraphics[width=0.175\linewidth]{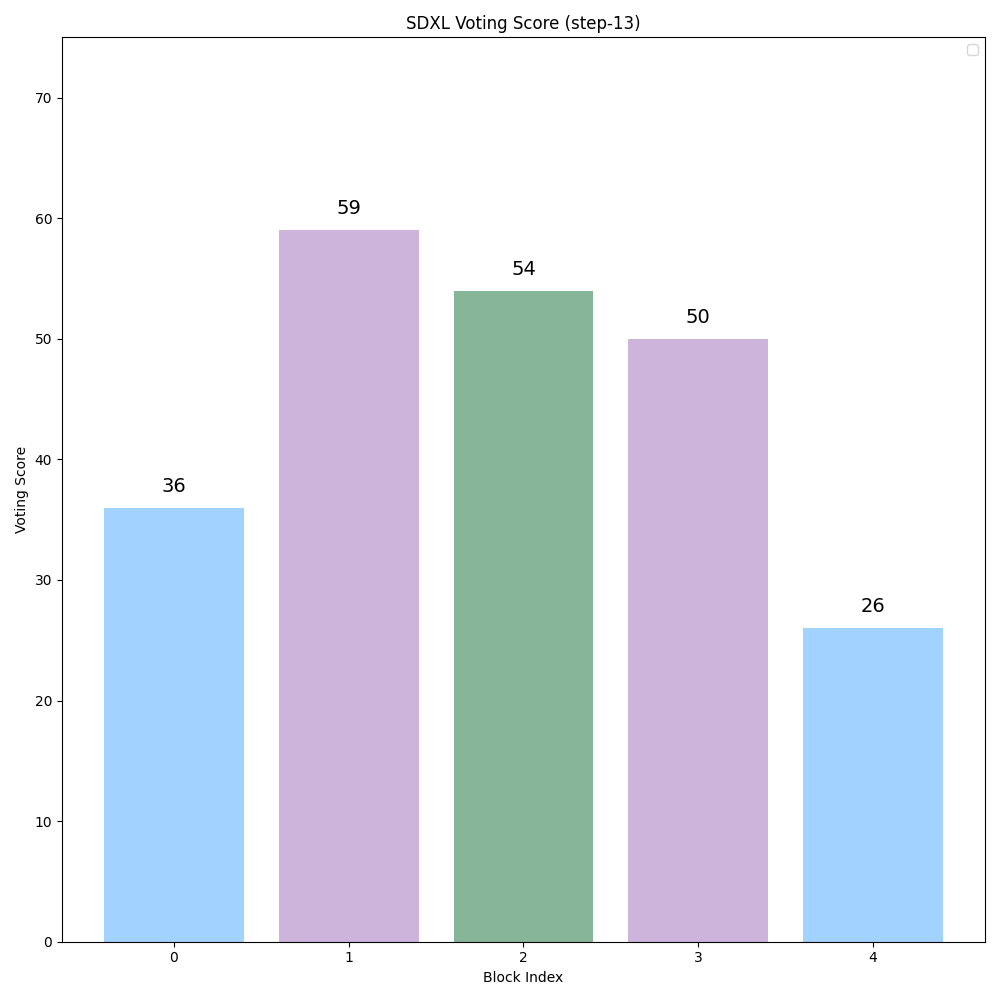}
        & 
        \includegraphics[width=0.175\linewidth]{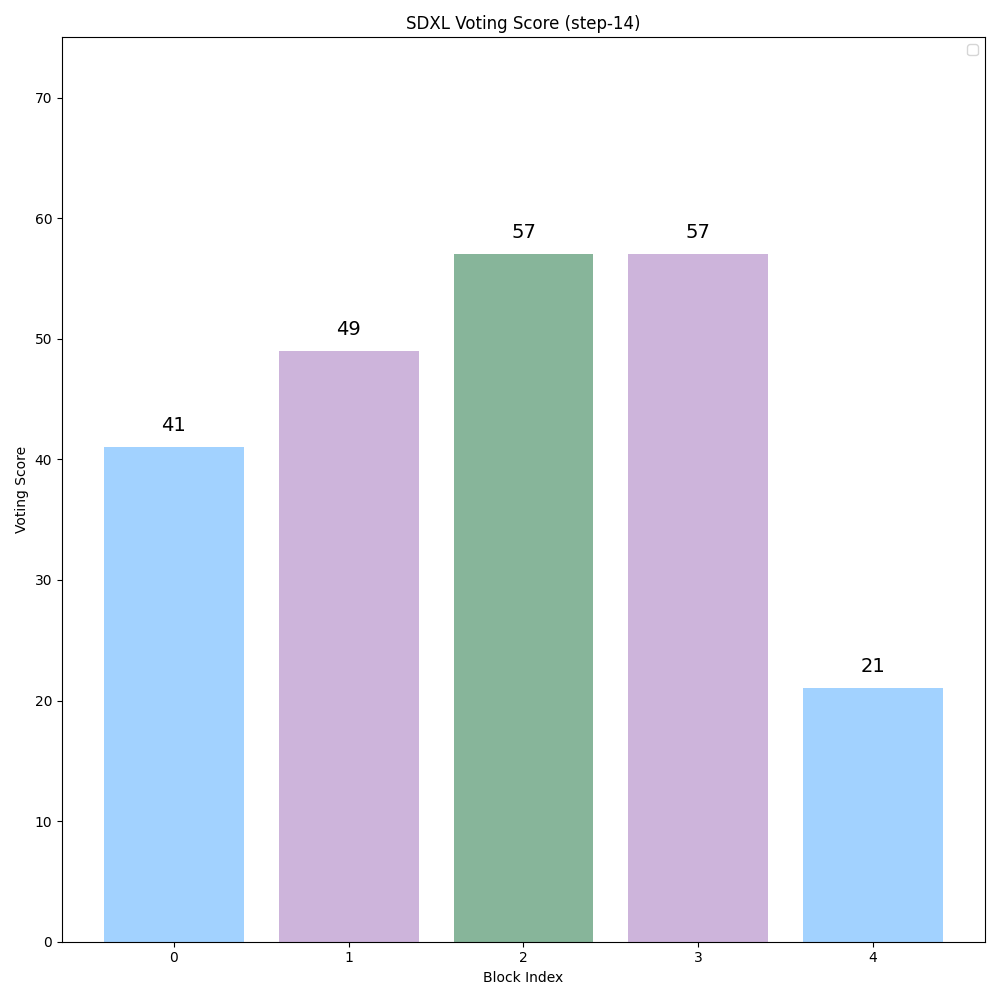}

        \\ 

        \includegraphics[width=0.175\linewidth]{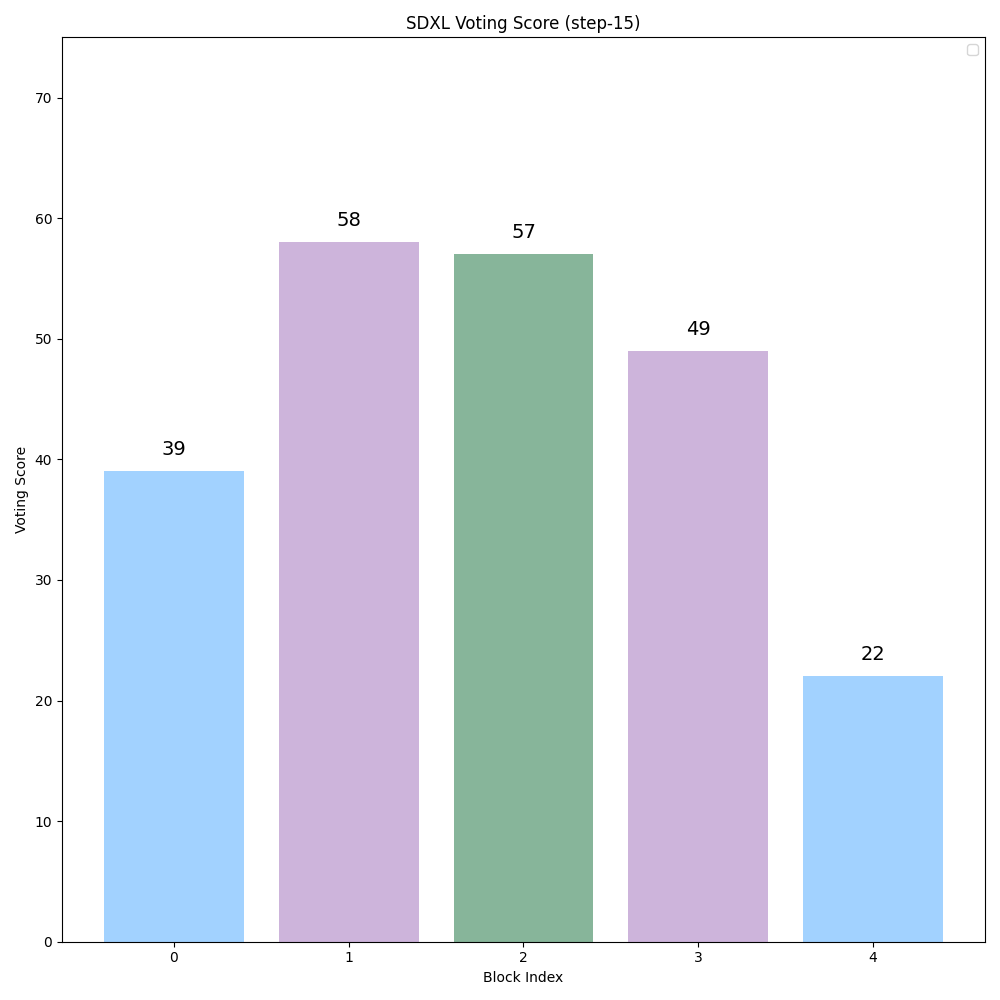} 
        & 
        \includegraphics[width=0.175\linewidth]{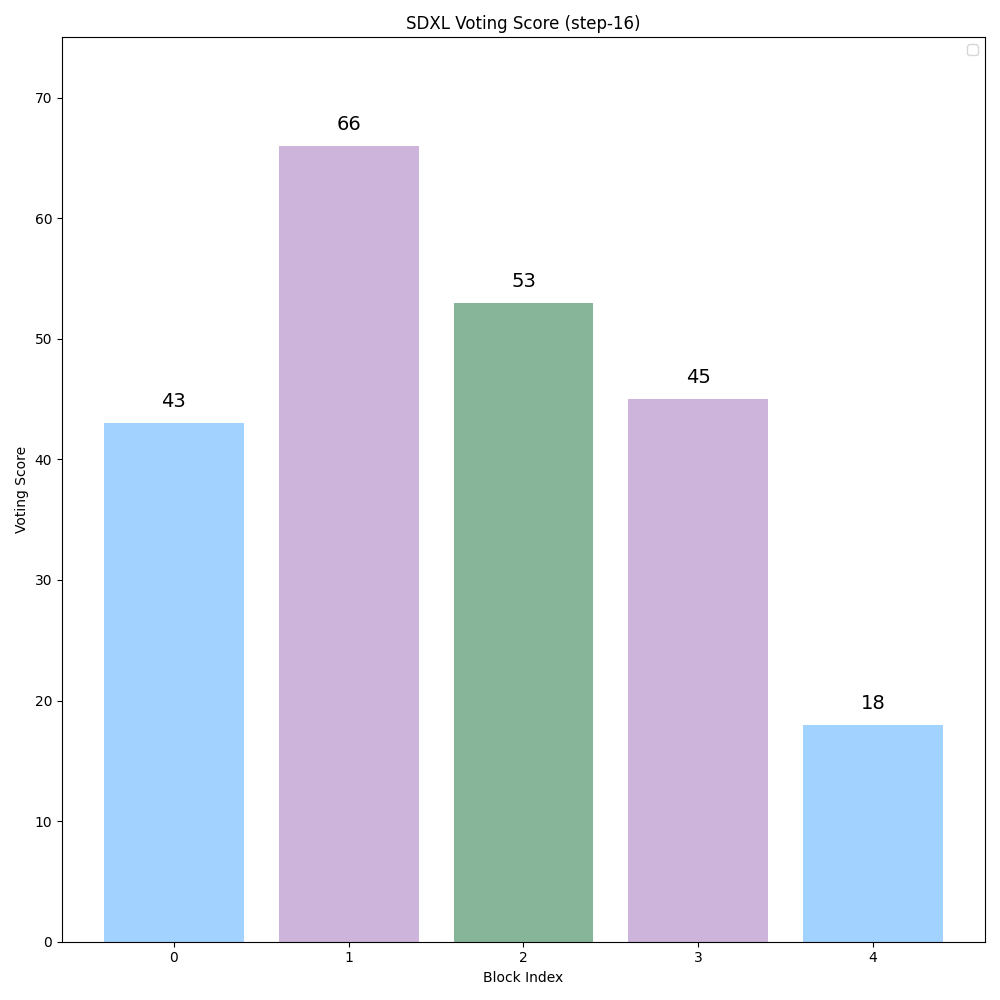}
        & 
        \includegraphics[width=0.175\linewidth]{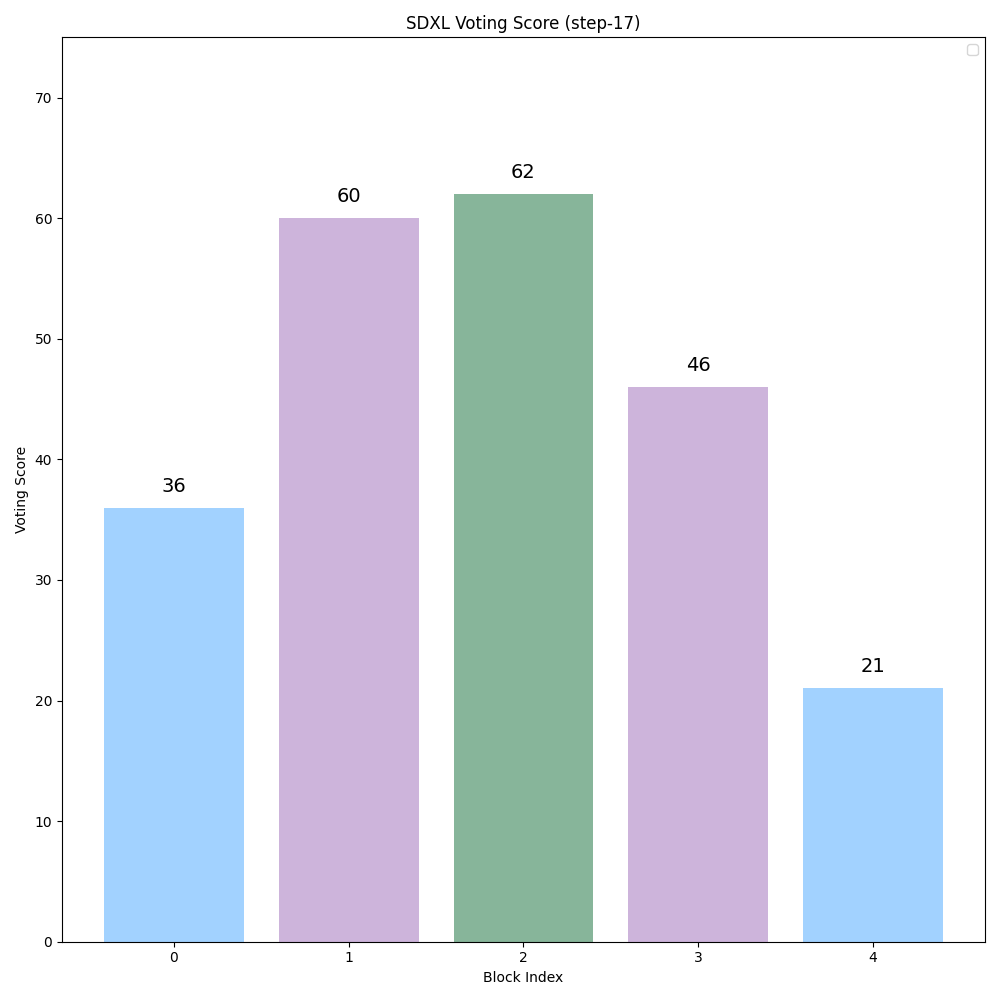}
        & 
        \includegraphics[width=0.175\linewidth]{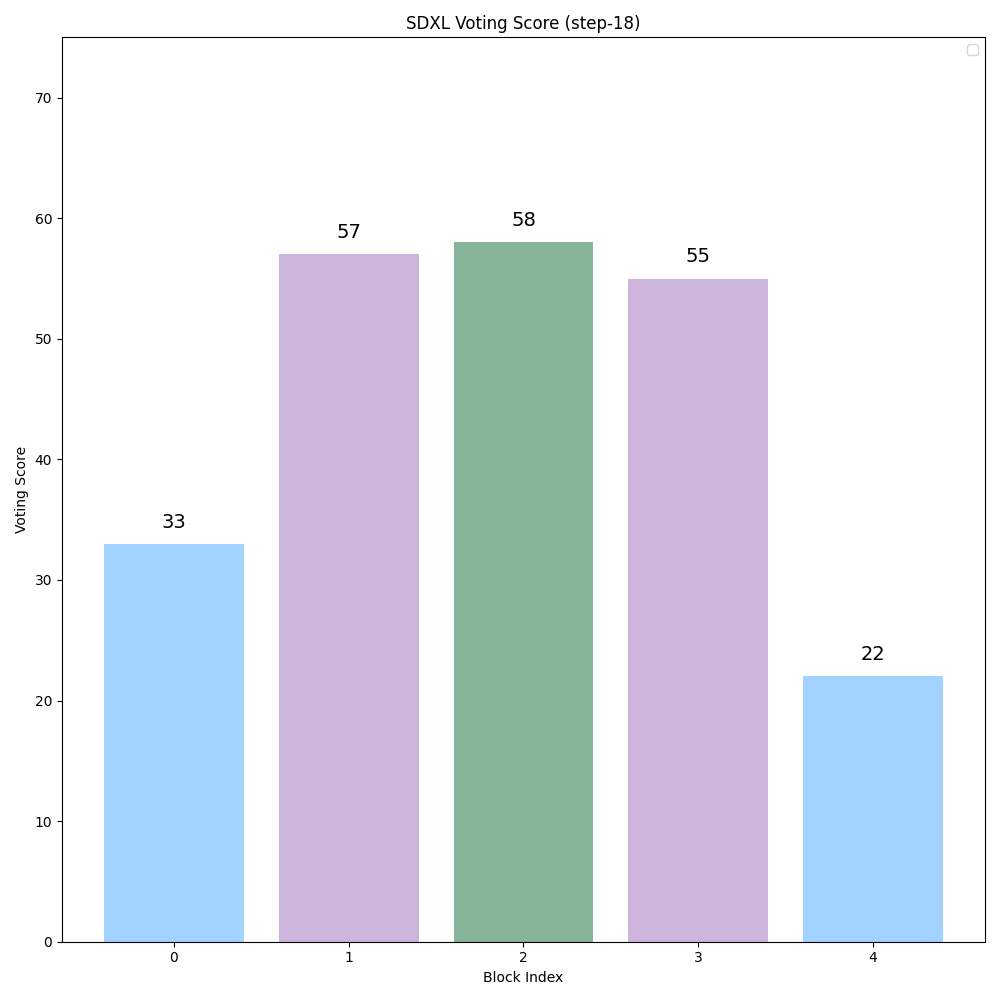}
        & 
        \includegraphics[width=0.175\linewidth]{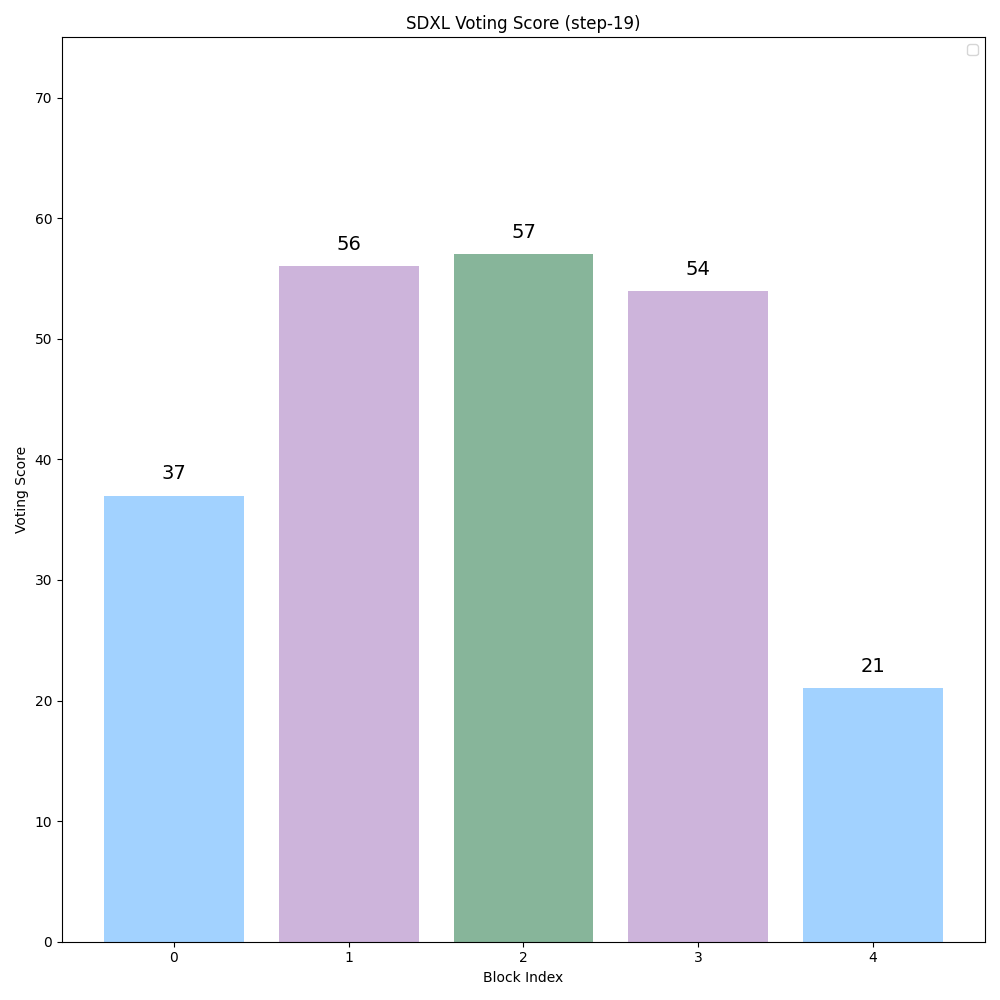}
    \end{tabular}
    \captionof{figure}{
        Bar charts of voting scores for SDXL. 
    }
    \label{tab-bar_chart_voting_score-sdxl}
\end{table*}

\paragraph{Importance Score}

To normalize the voting scores, we divide the above-mentioned voting scores by the maximum possible number of votes, and obtain the importance scores. 
The resulting heatmap is shown in Fig.~\ref{fig-heatmap_importance_score-sdturbo}, Fig.~\ref{fig-heatmap_importance_score-sdxlturbo}, Fig.~\ref{fig-heatmap_importance_score-sd} and Fig.~\ref{fig-heatmap_importance_score-sdxl}. 

The results demonstrate that, across different models and varying inference steps, the three blocks centered around the bottleneck consistently maintain a high level of importance throughout the inference process. 
This underscores the significance of the bottleneck structure to the U-Net's performance.

% 2 步 SD-Turbo 重要性得分热力图
\begin{figure}[ht]
    \centering
    \includegraphics[width=0.9\linewidth]{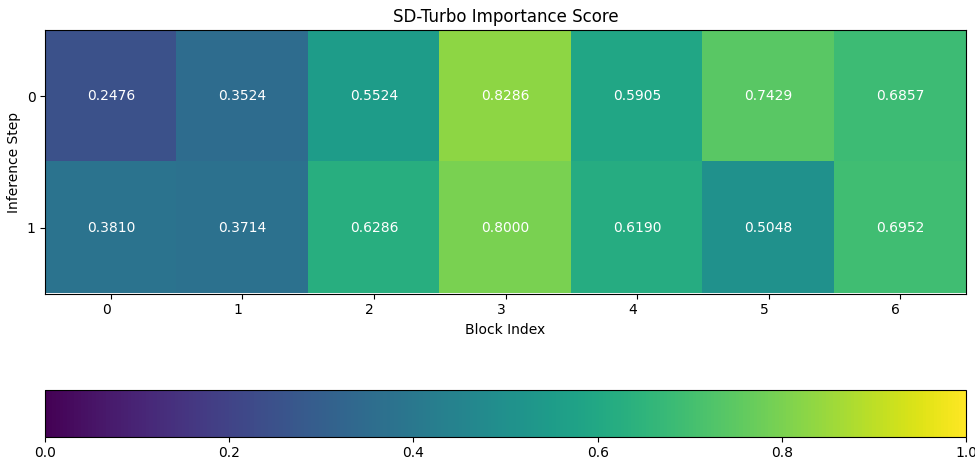}
    \caption{
        Heatmap of importance scores for SD-Turbo.  
    }
    \label{fig-heatmap_importance_score-sdturbo}
\end{figure}

% 2 步 SDXL-Turbo 重要性得分热力图
\begin{figure}[ht]
    \centering
    \includegraphics[width=0.9\linewidth]{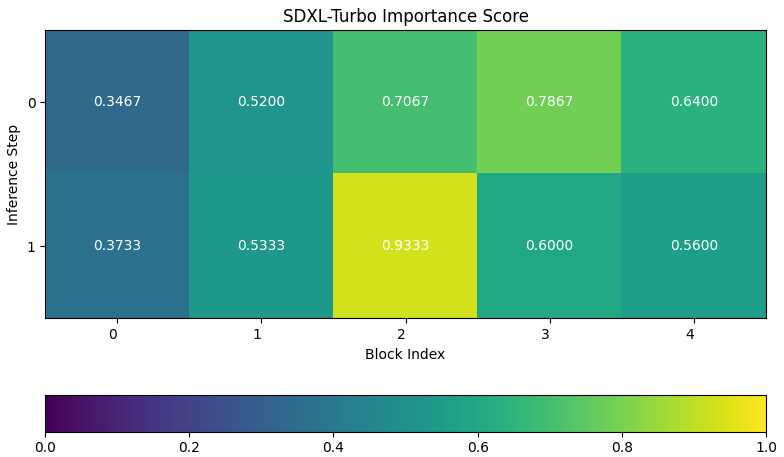}
    \caption{
        Heatmap of importance scores for SDXL-Turbo. 
    }
    \label{fig-heatmap_importance_score-sdxlturbo}
\end{figure}

% 20 步 SD 重要性得分热力图
\begin{figure}[ht]
    \centering
    \includegraphics[width=0.9\linewidth]{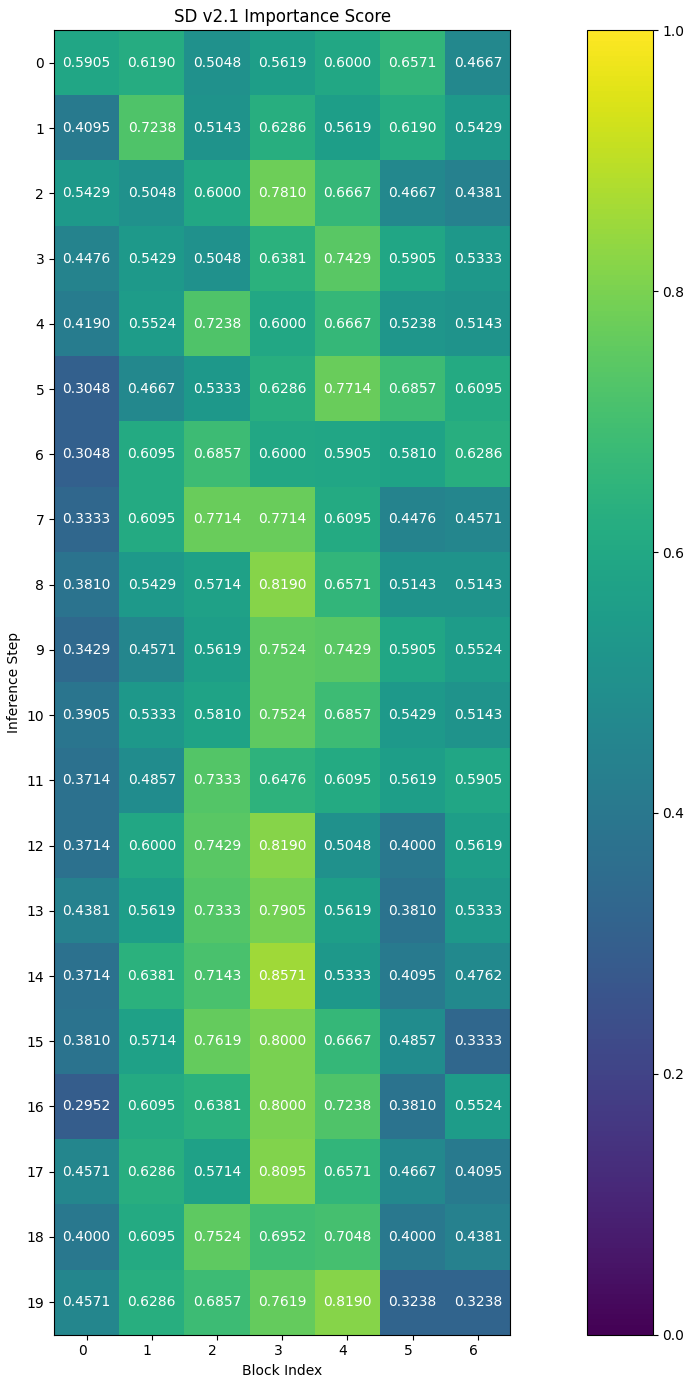}
    \caption{
        Heatmap of importance scores for SD v2.1. 
    }
    \label{fig-heatmap_importance_score-sd}
\end{figure}

% 20 步 SDXL 重要性得分热力图
\begin{figure}[ht]
    \centering
    \includegraphics[width=0.9\linewidth]{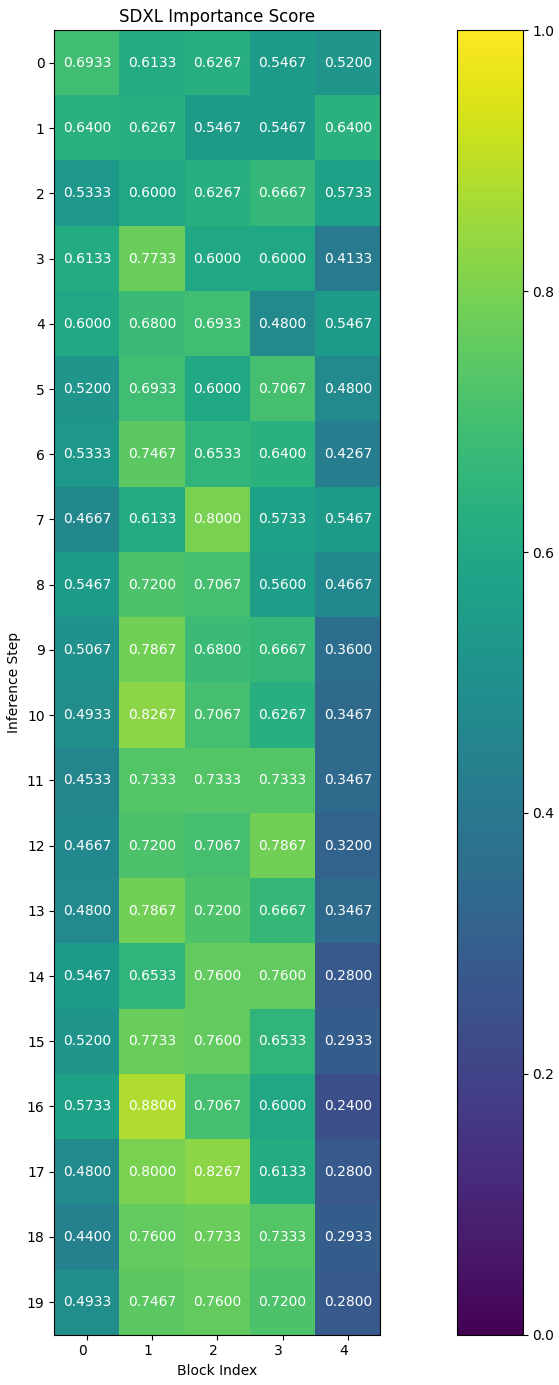}
    \caption{
        Heatmap of importance scores for SDXL. 
    }
    \label{fig-heatmap_importance_score-sdxl}
\end{figure}

\paragraph{Importance-based Re-weighting Schedule. }

We apply importance-based re-weighting to a wide range of prompts. 

Results are shown in Fig.~\ref{fig-hpd_sdturbo_sdxlturbo_fix_r_appx}. 
Unlike the static re-weighting schedules in Tab.~\ref{tab-comparison_between_different_models_and_steps_appx}, all our importance-based re-weighting schedules lead to performance improvements. 
It empirically validates the effectiveness of the IP, and the consistency between the experimental phenomena and theoretical analysis. 

% SD-Turbo/SDXL-Turbo 固定 r = 1.1, 随 l 变化的折线图
\begin{figure}[h]
    \centering
    \includegraphics[width=0.98\linewidth]{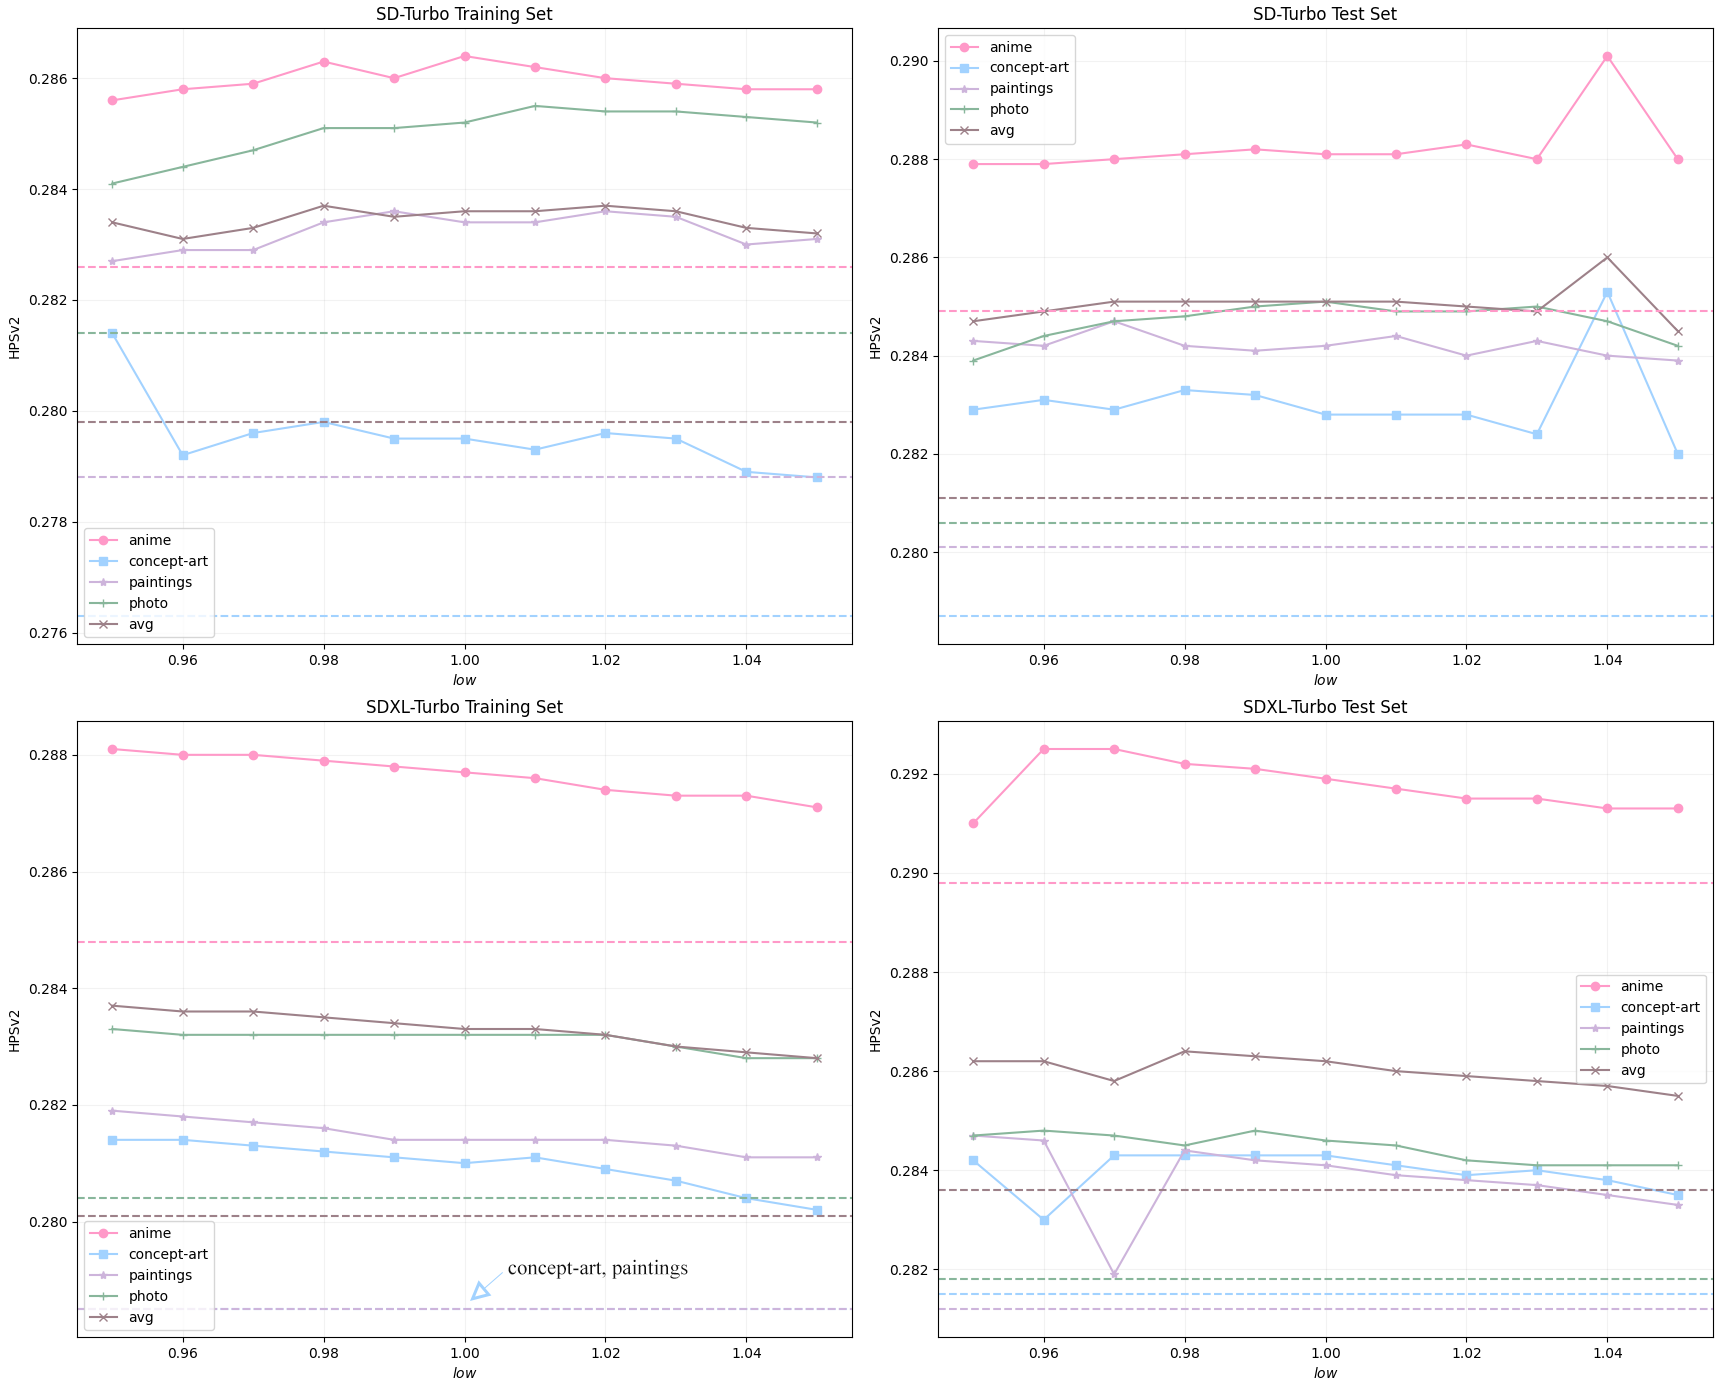}
    \caption{
        (Fig.~\ref{fig-hpd_sdturbo_sdxlturbo_fix_r} in the main paper. ) 
        Line chart showing the effect of re-weighting on SD-Turbo and SDXL-Turbo with fixed $high = 1.1$ as $low$ varies. 
        Lines of the same color represent the same category, where dashed lines indicate the vanilla schedule, and solid lines represent our re-weighting schedule. 
    }
    \label{fig-hpd_sdturbo_sdxlturbo_fix_r_appx}
\end{figure}
