# Supplementary material for: Dynamic Importance in Diffusion U-Net for Enhanced Image Synthesis
Source: arXiv:2504.03471 source file (2025-05-05)
Supplement: Supplementary file 4 [file enhanced_image_synthesis_details.tex]

\section{Supplementary to Enhanced Image Synthesis}
\label{appx_sec-empirical_analysis_of_synthesis_improvements}

\subsection{Static Re-weighting Schedule Details}

\paragraph{Experimental Settings}

The results in Tab.~\ref{tab-comparison_between_different_models_and_steps_appx} are evaluated with 20 samples for each model under the following settings: 

\begin{itemize}
    \item \textbf{SD-Turbo}: 2-step inference with prompt ``\emph{A small baby bird on a piece of metal.}" from the \emph{photo} category in Human Preference Dataset v2~\cite{wu2023humanpreferencescorev2}. 

    \item \textbf{SDXL-Turbo}: 2-step inference with prompt ``\emph{A landscape with a building in the style of Simon Stalenhag.}" from the \emph{concept-art} category. 
    
    \item \textbf{SD v2.1}: 20-step inference with prompt ``\emph{A portrait of Fox McCloud firing a blaster in anthropomorphic furry art style from the Star Fox series, illustrated by Jim Burns.}" from the \emph{anime} category. 

    \item \textbf{SDXL}: 20-step inference with prompt ``\emph{An English woman plays the lute with a slender neck and long dark hair in a painting by WilliamAdolphe Bouguereau.}" from the \emph{paintings} category. 
\end{itemize}

\paragraph{Qualitative Results}

Samples of difference models with different inference steps, using the vanilla re-weighting schedule and our best re-weighting schedule (in Tab.~\ref{tab-comparison_between_different_models_and_steps_appx}) are shown in Fig.~\ref{fig-static_reweighting_sdturbo_sdxlturbo_appx} and Fig.~\ref{fig-static_reweighting_sd_sdxl_appx}, respectively. 

Under the same number of inference steps, the samples generated under our re-weighting schedule exhibit greater clarity and more vibrant colors, indicating our method's capability to enhance sampling aesthetics. 
Across different numbers of inference steps, the aesthetic quality of samples under our re-weighting schedule with fewer steps even surpasses that of samples under the vanilla re-weighting schedule with more steps. 
This suggests that, our method improves the SNR during sampling, thereby enhancing inference efficiency.

% SD-Turbo / SDXL-Turbo, static re-weighting 的采样图
\begin{table*}[h]
    \centering
    \begin{tabular}{c | c c c | c c c}
        \hline

        \textbf{Re-Weighting} & \multicolumn{3}{c|}{\textbf{SD-Turbo}} & \multicolumn{3}{c}{\textbf{SDXL-Turbo}} \\
        \textbf{Strategy} & 1-step & 2-step & 3-step & 1-step & 2-step & 3-step \\
        
        \hline

        \rule{0pt}{0pt} \\
        
        % default
        \parbox[t][-2.25cm][c]{2.0cm}{\centering Vanilla} & 
        \includegraphics[width=0.12\textwidth]{algorithm-figure-table/static_reweighting/sd-turbo/1_step/default.png} & 
        \includegraphics[width=0.12\textwidth]{algorithm-figure-table/static_reweighting/sd-turbo/2_step/default.png} & 
        \includegraphics[width=0.12\textwidth]{algorithm-figure-table/static_reweighting/sd-turbo/3_step/default.png} & 
        \includegraphics[width=0.12\textwidth]{algorithm-figure-table/static_reweighting/sdxl-turbo/1_step/default.png} & 
        \includegraphics[width=0.12\textwidth]{algorithm-figure-table/static_reweighting/sdxl-turbo/2_step/default.png} & 
        \includegraphics[width=0.12\textwidth]{algorithm-figure-table/static_reweighting/sdxl-turbo/3_step/default.png} \\
        
        % ours
        \parbox[t][-2.25cm][c]{2.0cm}{\centering Vanilla} & 
        \includegraphics[width=0.12\textwidth]{algorithm-figure-table/static_reweighting/sd-turbo/1_step/ours.png} & 
        \includegraphics[width=0.12\textwidth]{algorithm-figure-table/static_reweighting/sd-turbo/2_step/ours.png} & 
        \includegraphics[width=0.12\textwidth]{algorithm-figure-table/static_reweighting/sd-turbo/3_step/ours.png} & 
        \includegraphics[width=0.12\textwidth]{algorithm-figure-table/static_reweighting/sdxl-turbo/1_step/ours.png} & 
        \includegraphics[width=0.12\textwidth]{algorithm-figure-table/static_reweighting/sdxl-turbo/2_step/ours.png} & 
        \includegraphics[width=0.12\textwidth]{algorithm-figure-table/static_reweighting/sdxl-turbo/3_step/ours.png}
        \rule{0pt}{0pt} \\

        \rule{0pt}{0pt} \\

        \hline
    \end{tabular}
    \captionof{figure}{
        Samples of SD-Turbo and SDXL-Turbo with different inference steps, using the vanilla re-weighting schedule and our best re-weighting schedule, respectively. 
    }
    \label{fig-static_reweighting_sdturbo_sdxlturbo_appx}
\end{table*}

% SD / SDXL static re-weighting 的采样图
\begin{table*}[h]
    \centering
    \begin{tabular}{c | c c c | c c c}
        \hline

        \textbf{Re-Weighting} & \multicolumn{3}{c|}{\textbf{SD v2.1}} & \multicolumn{3}{c}{\textbf{SDXL}} \\
        \textbf{Strategy} & 10-step & 15-step & 20-step & 10-step & 15-step & 20-step \\
        
        \hline

        \rule{0pt}{0pt} \\
        
        % default
        \parbox[t][-2.25cm][c]{2.0cm}{\centering Vanilla} & 
        \includegraphics[width=0.12\textwidth]{algorithm-figure-table/static_reweighting/sd/10_step/default.png} & 
        \includegraphics[width=0.12\textwidth]{algorithm-figure-table/static_reweighting/sd/15_step/default.png} & 
        \includegraphics[width=0.12\textwidth]{algorithm-figure-table/static_reweighting/sd/20_step/default.png} & 
        \includegraphics[width=0.12\textwidth]{algorithm-figure-table/static_reweighting/sdxl/10_step/default.png} & 
        \includegraphics[width=0.12\textwidth]{algorithm-figure-table/static_reweighting/sdxl/15_step/default.png} & 
        \includegraphics[width=0.12\textwidth]{algorithm-figure-table/static_reweighting/sdxl/20_step/default.png} \\
        
        % ours
        \parbox[t][-2.25cm][c]{2.0cm}{\centering Vanilla} & 
        \includegraphics[width=0.12\textwidth]{algorithm-figure-table/static_reweighting/sd/10_step/ours.png} & 
        \includegraphics[width=0.12\textwidth]{algorithm-figure-table/static_reweighting/sd/15_step/ours.png} & 
        \includegraphics[width=0.12\textwidth]{algorithm-figure-table/static_reweighting/sd/20_step/ours.png} & 
        \includegraphics[width=0.12\textwidth]{algorithm-figure-table/static_reweighting/sdxl/10_step/ours.png} & 
        \includegraphics[width=0.12\textwidth]{algorithm-figure-table/static_reweighting/sdxl/15_step/ours.png} & 
        \includegraphics[width=0.12\textwidth]{algorithm-figure-table/static_reweighting/sdxl/20_step/ours.png} \\
        
        \rule{0pt}{0pt} \\

        \hline
    \end{tabular}
    \captionof{figure}{
        Samples of SD and SDXL with different inference steps, using the vanilla re-weighting schedule and our best re-weighting schedule, respectively. 
    }
    \label{fig-static_reweighting_sd_sdxl_appx}
\end{table*}

% importance-based re-weighting, SDXL-Turbo, 2
\begin{table*}[t]
    \centering
    \begin{tabular}{c | c c c c}
        \hline

        \multirow{2}{*}{\textbf{Models}} & \multicolumn{4}{c}{\textbf{Re-weighting Schedule}} \\
        ~ & Vanilla & $[0.98, 1.1]$ / $[0.95, 1.1]$ & $[0.98, 1.15]$ / $[0.95, 1.15]$ & $[0.98, 1.2]$ / $[0.95, 1.2]$ \\
        
        \hline

        \rule{0pt}{0pt} \\
        
        % SD-Turbo
        \parbox[t][-2.75cm][c]{2.0cm}{\centering SD-Turbo} & 
        \includegraphics[width=0.15\textwidth]{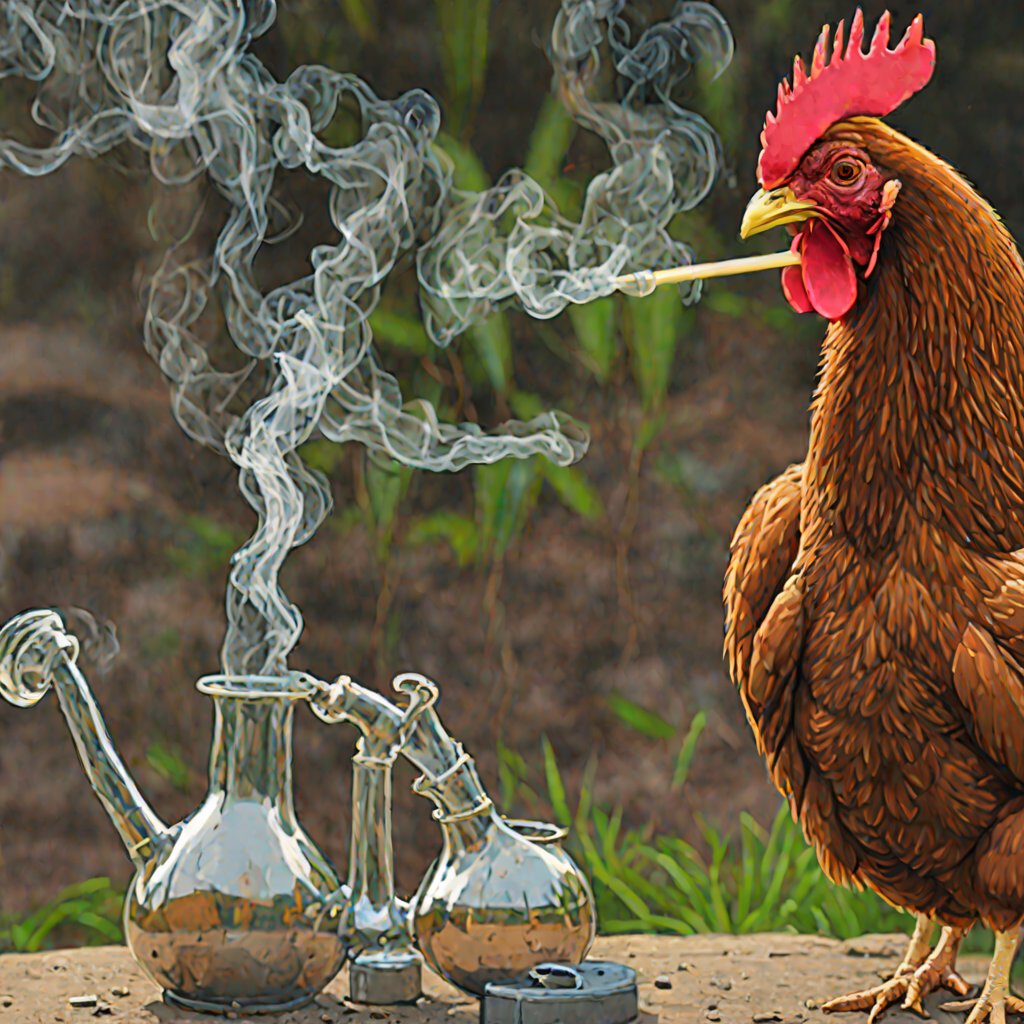} & \includegraphics[width=0.15\textwidth]{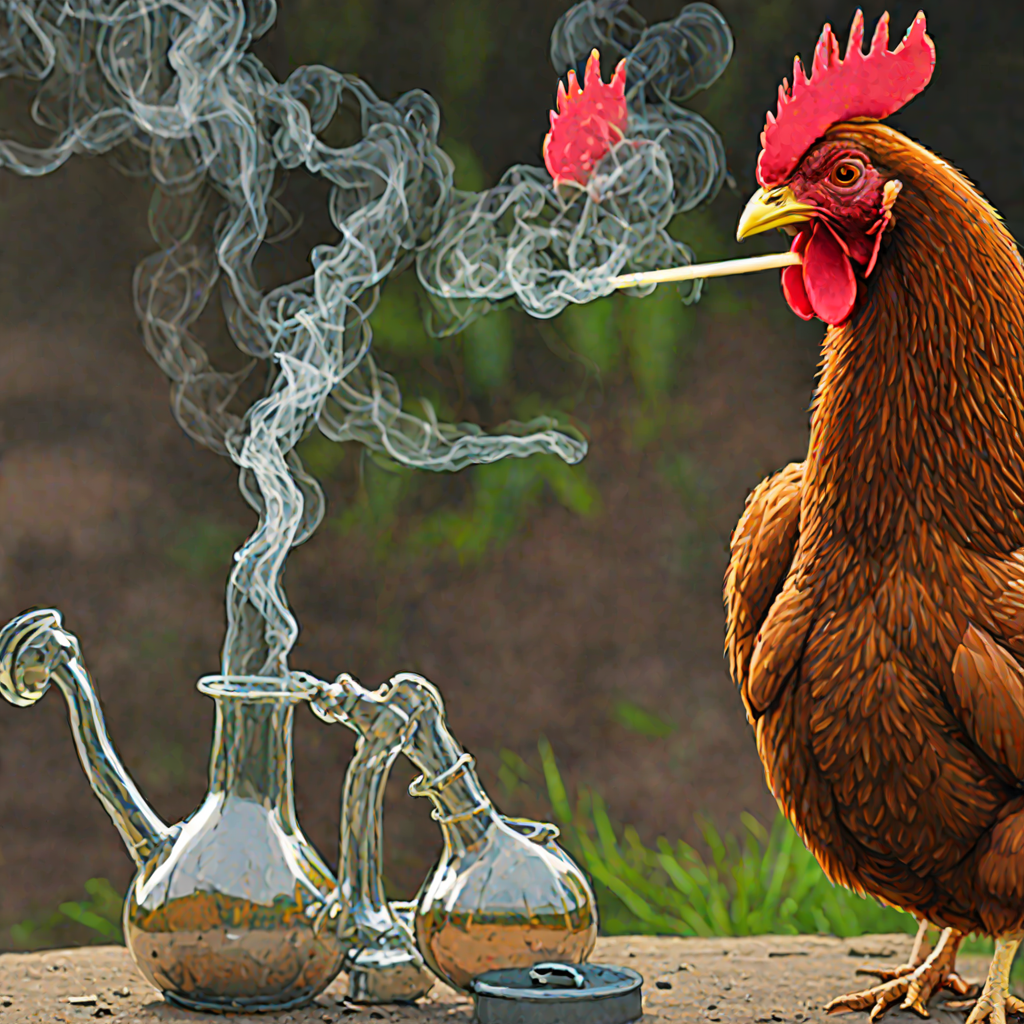} & 
        \includegraphics[width=0.15\textwidth]{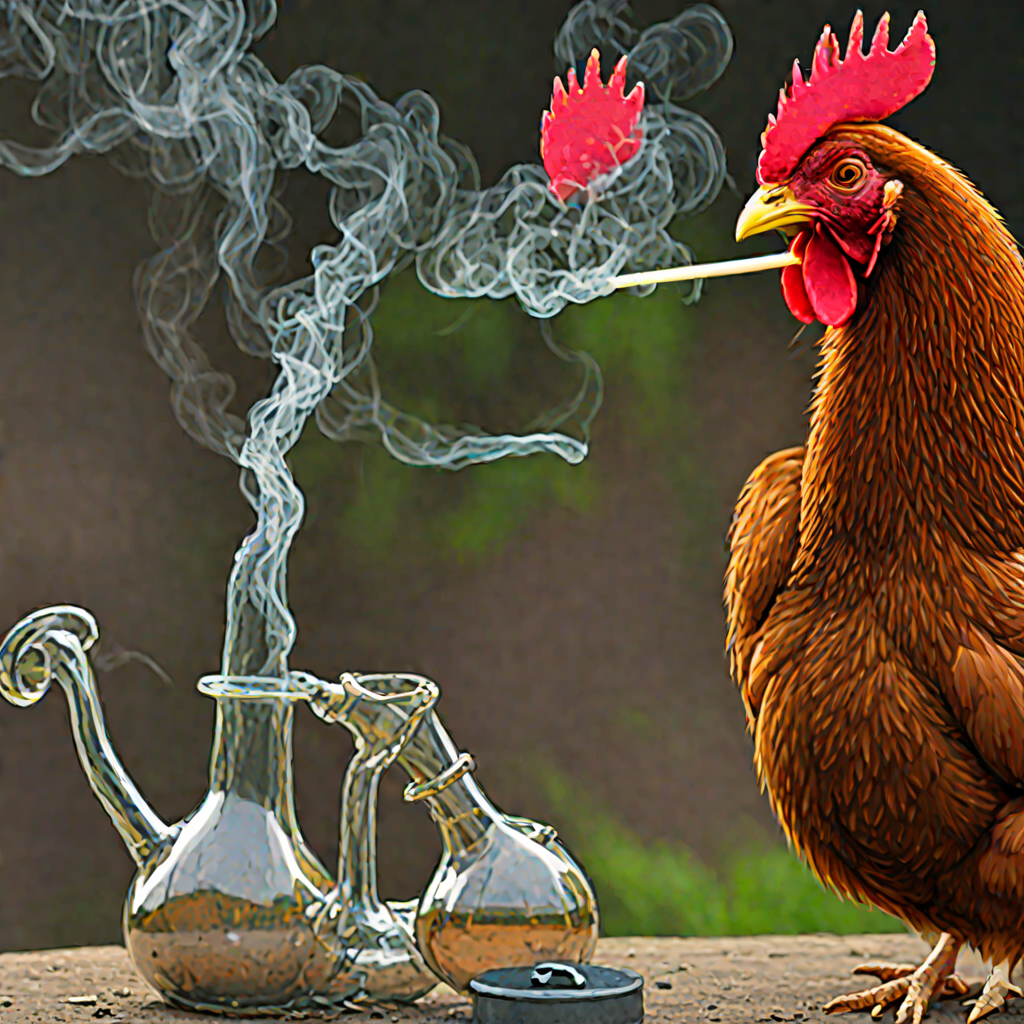} & 
        \includegraphics[width=0.15\textwidth]{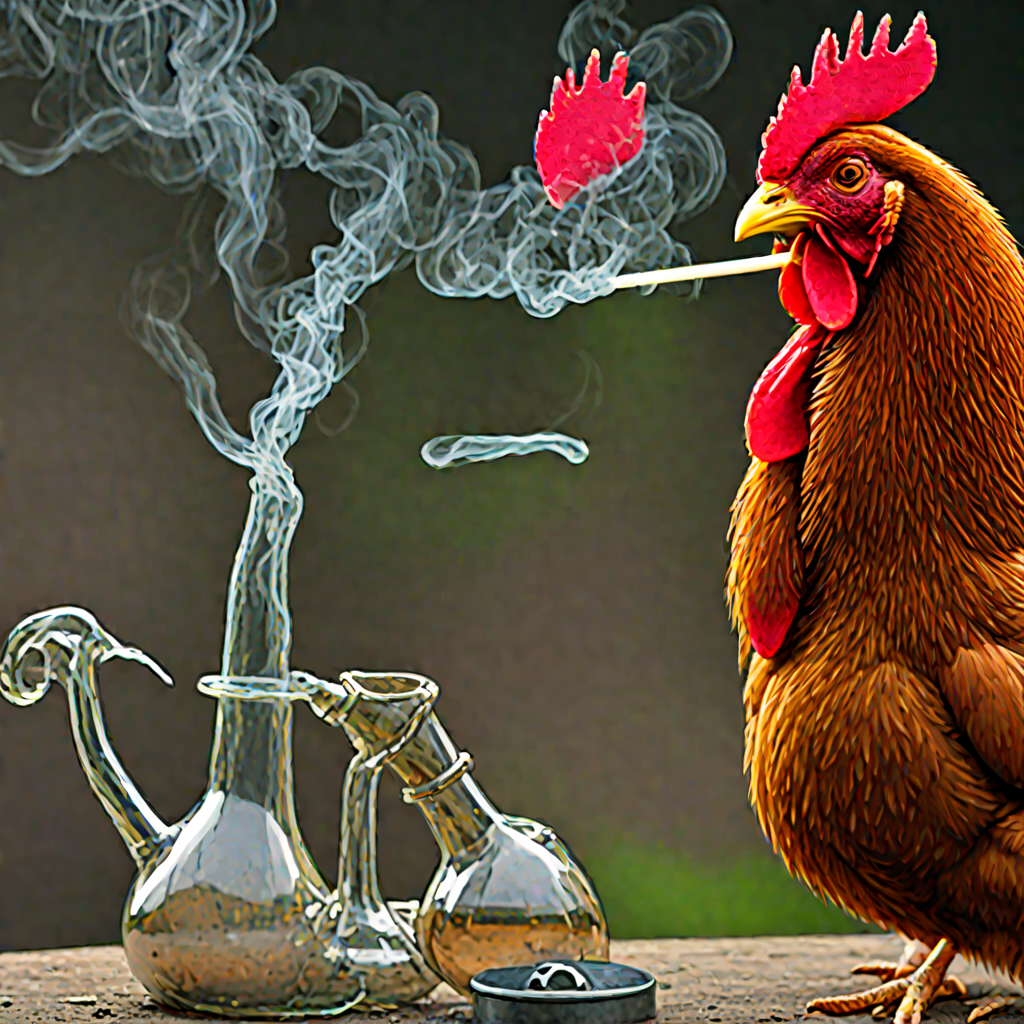} \\

        % SDXL-Turbo
        \parbox[t][-2.75cm][c]{2.0cm}{\centering SDXL-Turbo} & 
        \includegraphics[width=0.15\textwidth]{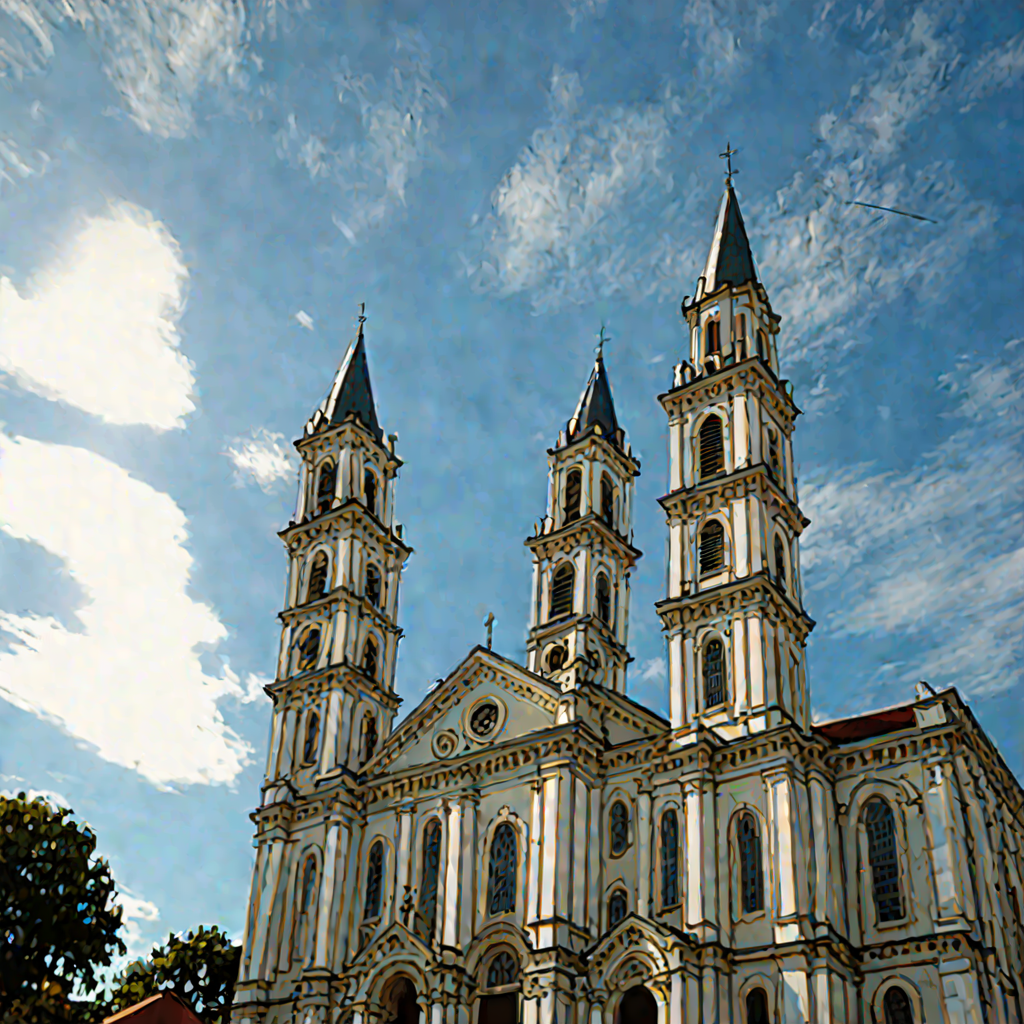} & \includegraphics[width=0.15\textwidth]{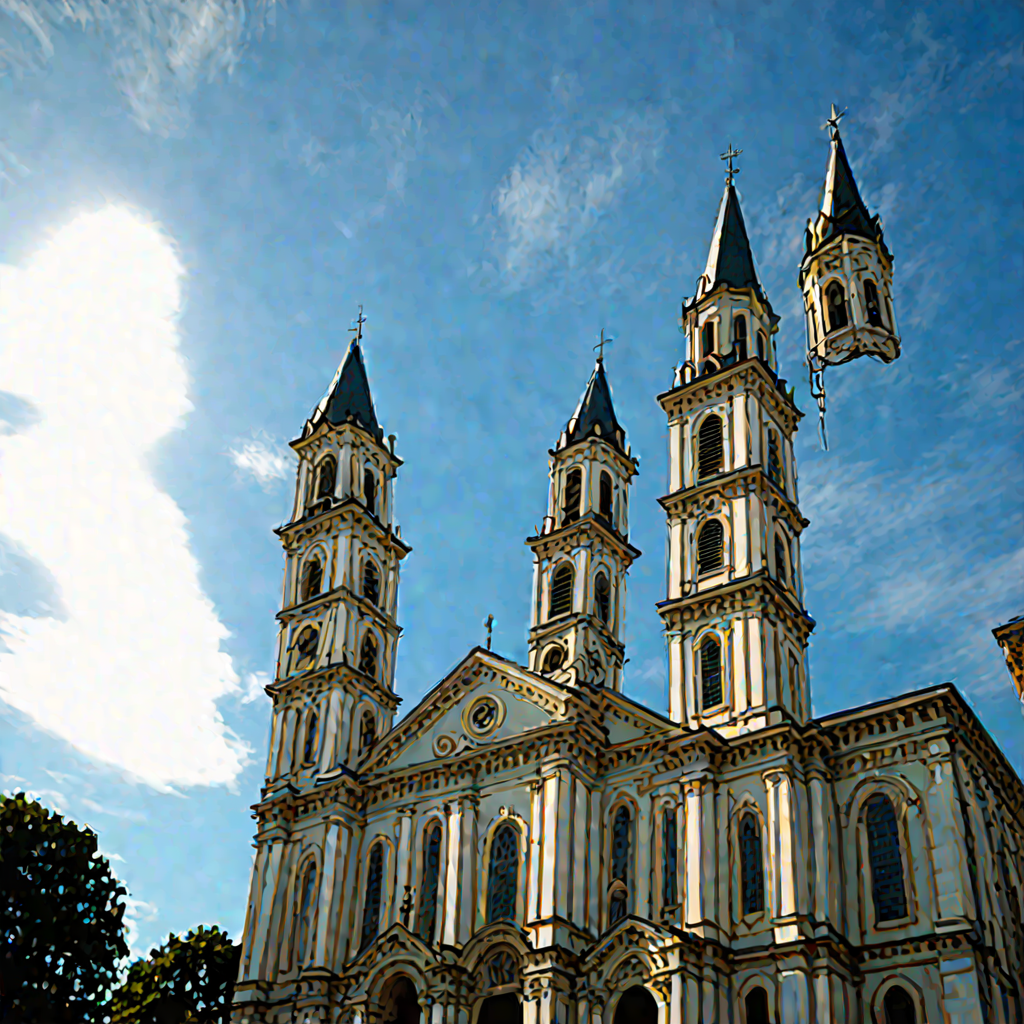} & 
        \includegraphics[width=0.15\textwidth]{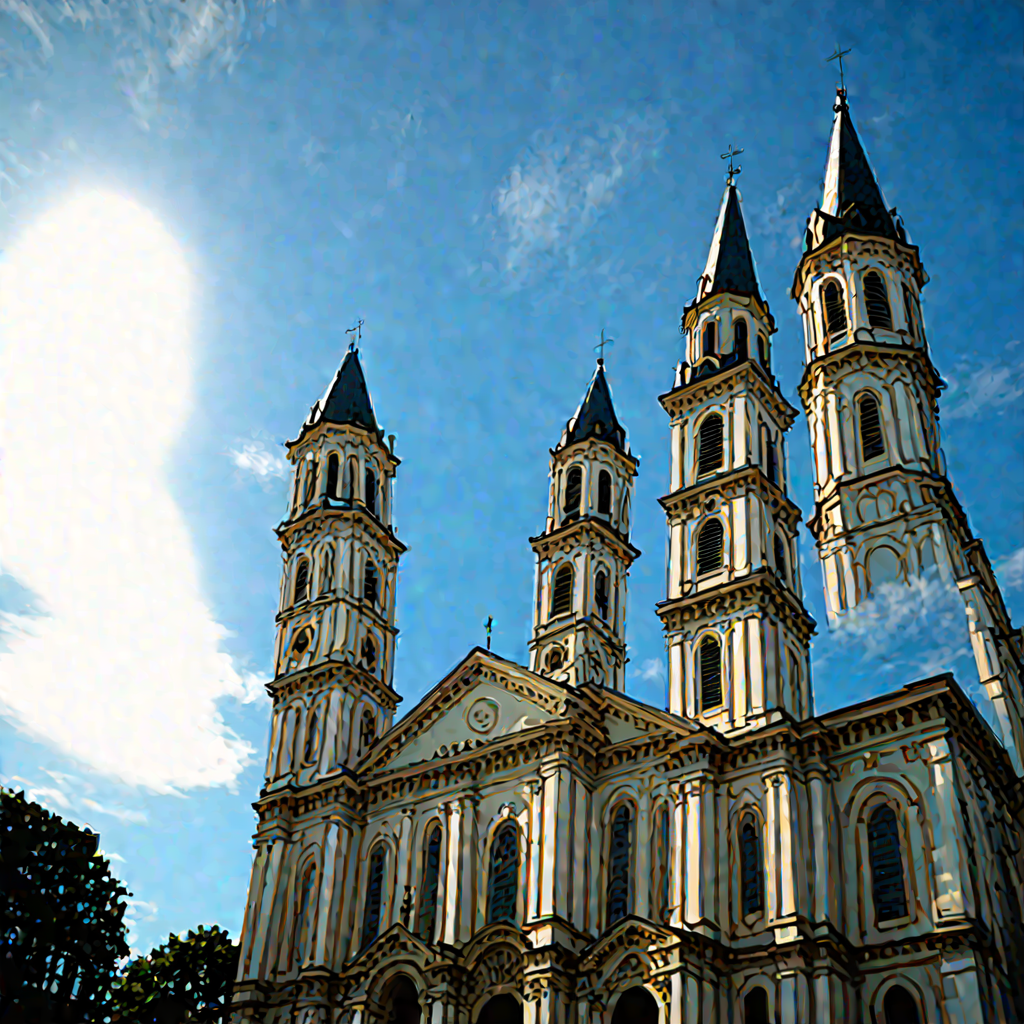} & 
        \includegraphics[width=0.15\textwidth]{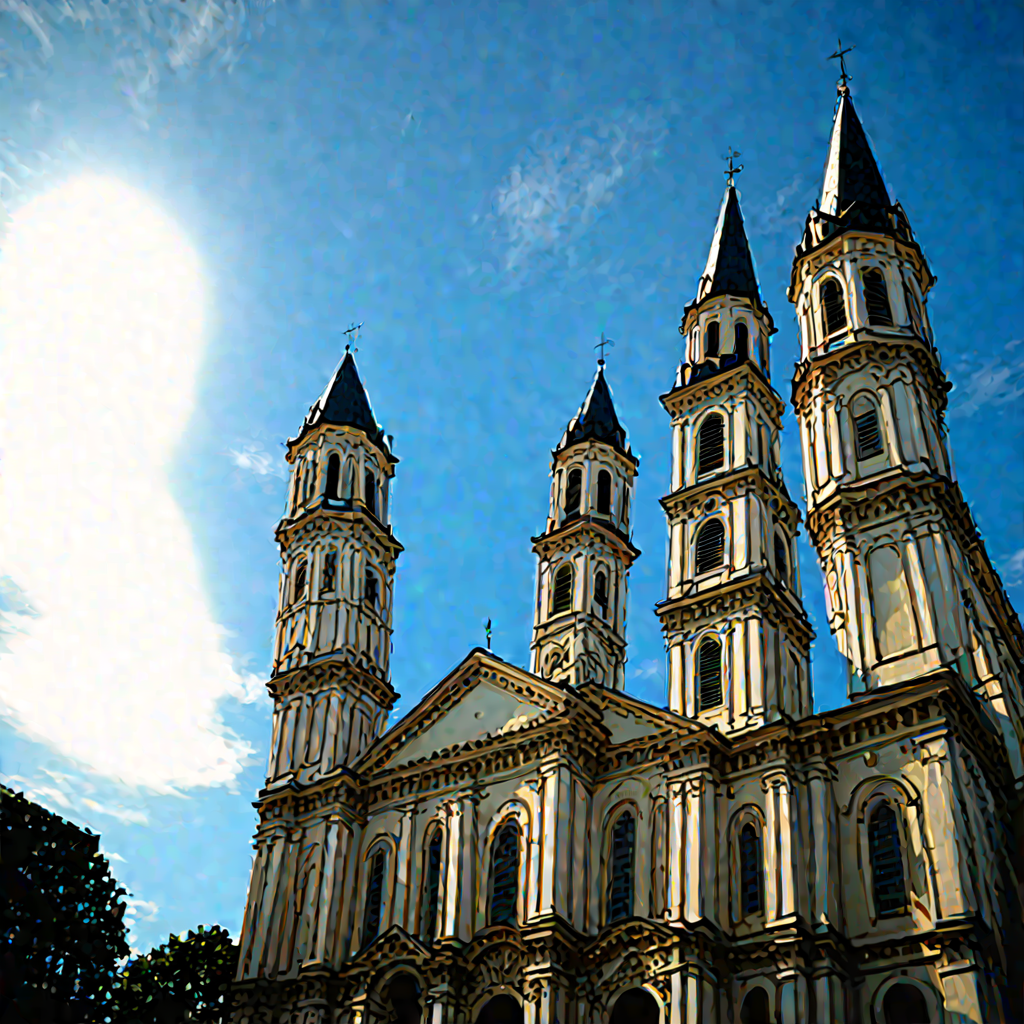} \\

        \rule{0pt}{0pt} \\

        \hline
    \end{tabular}
    \captionof{figure}{
        Failure cases of SD-Turbo and SDXL-Turbo under the optimal re-weighting schedules. 
    }
    \label{fig-failure_case}
\end{table*}

\subsection{Importance-based Re-weighting Schedule Details}

\paragraph{Qualitative Results}

The qualitative results shown in Fig.~\ref{fig-importance_based_reweighting_sdturbo_appx_1} and Fig.~\ref{fig-importance_based_reweighting_sdturbo_appx_2} are generated using 2-step-inference SD-Turbo under the following settings: 

\begin{itemize}
    \item \textbf{anime}: with prompt ``\emph{Walter White dressed as a medievalstyle king.}". 

    \item \textbf{concept-art}: with prompt ``\emph{Portrait of Guts from Berserk submerged in red water.}". 
    
    \item \textbf{paintings}: with prompt ``\emph{Male playing piano with audience surrounded by paintings by Gaston Bussiere, Craig Mullins, and J.C. Leyendecker.}". 

    \item \textbf{photo}: with prompt ``\emph{An old classic church is in front a big blue sky.}". 
\end{itemize}

It can be observed that our re-weighting schedule enhances the aesthetic quality of the samples (anime and photo), improves clarity (concept-art), and reduces background anomalies (paintings). 

The qualitative results shown in Fig.~\ref{fig-importance_based_reweighting_sdxlturbo_appx_1} and Fig.~\ref{fig-importance_based_reweighting_sdxlturbo_appx_2} are generated using 2-step-inference SDXL-Turbo under the following settings: 

\begin{itemize}
    \item \textbf{anime}: with prompt ``\emph{A cute anthropomorphic bear knight wearing a cape and crown in pale blue armor.}". 

    \item \textbf{concept-art}: with prompt ``\emph{A digital concept art of a machinist in uniform with a scifi repair tool and glowing lights.}". 
    
    \item \textbf{paintings}: with prompt ``\emph{A group of fairies playing cards on a table in a moonlit forest next to a pond filled with water lilies, artwork by Ida Rentoul Outhwaite.}". 

    \item \textbf{photo}: with prompt ``\emph{Two cats chill in the bathtub one is laying down. }". 
\end{itemize}

It can also be observed that our re-weighting schedule enhances the aesthetic quality of the samples (anime and concept-art), improves prompt alignment (paintings), and reduces anomalies in the main subjects (photo). 

% importance-based re-weighting, SD-Turbo, 1
\begin{table*}[t]
    \centering
    \begin{tabular}{c | c c c c}
        \hline

        \textbf{Re-Weighting} & \multicolumn{4}{c}{\textbf{SD-Turbo}} \\
        \textbf{Strategy} & anime & concept-art & paintings & photo \\
        
        \hline

        \rule{0pt}{0pt} \\
        
        % Vanilla
        \parbox[t][-2.75cm][c]{2.0cm}{\centering Vanilla} & 
        \includegraphics[width=0.15\textwidth]{algorithm-figure-table/importance_based_reweighting/sd-turbo/anime/default.png} & 
        \includegraphics[width=0.15\textwidth]{algorithm-figure-table/importance_based_reweighting/sd-turbo/concept-art/default.png} & 
        \includegraphics[width=0.15\textwidth]{algorithm-figure-table/importance_based_reweighting/sd-turbo/paintings/default.png} & 
        \includegraphics[width=0.15\textwidth]{algorithm-figure-table/importance_based_reweighting/sd-turbo/photo/default.png} \\

        \rule{0pt}{0pt} \\

        \hdashline

        \rule{0pt}{0pt} \\
            
        % [0.95, 1.1]
        \parbox[t][-2.75cm][c]{2.0cm}{\centering $[0.95, 1.1]$} & 
        \includegraphics[width=0.15\textwidth]{algorithm-figure-table/importance_based_reweighting/sd-turbo/anime/0.95_1.1.png} & 
        \includegraphics[width=0.15\textwidth]{algorithm-figure-table/importance_based_reweighting/sd-turbo/concept-art/0.95_1.1.png} & 
        \includegraphics[width=0.15\textwidth]{algorithm-figure-table/importance_based_reweighting/sd-turbo/paintings/0.95_1.1.png} & 
        \includegraphics[width=0.15\textwidth]{algorithm-figure-table/importance_based_reweighting/sd-turbo/photo/0.95_1.1.png} \\

        % [0.96, 1.1]
        \parbox[t][-2.75cm][c]{2.0cm}{\centering $[0.96, 1.1]$} & 
        \includegraphics[width=0.15\textwidth]{algorithm-figure-table/importance_based_reweighting/sd-turbo/anime/0.96_1.1.png} & 
        \includegraphics[width=0.15\textwidth]{algorithm-figure-table/importance_based_reweighting/sd-turbo/concept-art/0.96_1.1.png} & 
        \includegraphics[width=0.15\textwidth]{algorithm-figure-table/importance_based_reweighting/sd-turbo/paintings/0.96_1.1.png} & 
        \includegraphics[width=0.15\textwidth]{algorithm-figure-table/importance_based_reweighting/sd-turbo/photo/0.96_1.1.png} \\

        % [0.97, 1.1]
        \parbox[t][-2.75cm][c]{2.0cm}{\centering $[0.97, 1.1]$} & 
        \includegraphics[width=0.15\textwidth]{algorithm-figure-table/importance_based_reweighting/sd-turbo/anime/0.97_1.1.png} & 
        \includegraphics[width=0.15\textwidth]{algorithm-figure-table/importance_based_reweighting/sd-turbo/concept-art/0.97_1.1.png} & 
        \includegraphics[width=0.15\textwidth]{algorithm-figure-table/importance_based_reweighting/sd-turbo/paintings/0.97_1.1.png} & 
        \includegraphics[width=0.15\textwidth]{algorithm-figure-table/importance_based_reweighting/sd-turbo/photo/0.97_1.1.png} \\

        % [0.98, 1.1]
        \parbox[t][-2.75cm][c]{2.0cm}{\centering $[0.98, 1.1]$} & 
        \includegraphics[width=0.15\textwidth]{algorithm-figure-table/importance_based_reweighting/sd-turbo/anime/0.98_1.1.png} & 
        \includegraphics[width=0.15\textwidth]{algorithm-figure-table/importance_based_reweighting/sd-turbo/concept-art/0.98_1.1.png} & 
        \includegraphics[width=0.15\textwidth]{algorithm-figure-table/importance_based_reweighting/sd-turbo/paintings/0.98_1.1.png} & 
        \includegraphics[width=0.15\textwidth]{algorithm-figure-table/importance_based_reweighting/sd-turbo/photo/0.98_1.1.png} \\

        % [0.99, 1.1]
        \parbox[t][-2.75cm][c]{2.0cm}{\centering $[0.99, 1.1]$} & 
        \includegraphics[width=0.15\textwidth]{algorithm-figure-table/importance_based_reweighting/sd-turbo/anime/0.99_1.1.png} & 
        \includegraphics[width=0.15\textwidth]{algorithm-figure-table/importance_based_reweighting/sd-turbo/concept-art/0.99_1.1.png} & 
        \includegraphics[width=0.15\textwidth]{algorithm-figure-table/importance_based_reweighting/sd-turbo/paintings/0.99_1.1.png} & 
        \includegraphics[width=0.15\textwidth]{algorithm-figure-table/importance_based_reweighting/sd-turbo/photo/0.99_1.1.png} \\

        % [1.0, 1.1]
        \parbox[t][-2.75cm][c]{2.0cm}{\centering $[1.0, 1.1]$} & 
        \includegraphics[width=0.15\textwidth]{algorithm-figure-table/importance_based_reweighting/sd-turbo/anime/1.0_1.1.png} & 
        \includegraphics[width=0.15\textwidth]{algorithm-figure-table/importance_based_reweighting/sd-turbo/concept-art/1.0_1.1.png} & 
        \includegraphics[width=0.15\textwidth]{algorithm-figure-table/importance_based_reweighting/sd-turbo/paintings/1.0_1.1.png} & 
        \includegraphics[width=0.15\textwidth]{algorithm-figure-table/importance_based_reweighting/sd-turbo/photo/1.0_1.1.png} \\

        \rule{0pt}{0pt} \\

        \hline
    \end{tabular}
    \captionof{figure}{
        Samples synthesized by 2-step-inference SD-Turbo under difference re-weighting schedule. 
    }
    \label{fig-importance_based_reweighting_sdturbo_appx_1}
\end{table*}

% importance-based re-weighting, SD-Turbo, 2
% importance-based re-weighting, SD-Turbo, 2
\begin{table*}[t]
    \centering
    \begin{tabular}{c | c c c c}
        \hline

        \textbf{Re-Weighting} & \multicolumn{4}{c}{\textbf{SD-Turbo}} \\
        \textbf{Strategy} & anime & concept-art & paintings & photo \\
        
        \hline

        \rule{0pt}{0pt} \\
        
        % [1.01, 1.1]
        \parbox[t][-2.75cm][c]{2.0cm}{\centering $[1.01, 1.1]$} & 
        \includegraphics[width=0.15\textwidth]{algorithm-figure-table/importance_based_reweighting/sd-turbo/anime/1.01_1.1.png} & 
        \includegraphics[width=0.15\textwidth]{algorithm-figure-table/importance_based_reweighting/sd-turbo/concept-art/1.01_1.1.png} & 
        \includegraphics[width=0.15\textwidth]{algorithm-figure-table/importance_based_reweighting/sd-turbo/paintings/1.01_1.1.png} & 
        \includegraphics[width=0.15\textwidth]{algorithm-figure-table/importance_based_reweighting/sd-turbo/photo/1.01_1.1.png} \\

        % [1.02, 1.1]
        \parbox[t][-2.75cm][c]{2.0cm}{\centering $[1.02, 1.1]$} & 
        \includegraphics[width=0.15\textwidth]{algorithm-figure-table/importance_based_reweighting/sd-turbo/anime/1.02_1.1.png} & 
        \includegraphics[width=0.15\textwidth]{algorithm-figure-table/importance_based_reweighting/sd-turbo/concept-art/1.02_1.1.png} & 
        \includegraphics[width=0.15\textwidth]{algorithm-figure-table/importance_based_reweighting/sd-turbo/paintings/1.02_1.1.png} & 
        \includegraphics[width=0.15\textwidth]{algorithm-figure-table/importance_based_reweighting/sd-turbo/photo/1.02_1.1.png} \\

        % [1.03, 1.1]
        \parbox[t][-2.75cm][c]{2.0cm}{\centering $[1.03, 1.1]$} & 
        \includegraphics[width=0.15\textwidth]{algorithm-figure-table/importance_based_reweighting/sd-turbo/anime/1.03_1.1.png} & 
        \includegraphics[width=0.15\textwidth]{algorithm-figure-table/importance_based_reweighting/sd-turbo/concept-art/1.03_1.1.png} & 
        \includegraphics[width=0.15\textwidth]{algorithm-figure-table/importance_based_reweighting/sd-turbo/paintings/1.03_1.1.png} & 
        \includegraphics[width=0.15\textwidth]{algorithm-figure-table/importance_based_reweighting/sd-turbo/photo/1.03_1.1.png} \\

        % [1.04, 1.1]
        \parbox[t][-2.75cm][c]{2.0cm}{\centering $[1.04, 1.1]$} & 
        \includegraphics[width=0.15\textwidth]{algorithm-figure-table/importance_based_reweighting/sd-turbo/anime/1.04_1.1.png} & 
        \includegraphics[width=0.15\textwidth]{algorithm-figure-table/importance_based_reweighting/sd-turbo/concept-art/1.04_1.1.png} & 
        \includegraphics[width=0.15\textwidth]{algorithm-figure-table/importance_based_reweighting/sd-turbo/paintings/1.04_1.1.png} & 
        \includegraphics[width=0.15\textwidth]{algorithm-figure-table/importance_based_reweighting/sd-turbo/photo/1.04_1.1.png} \\

        % [1.05, 1.1]
        \parbox[t][-2.75cm][c]{2.0cm}{\centering $[1.05, 1.1]$} & 
        \includegraphics[width=0.15\textwidth]{algorithm-figure-table/importance_based_reweighting/sd-turbo/anime/1.05_1.1.png} & 
        \includegraphics[width=0.15\textwidth]{algorithm-figure-table/importance_based_reweighting/sd-turbo/concept-art/1.05_1.1.png} & 
        \includegraphics[width=0.15\textwidth]{algorithm-figure-table/importance_based_reweighting/sd-turbo/paintings/1.05_1.1.png} & 
        \includegraphics[width=0.15\textwidth]{algorithm-figure-table/importance_based_reweighting/sd-turbo/photo/1.05_1.1.png} \\

        \rule{0pt}{0pt} \\

        \hdashline

        \rule{0pt}{0pt} \\

        % [0.98, 1.15]
        \parbox[t][-2.75cm][c]{2.0cm}{\centering $[0.98, 1.15]$} & 
        \includegraphics[width=0.15\textwidth]{algorithm-figure-table/importance_based_reweighting/sd-turbo/anime/0.98_1.15.png} & 
        \includegraphics[width=0.15\textwidth]{algorithm-figure-table/importance_based_reweighting/sd-turbo/concept-art/0.98_1.15.png} & 
        \includegraphics[width=0.15\textwidth]{algorithm-figure-table/importance_based_reweighting/sd-turbo/paintings/0.98_1.15.png} & 
        \includegraphics[width=0.15\textwidth]{algorithm-figure-table/importance_based_reweighting/sd-turbo/photo/0.98_1.15.png} \\

        % [0.98, 1.2]
        \parbox[t][-2.75cm][c]{2.0cm}{\centering $[0.98, 1.2]$} & 
        \includegraphics[width=0.15\textwidth]{algorithm-figure-table/importance_based_reweighting/sd-turbo/anime/0.98_1.2.png} & 
        \includegraphics[width=0.15\textwidth]{algorithm-figure-table/importance_based_reweighting/sd-turbo/concept-art/0.98_1.2.png} & 
        \includegraphics[width=0.15\textwidth]{algorithm-figure-table/importance_based_reweighting/sd-turbo/paintings/0.98_1.2.png} & 
        \includegraphics[width=0.15\textwidth]{algorithm-figure-table/importance_based_reweighting/sd-turbo/photo/0.98_1.2.png} \\

        \rule{0pt}{0pt} \\

        \hline
    \end{tabular}
    \captionof{figure}{
        Samples synthesized by 2-step-inference SD-Turbo under difference re-weighting schedule (cont.). 
    }
    \label{fig-importance_based_reweighting_sdturbo_appx_2}
\end{table*}

% importance-based re-weighting, SDXL-Turbo, 1
% importance-based re-weighting, SDXL-Turbo, 1
\begin{table*}[t]
    \centering
    \begin{tabular}{c | c c c c}
        \hline

        \textbf{Re-Weighting} & \multicolumn{4}{c}{\textbf{SDXL-Turbo}} \\
        \textbf{Strategy} & anime & concept-art & paintings & photo \\
        
        \hline

        \rule{0pt}{0pt} \\
        
        % Vanilla
        \parbox[t][-2.75cm][c]{2.0cm}{\centering Vanilla} & 
        \includegraphics[width=0.15\textwidth]{algorithm-figure-table/importance_based_reweighting/sdxl-turbo/anime/default.png} & 
        \includegraphics[width=0.15\textwidth]{algorithm-figure-table/importance_based_reweighting/sdxl-turbo/concept-art/default.png} & 
        \includegraphics[width=0.15\textwidth]{algorithm-figure-table/importance_based_reweighting/sdxl-turbo/paintings/default.png} & 
        \includegraphics[width=0.15\textwidth]{algorithm-figure-table/importance_based_reweighting/sdxl-turbo/photo/default.png} \\

        \rule{0pt}{0pt} \\

        \hdashline

        \rule{0pt}{0pt} \\
            
        % [0.95, 1.1]
        \parbox[t][-2.75cm][c]{2.0cm}{\centering $[0.95, 1.1]$} & 
        \includegraphics[width=0.15\textwidth]{algorithm-figure-table/importance_based_reweighting/sdxl-turbo/anime/0.95_1.1.png} & 
        \includegraphics[width=0.15\textwidth]{algorithm-figure-table/importance_based_reweighting/sdxl-turbo/concept-art/0.95_1.1.png} & 
        \includegraphics[width=0.15\textwidth]{algorithm-figure-table/importance_based_reweighting/sdxl-turbo/paintings/0.95_1.1.png} & 
        \includegraphics[width=0.15\textwidth]{algorithm-figure-table/importance_based_reweighting/sdxl-turbo/photo/0.95_1.1.png} \\

        % [0.96, 1.1]
        \parbox[t][-2.75cm][c]{2.0cm}{\centering $[0.96, 1.1]$} & 
        \includegraphics[width=0.15\textwidth]{algorithm-figure-table/importance_based_reweighting/sdxl-turbo/anime/0.96_1.1.png} & 
        \includegraphics[width=0.15\textwidth]{algorithm-figure-table/importance_based_reweighting/sdxl-turbo/concept-art/0.96_1.1.png} & 
        \includegraphics[width=0.15\textwidth]{algorithm-figure-table/importance_based_reweighting/sdxl-turbo/paintings/0.96_1.1.png} & 
        \includegraphics[width=0.15\textwidth]{algorithm-figure-table/importance_based_reweighting/sdxl-turbo/photo/0.96_1.1.png} \\

        % [0.97, 1.1]
        \parbox[t][-2.75cm][c]{2.0cm}{\centering $[0.97, 1.1]$} & 
        \includegraphics[width=0.15\textwidth]{algorithm-figure-table/importance_based_reweighting/sdxl-turbo/anime/0.97_1.1.png} & 
        \includegraphics[width=0.15\textwidth]{algorithm-figure-table/importance_based_reweighting/sdxl-turbo/concept-art/0.97_1.1.png} & 
        \includegraphics[width=0.15\textwidth]{algorithm-figure-table/importance_based_reweighting/sdxl-turbo/paintings/0.97_1.1.png} & 
        \includegraphics[width=0.15\textwidth]{algorithm-figure-table/importance_based_reweighting/sdxl-turbo/photo/0.97_1.1.png} \\

        % [0.98, 1.1]
        \parbox[t][-2.75cm][c]{2.0cm}{\centering $[0.98, 1.1]$} & 
        \includegraphics[width=0.15\textwidth]{algorithm-figure-table/importance_based_reweighting/sdxl-turbo/anime/0.98_1.1.png} & 
        \includegraphics[width=0.15\textwidth]{algorithm-figure-table/importance_based_reweighting/sdxl-turbo/concept-art/0.98_1.1.png} & 
        \includegraphics[width=0.15\textwidth]{algorithm-figure-table/importance_based_reweighting/sdxl-turbo/paintings/0.98_1.1.png} & 
        \includegraphics[width=0.15\textwidth]{algorithm-figure-table/importance_based_reweighting/sdxl-turbo/photo/0.98_1.1.png} \\

        % [0.99, 1.1]
        \parbox[t][-2.75cm][c]{2.0cm}{\centering $[0.99, 1.1]$} & 
        \includegraphics[width=0.15\textwidth]{algorithm-figure-table/importance_based_reweighting/sdxl-turbo/anime/0.99_1.1.png} & 
        \includegraphics[width=0.15\textwidth]{algorithm-figure-table/importance_based_reweighting/sdxl-turbo/concept-art/0.99_1.1.png} & 
        \includegraphics[width=0.15\textwidth]{algorithm-figure-table/importance_based_reweighting/sdxl-turbo/paintings/0.99_1.1.png} & 
        \includegraphics[width=0.15\textwidth]{algorithm-figure-table/importance_based_reweighting/sdxl-turbo/photo/0.99_1.1.png} \\

        % [1.0, 1.1]
        \parbox[t][-2.75cm][c]{2.0cm}{\centering $[1.0, 1.1]$} & 
        \includegraphics[width=0.15\textwidth]{algorithm-figure-table/importance_based_reweighting/sdxl-turbo/anime/1.0_1.1.png} & 
        \includegraphics[width=0.15\textwidth]{algorithm-figure-table/importance_based_reweighting/sdxl-turbo/concept-art/1.0_1.1.png} & 
        \includegraphics[width=0.15\textwidth]{algorithm-figure-table/importance_based_reweighting/sdxl-turbo/paintings/1.0_1.1.png} & 
        \includegraphics[width=0.15\textwidth]{algorithm-figure-table/importance_based_reweighting/sdxl-turbo/photo/1.0_1.1.png} \\

        \rule{0pt}{0pt} \\

        \hline
    \end{tabular}
    \captionof{figure}{
        Samples synthesized by 2-step-inference SD-Turbo under difference re-weighting schedule. 
    }
    \label{fig-importance_based_reweighting_sdxlturbo_appx_1}
\end{table*}

% importance-based re-weighting, SDXL-Turbo, 2
% importance-based re-weighting, SDXL-Turbo, 2
\begin{table*}[t]
    \centering
    \begin{tabular}{c | c c c c}
        \hline

        \textbf{Re-Weighting} & \multicolumn{4}{c}{\textbf{SDXL-Turbo}} \\
        \textbf{Strategy} & anime & concept-art & paintings & photo \\
        
        \hline

        \rule{0pt}{0pt} \\
        
        % [1.01, 1.1]
        \parbox[t][-2.75cm][c]{2.0cm}{\centering $[1.01, 1.1]$} & 
        \includegraphics[width=0.15\textwidth]{algorithm-figure-table/importance_based_reweighting/sdxl-turbo/anime/1.01_1.1.png} & 
        \includegraphics[width=0.15\textwidth]{algorithm-figure-table/importance_based_reweighting/sdxl-turbo/concept-art/1.01_1.1.png} & 
        \includegraphics[width=0.15\textwidth]{algorithm-figure-table/importance_based_reweighting/sdxl-turbo/paintings/1.01_1.1.png} & 
        \includegraphics[width=0.15\textwidth]{algorithm-figure-table/importance_based_reweighting/sdxl-turbo/photo/1.01_1.1.png} \\

        % [1.02, 1.1]
        \parbox[t][-2.75cm][c]{2.0cm}{\centering $[1.02, 1.1]$} & 
        \includegraphics[width=0.15\textwidth]{algorithm-figure-table/importance_based_reweighting/sdxl-turbo/anime/1.02_1.1.png} & 
        \includegraphics[width=0.15\textwidth]{algorithm-figure-table/importance_based_reweighting/sdxl-turbo/concept-art/1.02_1.1.png} & 
        \includegraphics[width=0.15\textwidth]{algorithm-figure-table/importance_based_reweighting/sdxl-turbo/paintings/1.02_1.1.png} & 
        \includegraphics[width=0.15\textwidth]{algorithm-figure-table/importance_based_reweighting/sdxl-turbo/photo/1.02_1.1.png} \\

        % [1.03, 1.1]
        \parbox[t][-2.75cm][c]{2.0cm}{\centering $[1.03, 1.1]$} & 
        \includegraphics[width=0.15\textwidth]{algorithm-figure-table/importance_based_reweighting/sdxl-turbo/anime/1.03_1.1.png} & 
        \includegraphics[width=0.15\textwidth]{algorithm-figure-table/importance_based_reweighting/sdxl-turbo/concept-art/1.03_1.1.png} & 
        \includegraphics[width=0.15\textwidth]{algorithm-figure-table/importance_based_reweighting/sdxl-turbo/paintings/1.03_1.1.png} & 
        \includegraphics[width=0.15\textwidth]{algorithm-figure-table/importance_based_reweighting/sdxl-turbo/photo/1.03_1.1.png} \\

        % [1.04, 1.1]
        \parbox[t][-2.75cm][c]{2.0cm}{\centering $[1.04, 1.1]$} & 
        \includegraphics[width=0.15\textwidth]{algorithm-figure-table/importance_based_reweighting/sdxl-turbo/anime/1.04_1.1.png} & 
        \includegraphics[width=0.15\textwidth]{algorithm-figure-table/importance_based_reweighting/sdxl-turbo/concept-art/1.04_1.1.png} & 
        \includegraphics[width=0.15\textwidth]{algorithm-figure-table/importance_based_reweighting/sdxl-turbo/paintings/1.04_1.1.png} & 
        \includegraphics[width=0.15\textwidth]{algorithm-figure-table/importance_based_reweighting/sdxl-turbo/photo/1.04_1.1.png} \\

        % [1.05, 1.1]
        \parbox[t][-2.75cm][c]{2.0cm}{\centering $[1.05, 1.1]$} & 
        \includegraphics[width=0.15\textwidth]{algorithm-figure-table/importance_based_reweighting/sdxl-turbo/anime/1.05_1.1.png} & 
        \includegraphics[width=0.15\textwidth]{algorithm-figure-table/importance_based_reweighting/sdxl-turbo/concept-art/1.05_1.1.png} & 
        \includegraphics[width=0.15\textwidth]{algorithm-figure-table/importance_based_reweighting/sdxl-turbo/paintings/1.05_1.1.png} & 
        \includegraphics[width=0.15\textwidth]{algorithm-figure-table/importance_based_reweighting/sdxl-turbo/photo/1.05_1.1.png} \\

        \rule{0pt}{0pt} \\

        \hdashline

        \rule{0pt}{0pt} \\

        % [0.95, 1.15]
        \parbox[t][-2.75cm][c]{2.0cm}{\centering $[0.95, 1.15]$} & 
        \includegraphics[width=0.15\textwidth]{algorithm-figure-table/importance_based_reweighting/sdxl-turbo/anime/0.95_1.15.png} & 
        \includegraphics[width=0.15\textwidth]{algorithm-figure-table/importance_based_reweighting/sdxl-turbo/concept-art/0.95_1.15.png} & 
        \includegraphics[width=0.15\textwidth]{algorithm-figure-table/importance_based_reweighting/sdxl-turbo/paintings/0.95_1.15.png} & 
        \includegraphics[width=0.15\textwidth]{algorithm-figure-table/importance_based_reweighting/sdxl-turbo/photo/0.95_1.15.png} \\

        % [0.95, 1.2]
        \parbox[t][-2.75cm][c]{2.0cm}{\centering $[0.95, 1.2]$} & 
        \includegraphics[width=0.15\textwidth]{algorithm-figure-table/importance_based_reweighting/sdxl-turbo/anime/0.95_1.2.png} & 
        \includegraphics[width=0.15\textwidth]{algorithm-figure-table/importance_based_reweighting/sdxl-turbo/concept-art/0.95_1.2.png} & 
        \includegraphics[width=0.15\textwidth]{algorithm-figure-table/importance_based_reweighting/sdxl-turbo/paintings/0.95_1.2.png} & 
        \includegraphics[width=0.15\textwidth]{algorithm-figure-table/importance_based_reweighting/sdxl-turbo/photo/0.95_1.2.png} \\

        \rule{0pt}{0pt} \\

        \hline
    \end{tabular}
    \captionof{figure}{
        Samples synthesized by 2-step-inference SDXL-Turbo under difference re-weighting schedule (cont.). 
    }
    \label{fig-importance_based_reweighting_sdxlturbo_appx_2}
\end{table*}

\paragraph{Impacts of Parameters}

Fixing the upper bound $high$ of the weight range $[low, high]$, it can be observed that, as $low$ increases, the samples become clearer and sharper with more saturated colors. 
However, an excessively large $low$ may introduce anomalies, and lead to over-saturation of colors. 

Fixing the lower bound $low$ of the optimal re-weighting schedule ($low = 0.98$ for SD, and $low = 0.95$ for SDXL), it can be observed that, as $high$ increases, the colors in the samples become more saturated. 
An excessively large $high$ may also lead to over-saturation.

We provide the following empirical guidelines for selecting the range $[low, high]$: set $low$ slightly below $1.0$, and choose $high$ within the range $(1.0, 1.15)$. 

\paragraph{Failure Cases}

We present failure cases for SD-Turbo and SDXL-Turbo under their respective optimal re-weighting schedules, with samples generated under the following settings: 

\begin{itemize}
    \item \textbf{SD-Turbo}: 2-step inference with prompt ``\emph{A chicken smoking from a bong.}" under the re-weighting schedules of vanilla, $[0.98, 1.1]$, $[0.98, 1.15]$ and $[0.98, 1.2]$. 

    \item \textbf{SDXL-Turbo}: 2-step inference with prompt ``\emph{An old classic church is in front a big blue sky.}" under the re-weighting schedules of vanilla, $[0.95, 1.1]$, $[0.95, 1.15]$ and $[0.95, 1.2]$. 
\end{itemize}

It can be observed that, all our re-weighting schedules introduces anomalies in these cases. 

\subsection{Limitations}

Our importance-based re-weighting schedule essentially serves as an enhancement of the U-Net's inherent capabilities, which may account for our method's ability to achieve aesthetic enhancement while maintaining identity consistency. 

Consequently, the effects of re-weighting are partially contingent upon the quality of the original denoising trajectory. 
If the original trajectory leads to a low-quality region, our method may potentially further degrade the sampling quality.
