# Supplementary material for: Dynamic Importance in Diffusion U-Net for Enhanced Image Synthesis
Source: arXiv:2504.03471 source file (2025-05-05)
Supplement: Supplementary file 5 [file implementation_details.tex]

\section{Experiment Setup and Configuration}
\label{appx_sec-experimental_setup_and_model_configuration}

This section provides the implementation details of our experiments to facilitate the reproduction.

\subsection{Pre-trained Models}

We selected the following pre-trained models as fundamental models in this project: 

\begin{itemize}
    \item \textbf{stabilityai/sd-turbo}~\cite{sauer2023adversarialdiffusiondistillation} at \\
    \href{https://huggingface.co/stabilityai/sd-turbo}{https://huggingface.co/stabilityai/sd-turbo}. 

    \item \textbf{stabilityai/sdxl-turbo}~\cite{sauer2024fasthighresolutionimagesynthesis} at \\
    \href{https://huggingface.co/stabilityai/sdxl-turbo}{https://huggingface.co/stabilityai/sdxl-turbo}. 

    \item \textbf{stabilityai/stable-diffusion-2-1-base}~\cite{rombach2022highresolutionimagesynthesislatent} at \\
    \href{https://huggingface.co/stabilityai/stable-diffusion-2-1-base}{https://huggingface.co/stabilityai/stable-diffusion-2-1-base}. 

    \item \textbf{stabilityai/stable-diffusion-xl-base-1.0}~\cite{podell2023sdxlimprovinglatentdiffusion} at \\ 
    \href{https://huggingface.co/stabilityai/stable-diffusion-xl-base-1.0}{https://huggingface.co/stabilityai/stable-diffusion-xl-base-1.0}. 
\end{itemize}

We employ the fp16 versions of the aforementioned models for fine-tuning and inference. 

\subsection{Metric Computation}

We utilized the following third-party libraries for metric computation: 

\begin{itemize}
    \item \textbf{Human Preference Score v2} (1.2.0)~\cite{wu2023humanpreferencescorev2} at \\
    \href{https://github.com/tgxs002/HPSv2}{https://github.com/tgxs002/HPSv2}. 

    \item \text{pytorch-fid} (0.3.0)~\cite{yu2021frechet} at \\
    \href{https://github.com/mseitzer/pytorch-fid}{https://github.com/mseitzer/pytorch-fid}. 

    \item \text{lpips} (0.1.4)~\cite{zhang2018unreasonable} at \\ 
    \href{https://github.com/richzhang/PerceptualSimilarity}{https://github.com/richzhang/PerceptualSimilarity}. 
\end{itemize}

\subsection{Implementation}

We modified the the HuggingFace diffusers~\cite{von-platen-etal-2022-diffusers} library for implementation in this project.
