# Supplementary material for: Dynamic Importance in Diffusion U-Net for Enhanced Image Synthesis
Source: arXiv:2504.03471 source file (2025-05-05)
Supplement: Supplementary file 6 [file importance_probe_details.tex]

\section{More details of Importance Probe}
\label{appx_sec-the_methodology_and_implementation_of_importance_probe}

\subsection{Pseudo-Code of Importance Probe}

The pseudo-code of Importance Probe (IP) is summarized in Algo.~\ref{alg-weight_threshold_update}. 

% ---------= 伪代码中出现的操作 =---------
% 多参数 Input 的首个参数
\newcommand{\MultiInput}[1]{
  \textbf{Input:} 
  \begin{itemize}[leftmargin = 2em, noitemsep, topsep = 0pt]
    \item #1
  \end{itemize}
}

% 多参数 Output 的首个参数

% 增加参数
\newcommand{\AddItem}[1]{
  \begin{itemize}[leftmargin = 2em, noitemsep, topsep = 0pt]
    \item #1
  \end{itemize}
}

% 阈值更新过程伪代码
\begin{algorithm}
\caption{Importance Probe in a Epoch}
    % Input
    \MultiInput{\text{weight\_threshold\_matrix}}
    \AddItem{\text{history\_best\_weight\_matrix}}
    \AddItem{\text{letents}, \text{conditions}}

    \vspace{5pt}
    
    \begin{algorithmic}[1]
        \State $\text{weight\_threshold\_list} \newline
        \hspace*{10pt} \leftarrow \text{weight\_threshold\_matrix}[\text{inference\_step}]$
        \State $\text{best\_fitness} \leftarrow \text{cal\_fitness}(\text{weight\_threshold\_list})$
        \State
        \State $\text{best\_weight\_list} \leftarrow \varnothing$
        \State $\text{accepted\_mask} \leftarrow [\text{False}] \times \text{num\_inference\_step}$

        \State
        
        \For{$\text{inference\_step} = 0$ to $(\text{num\_inference\_step} - 1)$}
            \State $\text{time\_step} \leftarrow \text{time\_steps}[\text{inference\_step}]$
            \State $\epsilon_{\text{tea}} \leftarrow \text{tea\_U-Net}(\text{letents}, \text{conditions}, \text{time\_step})$
            
            \State 
            
            \State $\text{cur\_weight\_list} \newline 
            \hspace*{20pt} \leftarrow \text{history\_best\_weight\_matrix}[\text{inference\_step}]$
            
            \For{$\text{stu\_try} = 1$ to $(\text{num\_stu\_try} - 1)$}
                \State $\text{weight\_list}$ \newline 
                    \hspace*{40pt} $\leftarrow \text{WeightBiasSchedule}(\text{cur\_weight\_list})$ 
                
                \State $\text{stu\_U-Net.set\_weight}(\text{weight\_list})$
                
                \State $\epsilon_{\text{stu}} \leftarrow \text{stu\_U-Net}(\text{letents},  \text{conditions}, \text{time\_step})$

                \State 
                
                \If{$\text{criterion}(\epsilon_{\text{tea}}, \epsilon_{\text{stu}}) \leq \text{loss\_threshold}$}
                    \State $\text{tmp\_fitness} = \text{cal\_fitness}(\text{weight\_list})$
                    \If{$\text{tmp\_fitness} > \text{best\_fitness}$}
                        \State $\text{best\_fitness} \leftarrow \text{tmp\_fitness}$
                        \State $\text{best\_weight\_list} \leftarrow \text{weight\_list}$
                    \EndIf
                \EndIf
            \EndFor
            \State
            \If{$\text{best\_weight\_list} == \varnothing$}
                \State $\text{weight\_threshold\_matrix}[\text{inference\_step}]$ \newline
                    \hspace*{40pt} $\leftarrow \text{cur\_weight\_list}$
            \Else
                \State $\text{accepted\_mask}[\text{inference\_step}] \leftarrow \text{True}$
                \State $\text{weight\_threshold\_matrix}[\text{inference\_step}]$ \newline
                    \hspace*{40pt} $\leftarrow \text{best\_weight\_list}$
                \State $\text{history\_best\_weight\_matrix}[\text{inference\_step}]$ \newline
                    \hspace*{40pt} $\leftarrow \text{best\_weight\_list}$
            \EndIf

            \State 

            \State $\text{latents} \leftarrow \text{scheduler.step}(\text{latents}, \epsilon_{\text{tea}}, \text{time\_step})$
        \EndFor

        \State 

        \State $\text{weight\_threshold\_matrix}$ \newline
            \hspace*{10pt} $\leftarrow \text{ThresholdUpdateScheduler}(\text{accepted\_mask})$
    \end{algorithmic}
\label{alg-weight_threshold_update}
\end{algorithm}

\subsection{Threshold Update Schedule}

Let ``the weight set is accepted" to be event $A$, and ``the current threshold being too high, moderate, or too low" be events $B_1$, $B_2$ and $B_3$, respectively. 

Let $Q = [\pmb{q}_1, \cdots, \pmb{q}_n]$ be the current optimal threshold matrix, where $n$ is the number of inference steps and $\pmb{q}_i \in [0, 1]^m\ \ (1 \leq i \leq n)$ stands for the optimal thresholds for the $m$ target blocks. 

If an optimal weight matrix $W = [\pmb{w}_1, \cdots, \pmb{w}_n]$ is found during an iteration, where $\pmb{w}_i \in [0, 1]^m\ \ (1 \leq i \leq n)$ represents the optimal weights for the $m$ target layers, then the new thresholds matrix $Q' = [\pmb{q}_1', \cdots, \pmb{q}_n']$ are obtained as follows:

For an accepted weight set $\pmb{w}_i$ :

\begin{equation}
    \begin{aligned}
        \pmb{q}_i' =
        &~ P(B_1 \mid A) \times (\pmb{q}_i / 2) \\
        &+ P(B_2 \mid A) \times \pmb{q}_i + P(B_3 \mid A) \times (\pmb{w}_i - \varepsilon)
    \end{aligned}, 
    \label{eq-threshold_update_accpeted}
\end{equation}
while for a rejected one $\pmb{w}_j$:
\begin{equation}
    \begin{aligned}
        \pmb{q}_j' = 
        &~ P(B_1 \mid \overline{A}) \times (\pmb{q}_j / 2) \\
        &+ P(B_2 \mid \overline{A}) \times \pmb{q}_j + P(B_3 \mid \overline{A}) \times (\pmb{w}_j - \varepsilon)
    \end{aligned}, 
    \label{eq-threshold_update_rejected}
\end{equation}
where $\varepsilon$ is a minute positive number. 

Since the thresholds tend to stabilize to moderate values during the probing process, we set $P(B_2 \mid A)$ in Eq.~\ref{eq-threshold_update_accpeted} to linearly increase from $P_{\text{st}} (B_2 \mid A)$ to $P_{\text{ed}} (B_2 \mid A)$, and $P(B_3 \mid A)$ to linearly decrease from $P_{\text{st}} (B_3 \mid A)$ to $P_{\text{ed}} (B_3 \mid A)$. 
Similarly, in Eq.~\ref{eq-threshold_update_rejected}, $P(B_1 \mid \overline{A})$ and $P(B_2 \mid \overline{A})$ are set to decrease and increase, respectively. 

Compared to the common hard or soft update strategies, our conditional-expectation-based threshold update strategy can counteract the biases introduced by randomness in a stochastic environment, providing more reliable updates.

\subsection{Importance Ranking in a Single Run of IP}

Let $n$ and $m$ be the number of inference steps and the number of probing targets (the number of attention blocks in this study) respectively. 

We will obtain a sequence of weight threshold lists in a run of IP, denoted by $\pmb{\text{wt}} = [\pmb{\text{wt}}^{(0)}, \cdots, \pmb{\text{wt}}^{(n - 1)}]$, where $\pmb{\text{wt}}^{(t)} = [\pmb{\text{wt}}_0^{(t)}, \cdots, \pmb{\text{wt}}_{m - 1}^{(t)}]$ represents the weight thresholds for each block at denoising step $t$. 

For each inference step $t$, the \emph{importance ranking} $\pmb{\text{rk}}^{(t)}$ is derived by sorting the list of block indices $[0, \cdots, m - 1]$ based on the corresponding weight thresholds in $\text{wt}^{(t)}$ in non-descreasing order. 
For short, $\pmb{\text{rk}}^{(t)} = \mathrm{argsort}(\pmb{\text{wt}}^{(t)})$, where $\mathrm{argsort}$ returns the permutation of indices that sorts $\pmb{\text{wt}}^{(t)}$ in ascending order. 
To ensure the uniqueness of each threshold value and avoid redundancy, we introduce small random perturbations to $\pmb{\text{wt}}^{(t)}$ before computation, which ensures that no identical threshold values exist, thereby allowing for the derivation of a reasonable importance ranking for any set of threshold values.

The derived importance rankings can be represented as a sequence of vectors $\pmb{\text{rk}} = [\pmb{\text{rk}}^{(0)}, \cdots, \pmb{\text{rk}}^{(n - 1)}]$, where each vector corresponds to a permutation of $0$ to $(m - 1)$.

\subsection{Noise Prediction Tolerance \& Weight Bias Schedule}

\cite{esser2024scaling} noted that, when training diffusion models, the time steps at the beginning and end are easier to learn, while the intermediate time steps are more challenging. 

We selectively follow this observation.  
The maximum allowed tolerance for noise prediction and the maximum magnitude of perturbations in the Importance Bias Schedule are set to increase linearly along the inference progress. 
It aims to constrain the student U-Net to follow the denoising trajectory of the teacher U-Net in the early stages, while encouraging the student U-Net to explore finer image details in the later stages independently. 
This strategy enables the IP to better distinguish the importance of different blocks through larger perturbations.

In the early denoising, we choose a smaller tolerance to counteract the stochasticity in the probing process, thereby achieving faster convergence.

\subsection{Hyper-parameters}

\paragraph{Importance Probe}

For each specific task, we conduct a few runs of IP, with each round consisting of several perturbations to the weights and updates to the threshold values. 
We empirically found that the setting of $15$ runs and $20$ perturbations per run, is sufficient to achieve a relatively \emph{stable} importance ranking in the subsequent voting mechanism. 

Specifically, it can be ensured that, when the statistics from the rounds of voting are traversed in any order, the sequences of importance rankings derived from the last $5$ prefixes of each traversal have a distance no greater than $\dfrac{n}{2}$. 
The \emph{distance} of two sequences of importance rankings $\pmb{\text{rk}}_a = [\pmb{\text{rk}}_{a}^{(0)}, \cdots, \pmb{\text{rk}}_{a}^{(n - 1)}]$ and $\pmb{\text{rk}}_b = [\pmb{\text{rk}}_{b}^{(0)}, \cdots, \pmb{\text{rk}}_{b}^{(n - 1)}]$ is computed as
\begin{equation}
    \text{dist} (\pmb{\text{rk}}_a, \pmb{\text{rk}}_b)
    = 
    \sum_{t = 0}^{n - 1} \text{dist} (\pmb{\text{rk}}_{a}^{(t)}, \pmb{\text{rk}}_{b}^{(t)})
    , 
\end{equation}
where $\text{dist} (\pmb{\text{rk}}_{a}^{(t)}, \pmb{\text{rk}}_{b}^{(t)})$ is the \emph{distance} between the two importance rankings $\pmb{\text{rk}}_{a}^{(t)}$ and $\pmb{\text{rk}}_{b}^{(t)}$, which is defined as the bubble sort distance of these two permutations. 

\paragraph{Noise Prediction Tolerance \& Weight Bias Schedule}

The maximum allowed noise prediction tolerance is set to linearly increase from $1\text{e}-4$ to $2\text{e}-4$. 

The maximum magnitude of the perturbations in the Weight Bias Schedule is set to linearly increase from $0.02$ to $0.05$. 

\paragraph{Threshold Update Schedule}

We selected the following hyper-parameters for the Threshold Update Schedule across all tasks. 

\begin{table}[h]
    \centering
    \caption{
        Hyper-parameters for the Weight Threshold Update Schedule. 
    }
    \begin{tabular}{c | c}
        \hline
        Param Name & Value \\
        \hline

        $\epsilon$ & $1\text{e}-2$ \\

        \hdashline

        $P(B_1 \mid A)$ & $0.06$ \\
        $P_{\text{st}} (B_2 \mid A)$ & $0.47$ \\ 
        $P_{\text{ed}} (B_2 \mid A)$ & $0.84$ \\ 
        $P_{\text{st}} (B_3 \mid A)$ & $0.47$ \\ 
        $P_{\text{ed}} (B_3 \mid A)$ & $0.10$ \\ 

        \hdashline

        $P_{\text{st}} (B_1 \mid \overline{A})$ & $0.48$ \\ 
        $P_{\text{ed}} (B_1 \mid \overline{A})$ & $0.30$ \\ 
        $P_{\text{st}} (B_2 \mid \overline{A})$ & $0.48$ \\ 
        $P_{\text{ed}} (B_2 \mid \overline{A})$ & $0.66$ \\ 
        
        $P(B_3 \mid \overline{A})$ & $0.04$ \\ 

        \hline
    \end{tabular}
    \label{tab-hyper_parameter_weight_threshold_update_schedule}
\end{table}

\subsection{Limitations}

The Importance Probe requires multiple rounds of heuristic search, with each round involving several epochs, to counteract the influence of randomness. 
This process incurs a significant computational overhead. 

Besides, the maximum noise prediction tolerance, the maximum perturbation magnitude of the Weight Bias Schedule, and the conditional probabilities of the Threshold Update Schedule need to be empirically and manually selected, which may not be applicable to all scenarios.
