# Supplementary material for: Dynamic Importance in Diffusion U-Net for Enhanced Image Synthesis
Source: arXiv:2504.03471 source file (2025-05-05)
Supplement: Supplementary file 7 [file limitations_and_future_work.tex]

\section{Limitations and Future Work}
\label{appx_sec-limitations_and_future_work}

While our method demonstrates strong generalization and robustness, the selection of its parameters (e.g., the weight range) remains empirical and may not be universally applicable. 
Future work could replace these manually selected hyper-parameters with learnable parameters, thereby adapting to a broader range of scenarios and potentially achieving better performance. 

Additionally, our proposed approach of monitoring the dynamic importance of network components using the Importance Probe, as well as the method of enhancing network capacities based on importance, may be transferable to other domains.
