# Supplementary material for: Dynamic Importance in Diffusion U-Net for Enhanced Image Synthesis
Source: arXiv:2504.03471 source file (2025-05-05)
Supplement: Supplementary file 8 [file more_discussion_on_proposition_1.tex]

\setcounter{proposition}{0}

\section{Supplementary Proof and Analysis of Proposition 1}
\label{appx_sec-supplementary_proof_and_analysis_of_proposition_1}

We first prove Prop. ~\ref{prop-reweighting} in the main paper, and provide more discussion. 

\begin{proposition}
    \label{prop-reweighting_appx}
    
    (Prop.~\ref{prop-reweighting} in the main paper) The variance of the error
    \begin{equation}
        \label{eq-the_variance_of_error_appx}
        \begin{split}
            & \text{Var}(\Delta \hat{\pmb{\epsilon}}) 
            \approx \textstyle\sum_i A_i^2 (w_i - 1)^2 
            \text{Var} (\pmb{g}_i (\pmb{\epsilon}) )
            \\ 
            &~~~~ + 
            \textstyle\sum_i A_i^2 w_i^2 \text{Var}(\pmb{f}_i (\pmb{x}_0)) 
            + 
            \textstyle\sum_i A_i^2 w_i^2 \text{Var}(\pmb{n}_i)
            , 
        \end{split}
    \end{equation}
    where $A_i$ denotes the mapping transformation from the output of the $i$-th Transformer block to the final noise prediction. 
\end{proposition}

\subsection{Preliminary} 

Given a clean sample $\pmb{x}_0$ and a variance schedule $\{\overline{\alpha}_i\}_{i = 1}^n$, the forward process of DDIM~\cite{song2022denoisingdiffusionimplicitmodels} can be written as
\begin{equation}
    \pmb{x}_t 
    = 
    \sqrt{\overline{\alpha}_t} \pmb{x}_0 + \sqrt{1 - \overline{\alpha}_t} \pmb{\epsilon}
    , 
\end{equation}
where $\pmb{\epsilon} \sim \mathcal{N}(\pmb{0}, \pmb{I})$ is the true noise. 

The deterministic reverse step is
\begin{equation}
    \pmb{x}_{t - 1}
    = 
    \sqrt{\overline{\alpha}_{t - 1}} \left(\dfrac{\pmb{x}_t - \sqrt{1 - \overline{\alpha}_t} \hat{\pmb{\epsilon}}_t}{\sqrt{\overline{\alpha}_t}}\right) + \sqrt{1 - \overline{\alpha}_{t - 1}} \hat{\pmb{\epsilon}}_t
    , 
\end{equation}
where $\hat{\pmb{\epsilon}}_t = \pmb{\epsilon}_\theta (\pmb{x}_t, t)$ represents the noise predicted by the U-Net parameterized by $\theta$ at time step $t$. 

The signal-to-noise ratio (SNR) in this single step is defined as
\begin{equation}
    \text{SNR} (\pmb{x}_t) 
    = 
    \dfrac{||\pmb{x}_0||^2}{\text{Var} (\Delta\pmb{\epsilon}_t)}
    = 
    \dfrac{||\pmb{x}_0||^2}{\text{Var} (\pmb{\epsilon} - \hat{\pmb{\epsilon}}_t)}
    , 
\end{equation}
where the numerator $||\pmb{x}_0||^2$ represents the \emph{power} of the true signal $\pmb{x}_0$, and the denominator $\Delta \pmb{\epsilon}_t = \pmb{\epsilon} - \hat{\pmb{\epsilon}}_t$ denotes the \emph{error} between the true noise $\pmb{\epsilon}$ and the predicted noise $\hat{\pmb{\epsilon}}_t$. 

% 双栏
\begin{table*}[t]
    \caption{
        (Tab.~\ref{tab-comparison_between_different_models_and_steps} in the main paper) 
        Comparison between different models and inference steps. 
        Cells with a red/orange/yellow background indicate the best/second-best/third-best performance, respectively.  
        Cells where the weighted performance is worse than the vanilla schedule are marked with a downward arrow $\downarrow$. 
        Blocks within the SD/SDXL family are numbered from 0/1 for symmetry. 
    }
    \centering
    \begin{tabular}{c | c c c : c c c | c c c : c c c}
        \hline
        \multirow{2}{*}{\textbf{Weighting}} &
        \multicolumn{3}{c:}{\textbf{SD-Turbo}} & 
        \multicolumn{3}{c|}{\textbf{SDXL-Turbo}} & 
        \multicolumn{3}{c:}{\textbf{SD v2.1}} & 
        \multicolumn{3}{c}{\textbf{SDXL}} \\
        ~ & 1 & 2 & 3 & 1 & 2 & 3 &
        10 & 15 & 20 & 10 & 15 & 20 \\

        \hline
        Vanilla & 
        0.2961 & 0.3059 & 0.3034 & 
        0.2587 & 0.2693 & 0.2666 & 
        0.2876 & 0.2908 & 0.2932 & 
        0.2830 & \tbest{0.2889} & \tbest{0.2904} \\

        \hdashline

        blk-0 & 
        \sbest{0.2987} & \best{0.3088} & \tbest{0.3045} & 
        / & / & / & 
        0.2860$\downarrow$ & 0.2915 & \sbest{0.2946} & 
        / & / & / \\
        
        blk-1 & 
        \best{0.2993} & 0.3066 & 0.3019$\downarrow$ & 
        \best{0.2591} & 0.2685$\downarrow$ & 0.2666 & 
        \tbest{0.2881} & 0.2908 & \tbest{0.2943} & 
        \sbest{0.2863} & \best{0.2907} & \best{0.2924} \\
        
        blk-2 & 
        0.2966 & 0.3065 & 0.3037 & 
        0.2584$\downarrow$ & 0.2686$\downarrow$ & 0.2661$\downarrow$ & 
        0.2880 & 0.2896$\downarrow$ & 0.2935 & 
        0.2842 & 0.2886$\downarrow$ & 0.2889$\downarrow$ \\
        
        blk-3 & 
        0.2962 & 0.3055$\downarrow$ & 0.3035 & 
        \sbest{0.2589} & \best{0.2697} & \tbest{0.2668} & 
        0.2876 & 0.2909 & 0.2934 & 
        0.2839 & 0.2877$\downarrow$ & 0.2898$\downarrow$ \\
        
        blk-4 & 
        0.2965 & \sbest{0.3074} & \sbest{0.3052} & 
        \tbest{0.2588} & \sbest{0.2695} & \best{0.2671} & 
        \sbest{0.2894} & \tbest{0.2917} & 0.2939 & 
        \tbest{0.2851} & \tbest{0.2889} & 0.2892$\downarrow$ \\
        
        blk-5 & 
        \tbest{0.2981} & 0.3066 & \best{0.3062} & 
        0.2576$\downarrow$ & \tbest{0.2694} & \sbest{0.2670} & 
        \best{0.2902} & \best{0.2923} & \best{0.2950} & 
        \best{0.2868} & \sbest{0.2904} & \best{0.2910} \\
        
        blk-6 & 
        0.2962 & \tbest{0.3072} & 0.3025$\downarrow$ & 
        / & / & / & 
        0.2880 & \sbest{0.2919} & 0.2927$\downarrow$ & 
        / & / & / \\
        
        \hline
    \end{tabular}
    \label{tab-comparison_between_different_models_and_steps_appx}
\end{table*}

\subsection{Modeling the Noise Prediction in U-Net} 

The Transformer blocks~\cite{vaswani2023attentionneed} within the U-Net~\cite{ronneberger2015unetconvolutionalnetworksbiomedical, petit2021unettransformerselfcross} process the input $\pmb{x}_t$, whose output contains features associated with both the signal components and the noise components. 
Specifically, the output of the $i$-th Transformer block can be modeled as
\begin{equation}
    \pmb{y}_i 
    = 
    \pmb{f}_i (\pmb{x}_0) + \pmb{g}_i (\pmb{\epsilon}) + \pmb{n}_i
    , 
\end{equation}
where:

\begin{itemize}
    \item $\pmb{f}_i (\pmb{x}_0)$: The feature components related to the signal $\pmb{x}_0$. 

    \item $\pmb{g}_i (\pmb{\epsilon})$: The feature components related to the noise $\pmb{\epsilon}$. 

    \item $\pmb{n}_i$: The intrinsic noise of the Transformer block, which is introduced by approximation errors or nonlinearities within the block. 
\end{itemize}

The attention mechanisms within the pre-trained Transformer blocks, including self-attention and cross-attention, are capable of distinguishing between the signal and the noise components in the input latent. 
As a result, $\pmb{f}_i (\pmb{x}_0)$ primarily captures the signal information, while $\pmb{g}_i (\pmb{\epsilon})$ mainly captures the noise information. 
These two components are not independent, as both are influenced by the noisy input $\pmb{x}_t$. 

For simplicity, we assume that: 

\begin{itemize}
    \item The signal components $\pmb{f}_i (\pmb{x}_0)$s of all Transformer blocks are independent of each other, so do the noise components $\pmb{g}_i (\pmb{\epsilon})$s. 
    
     \item$\pmb{f}_i (\pmb{x}_0)$ is independent of $\pmb{g}_j (\pmb{\epsilon})$ for any $(i, j)$ pair. 

    \item $\pmb{n}_i$ has zero mean and a fixed variance $\text{Var} (\pmb{n}_i)$. 

    \item The intrinsic errors $\pmb{n}_i$s of all Transformer blocks are independent of each other, as well as independent of the true noise $\pmb{\epsilon}$ and the noise prediction $\pmb{\epsilon}_t$. 
\end{itemize}

The output $\pmb{y}_i$ of each Transformer block in processed by the subsequent blocks (such as ResNet~\cite{he2016deep} blocks), ultimately forming the noise prediction of the U-Net: 
\begin{equation}
    \hat{\pmb{\epsilon}}_t 
    = 
    \pmb{h}(\{\pmb{y}_i\})
    .
\end{equation}

For simplicity, we assume that $\pmb{h}(\cdot)$ is a linear combination of the outputs from the Transformer blocks: 
\begin{equation}
    \hat{\pmb{\epsilon}}_t 
    = 
    \sum_i A_i \pmb{y}_i
    = 
    \sum_i A_i (\pmb{f}_i (\pmb{x}_0) + \pmb{g}_i (\pmb{\epsilon}) + \pmb{n}_i)
    ,
\end{equation}
where $A_i$ denotes the mapping transformation from the output of the $i$-th Transformer block to the final noise prediction. 

\subsection{Re-weighting the Output of Transformer Blocks}

We propose to re-weight the output of the $i$-th $(i = 0, 1, \cdots)$ Transformer block by a scaling factor $w_i > 0$ before passing it to the subsequent ResNet block (see Fig.~\ref{fig-weighted_u_net_appx}). 

After re-weighting, the output of the $i$-th Transformer block becomes
\begin{equation}
    \pmb{y}_i' 
    = 
    w_i \pmb{y}_i, 
\end{equation}
while the noise prediction becomes
\begin{equation}
    \hat{\pmb{\epsilon}}_t' 
    = 
    \sum_i A_i \pmb{y}_i'
    = 
    \sum_i A_i w_i (\pmb{f}_i (\pmb{x}_0) + \pmb{g}_i (\pmb{\epsilon}) + \pmb{n}_i)
    .
\end{equation}

% 图: U-Net 加权
\begin{figure}[h]
    \centering
    \includegraphics[width=0.98\linewidth]{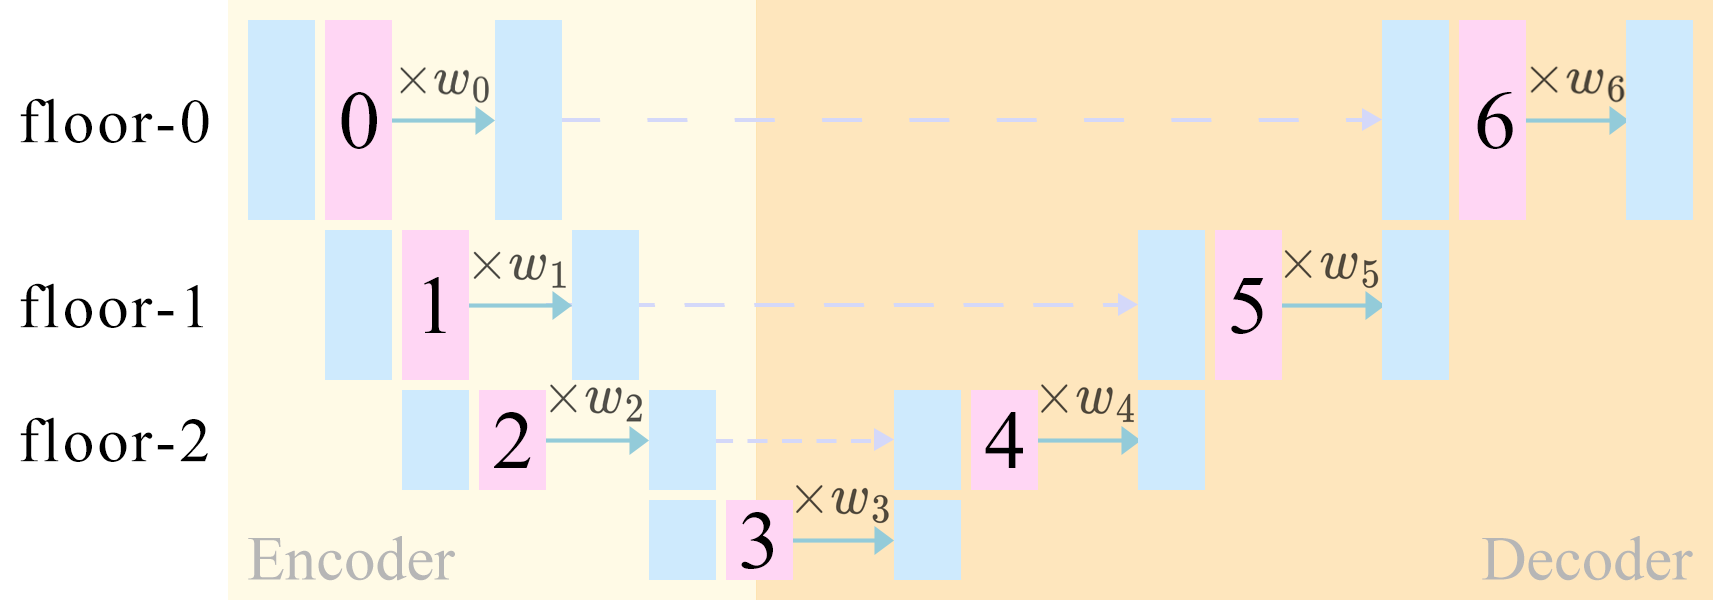}
    \caption{
        (Fig. 1 in the main paper) 
        Schematic of scaling the outputs of seven Transformer blocks before passing to the subsequent ResNet~\cite{he2016deep} blocks. 
        The blue rectangles represent the ResNet blocks, while the pink ones stand for the Transformer blocks. 
    }
    \label{fig-weighted_u_net_appx}
\end{figure}

\subsection{The Impact of Re-weighting on SNR}

The prediction error
\begin{equation}
    \Delta \hat{\pmb{\epsilon}}_t' 
    = 
    \pmb{\epsilon} - \hat{\pmb{\epsilon}}_t'
    = 
    \pmb{\epsilon} 
        - 
        \sum_i A_i w_i (\pmb{f}_i (\pmb{x}_0) + \pmb{g}_i (\pmb{\epsilon}) + \pmb{n}_i)
    . 
\end{equation}

The U-Net $\pmb{\epsilon}_\theta (\cdot)$ learns to predict noise from a noisy sample, which is trained with the objective
\begin{equation}
    \mathcal{L}_{\text{DM}}
    = 
    \mathbb{E}_{\pmb{x}_0, t, \pmb{\epsilon}} 
        ||
            \epsilon_\theta (\pmb{x}_t, t) - \pmb{\epsilon}
        ||_2^2. 
\end{equation}

Thus, 
\begin{equation}
    \sum_i A_i \pmb{g}_i (\pmb{\epsilon}) \approx \pmb{\epsilon}
    . 
\end{equation}

The variance of the error 
\begin{equation}
    \begin{split}
        &\text{Var} (\Delta \hat{\pmb{\epsilon}}_t')
        \\
        &= \text{Var}
            \left(
                \pmb{\epsilon} 
                - 
                \sum_i A_i w_i (\pmb{f}_i (\pmb{x}_0) + \pmb{g}_i (\pmb{\epsilon}) + \pmb{n}_i)
            \right)
        \\
        &\approx \text{Var}
            \left(
                \sum_i 
                [
                    A_i (w_i - 1) \pmb{g}_i (\pmb{\epsilon})
                    + A_i w_i \pmb{f}_i (\pmb{x}_0)
                    + A_i w_i \pmb{n}_i
                ]
            \right)
        \\
        &= 
            \sum_i A_i^2 (w_i - 1)^2 
            \text{Var} (\pmb{g}_i (\pmb{\epsilon}) )
            + 
            \sum_i A_i^2 w_i^2 \text{Var}(\pmb{f}_i (\pmb{x}_0))
        \\
        &~~~~+ 
            \sum_i A_i^2 w_i^2 \text{Var}(\pmb{n}_i)
        .
    \end{split}
    \label{eq-the_variance_of_the_error_appx}
\end{equation}

Thus, we have demonstrated Proposition 1. 

Note that, at any time step $t$, the variances $\text{Var}(\pmb{g}_i (\pmb{\epsilon}) )$, $\text{Var}(\pmb{f}_i (\pmb{x}_0))$ and $\text{Var}(\pmb{n}_i)$ are deterministic. 
To reduce $\text{Var} (\Delta \hat{\pmb{\epsilon}}_t')$, based on the \emph{rearrangement inequality}, we need to design a set of weights $\{w_i\}$ that assign higher weights to terms with smaller variances, while assign lower weights to terms with larger variances. 
Specifically: 

\begin{itemize}
    \item When $t$ is large, i.e., when the noise level is high, we should assign greater weights to blocks that can accurately distinguish the noise, namely those with smaller $\text{Var}(\pmb{g}_i)$. 

    \item When $t$ is small, i.e., when the noise level is low, we should assign greater weights to blocks that can accurately distinguish the signal, namely those with smaller $\text{Var}(\pmb{f}_i)$. 

    \item For all $t$, we should assign smaller weights to blocks with larger intrinsic noise, i.e., those with larger $\text{Var}(\pmb{n}_i)$. 
    It can also be seen as a measurement of the \emph{aleatoric uncertainty}
    \footnote{
        The aleatoric uncertainty refers to the inherent randomness or variability in the system or data. 
        It arises from stochastic processes or inherent noise in observations. 
        It cannot be reduced even with more information. 
    }
    \cite{der2009aleatory} of the block. 
\end{itemize}

By designing appropriate weights $\{w_i\}$, we can reduce $\text{Var} (\Delta \hat{\pmb{\epsilon}}_t')$, thus increasing the SNR. 
Simultaneously, we should balance the noise prediction and the signal prediction to avoid $\{w_i\}$ to misweight contributions of components, leading to degrade the denoising capability of the U-Net. 

\subsection{Relationships between Importance and Uncertainty}

On the one hand, high uncertainty often suggests high importance, as vital blocks tend to exhibit greater response variation when perturbed. 
This is because the model relies heavily on these blocks, making their outputs more sensitive to adjustments.

On the other hand, the capabilities of blocks with critical importance may be limited due to their unstable behavior. 
In other words, there exists an antagonistic relationship between importance and uncertainty. 
It necessitates additional constraints or adjustments (e.g., our proposed importance-based re-weighting schedule) for better and more stable performance. 

In summary, importance highlights the Transformer blocks within the U-Net that are most critical to the generation process, while uncertainty measures how robust or reliable their contributions are. 
Together, they offer a holistic view of the U-Net mechanisms, where importance indicates necessity, and uncertainty highlights stability, expanding the interpretability of DMs.

\subsection{Empirical Re-weighting Strategy}
\label{appx_sec-more_discussion_on_proposition_1-subsection-empirical_reweighting_strategy}

Our proposed \emph{Importance Probe} (IP) is designed to monitor the dynamic importance of the Transformer blocks throughout the denoising process. 
It can adaptively distinguish the importance of each block based on the denoising focus at each time step, which is measured by the mean squared error (MSE) between the noise predictions without explicit specification. 
The importance of each block is then quantified through the voting mechanism. 
More over, results from several runs of IP are aggregated via the voting mechanism, which helps to mitigate the impact of intrinsic noise $\pmb{n}_i$ on the importance ranking. 

By applying an importance-based re-weighting schedule, we can assign greater weights to the blocks that play a dominant role at each step, thereby increasing the SNR. Specifically: 

\begin{itemize}
    \item It is more likely to assign greater weights to bottleneck blocks, as they encode high-level features, and serve as the nexus between the encoder and decoder.
    
    \item In the early denoising, it is more likely to assign greater weights to mid-low-resolution blocks, emphasizing terms with smaller $\text{Var} (\pmb{f}_i)$. 

    \item In the later denoising, it is more likely to assign greater weights to high-resolution blocks, emphasizing terms with smaller $\text{Var} (\pmb{g}_i)$. 

    \item Throughout denoising, it is more likely to assign smaller weights to blocks with larger intrinsic noise, suppressing terms with larger $\text{Var} (\pmb{n}_i)$.
\end{itemize}
