# Supplementary material for: Dynamic Importance in Diffusion U-Net for Enhanced Image Synthesis
Source: arXiv:2504.03471 source file (2025-05-05)
Supplement: Supplementary file 9 [file threshold_update_schedule_details.tex]

\section{Threshold Update Schedule Details}

\subsection{Threshold Update Schedule}

Let ``the weight set is accepted" to be event $A$, and ``the current threshold being too high, moderate, or too low" be events $B_1$, $B_2$ and $B_3$, respectively. 

Let $Q = [\pmb{q}_1, \cdots, \pmb{q}_n]$ be the current optimal threshold matrix, where $n$ is the number of inference steps and $\pmb{q}_i \in [0, 1]^m\ \ (1 \leq i \leq n)$ stands for the optimal thresholds for the $m$ target blocks. 

If an optimal weight matrix $W = [\pmb{w}_1, \cdots, \pmb{w}_n]$ is found during an iteration, where $\pmb{w}_i \in [0, 1]^m\ \ (1 \leq i \leq n)$ represents the optimal weights for the $m$ target layers, then the new thresholds matrix $Q' = [\pmb{q}_1', \cdots, \pmb{q}_n']$ are obtained as follows:

For an accepted weight set $\pmb{w}_i$ :

\begin{equation}
    \begin{aligned}
        \pmb{q}_i' =
        &~ P(B_1 \mid A) \times (\pmb{q}_i / 2) \\
        &+ P(B_2 \mid A) \times \pmb{q}_i + P(B_3 \mid A) \times (\pmb{w}_i - \varepsilon)
    \end{aligned}, 
    \label{eq-threshold_update_accpeted}
\end{equation}
while for a rejected one $\pmb{w}_j$:
\begin{equation}
    \begin{aligned}
        \pmb{q}_j' = 
        &~ P(B_1 \mid \overline{A}) \times (\pmb{q}_j / 2) \\
        &+ P(B_2 \mid \overline{A}) \times \pmb{q}_j + P(B_3 \mid \overline{A}) \times (\pmb{w}_j - \varepsilon)
    \end{aligned}, 
    \label{eq-threshold_update_rejected}
\end{equation}
where $\varepsilon$ is a minute positive number. 

Since the thresholds tend to stabilize to moderate values during the importance probe process, we set $P(B_2 \mid A)$ in Eq.~\ref{eq-threshold_update_accpeted} to linearly increase from $P_{\text{st}} (B_2 \mid A)$ to $P_{\text{ed}} (B_2 \mid A)$, and $P(B_3 \mid A)$ to linearly decrease from $P_{\text{st}} (B_3 \mid A)$ to $P_{\text{ed}} (B_3 \mid A)$. 
Similarly, in Eq.~\ref{eq-threshold_update_rejected}, $P(B_1 \mid \overline{A})$ and $P(B_2 \mid \overline{A})$ are set to decrease and increase, respectively. 

Compared to the common hard or soft update strategies, our conditional-expectation-based threshold update strategy can counteract the biases introduced by randomness in a stochastic environment, providing more reliable updates.

\subsection{Hyper-parameters}

We selected the following hyper-parameters for the Threshold Update Schedule across all tasks. 

\begin{table}[h]
    \centering
    \caption{
        Hyper-parameters for the Weight Threshold Update Schedule. 
    }
    \begin{tabular}{c | c}
        \hline
        Param Name & Value \\
        \hline

        $\epsilon$ & $1\text{e}-2$ \\

        \hdashline

        $P(B_1 \mid A)$ & $0.06$ \\
        $P_{\text{st}} (B_2 \mid A)$ & $0.47$ \\ 
        $P_{\text{ed}} (B_2 \mid A)$ & $0.84$ \\ 
        $P_{\text{st}} (B_3 \mid A)$ & $0.47$ \\ 
        $P_{\text{ed}} (B_3 \mid A)$ & $0.10$ \\ 

        \hdashline

        $P_{\text{st}} (B_1 \mid \overline{A})$ & $0.48$ \\ 
        $P_{\text{ed}} (B_1 \mid \overline{A})$ & $0.30$ \\ 
        $P_{\text{st}} (B_2 \mid \overline{A})$ & $0.48$ \\ 
        $P_{\text{ed}} (B_2 \mid \overline{A})$ & $0.66$ \\ 
        
        $P(B_3 \mid \overline{A})$ & $0.04$ \\ 

        \hline
    \end{tabular}
    \label{tab-hyper_parameter_weight_threshold_update_schedule}
\end{table}

\subsection{Limitations}

The conditional probabilities involved in the Threshold Update Schedule need to be empirically and manually selected, which may not be applicable to all scenarios.
